# Supplementary material for: Data Diversity as Implicit Regularization: How Does Diversity Shape the Weight Space of Deep Neural Networks?
Source: arXiv:2410.14602 source file (2025-08-15)
Supplement: Supplementary file 1 [file appendix11.tex]

% \subsection{Curvature Analysis of Loss Function Landscape}
% \textcolor{blue}{Revision: make this concise and precise. Put this complete analysis into the appendix 11}\\

Section 4.2.3 and Figure \ref{fig:loss_vis} demonstrate three stages in the model optimization process: \textit{Rapid updates}, \textit{Transition between sharp and flat regions}, and \textit{Convergence to a flat region}, verifying that a similar regularization effect exists between data augmentations with other regularization. We present category-wise loss function curvature visualizations to better understand them.

\begin{figure}[htb]
    \begin{subfigure}
        \centering
        \includegraphics[width=0.32\textwidth]{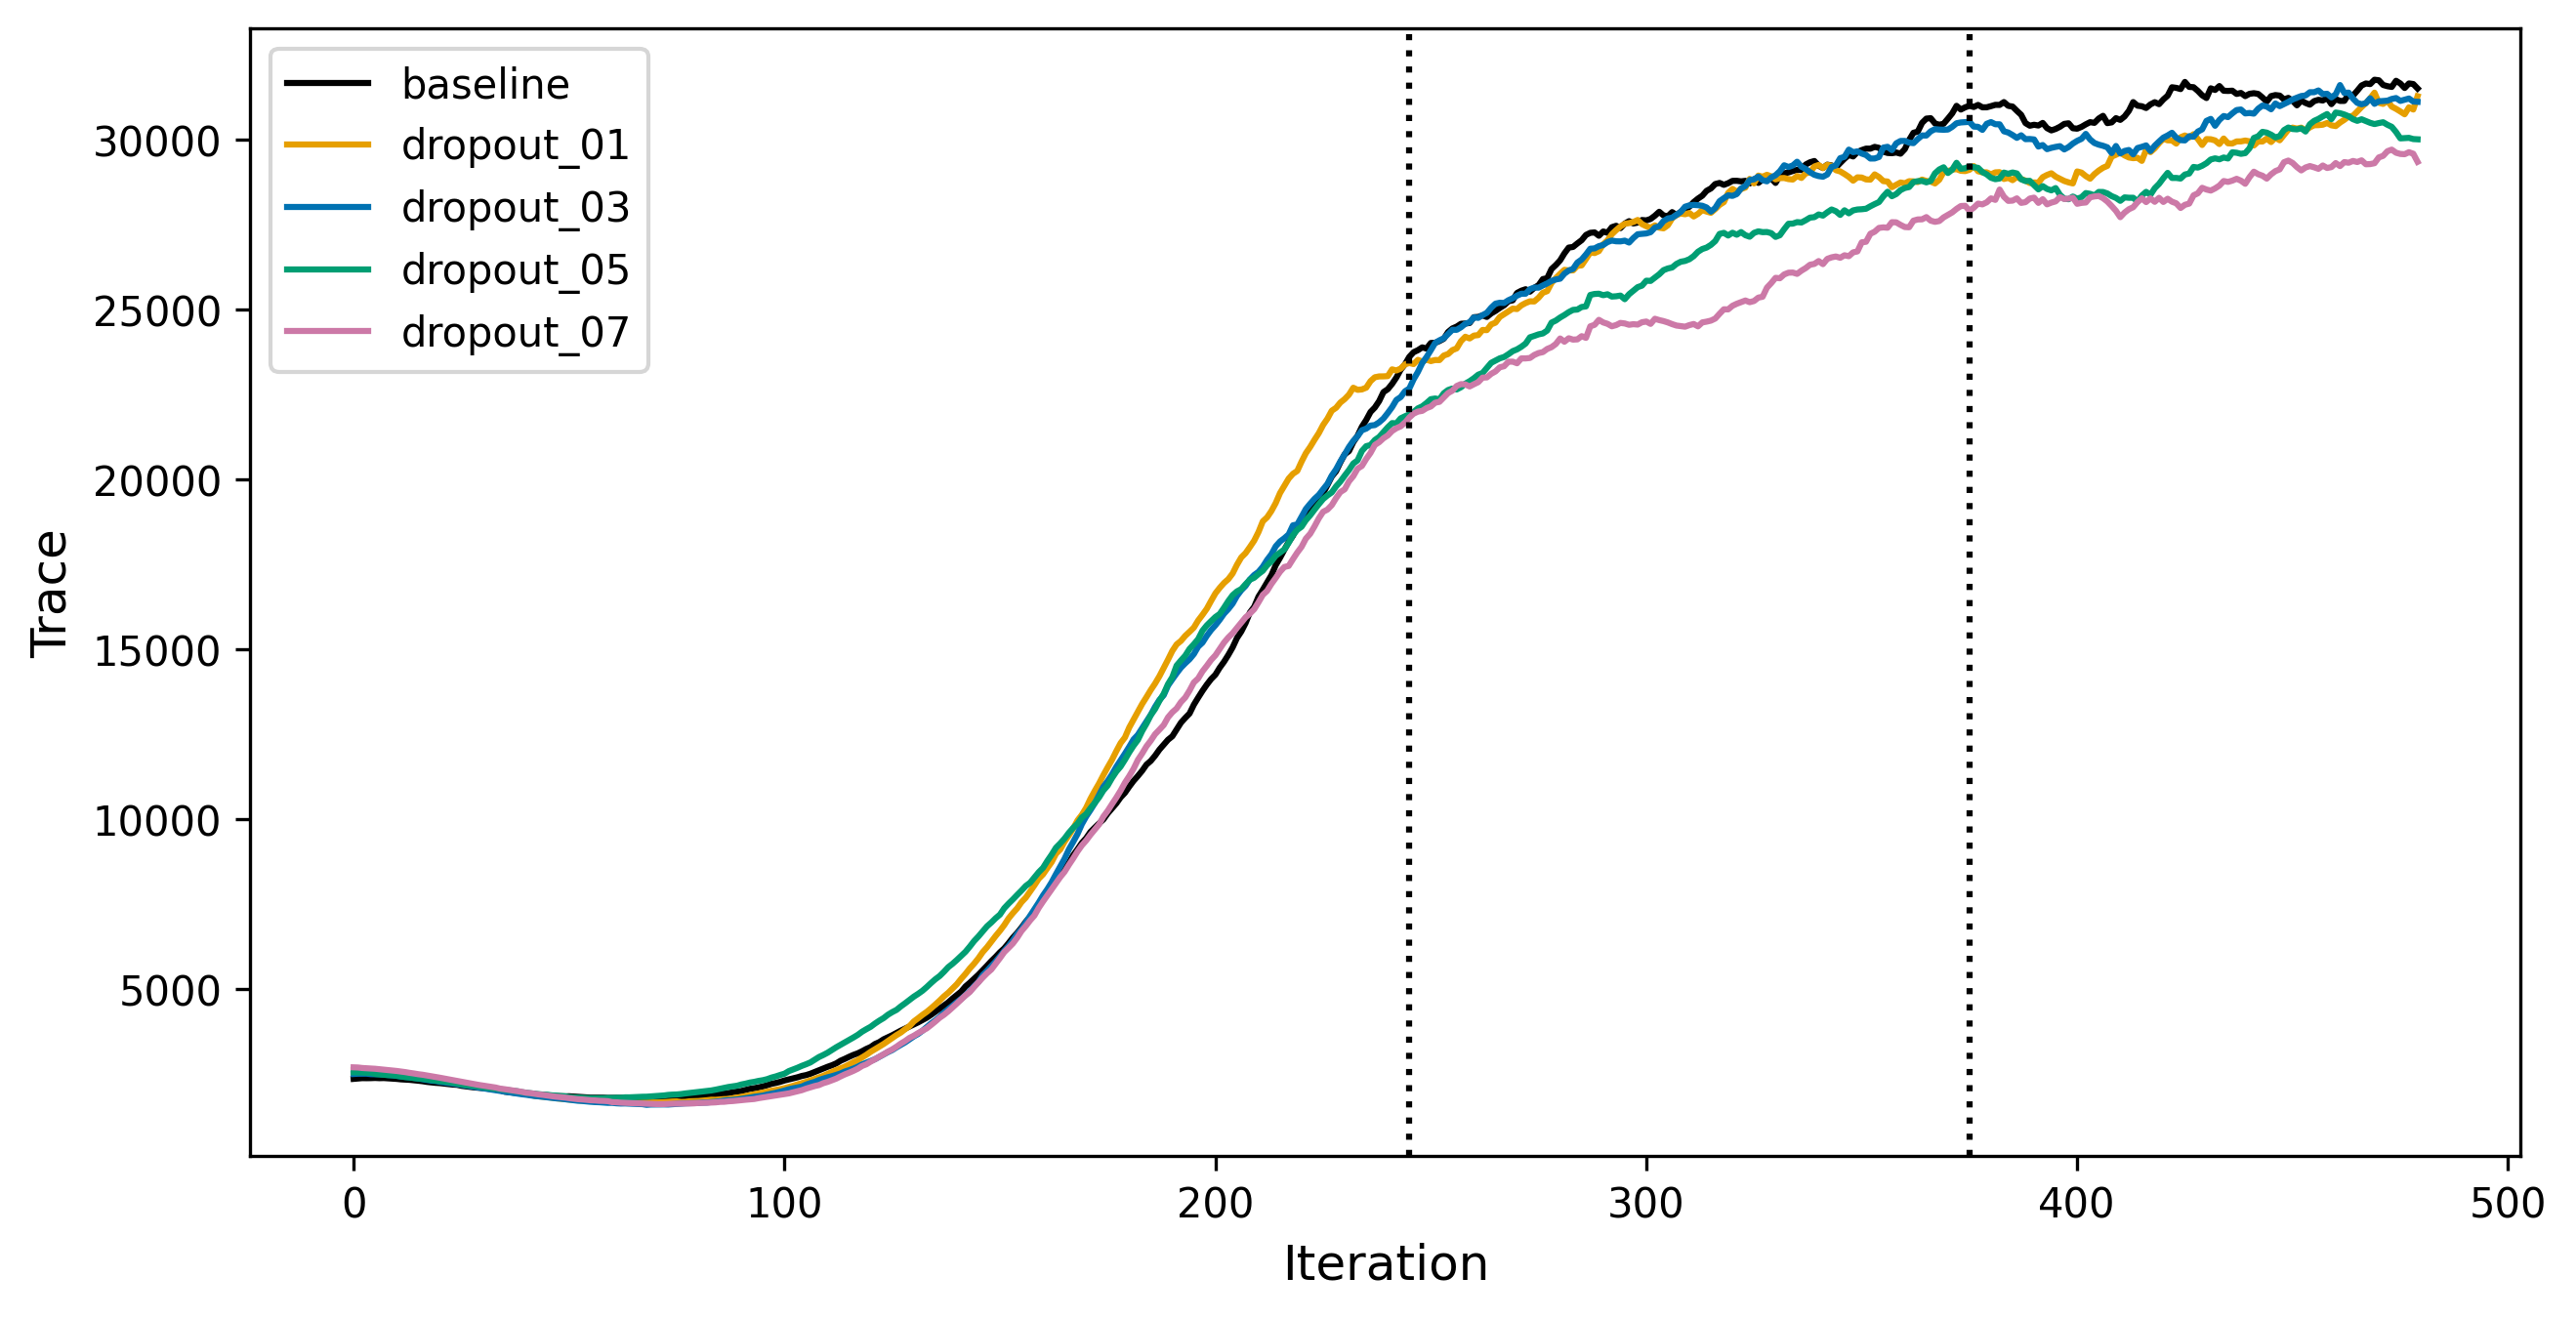}
        % \caption{Logarithmic scale}
        \label{fig:m1}
    \end{subfigure}
    % \hfill
    % Second subfigure (right column)
    \begin{subfigure}
        \centering
        \includegraphics[width=0.32\textwidth]{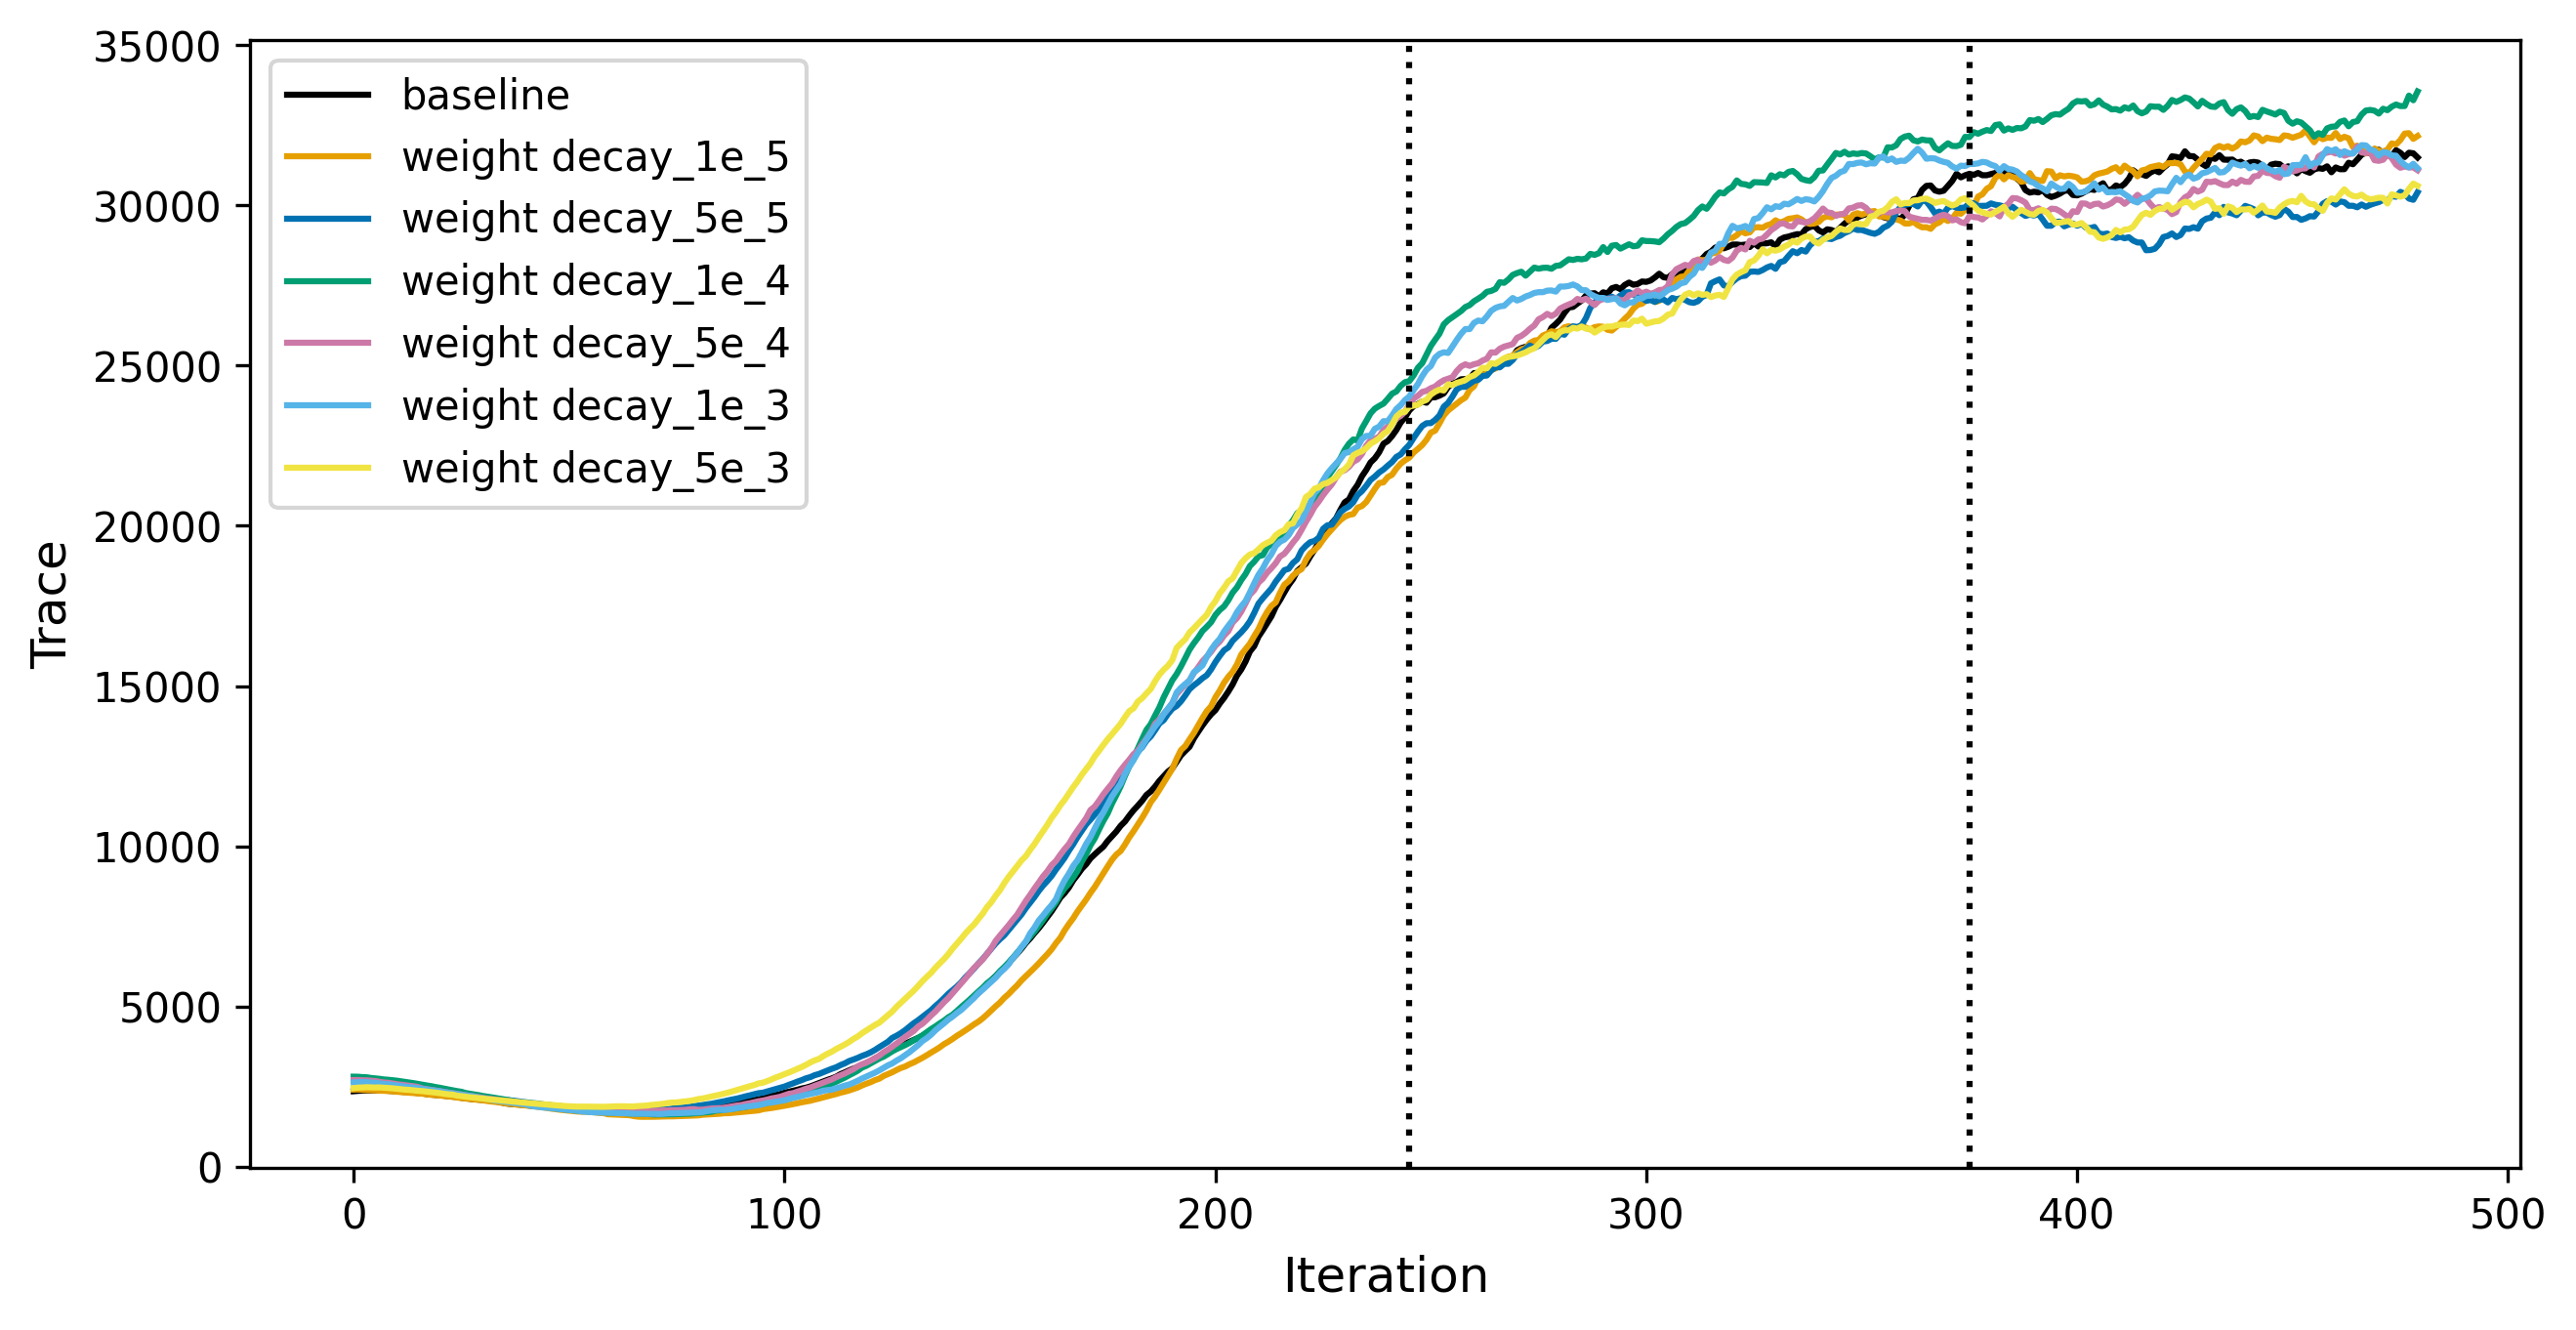}
        % \caption{Linear scale}
        \label{fig:m2}
    \end{subfigure}
    \begin{subfigure}
        \centering
        \includegraphics[width=0.32\textwidth]{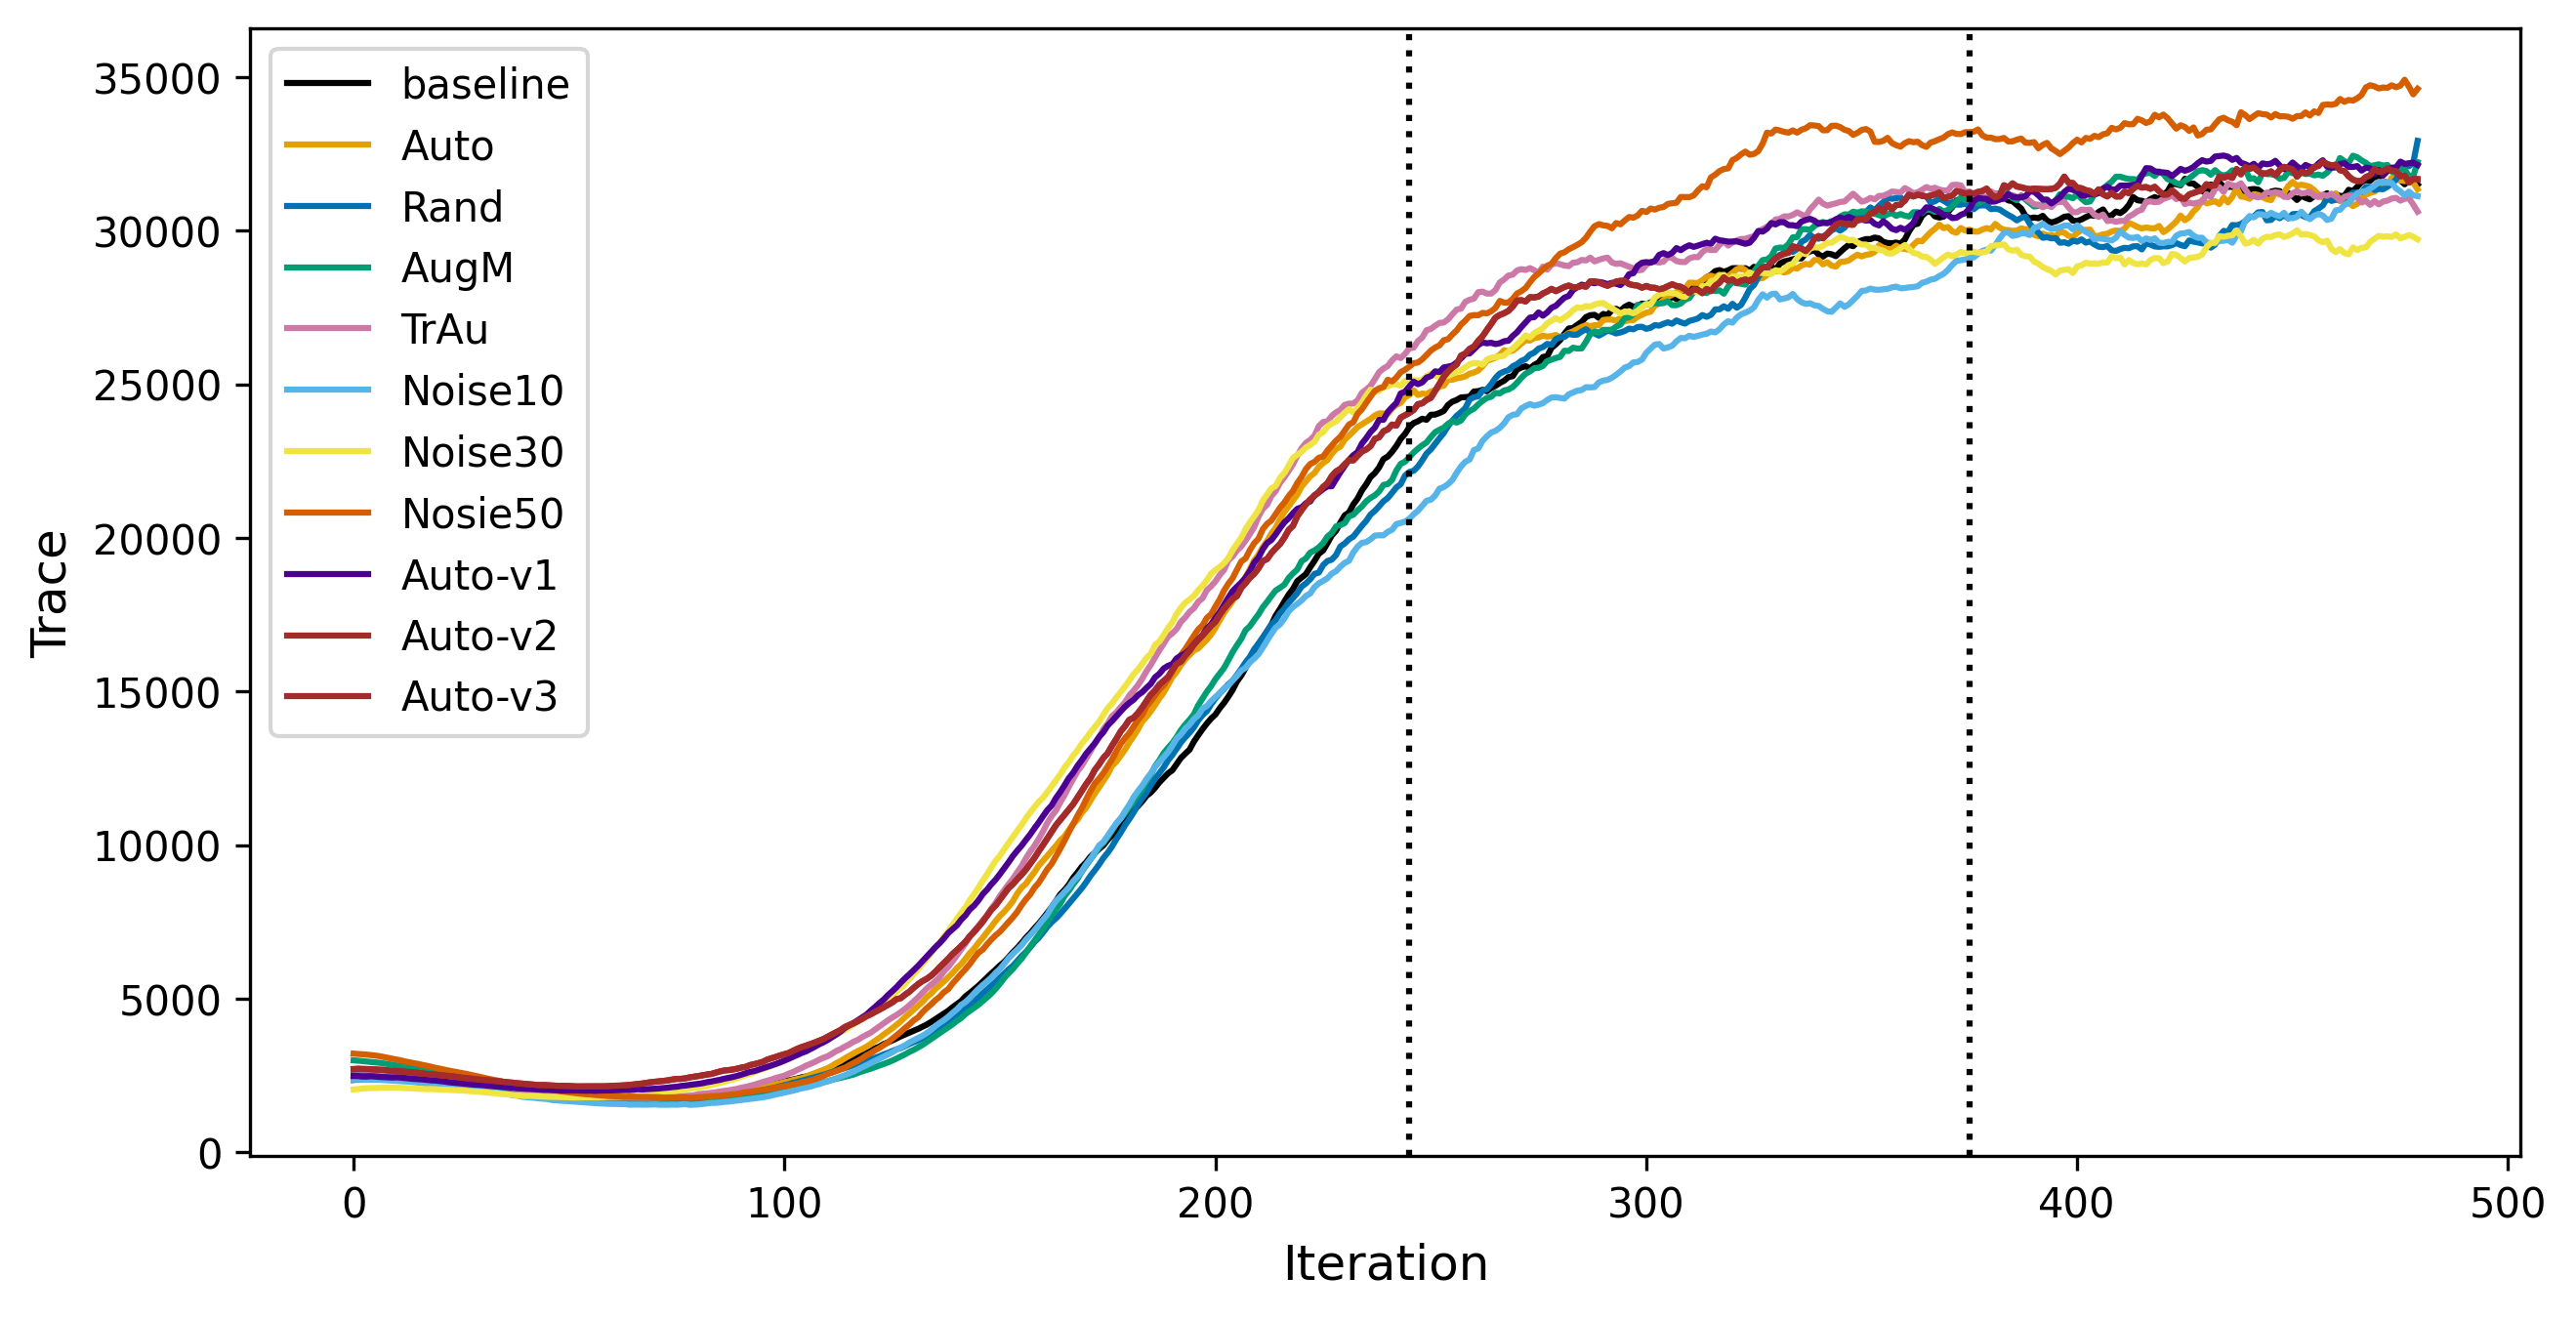}
        % \caption{Linear scale}
        \label{fig:m3}
    \end{subfigure}
    \caption{\textbf{Left:} loss function curvature for dropout,  \textbf{Middle:} loss function curvature for weight decay, and \textbf{Right:} loss function curvature for dropout for data augmentations. }
    \label{fig:loss-more}
\end{figure}

\textbf{Results.} In Figure \ref{fig:loss-more}, the left plot illustrates that dropout with higher rates, such as 0.5 and 0.7, exerts a stronger regularization effect, particularly in the later stages of training (Stage 2 and Stage 3), where their Hessian traces drop below the baseline. The higher the dropout rate, the more pronounced the effect. On the middle plot, we observe that a larger regularization term has a stronger impact on the trace of the Hessian, as seen with a weight decay value of 5e-3. The trace of the Hessian fluctuates more significantly during iterations 100 to 245 (Stage 1) and rapidly declines as training converges to a flat region (Stage 3), illustrating how regularization techniques influence the loss landscape. Finally, most data augmentations (the right plot) introduce additional information during Stage 1 (iterations 100 to 245), positioning the weight $W$ in a sharp region of the loss landscape and leading to an increase in the trace of the Hessian. As training progresses, the trace typically decreases in Stage 2 and falls below the baseline in Stage 3. However, advanced augmentation methods like Noise50 exhibit a different trend, with the Hessian trace continuing to grow, indicating a need for extended training time to reach the optimal solution.
