# Supplementary material for: Data Diversity as Implicit Regularization: How Does Diversity Shape the Weight Space of Deep Neural Networks?
Source: arXiv:2410.14602 source file (2025-08-15)
Supplement: Supplementary file 2 [file appendix9.tex]

\subsection{Limitation}

We conducted a series of comprehensive analyses and experiments across both vision and language tasks, encompassing a variety of datasets, model architectures, and training strategies, including training from scratch and fine-tuning. The models used in our study include CLIP-ViT-B/32, CLIP-ResNet-50, ResNet-18, and BERT. 

While we are confident that our theoretical framework and findings are generalizable, as evidenced by consistent patterns observed across diverse scenarios, we acknowledge that incorporating experiments with large language models (LLMs) would further strengthen our claims. Due to computational resource constraints, such experiments were not feasible. Nonetheless, since most modern LLMs are based on transformer architectures, we believe our conclusions remain applicable. This is further supported by the consistency of our findings in both transformer-based models studied—ViT and BERT.

\subsection{Impact Statement} 
This work advances our understanding of how data diversity shapes the weight landscape of deep neural networks and investigates its similarities with traditional regularization techniques such as dropout and weight decay. By framing data augmentation as an implicit regularizer, our findings provide a new perspective on why it improves generalization, particularly in low-data regimes where overfitting is a concern. The insights provided could guide the development of more robust machine learning models to make them better suited for real-world applications wherein training data is limited or expensive to obtain.

From a broader perspective, improving generalization and robustness introduces benefits across many domains, from medical diagnostics to security and autonomous systems. However, this work does not address potential biases introduced through data augmentation or the ethical considerations of synthetic data generation -- both of which are critical for ensuring fairness and reliability in deployed models, especially in high-stakes settings. Additionally, while data diversity can enhance performance, careless augmentation strategies may lead to unintended distribution shifts. Future research should explore ways to quantify and mitigate these risks to ensure that models trained with diverse data remain both reliable and equitable in practice.
