# Supplementary material for: Data Diversity as Implicit Regularization: How Does Diversity Shape the Weight Space of Deep Neural Networks?
Source: arXiv:2410.14602 source file (2025-08-15)
Supplement: Supplementary file 3 [file appendix0.tex]

\begin{figure}[h]
    \centering
    % First row
    \begin{subfigure}[b]{0.33\textwidth}
        \centering
        \includegraphics[width=\textwidth]{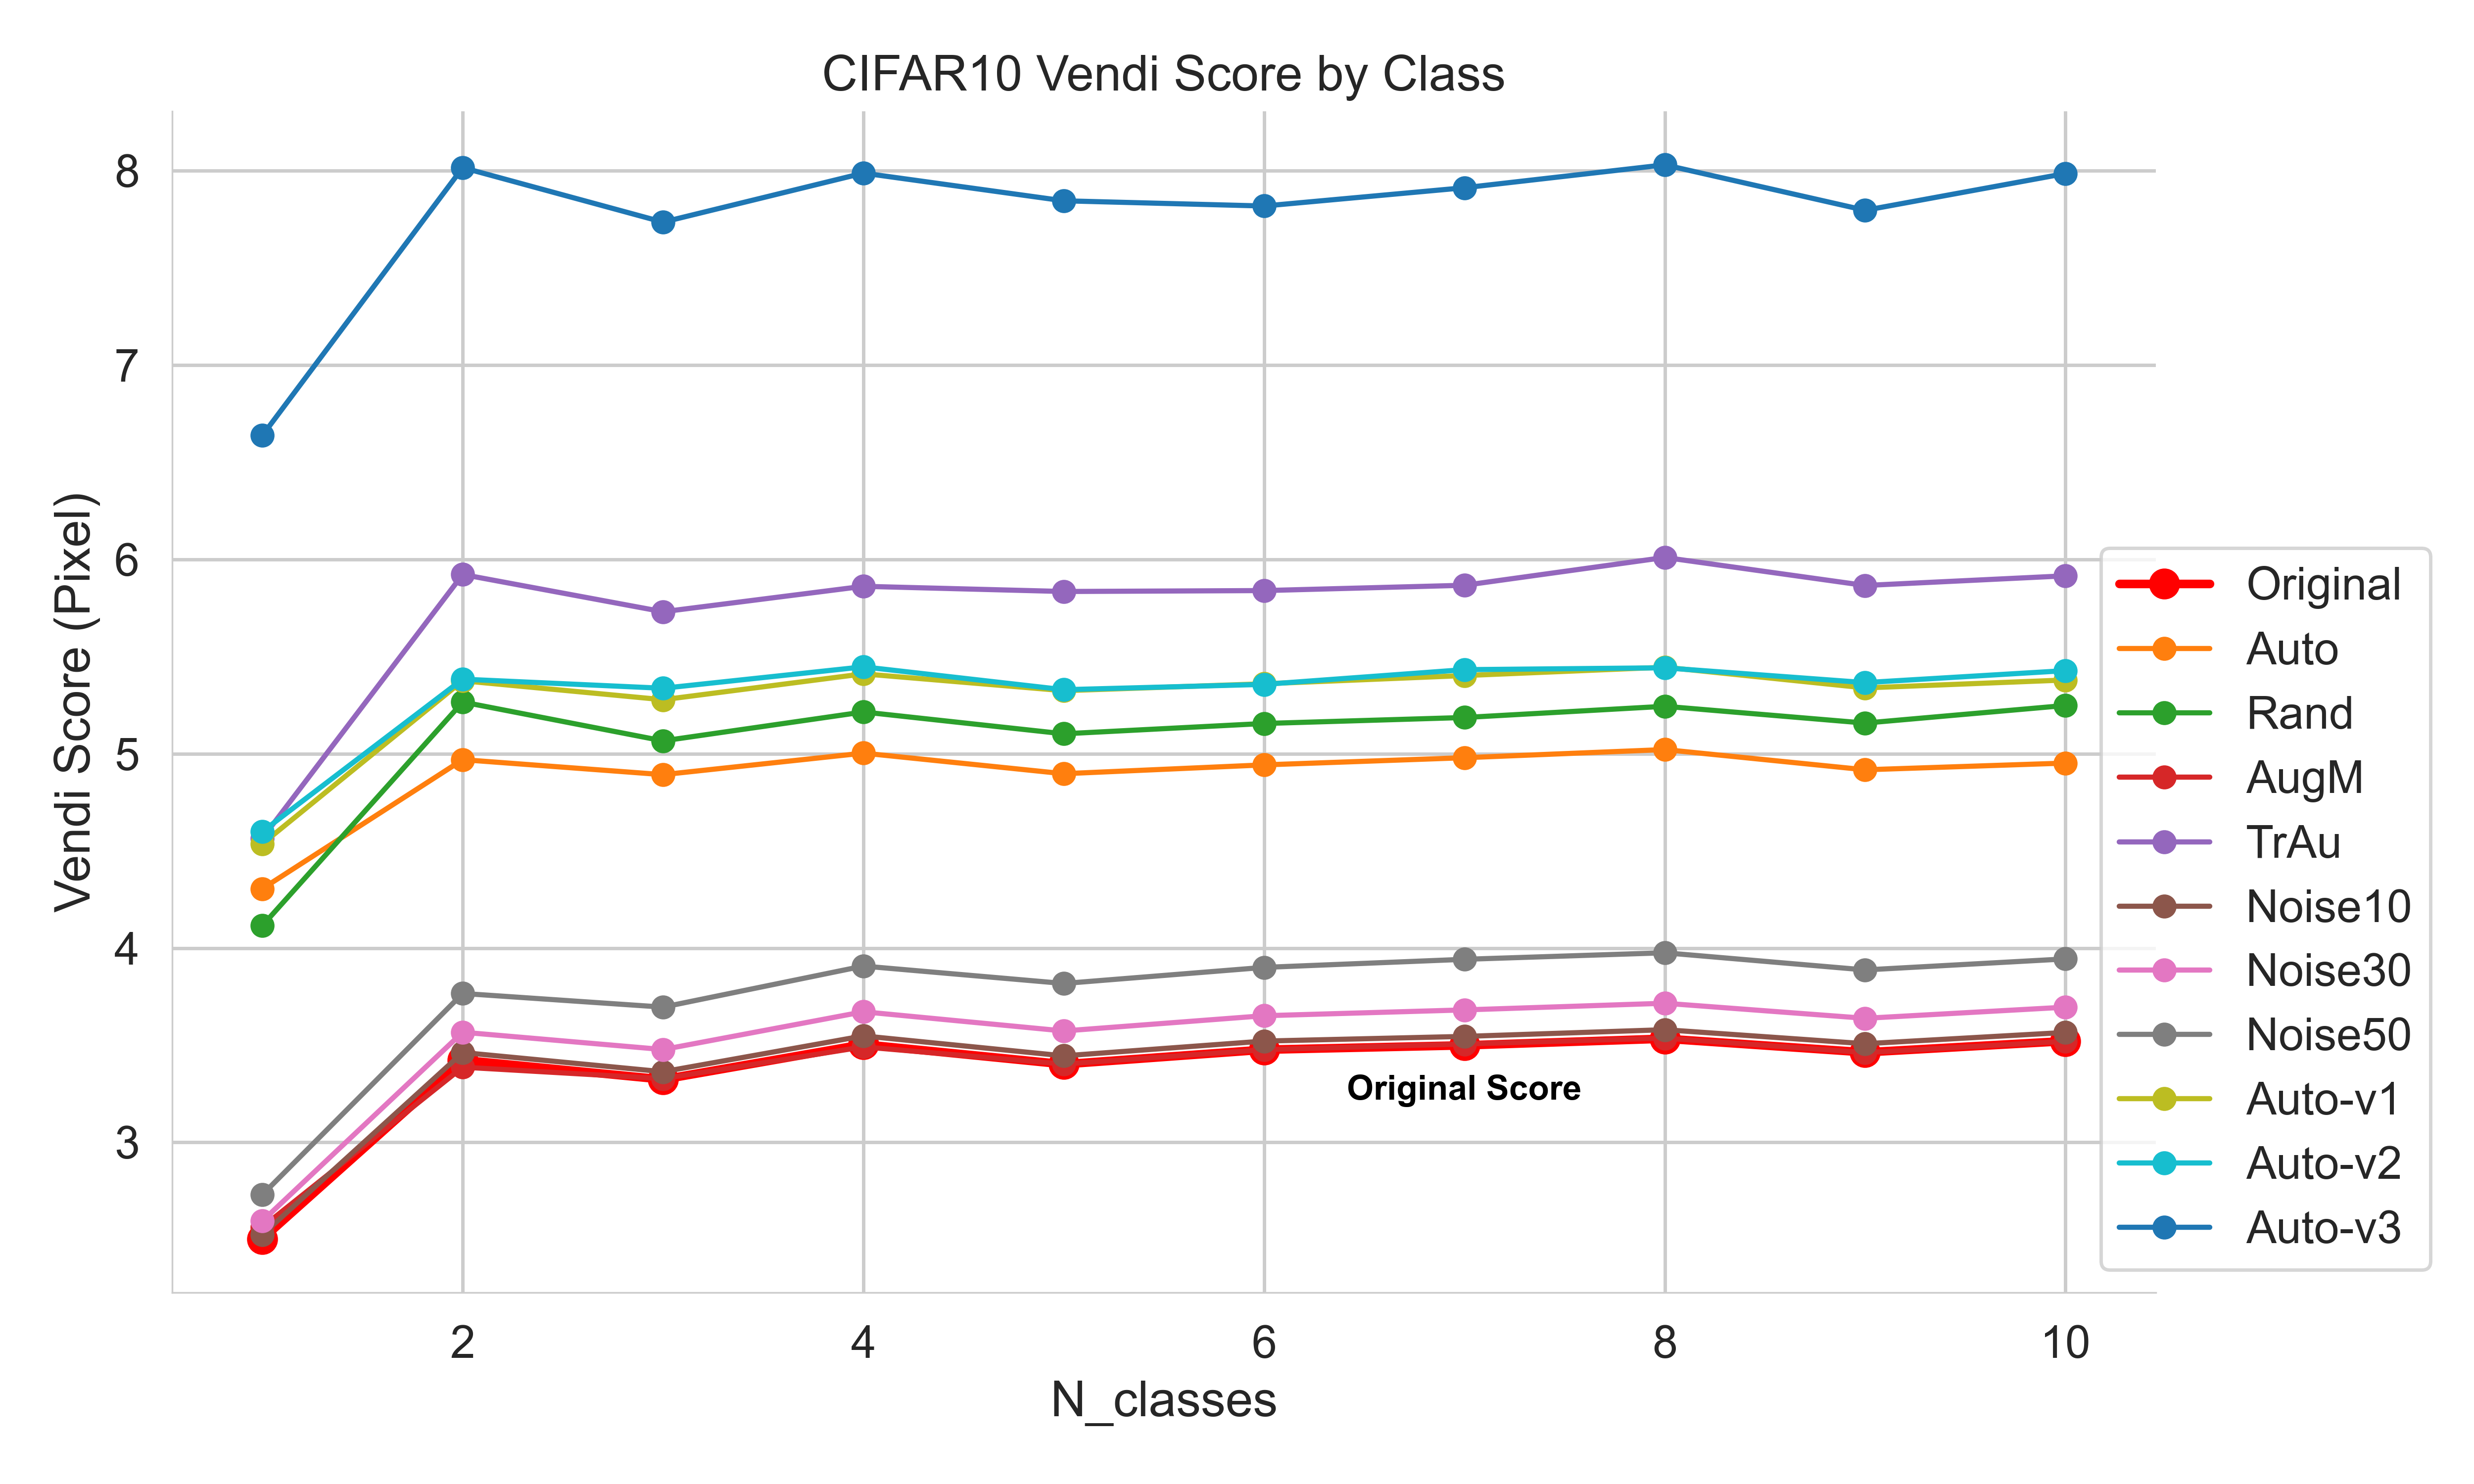}
        % \caption{Cf10}
        \label{fig:vs1}
    \end{subfigure}
    \hfill
    \begin{subfigure}[b]{0.33\textwidth}
        \centering
        \includegraphics[width=\textwidth]{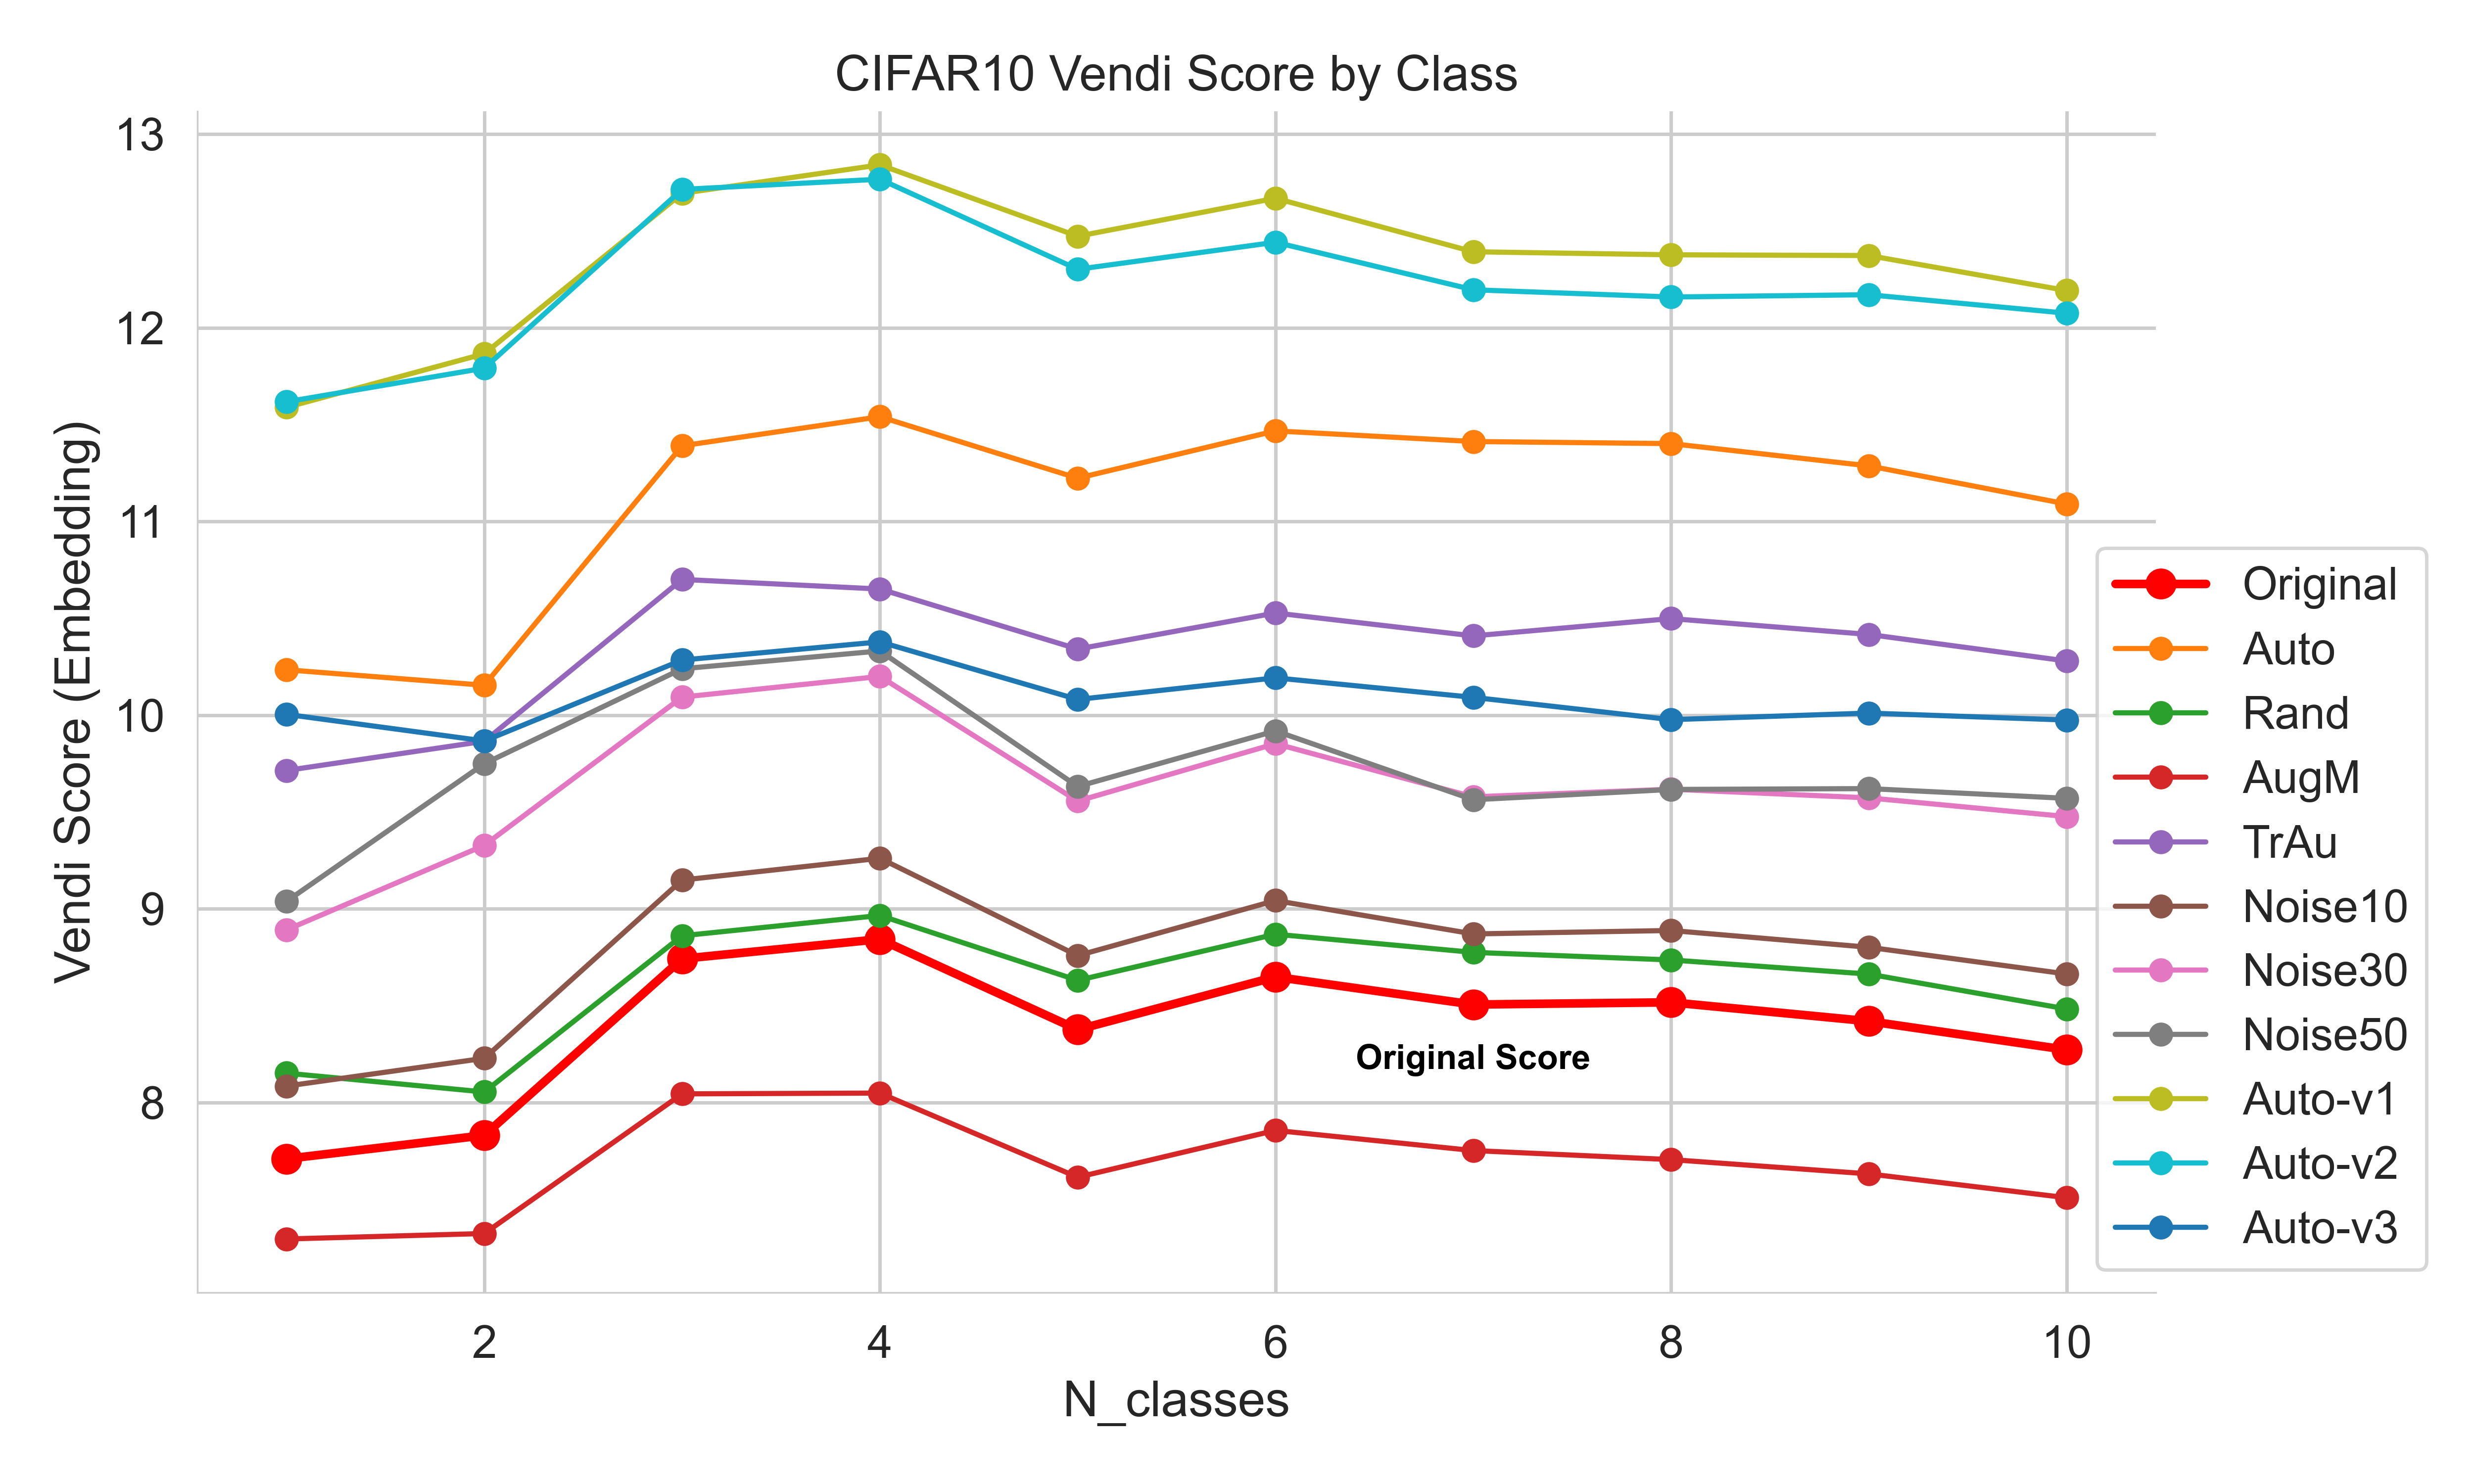}
        % \caption{Cf10}
        \label{fig:vs2}
    \end{subfigure}
    \hfill
  
    \caption{Data diversity on CIFAR-10 measured by Vendi Score. \textbf{Left} is the result based on pixel-wise similarity; \textbf{Right} is the result based on the similarity of embedding learned by CLIP. The red-colored line contains the VS values of the original CIFAR-10 dataset with different numbers of label classes. We employ automatic data augmentation packages to create other datasets: Auto, Rand, AugM, and TrAU. Noise10, Noise30, and Noise50 are created by adding Gaussian noise with a ratio of 0.1, 0.3, and 0.5. Auto-v1 to Auto-v3 are variants based on AutoAugment.}
    \label{fig:vs}
\end{figure}
