# Supplementary material for: Data Diversity as Implicit Regularization: How Does Diversity Shape the Weight Space of Deep Neural Networks?
Source: arXiv:2410.14602 source file (2025-08-15)
Supplement: Supplementary file 4 [file appendix1.tex]

We present more scale-shape plots here:

\begin{figure}[h]
    \centering
    % First row
    \begin{subfigure}[b]{0.3\textwidth}
        \centering
        \includegraphics[width=\textwidth]{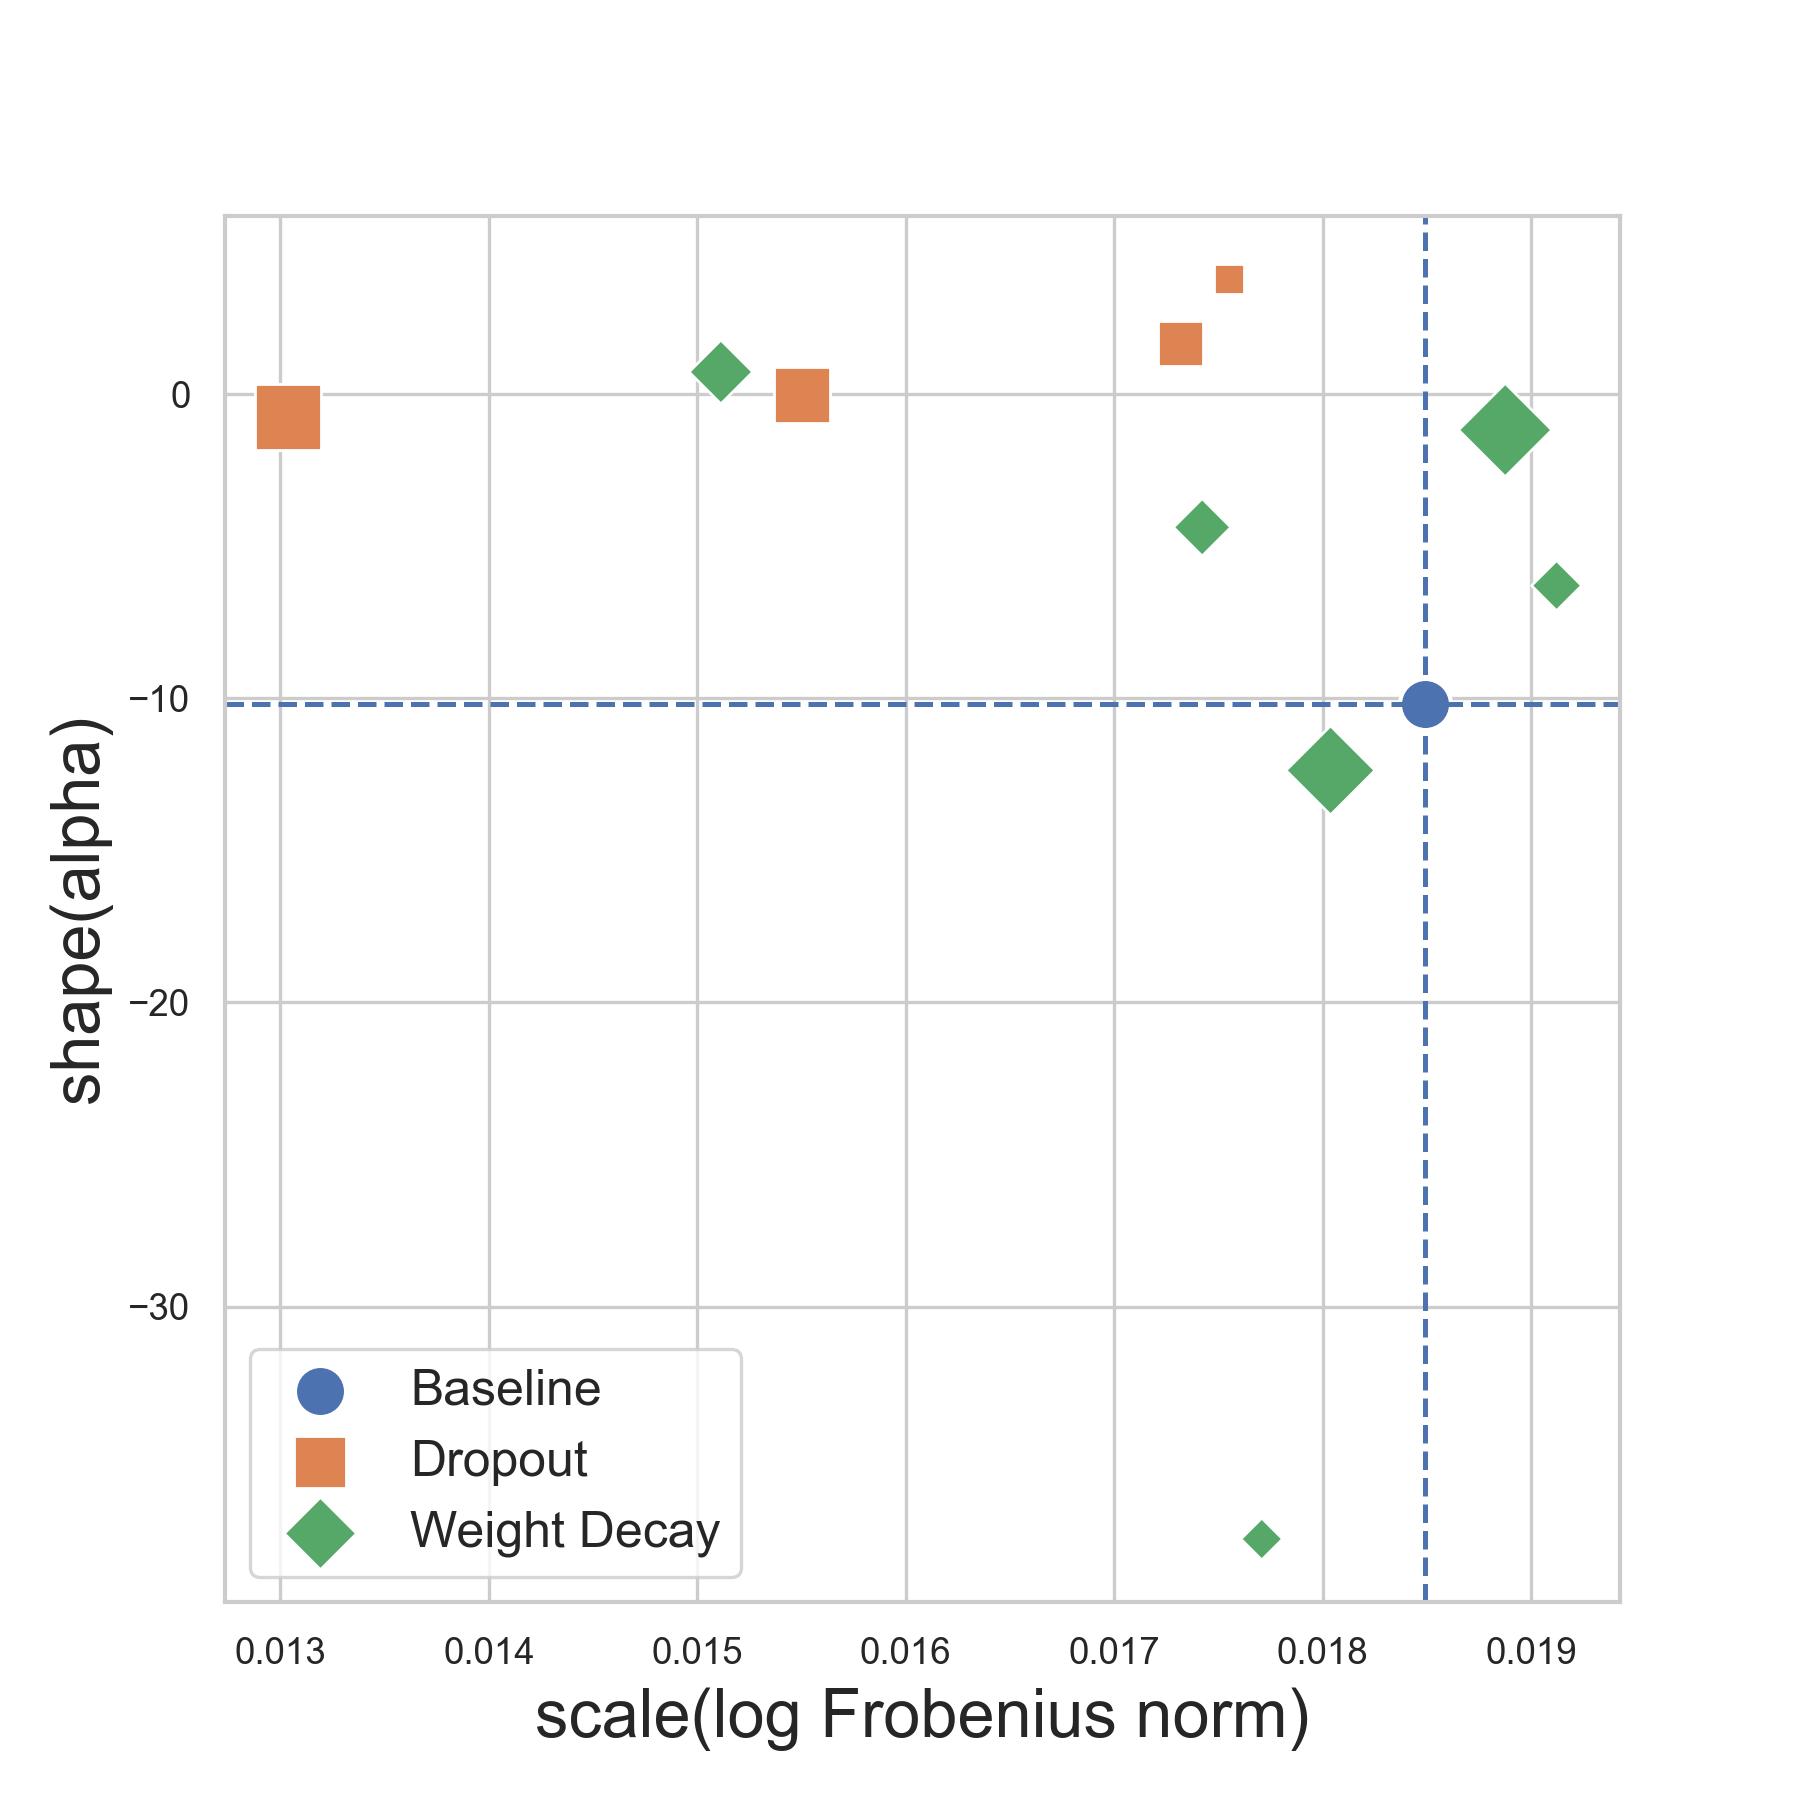}   % need to change 
        \caption{Frobenius norm vs. alpha on CIFAR-10}
        \label{fig:reg1}
    \end{subfigure}
    \hfill
    \begin{subfigure}[b]{0.3\textwidth}
        \centering
        \includegraphics[width=\textwidth]{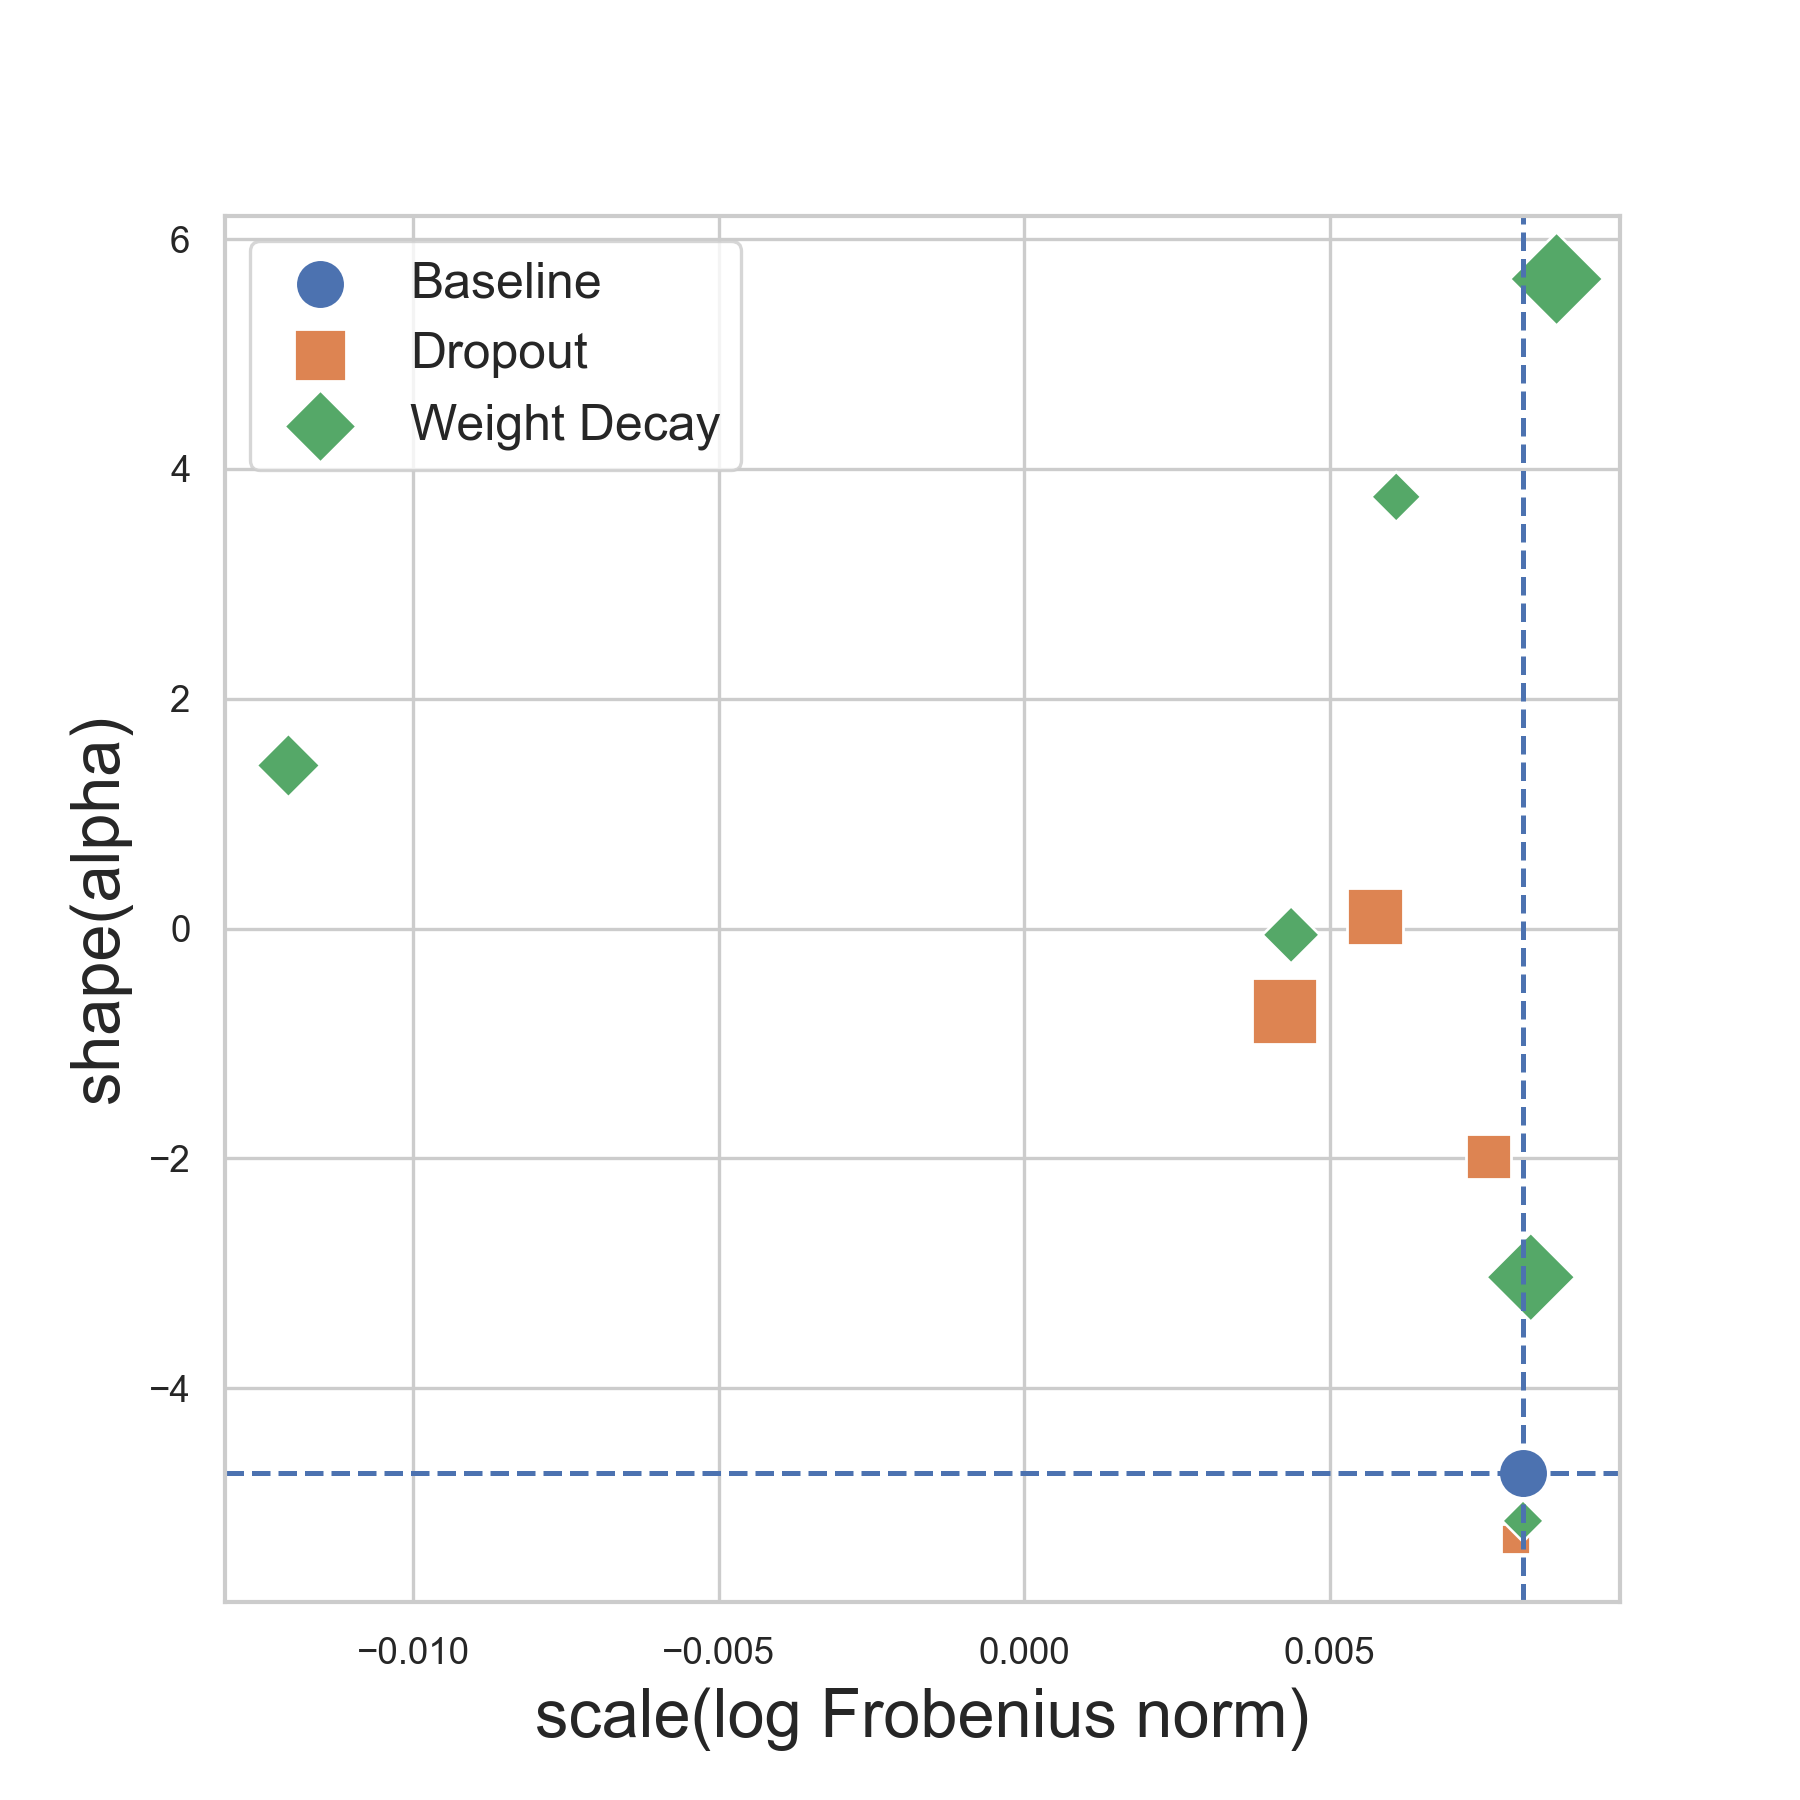}  % need to change 
        \caption{Frobenius norm vs. alpha on CIFAR-100}
        \label{fig:reg2}
    \end{subfigure}
    \hfill
    \begin{subfigure}[b]{0.3\textwidth}
        \centering
        \includegraphics[width=\textwidth]{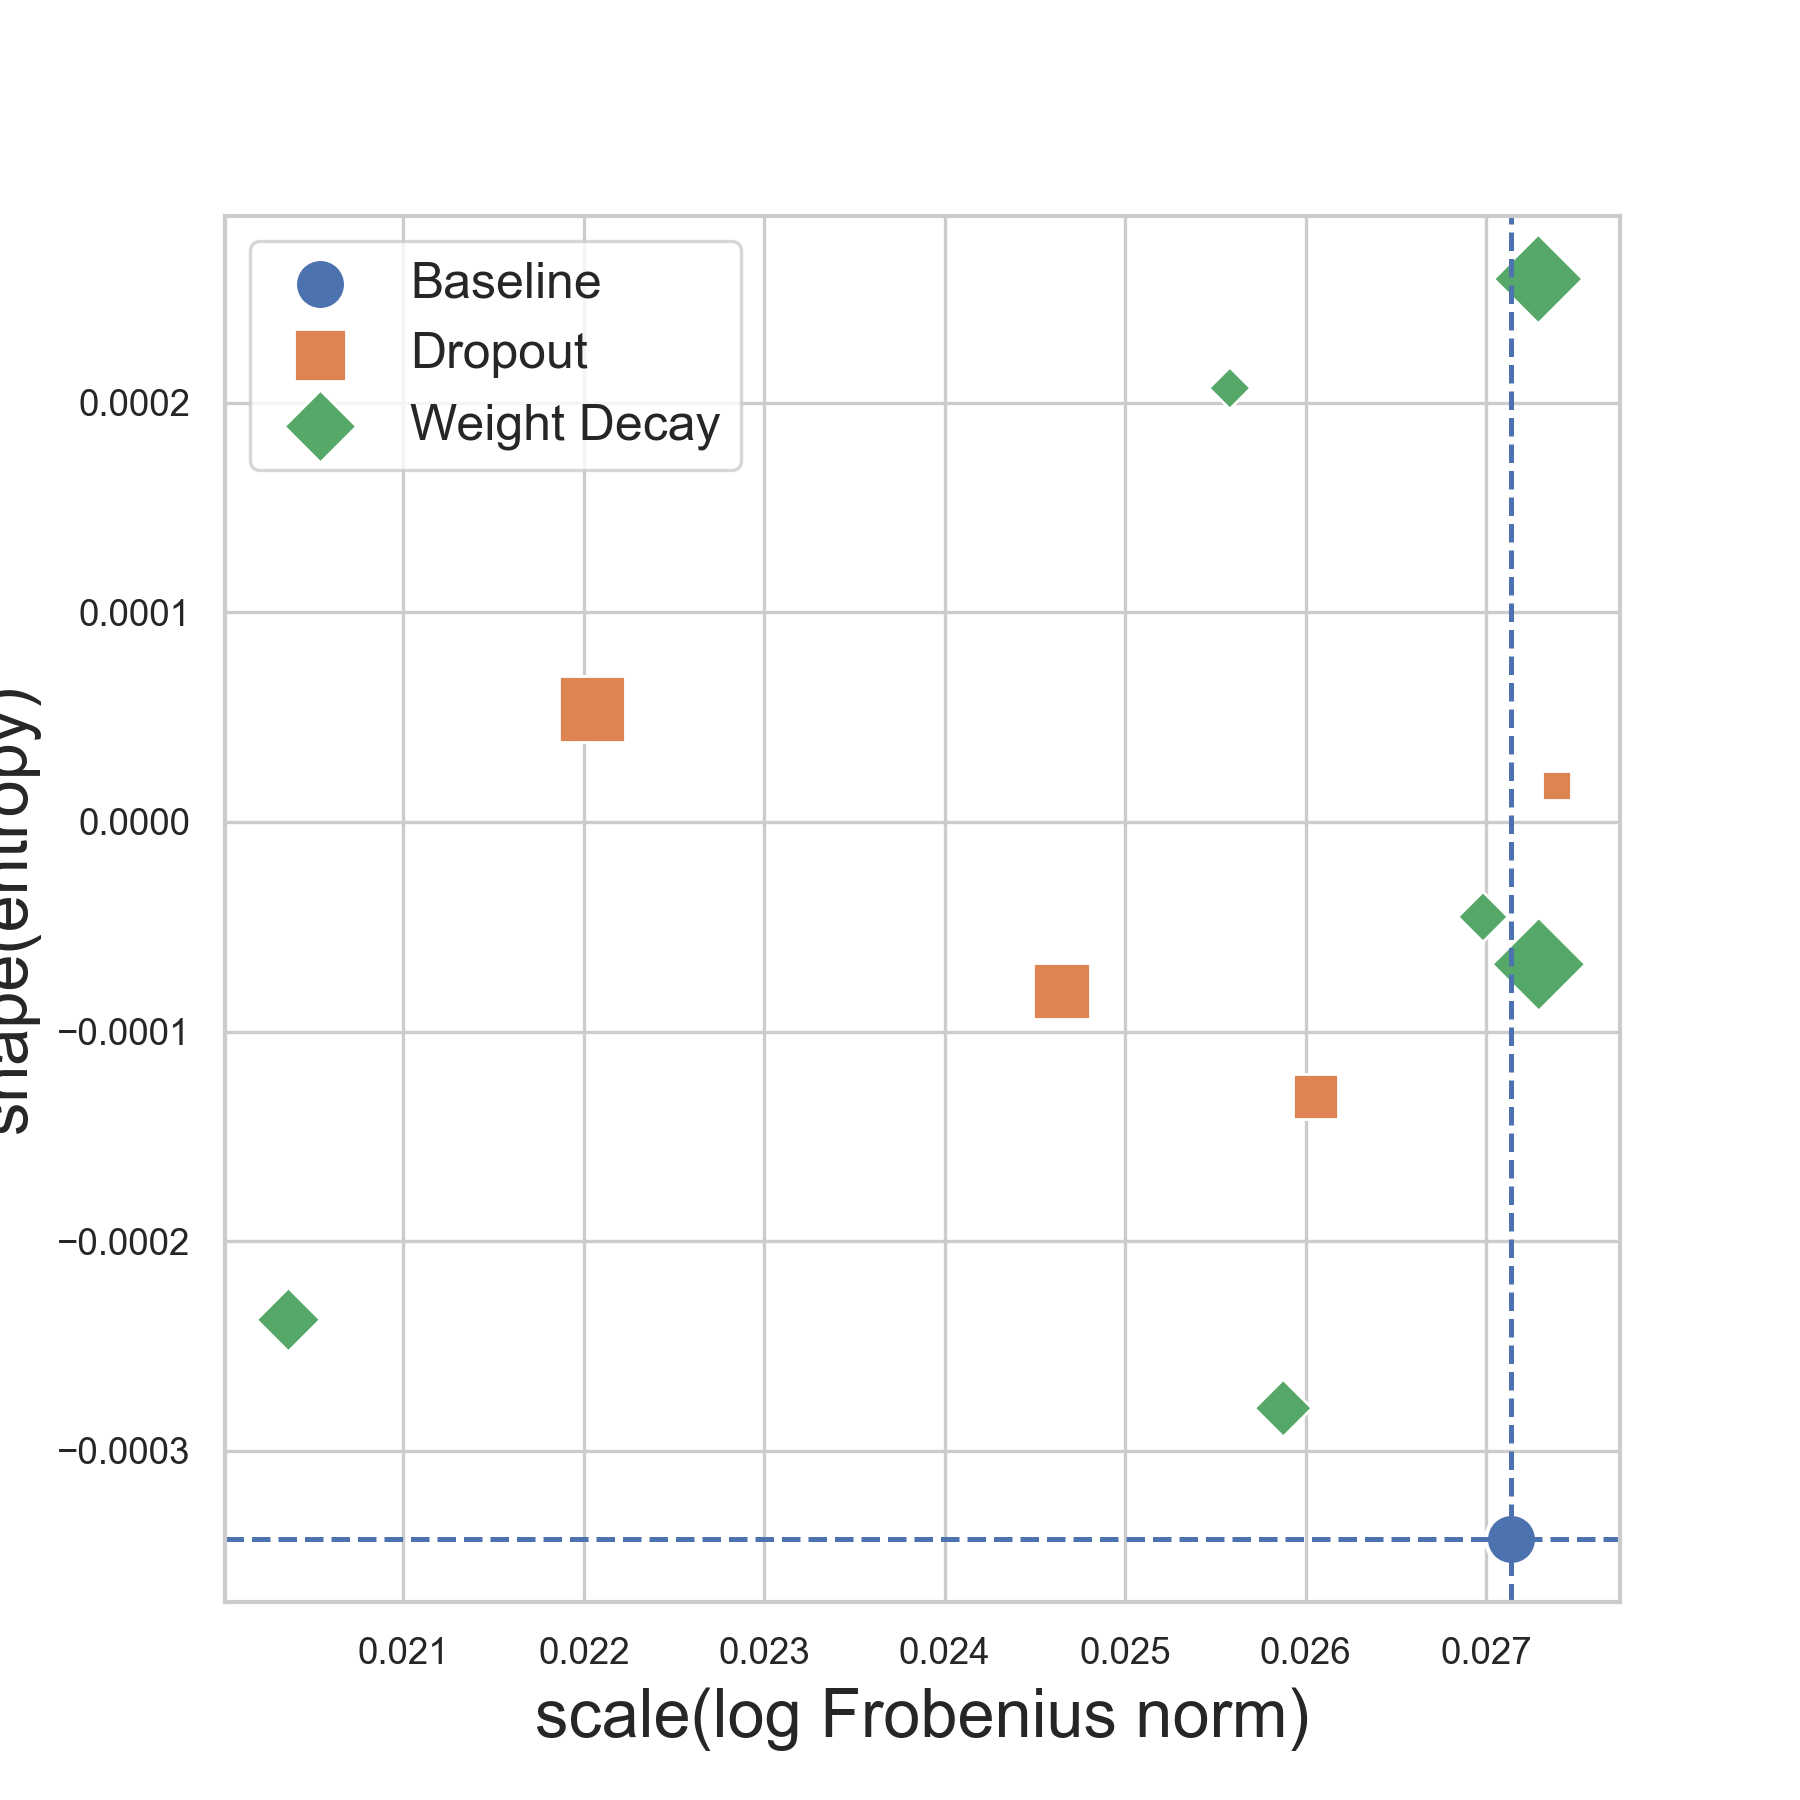}
        \caption{Frobenius norm vs. entropy on Imagenette}
        \label{fig:ref3}
    \end{subfigure}
    
    \vspace{1em} % Add some vertical space between rows
    
    % Second row
    \begin{subfigure}[b]{0.3\textwidth}
        \centering
        \includegraphics[width=\textwidth]{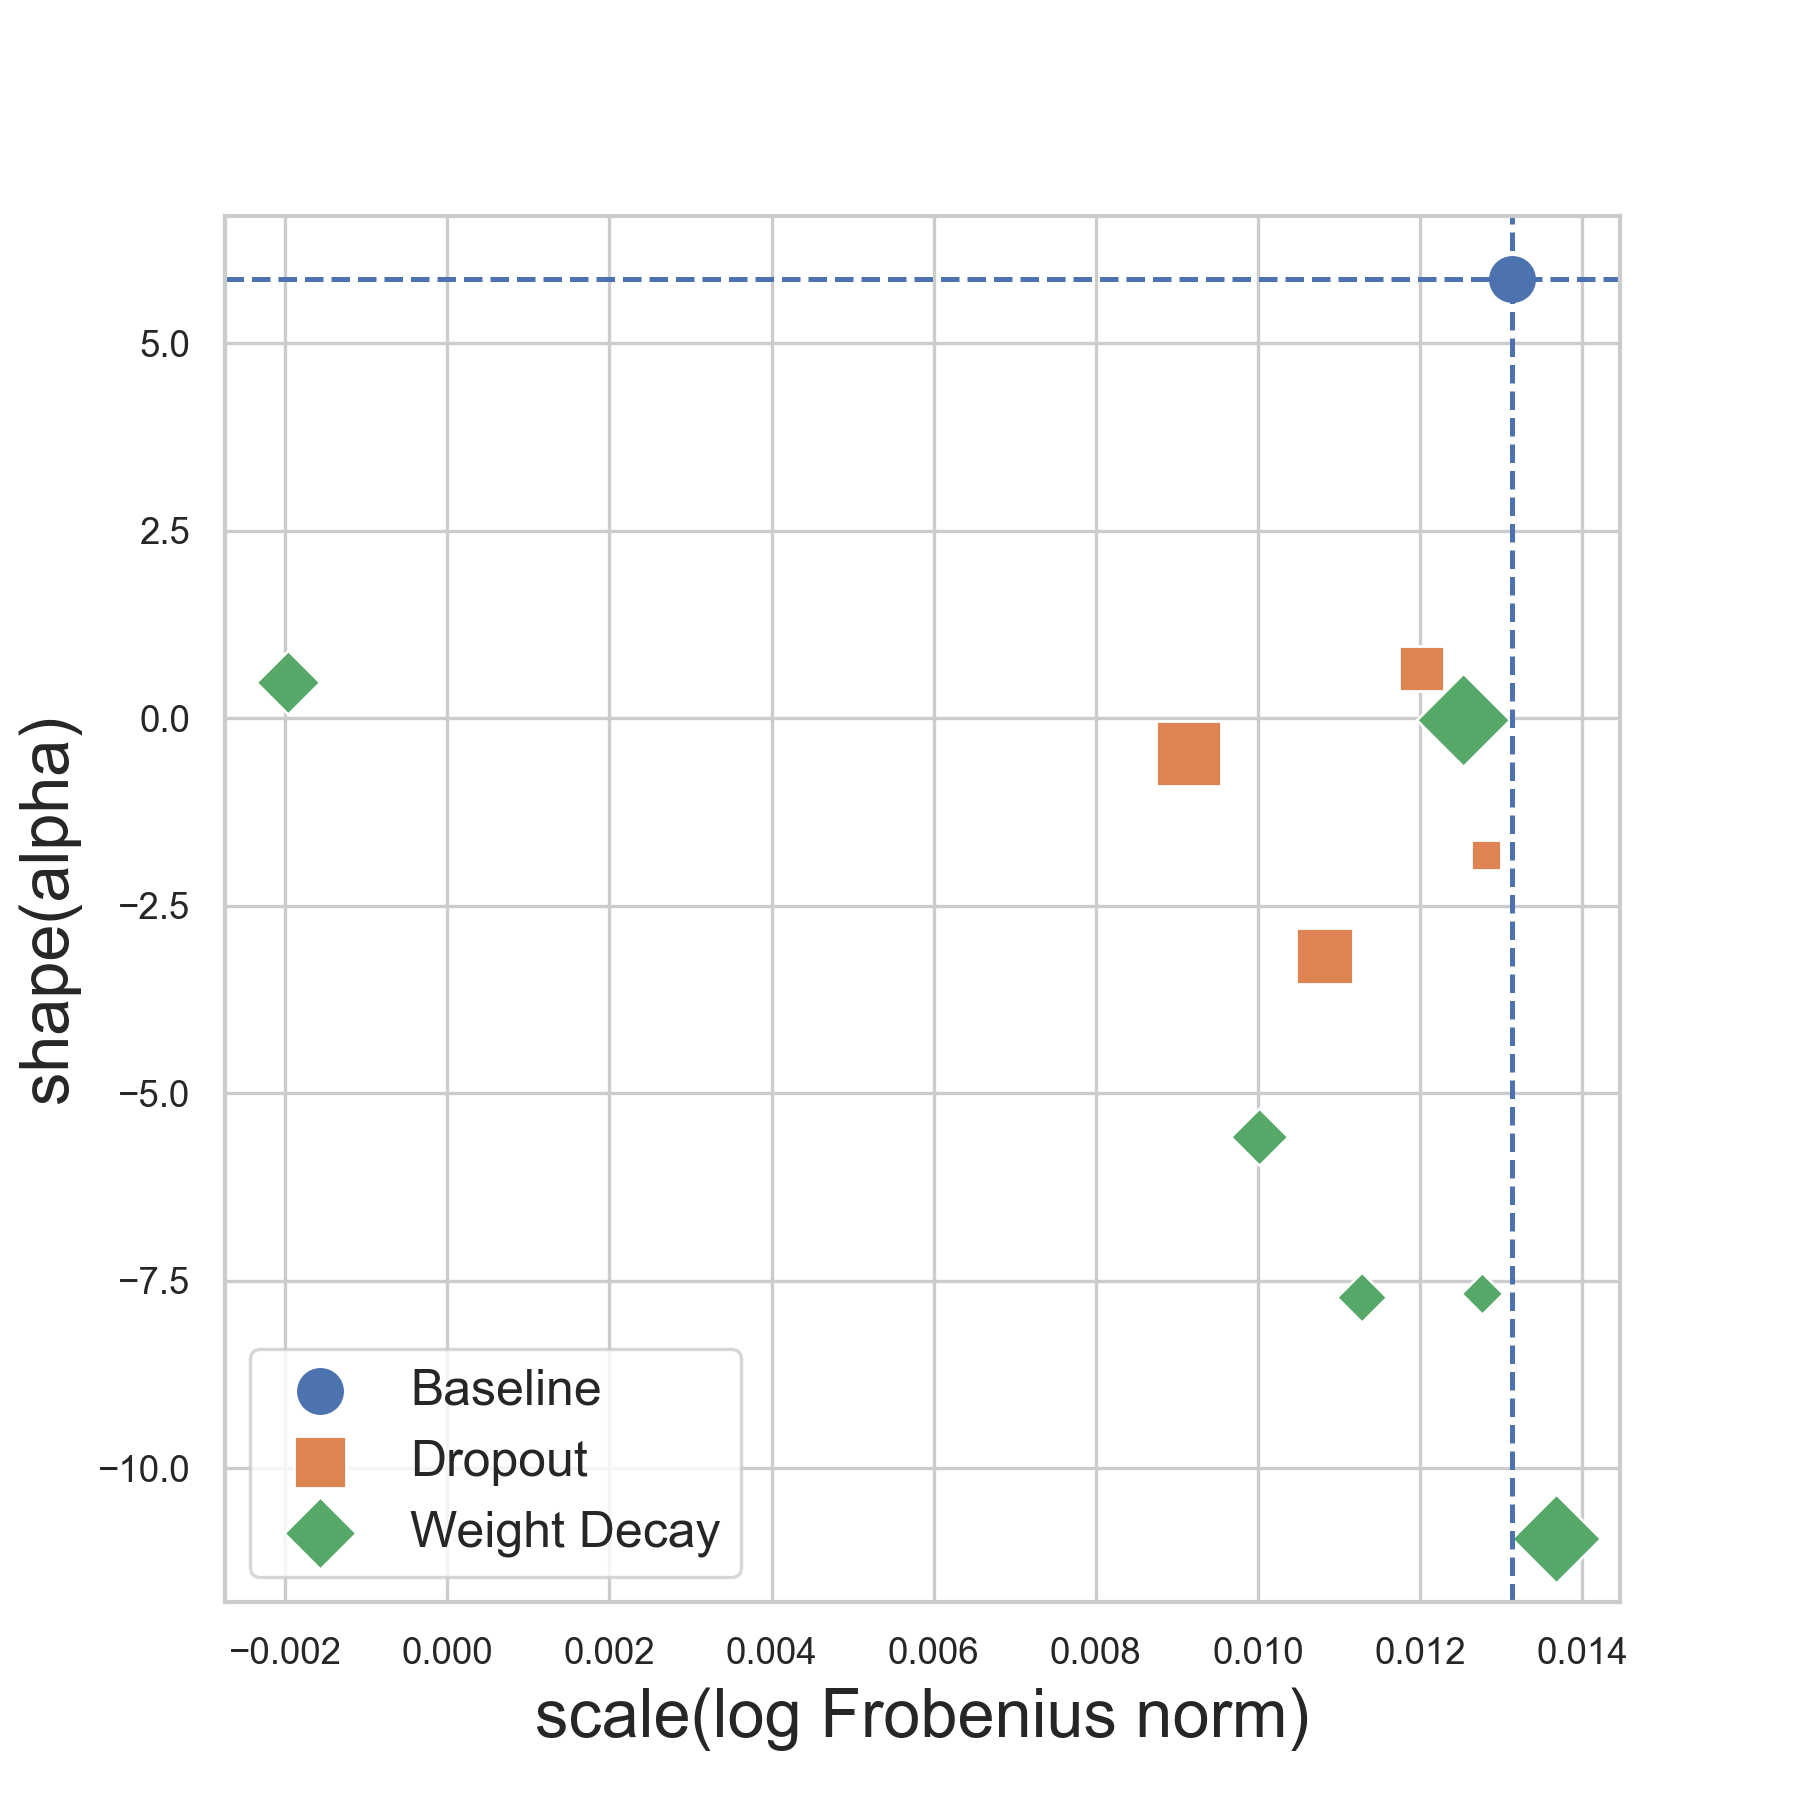}
        \caption{Frobenius norm vs. alpha on Flowers102}
        \label{fig:reg4}
    \end{subfigure}
    \hfill
    \begin{subfigure}[b]{0.3\textwidth}
        \centering
        \includegraphics[width=\textwidth]{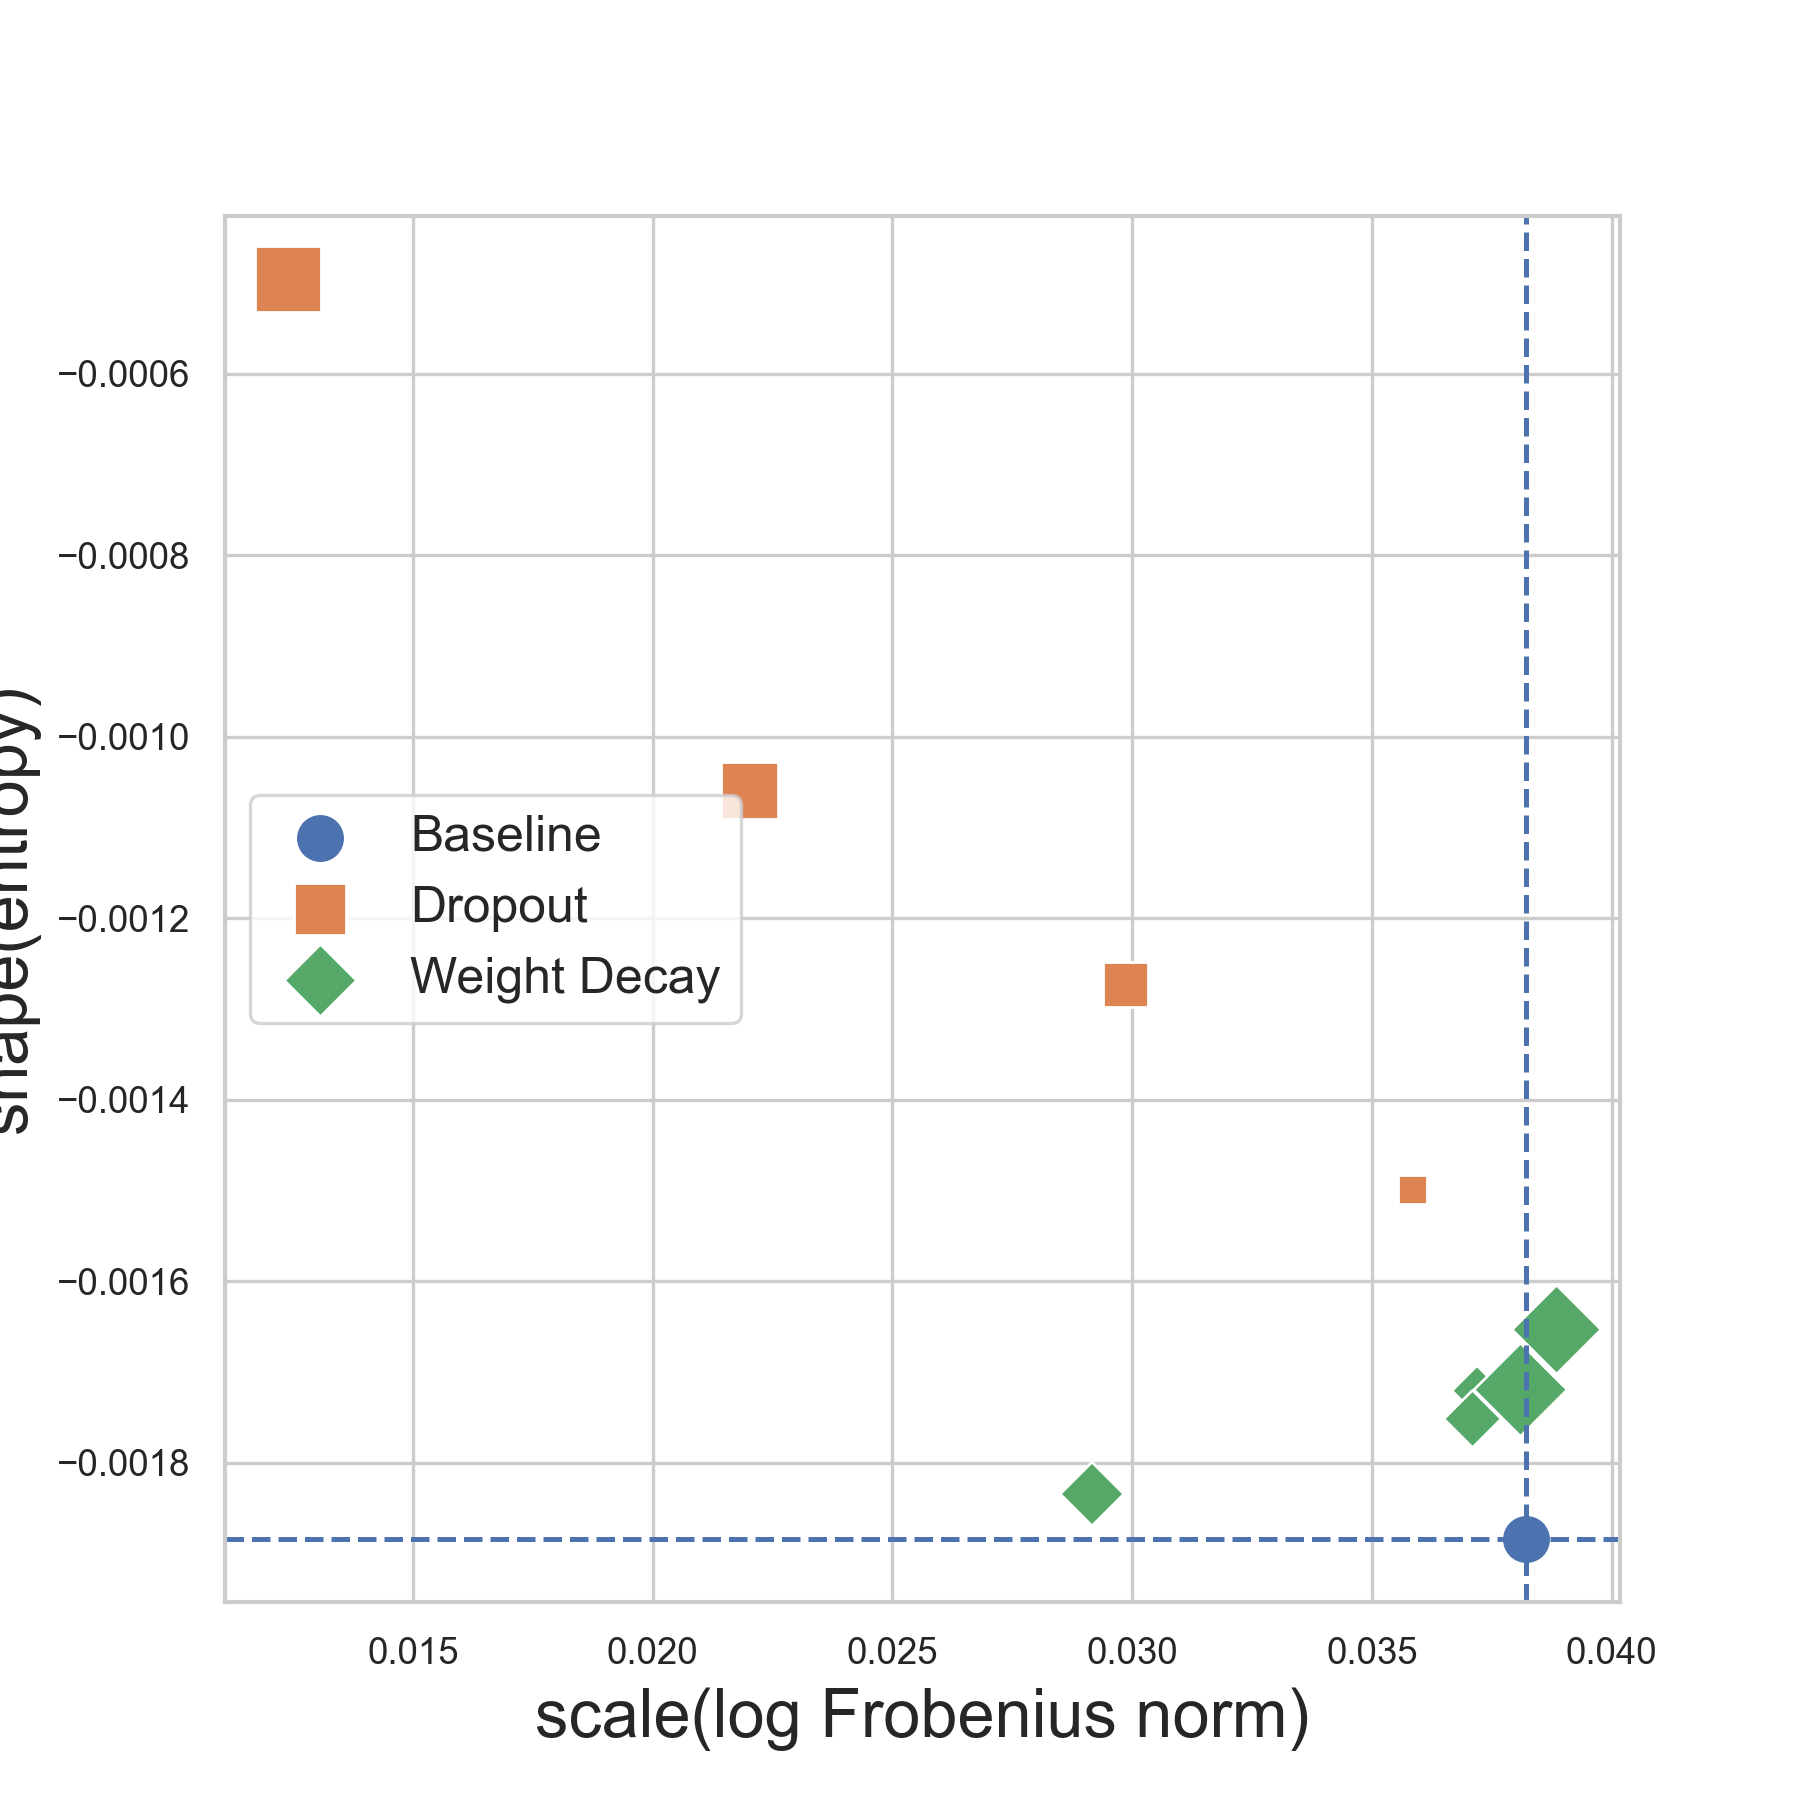}
        \caption{Frobenius norm vs. entropy on Stanford Cars}
        \label{fig:reg5}
    \end{subfigure}
    \hfill
    \begin{subfigure}[b]{0.3\textwidth}
        \centering
        \includegraphics[width=\textwidth]{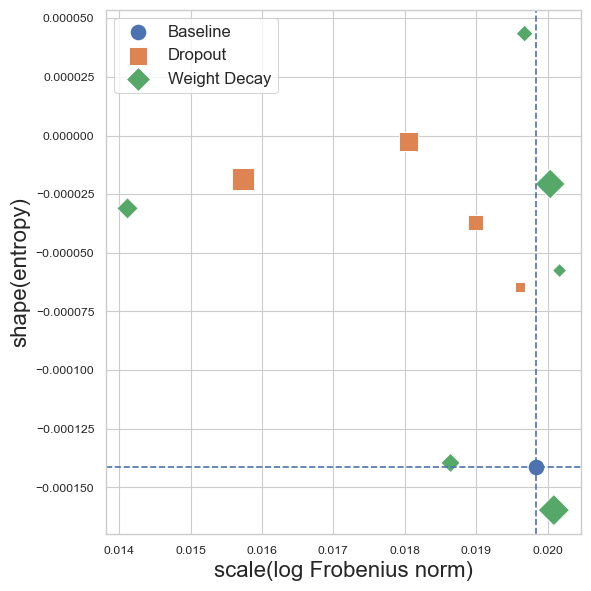}
        \caption{Frobenius norm vs. entropy on DomaineNet (Real)}
        \label{fig:reg_reg5}
    \end{subfigure}
    
    \caption{\textcolor{blue}{Scale-shape plots of ESDs of the classifier layers on CIFAR-10/100, Imagenette, Flower102, StandfordCars, DomainNet(Real). The results are marked with square and diamond shapes for dropout and weight decay regularization techniques, respectively. The size of markers represents the magnitude of the dropout rate and weight decay values. The results above are based on the ResNet50 backbone. Because of limitations of computing resources, CIFAR-10/100 and DomainNet(Real) refer to a subset that samples 5000 images for fine-tuning.}}
    \label{fig:regularization-cl_RN}
\end{figure}

\begin{figure}[h]
    \centering
    % First row
    \begin{subfigure}[b]{0.3\textwidth}
        \centering
        \includegraphics[width=\textwidth]{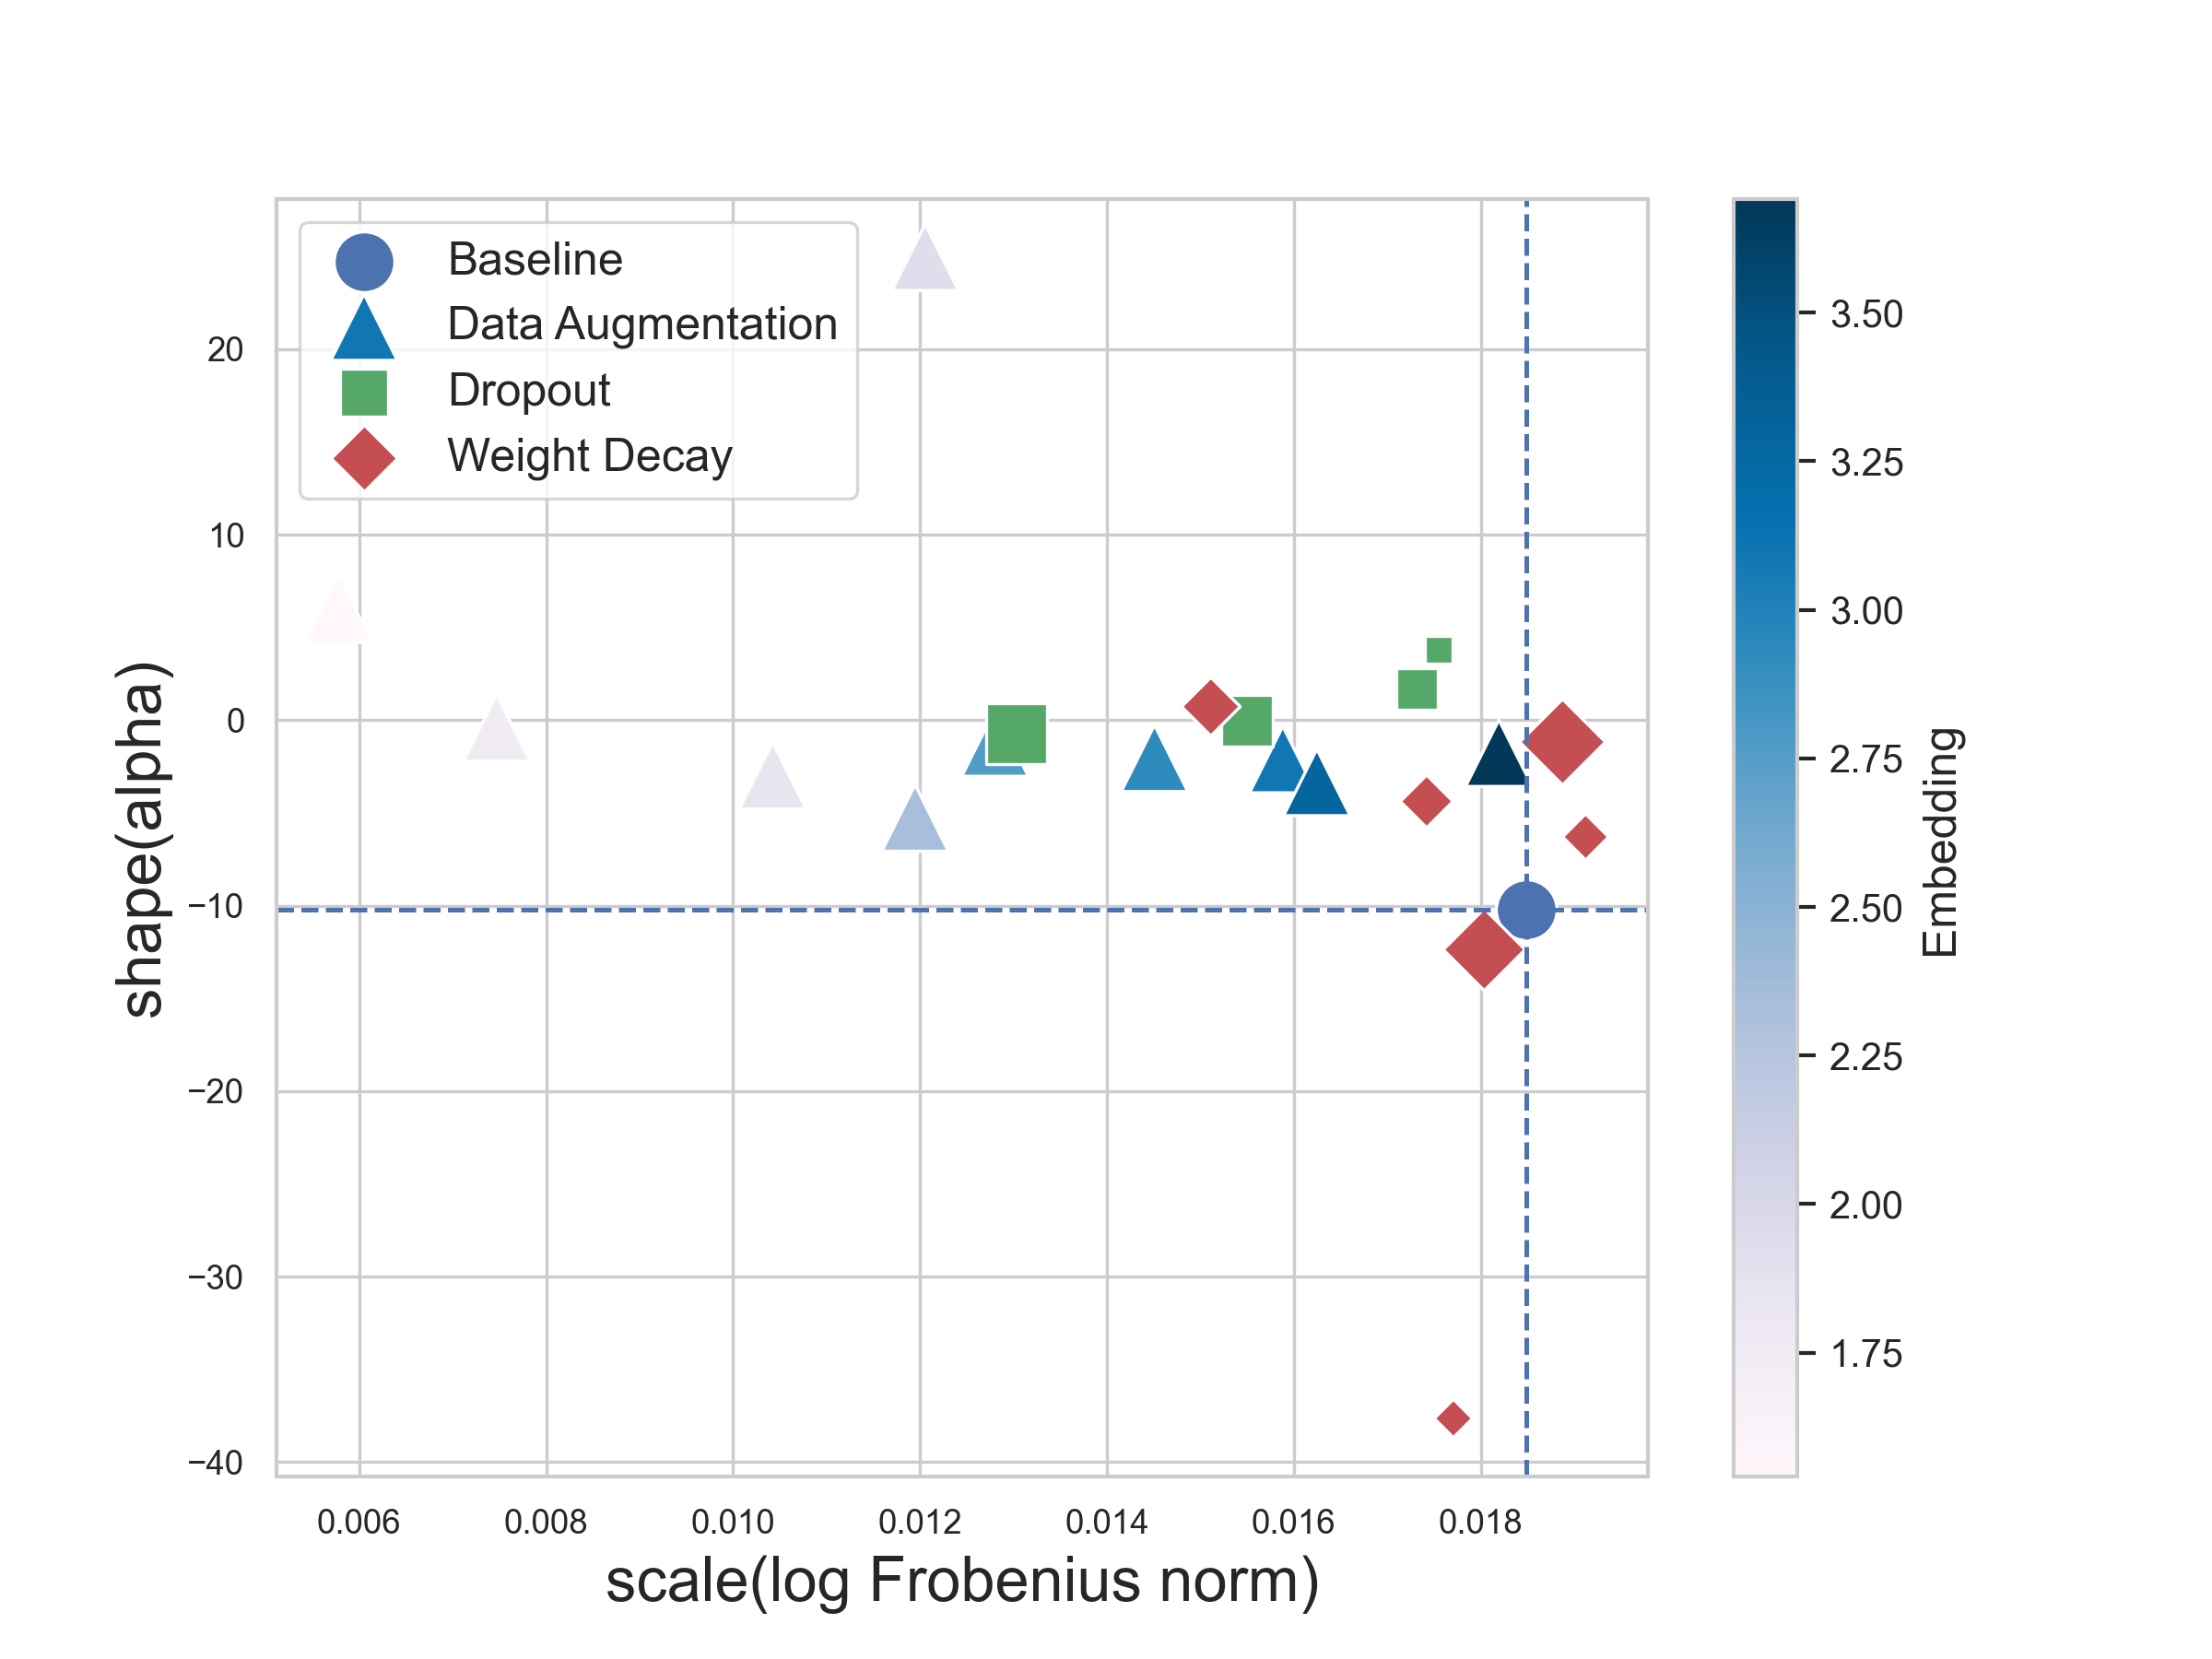}  % need to change 
        \caption{Frobenius norm vs. entropy on CIFAR-10}
        \label{fig:d-1}
    \end{subfigure}
    \hfill
    \begin{subfigure}[b]{0.3\textwidth}
        \centering
        \includegraphics[width=\textwidth]{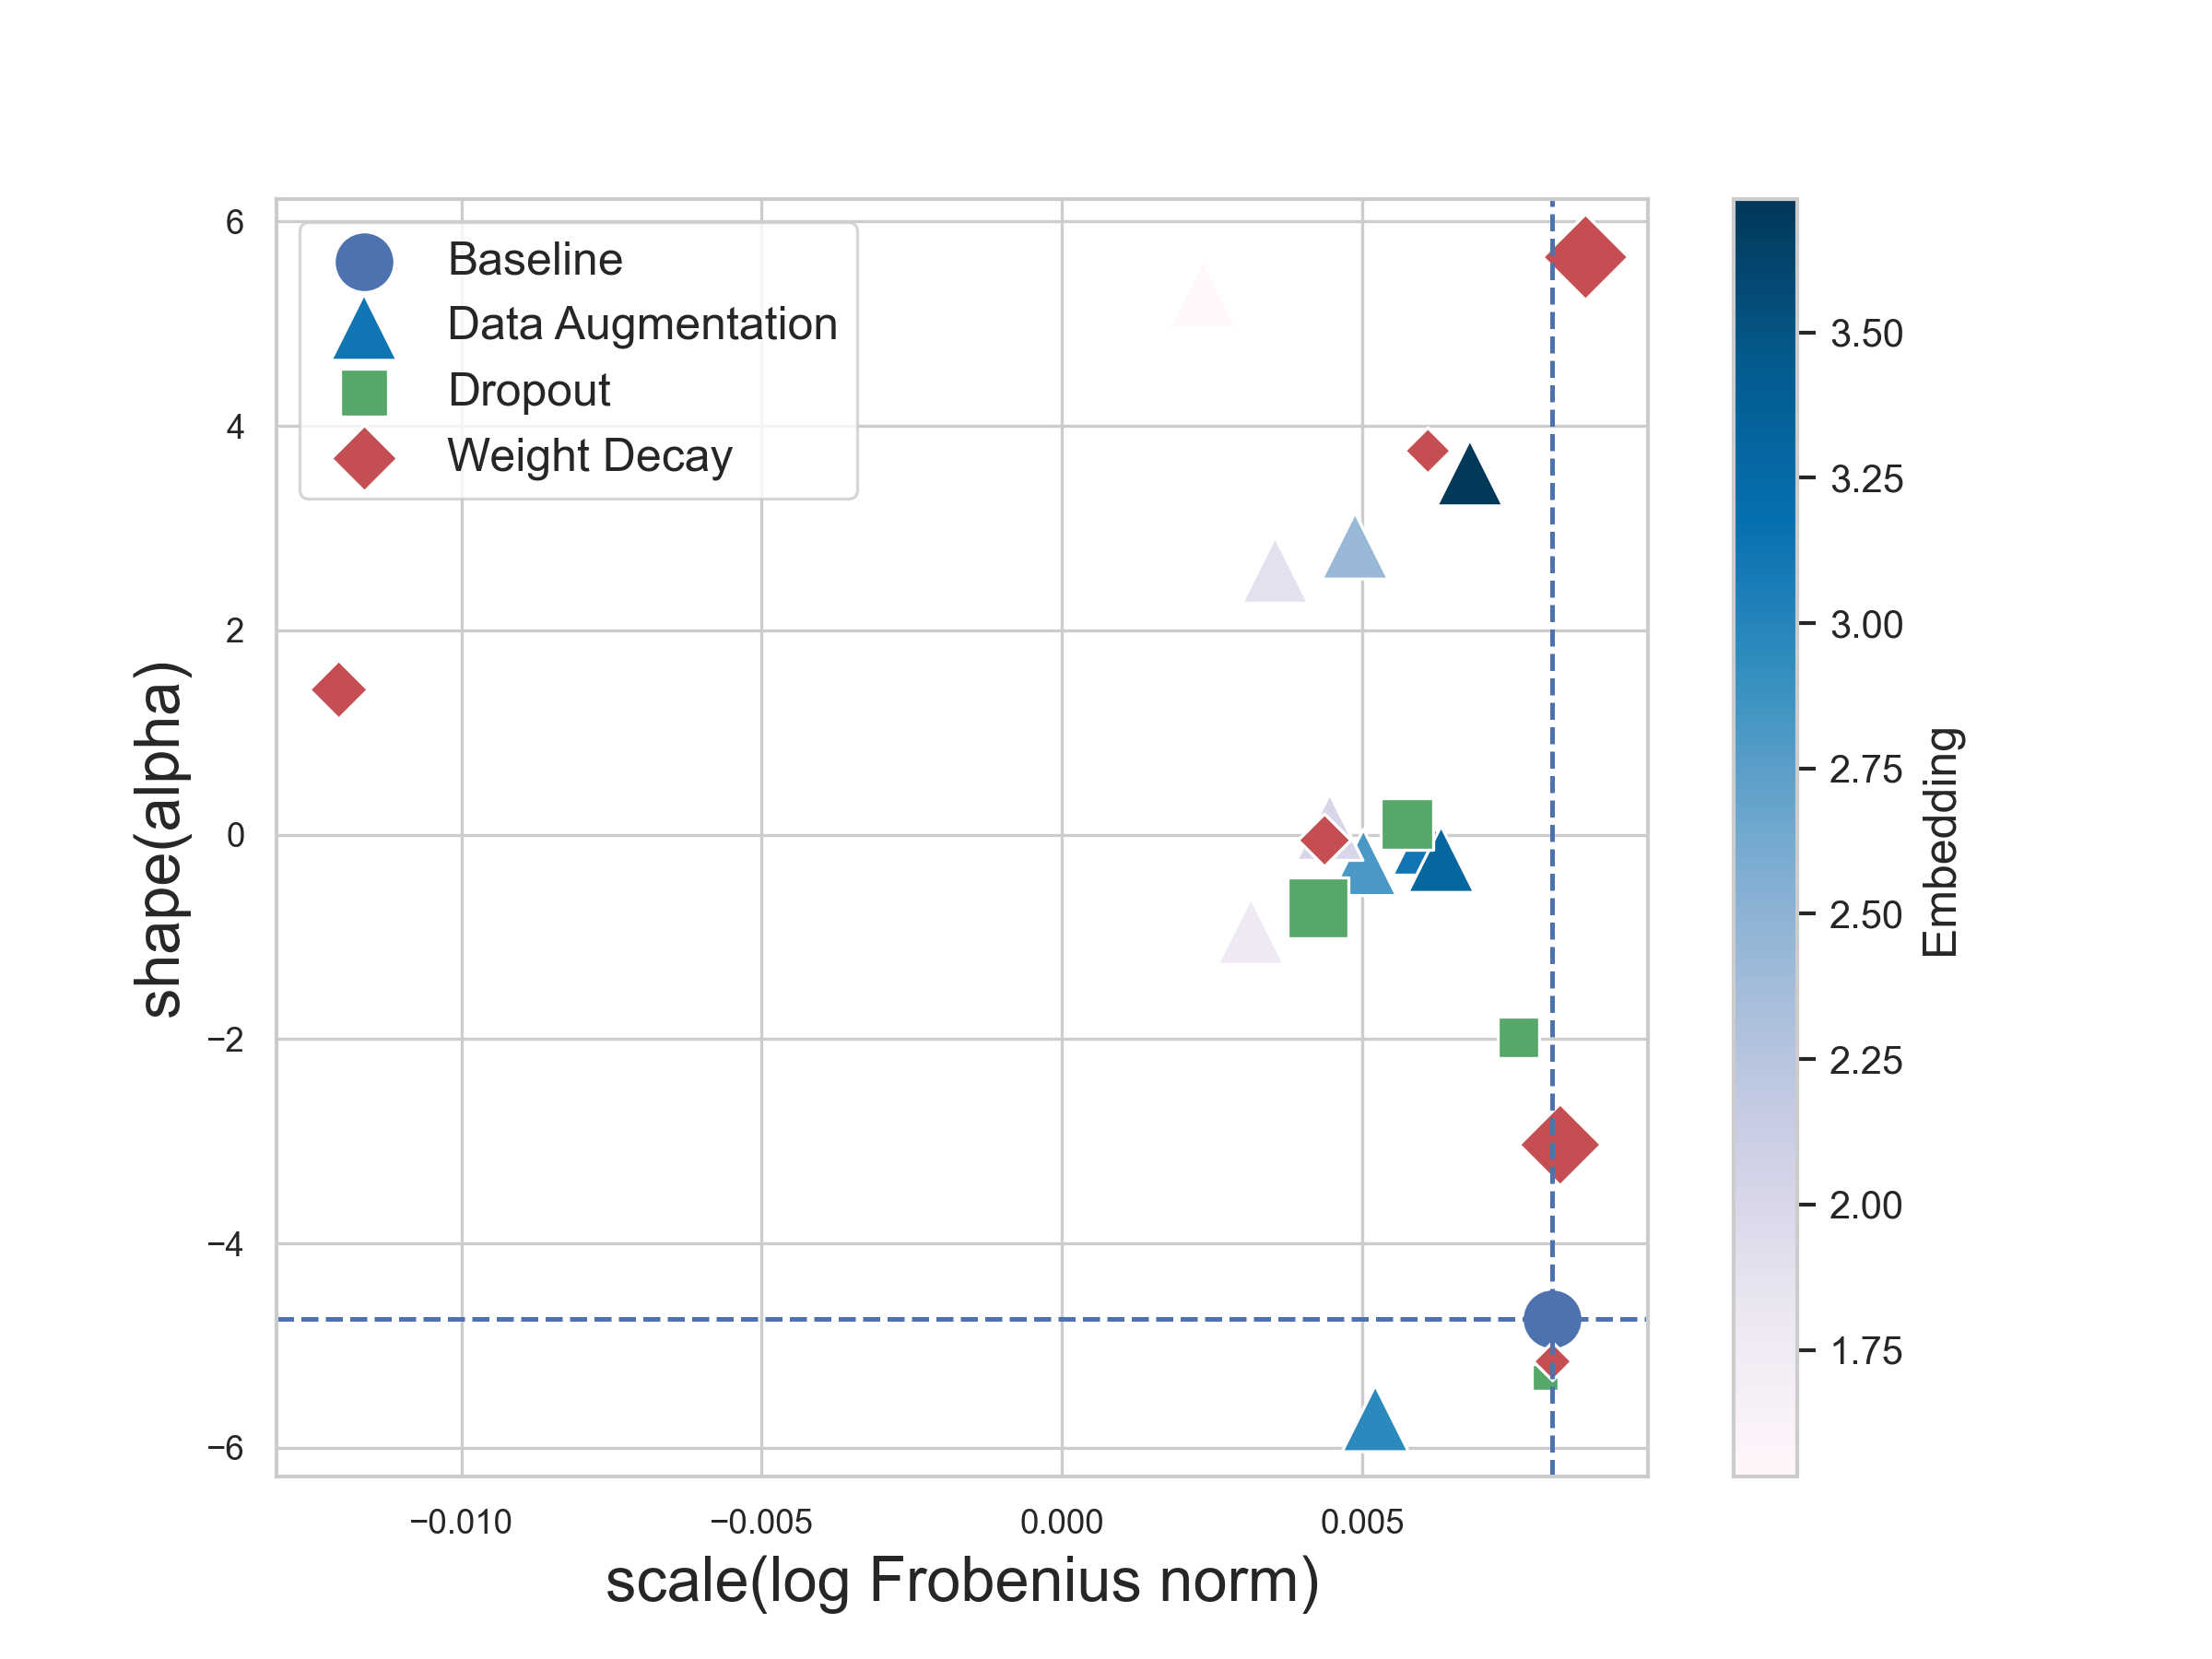}   % need to change 
        \caption{Frobenius norm vs. entropy on CIFAR-100}
        \label{fig:d-2}
    \end{subfigure}
    \hfill
    \begin{subfigure}[b]{0.3\textwidth}
        \centering
        \includegraphics[width=\textwidth]{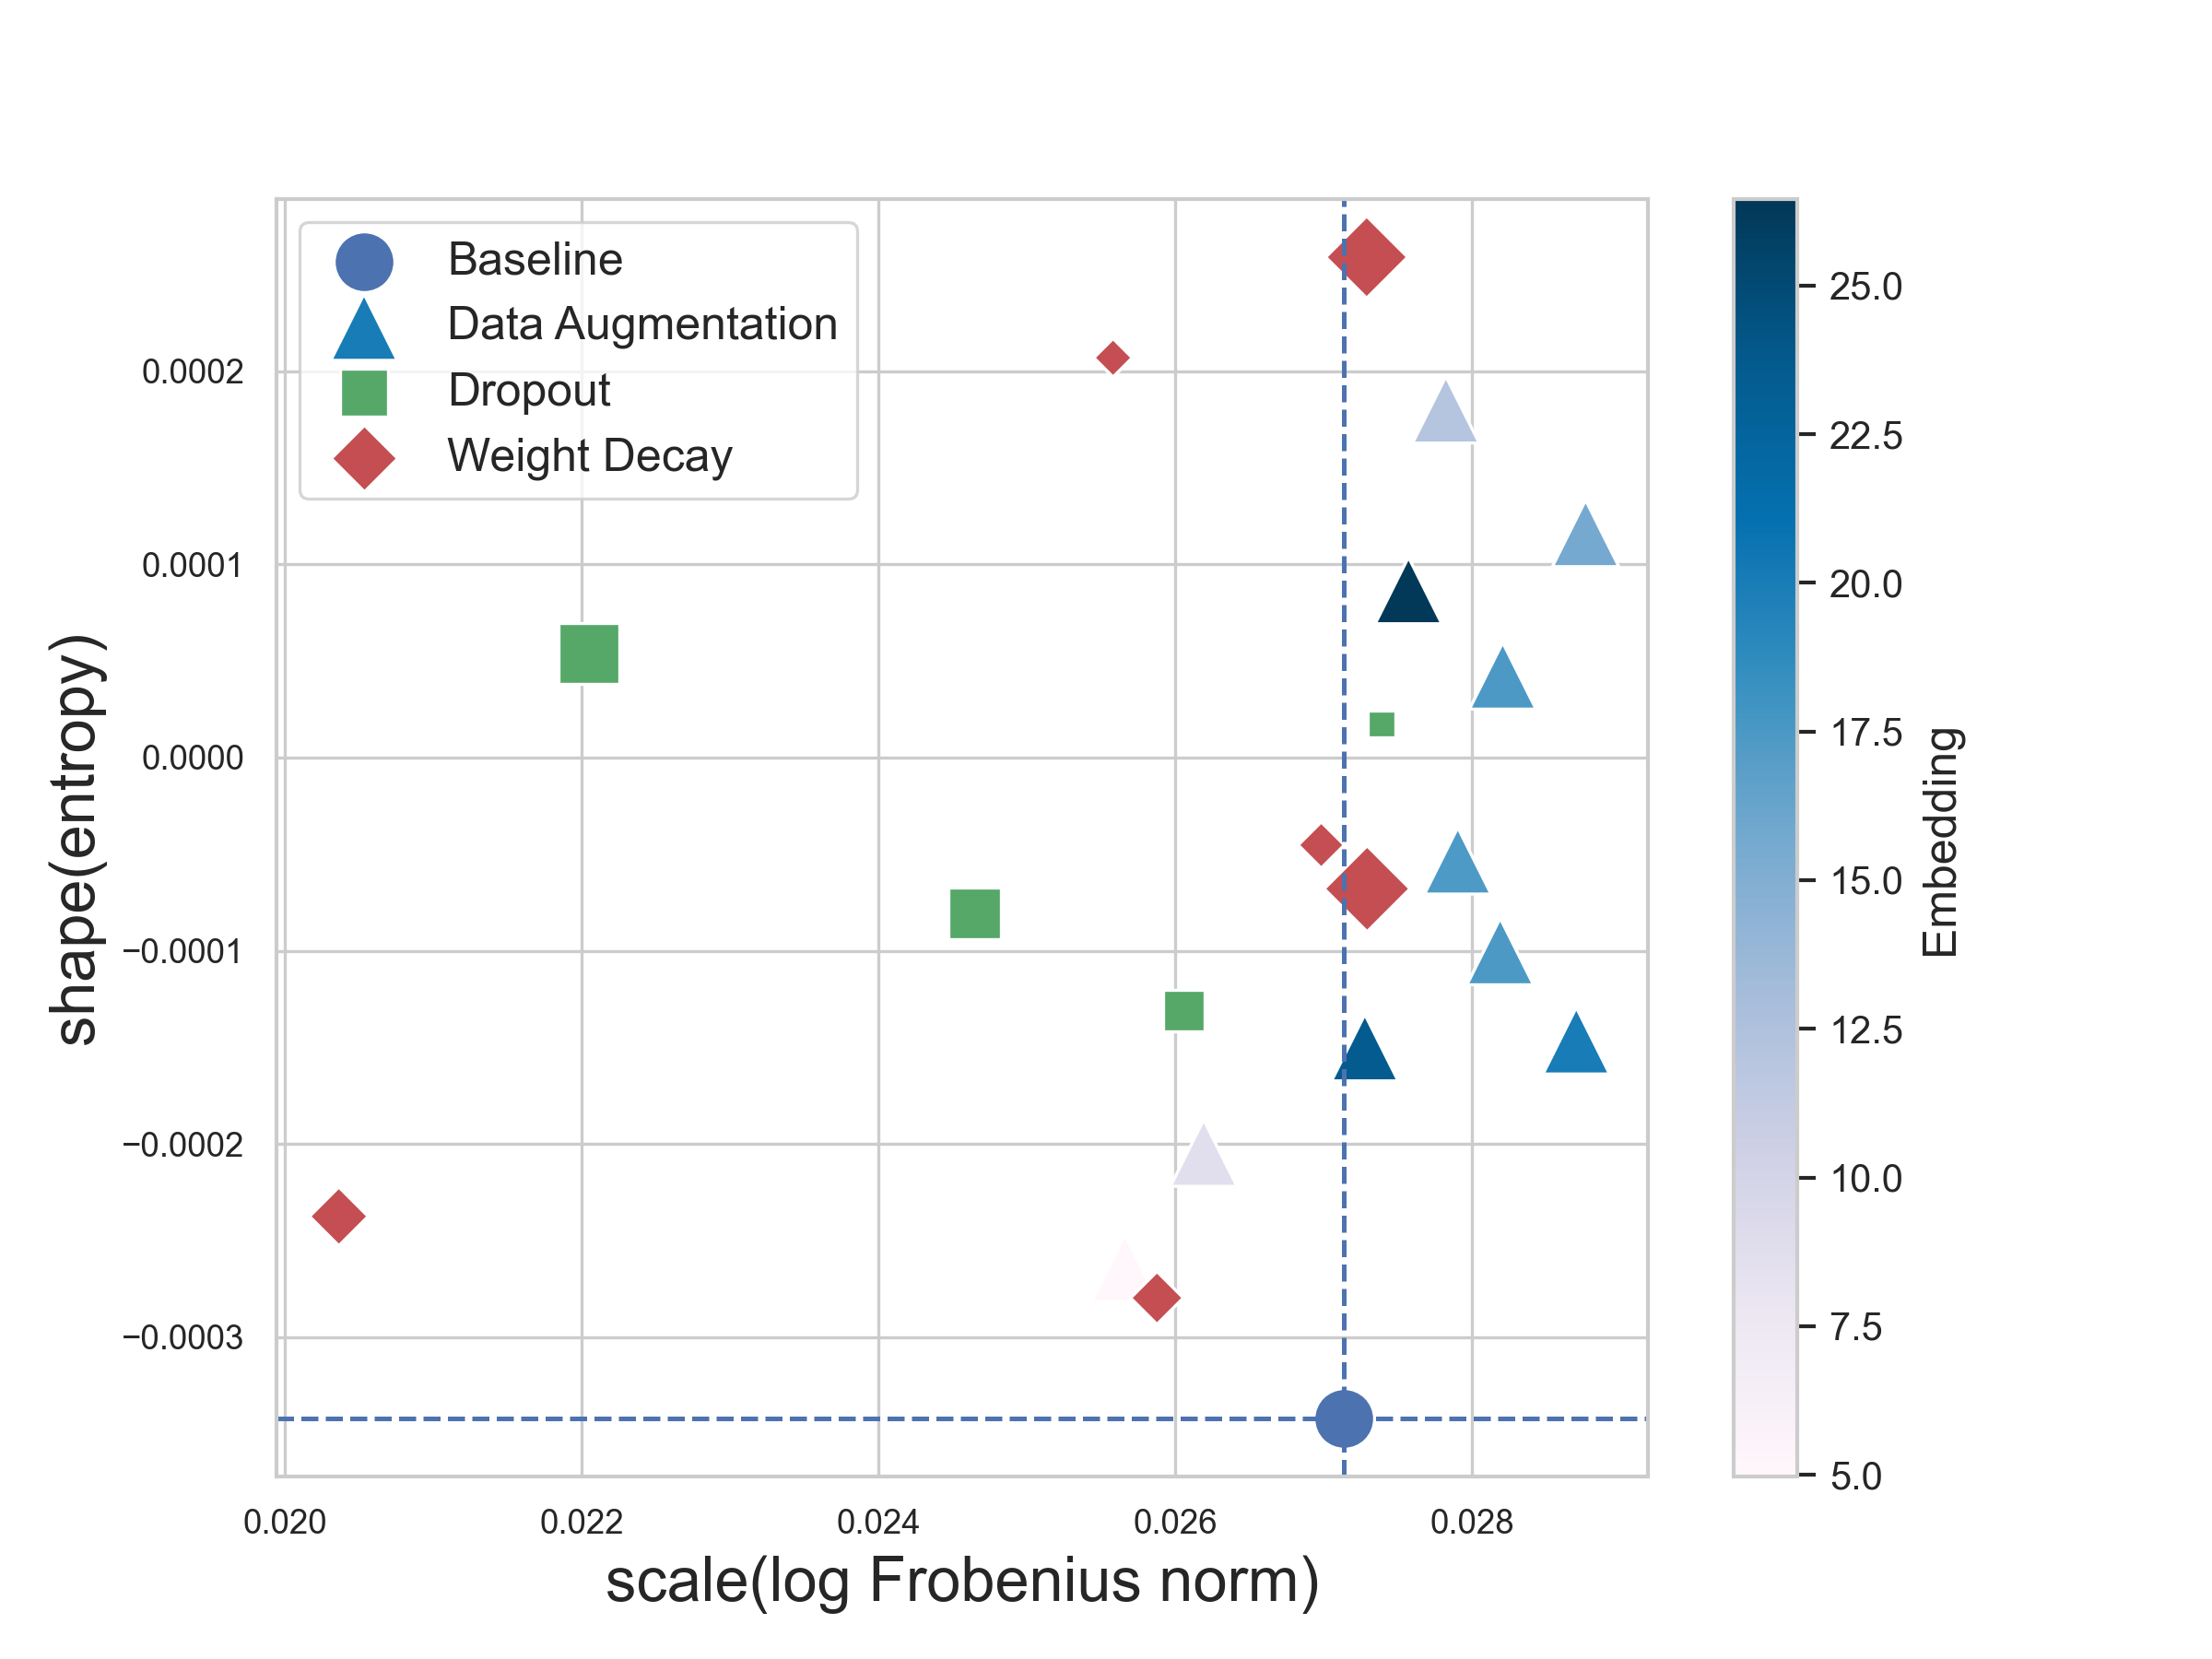}
        \caption{Frobenius norm vs. entropy on Imagenette}
        \label{fig:d-3}
    \end{subfigure}
    
    \vspace{1em} % Add some vertical space between rows
    
    % Second row
    \begin{subfigure}[b]{0.3\textwidth}
        \centering
        \includegraphics[width=\textwidth]{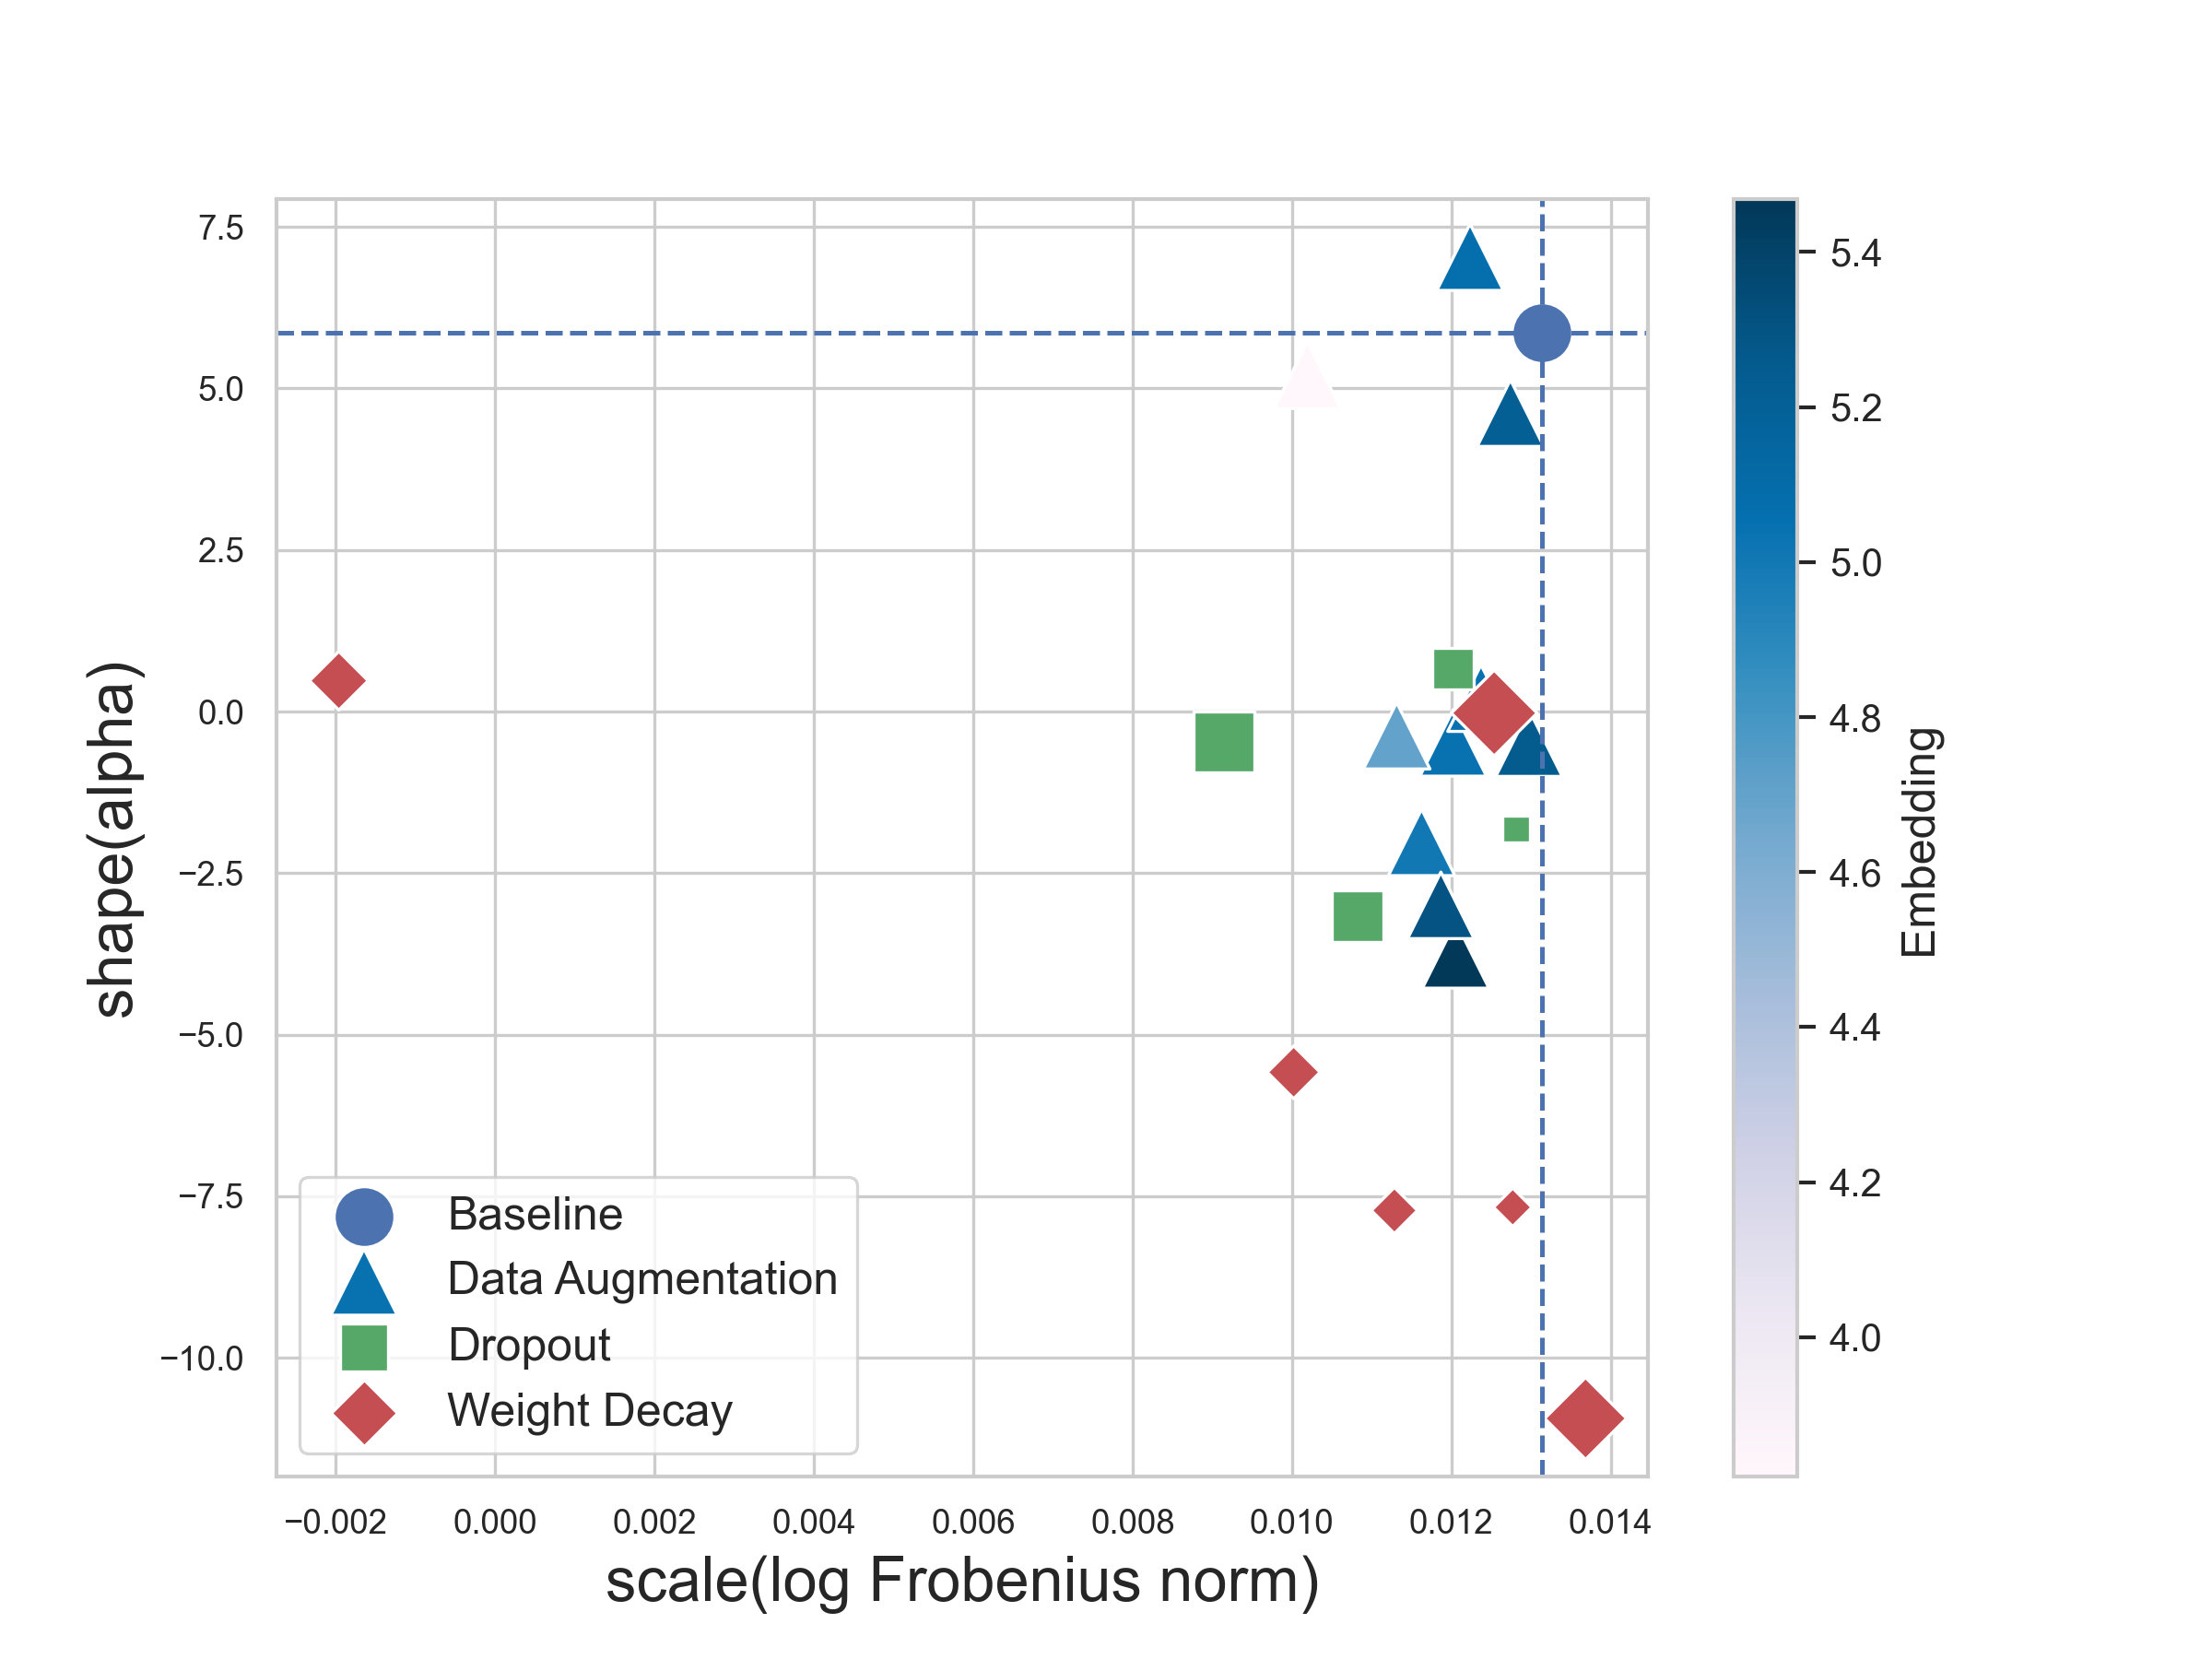}
        \caption{Frobenius norm vs. alpha on Flowers102}
        \label{fig:d-4}
    \end{subfigure}
    \hfill
    \begin{subfigure}[b]{0.3\textwidth}
        \centering
        \includegraphics[width=\textwidth]{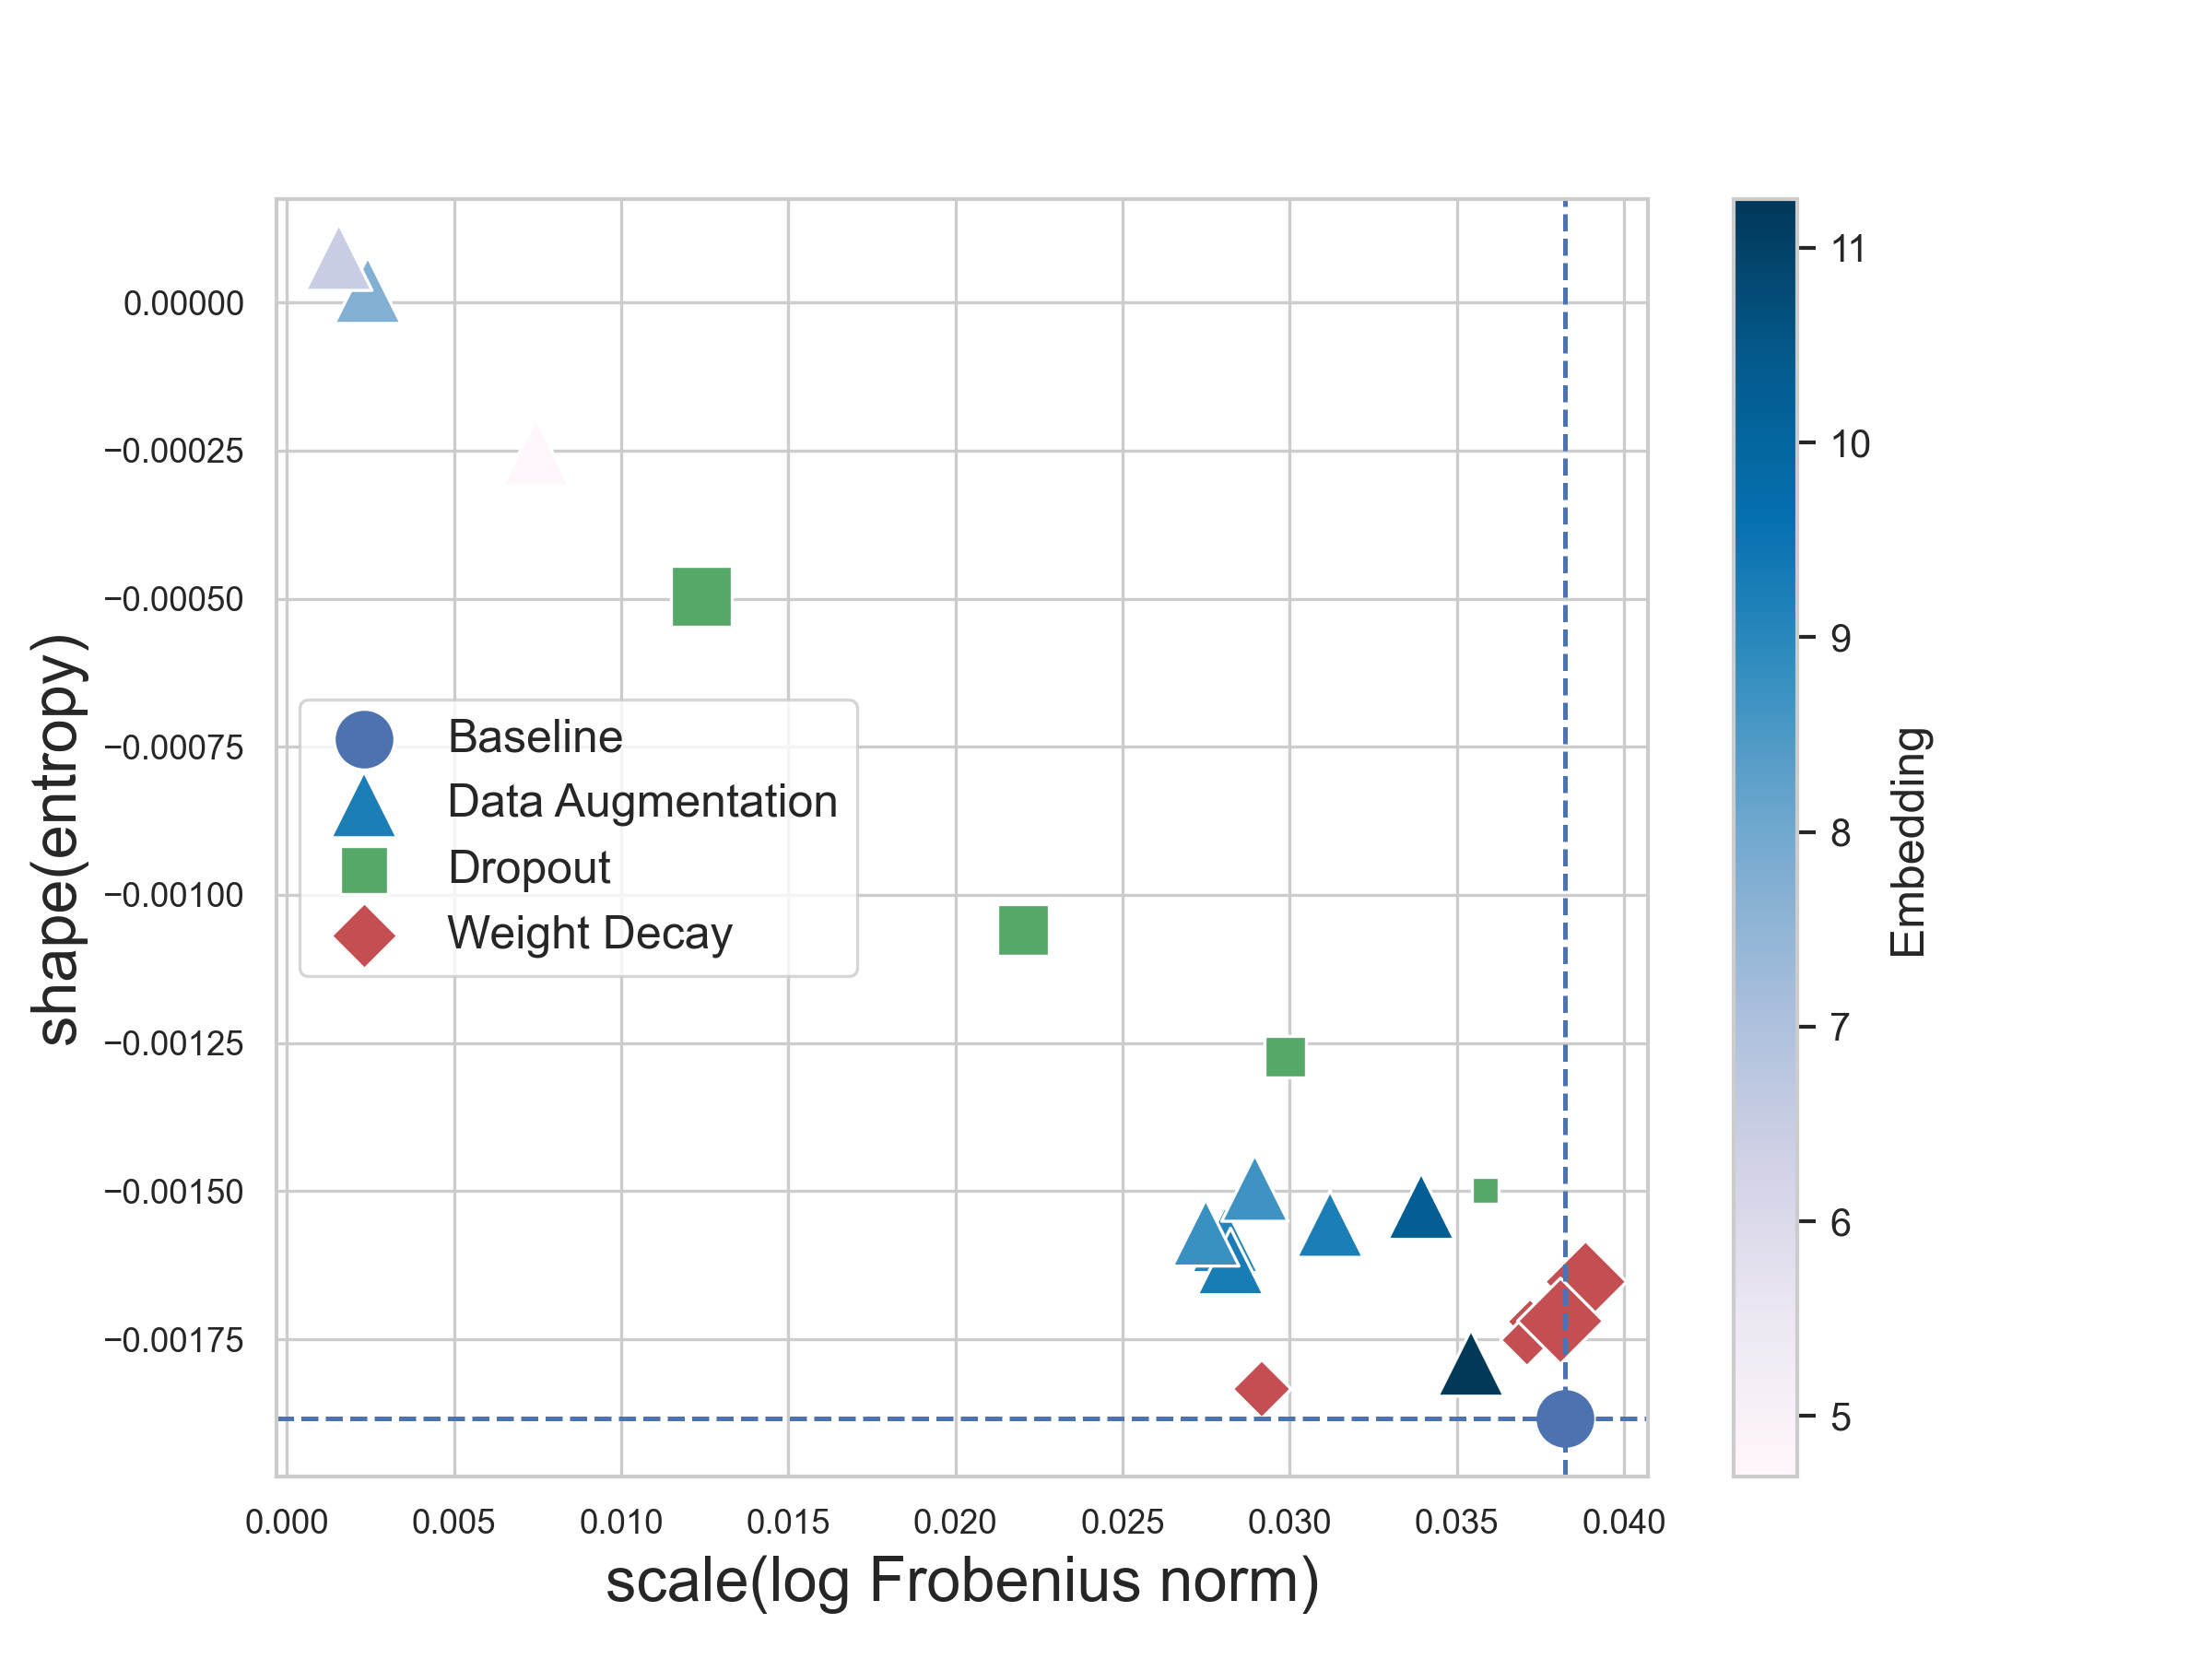}
        \caption{Frobenius norm vs. entropy on Stanford Cars}
        \label{fig:d-5}
    \end{subfigure}
    \hfill
    \begin{subfigure}[b]{0.3\textwidth}
        \centering
        \includegraphics[width=\textwidth]{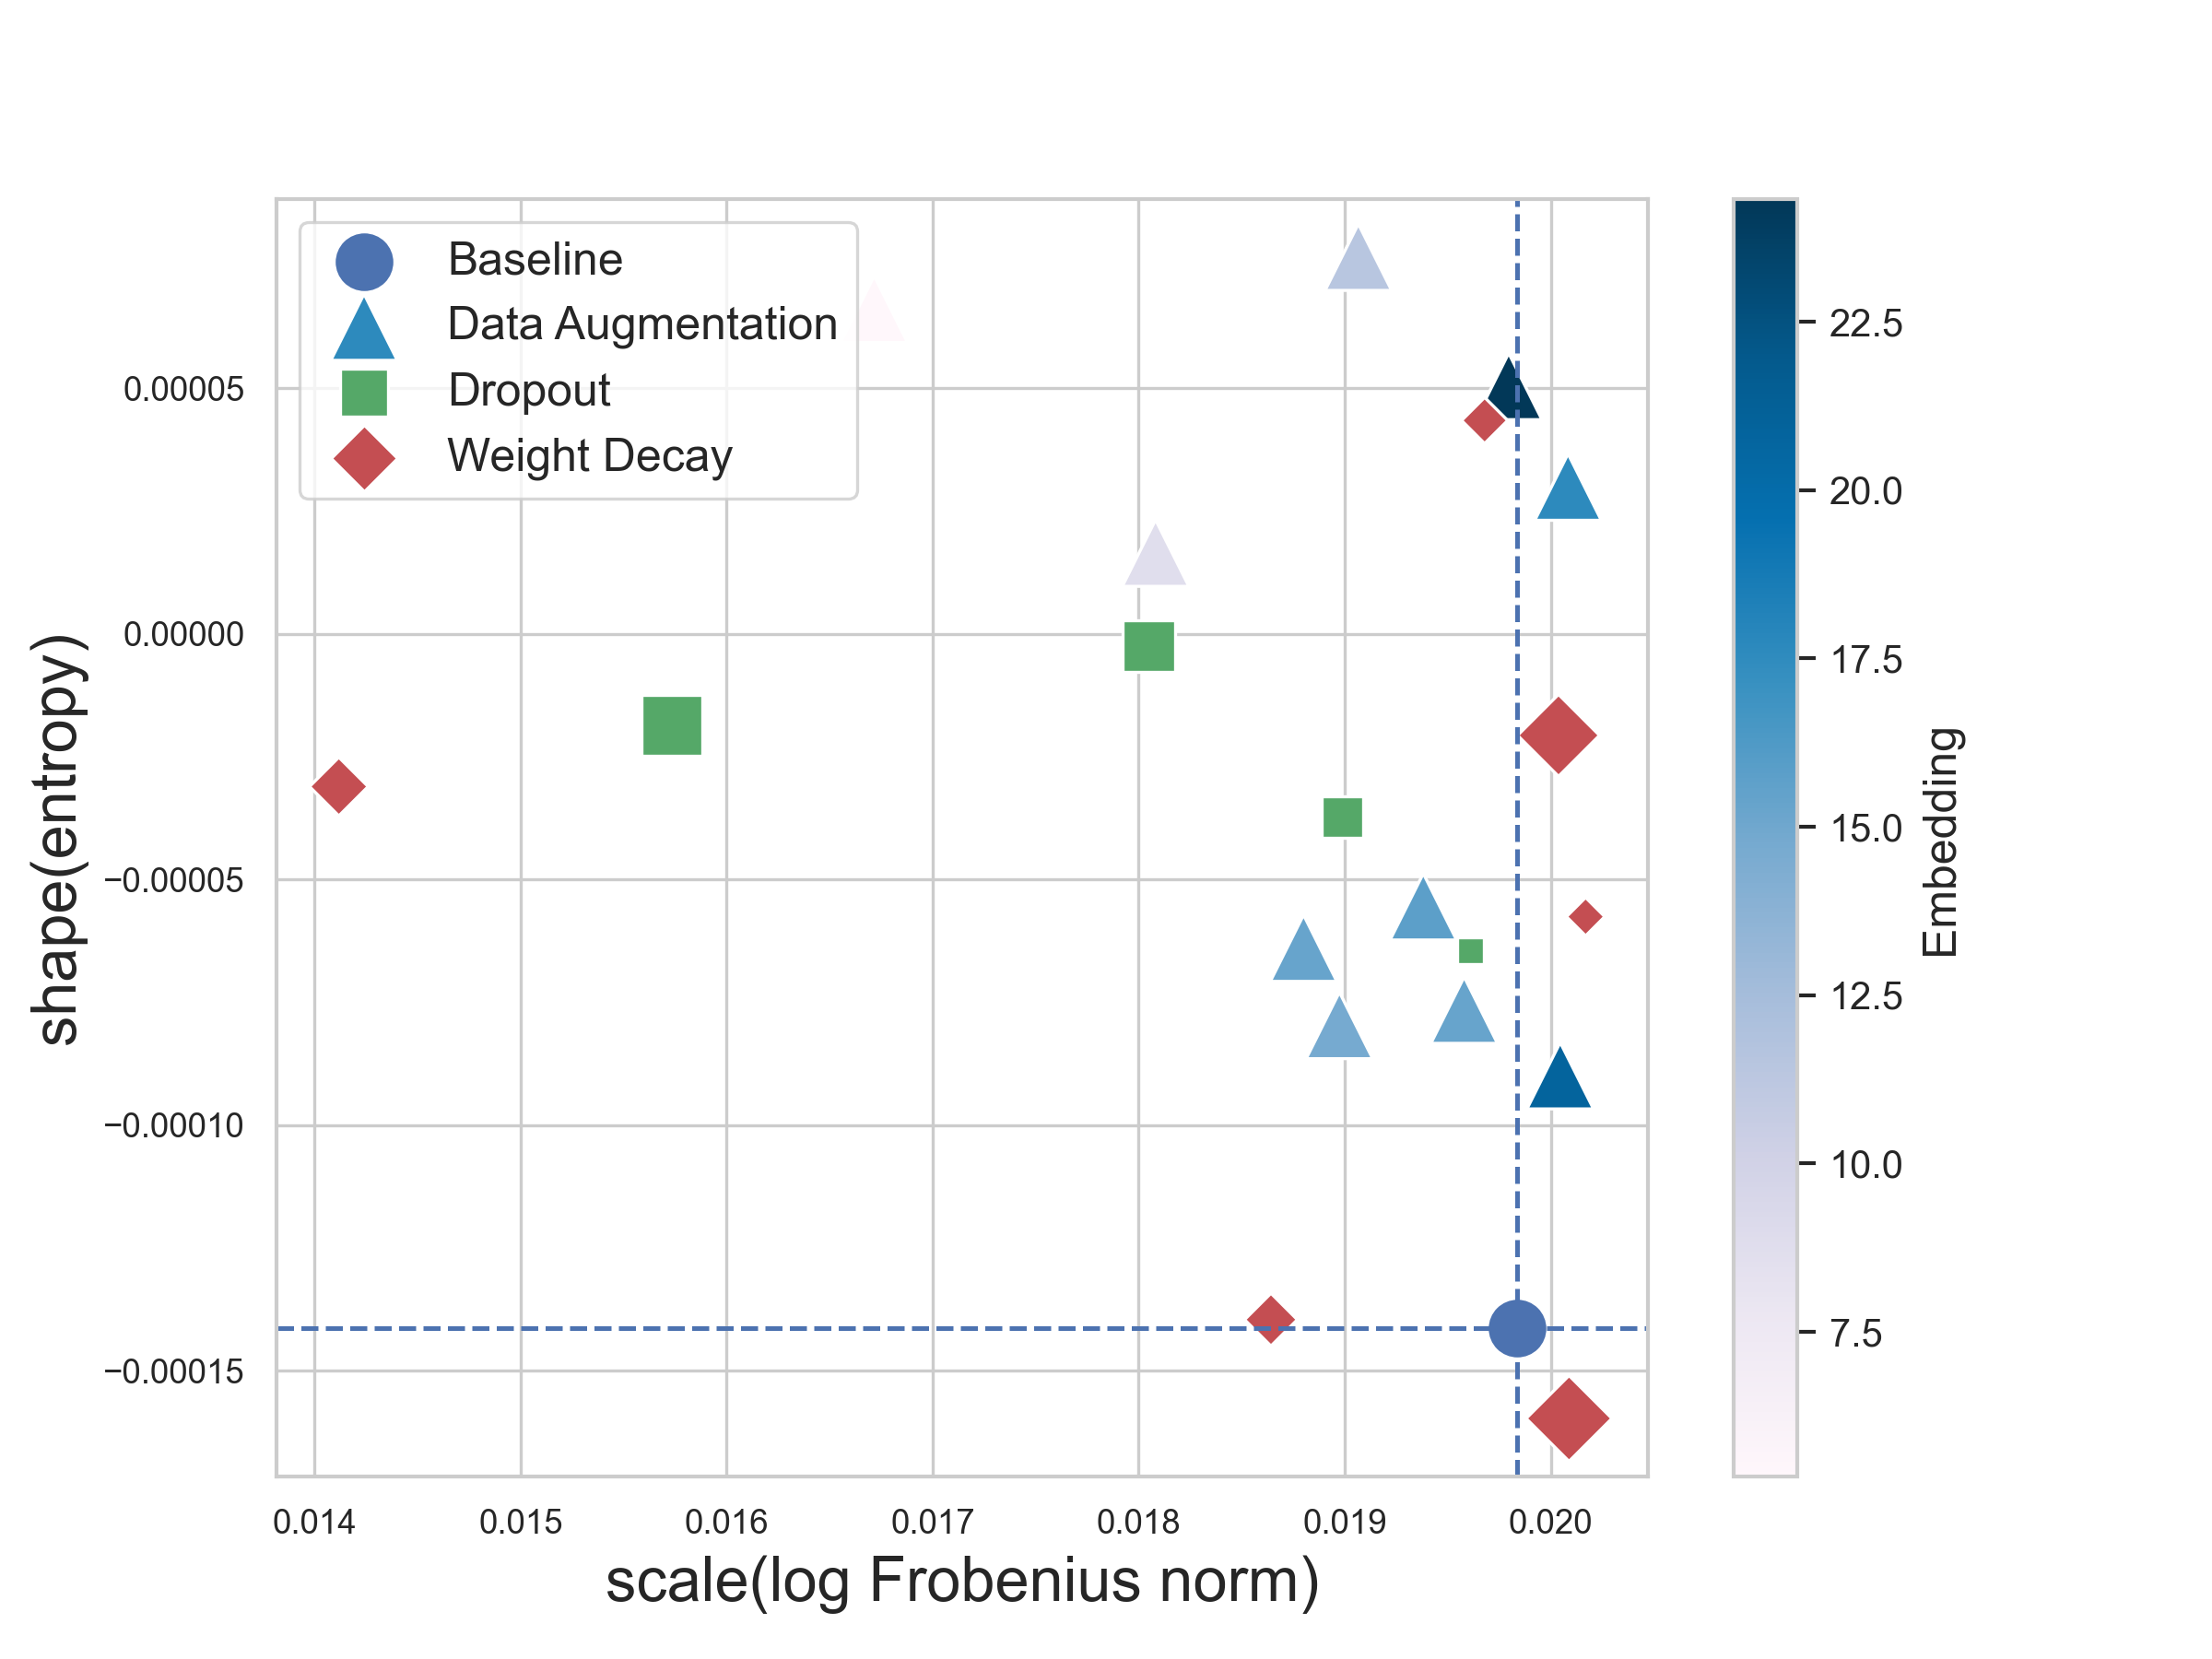}
        \caption{Frobenius norm vs. entropy on DomaineNet (real)}
        \label{fig:d-6}
    \end{subfigure}
    
    \caption{\textcolor{blue}{Scale-shape plots of ESDs of the classifier layers on CIFAR-10/100, Imagenette, Flower102, StandfordCars, DomainNet(Real). The results are marked with triangle, square, and diamond shapes for data augmentation, dropout, and weight decay, respectively. The color intensity of triangles represents the magnitude of embedding-based diversity scores. The results above are based on the ResNet50 backbone. Because of limitations of computing resources, CIFAR-10/100 and DomainNet(Real) refer to a subset that samples 5000 images for fine-tuning.}}
    \label{fig:div-cl-RN50}
\end{figure}

\begin{figure}[h]
    \centering
    % First row
    \begin{subfigure}[b]{0.45\textwidth}
        \centering
        \includegraphics[width=\textwidth]{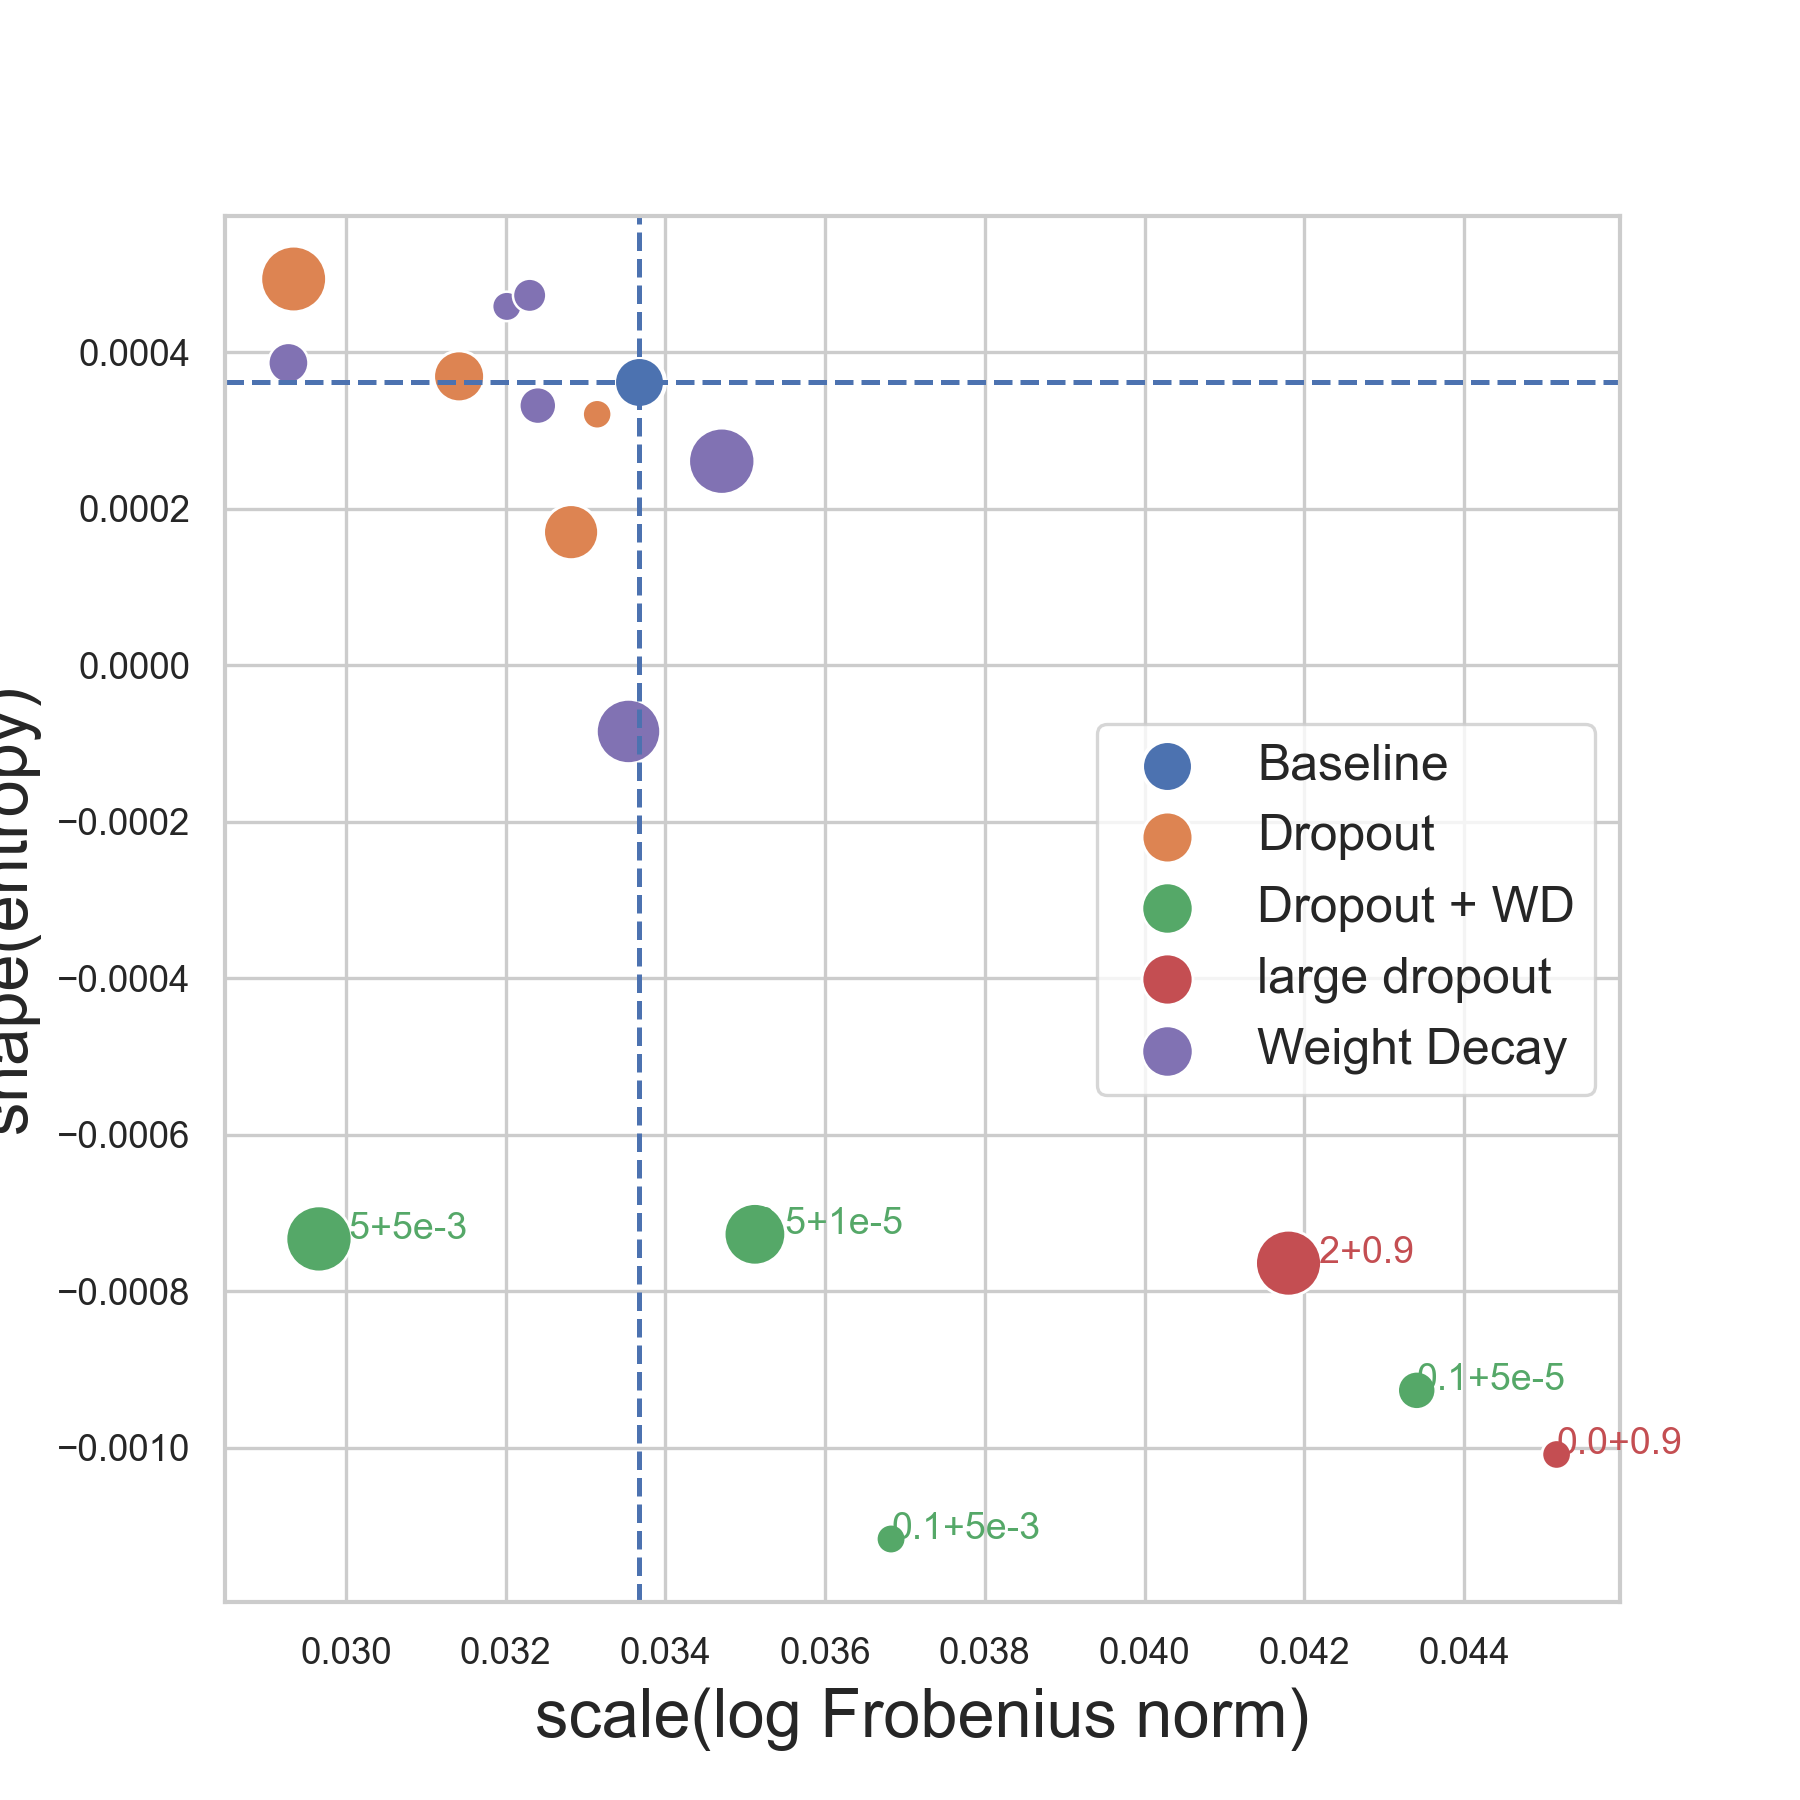}   % need to change 
        \caption{Frobenius norm vs. entropy on Imagenette (ViT)}
        \label{fig:reg1-}
    \end{subfigure}
    \hfill
    \begin{subfigure}[b]{0.45\textwidth}
        \centering
        \includegraphics[width=\textwidth]{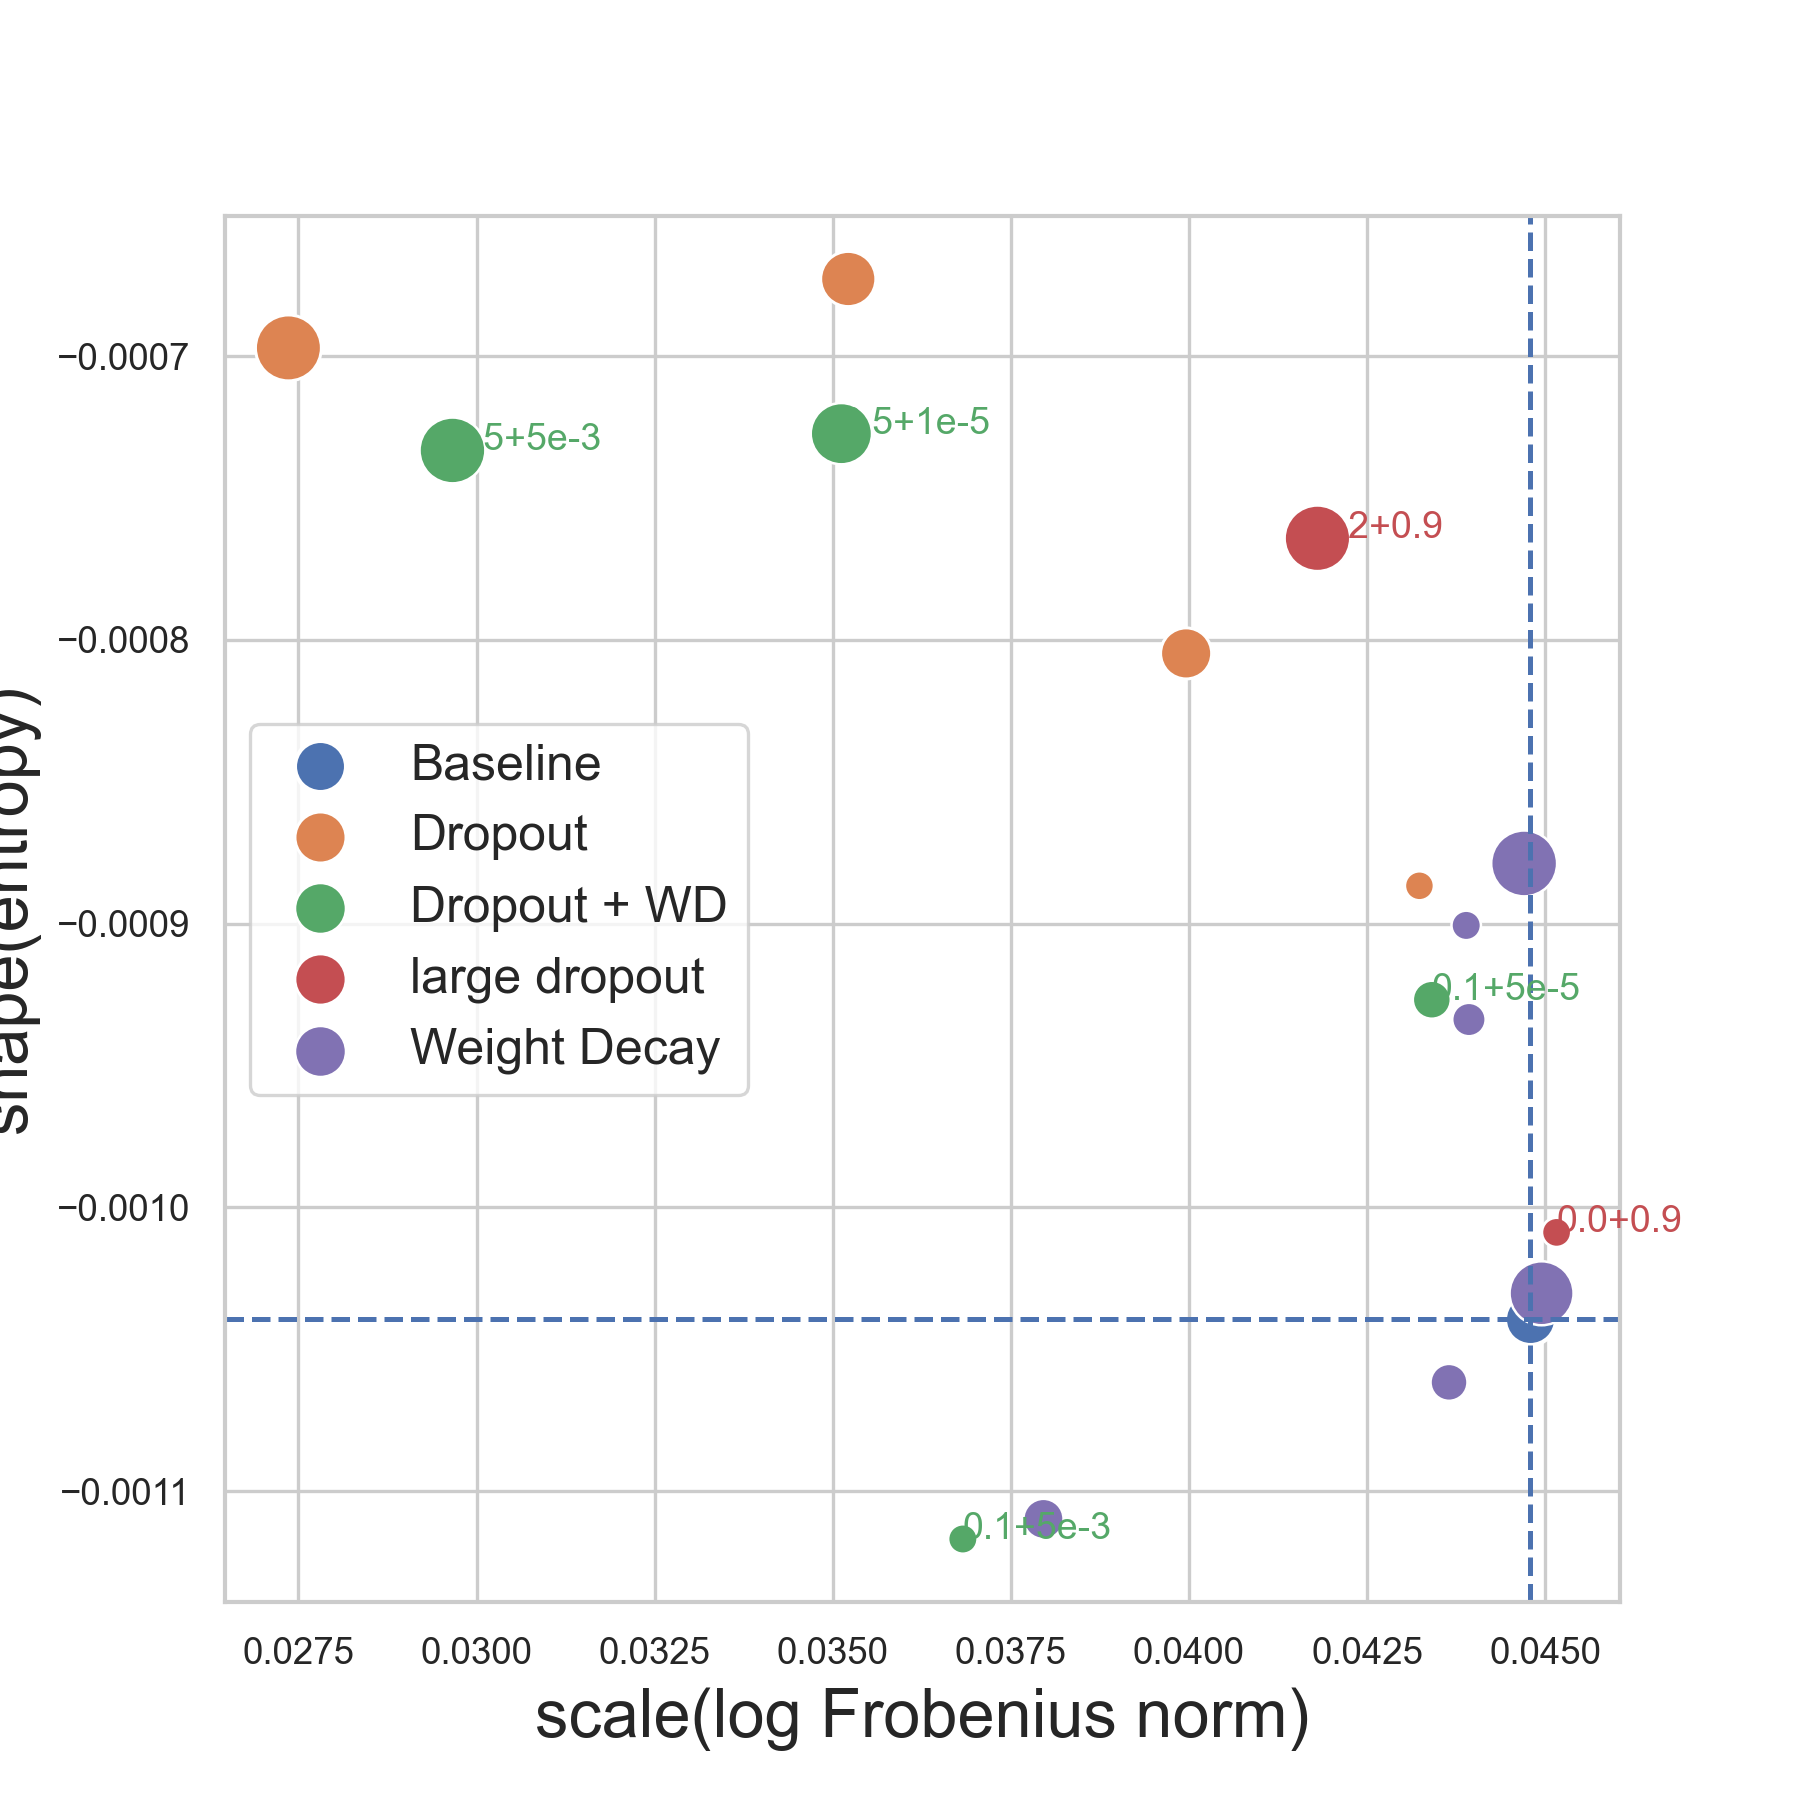}  % need to change 
        \caption{Frobenius norm vs. entropy on Flowers102 (ViT)}
        \label{fig:reg2-}
    \end{subfigure}
    
    \vspace{1em} % Add some vertical space between rows
    
    % Second row
    \begin{subfigure}[b]{0.45\textwidth}
        \centering
        \includegraphics[width=\textwidth]{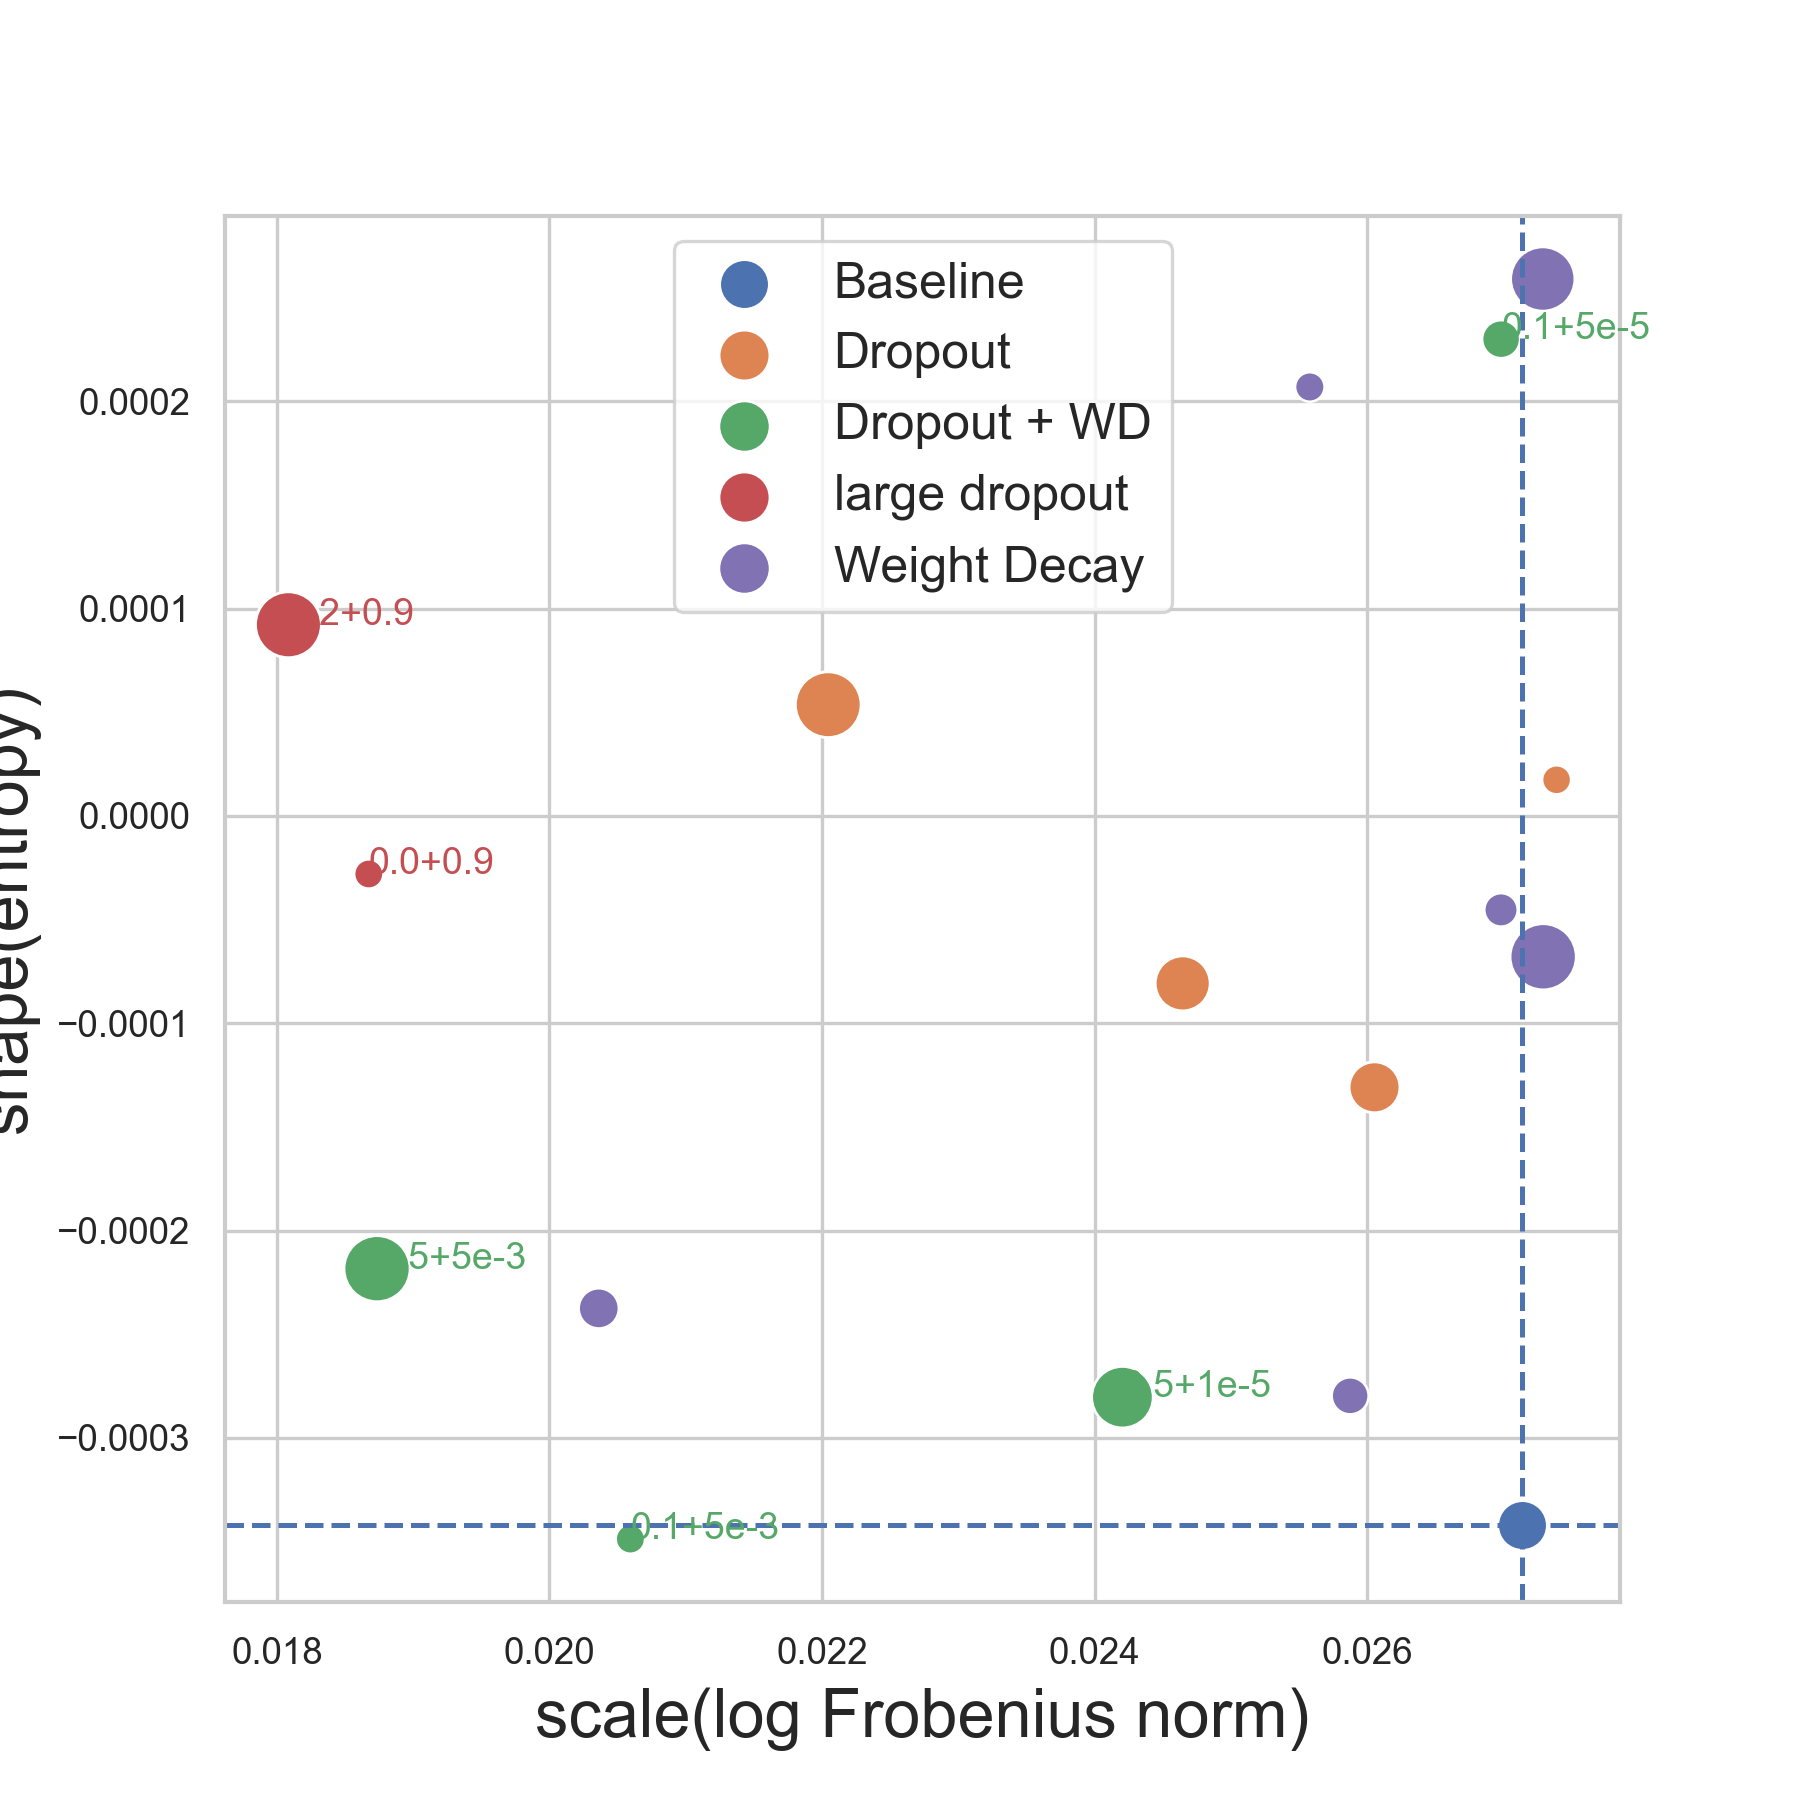}
        \caption{Frobenius norm vs. entropy on Imagenette (ResNet50)}
        \label{fig:reg4-}
    \end{subfigure}
    \hfill
    \begin{subfigure}[b]{0.45\textwidth}
        \centering
        \includegraphics[width=\textwidth]{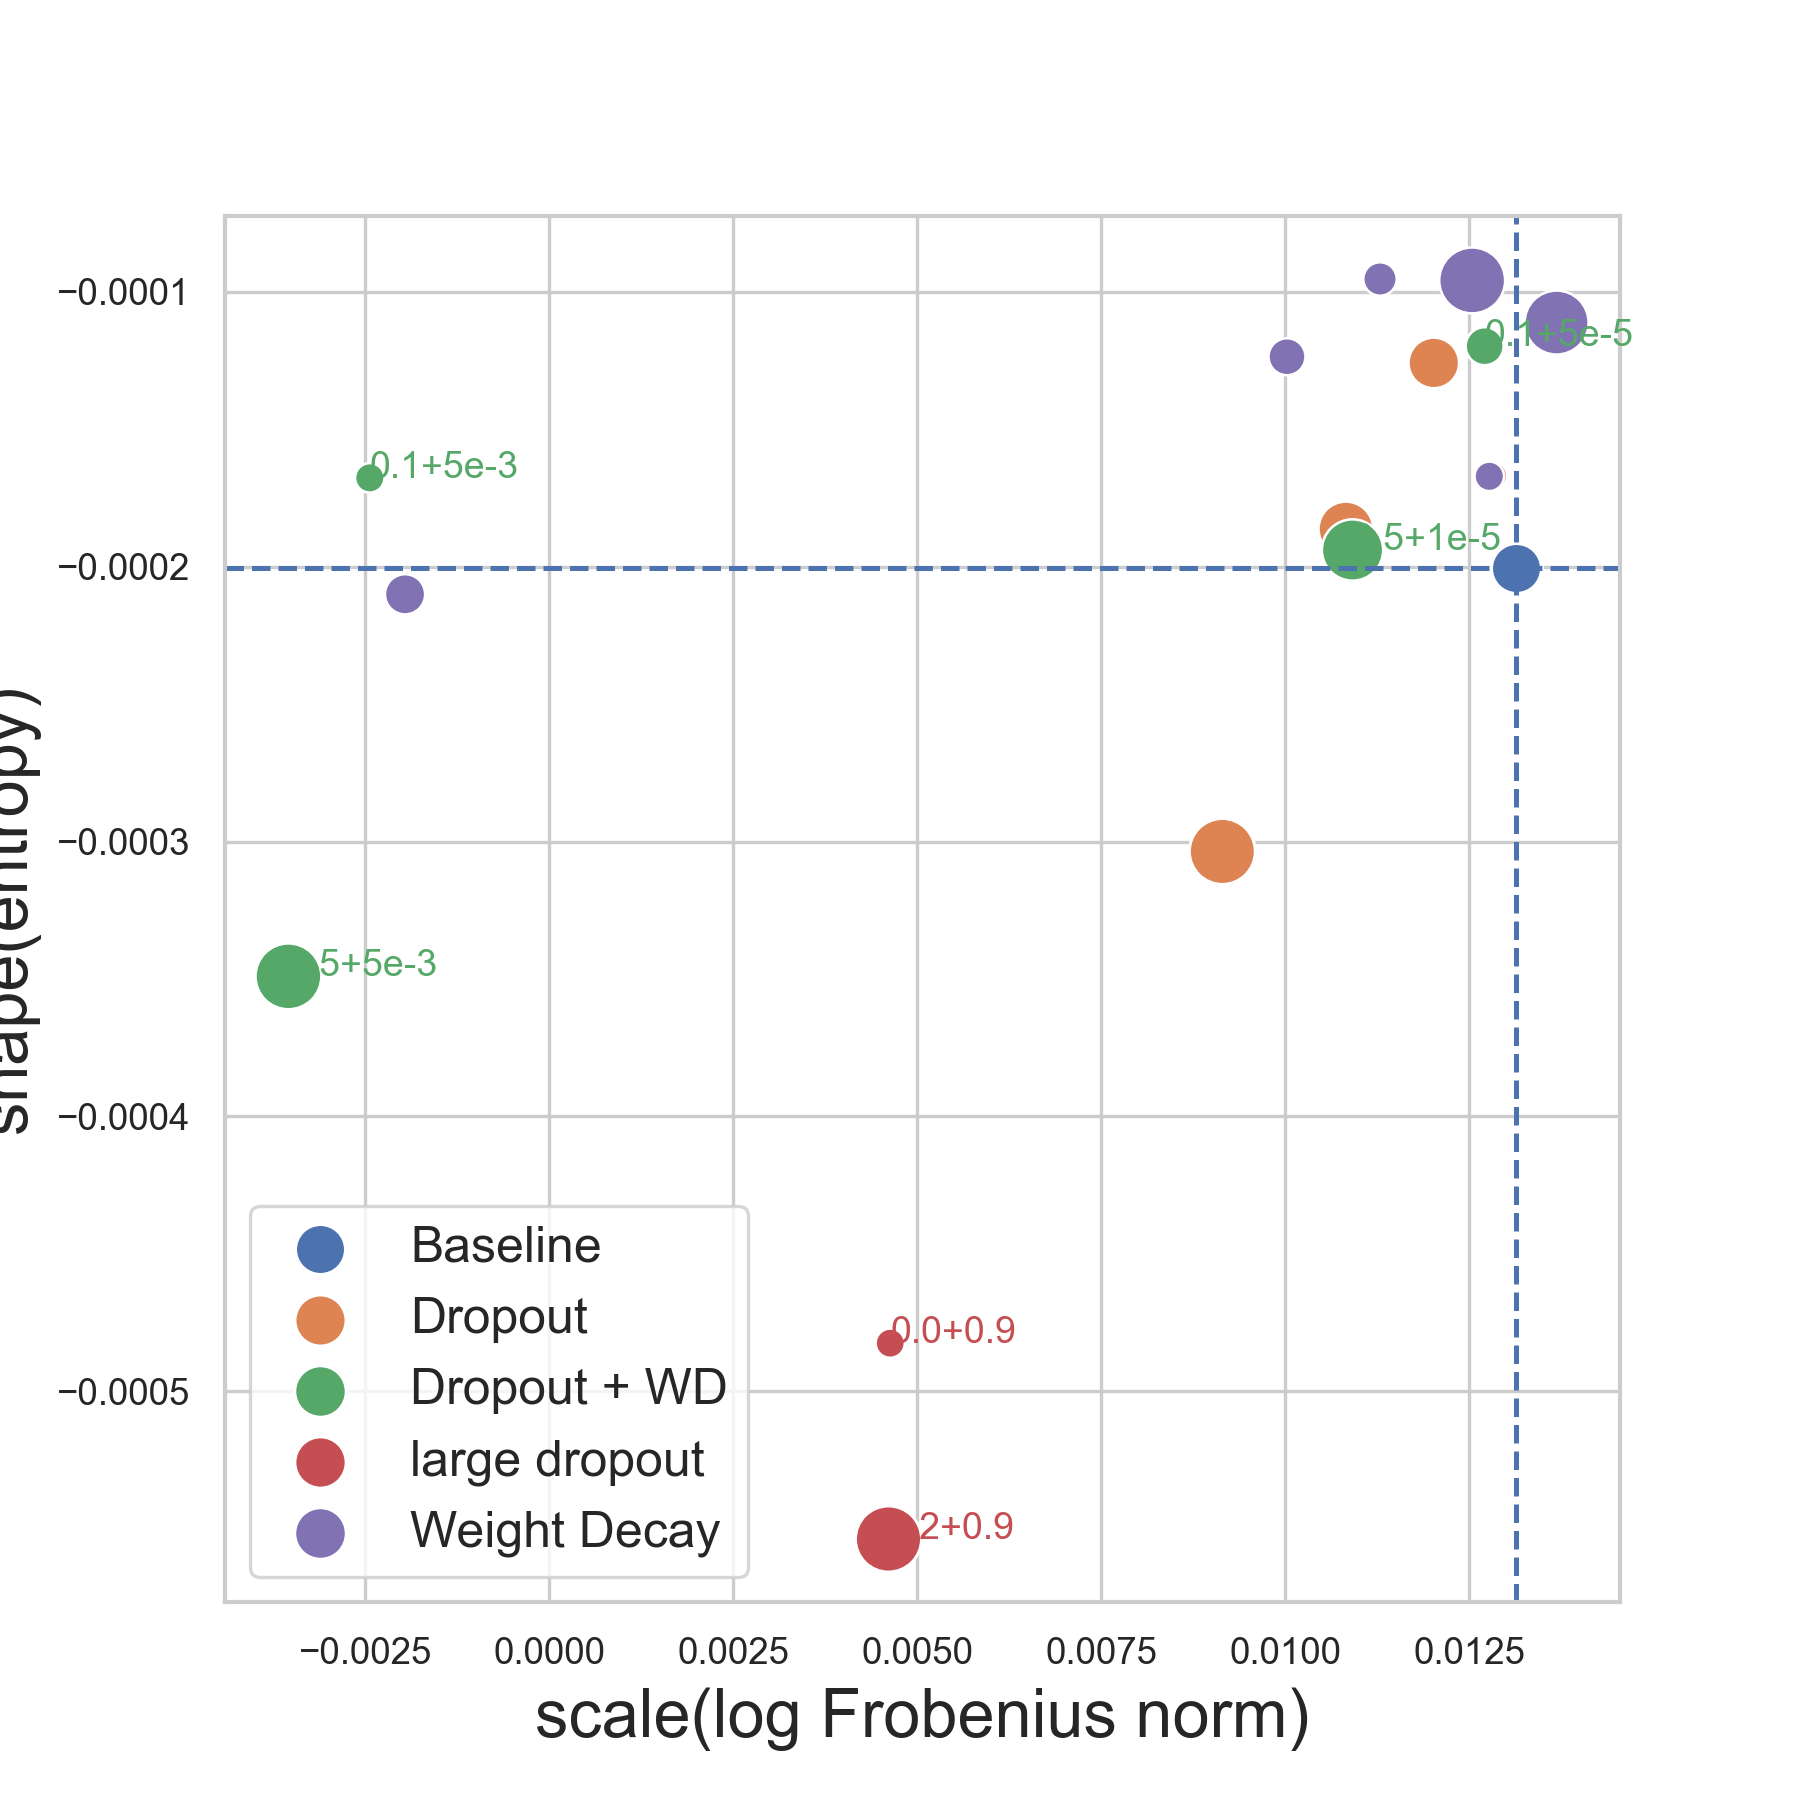}
        \caption{Frobenius norm vs. entropy on Flowers102 (ResNet50)}
        \label{fig:reg5-}
    \end{subfigure}
    
    \caption{\textcolor{blue}{Scale-shape plots of ESDs of the classifier layers on Imagenette and Flower102. The results are marked with square and diamond shapes for dropout and weight decay regularization techniques, respectively. The size of markers represents the magnitude of the dropout rate and weight decay values. We also refer \citep{zhang2024fine} to apply a very large dropout (0.9 at the last layer), as well as combinations with dropout(0.1, 0.5) and weight decay (1e-5, 5e-3). Results show us combinations with dropout and weight decay, as well as the very large dropout can make more intense changes in both scale and shape side.}}
    \label{fig:large}
\end{figure}

\begin{figure}[h]
    \centering
    % First row
    \begin{subfigure}[b]{0.3\textwidth}
        \centering
        \includegraphics[width=\textwidth]{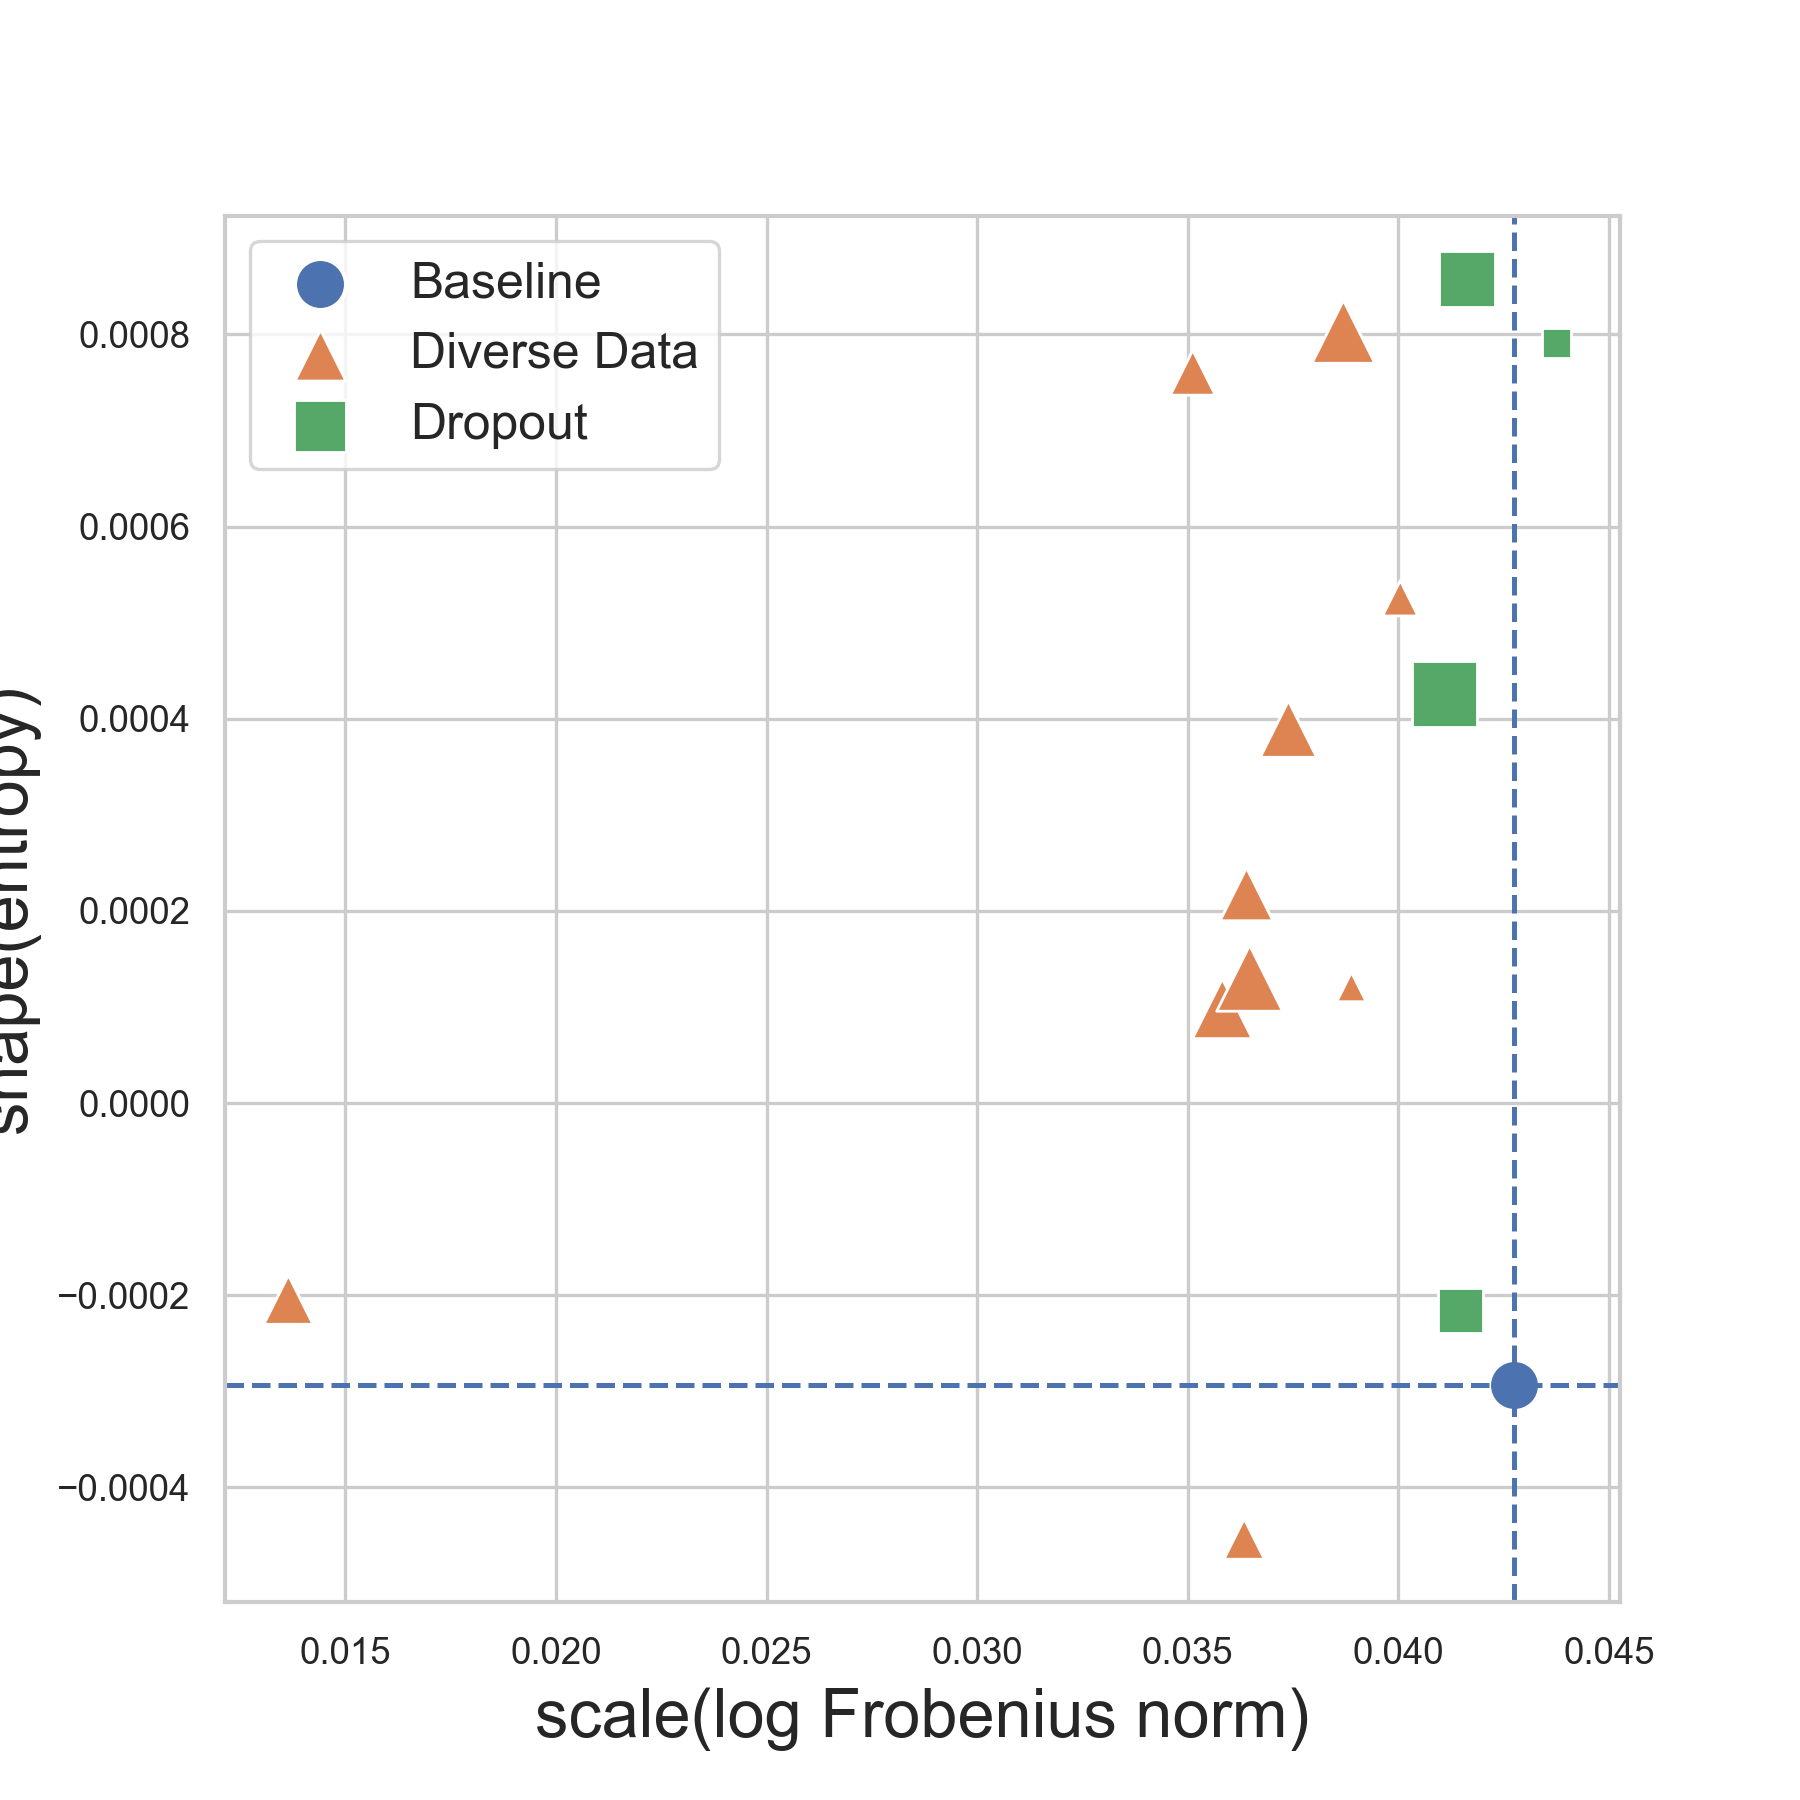}
        \caption{Frobenius norm vs. entropy on CIFAR-10}
        % \label{fig:div1}
    \end{subfigure}
    \hfill
    \begin{subfigure}[b]{0.3\textwidth}
        \centering
        \includegraphics[width=\textwidth]{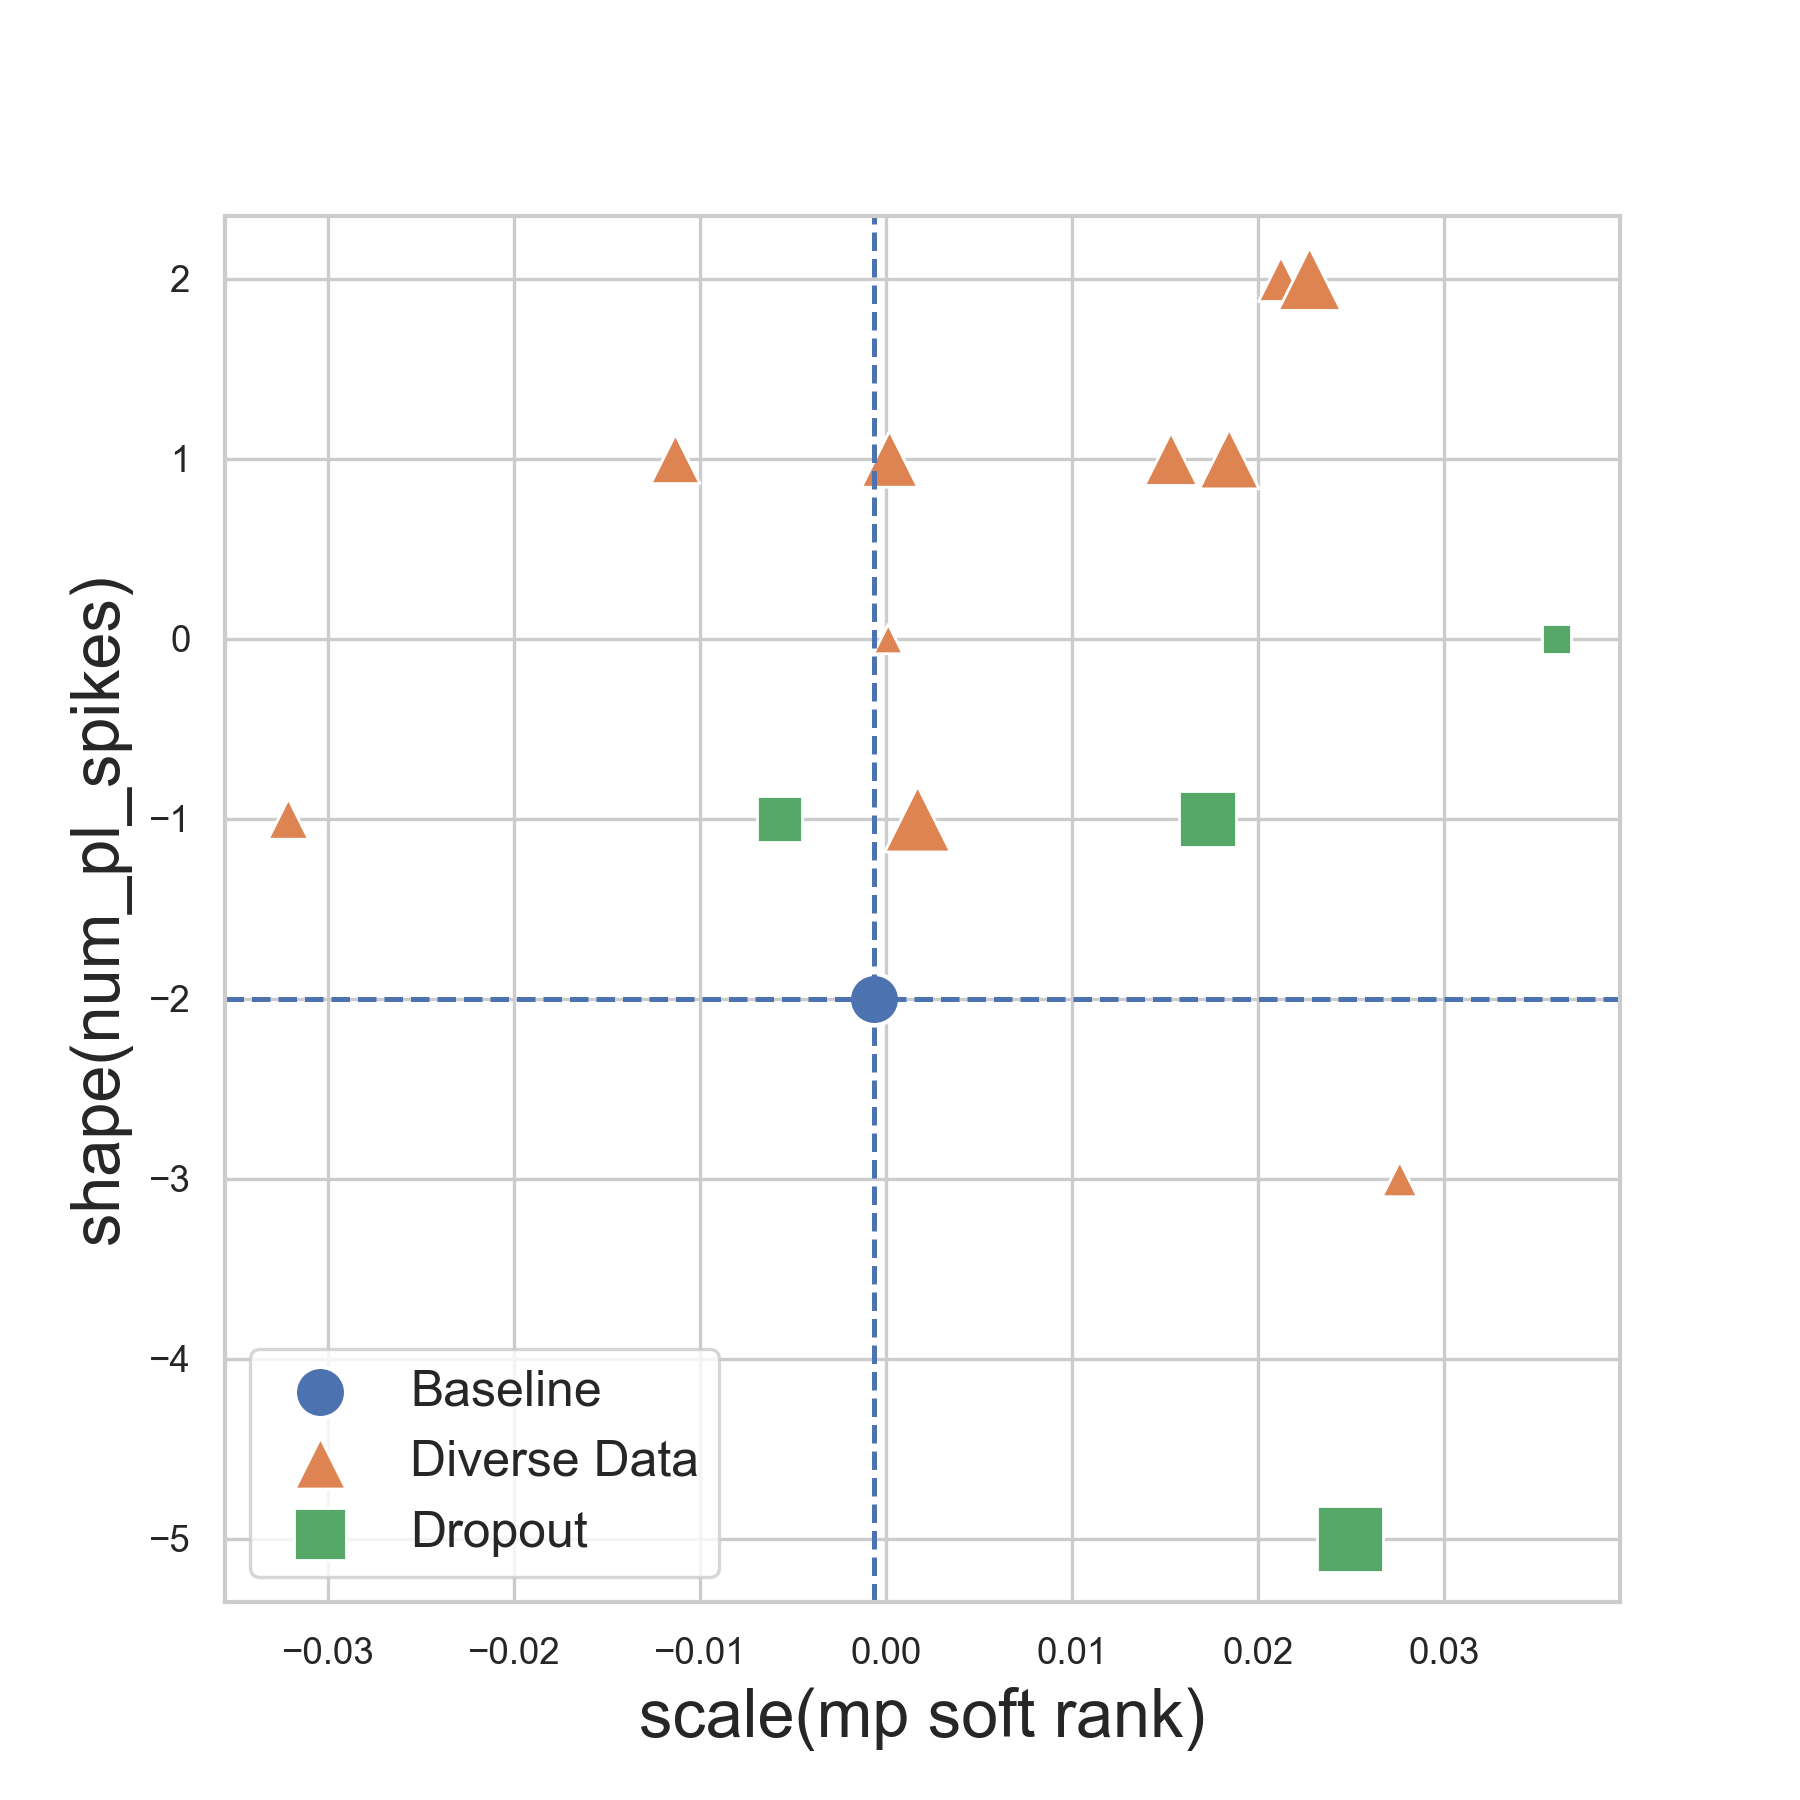}
        \caption{MP soft rank  vs. $\textit{num\_pl\_spikes}$ on CIFAR-10}
        % \label{fig:div2}
    \end{subfigure}
    \hfill
    \begin{subfigure}[b]{0.3\textwidth}
        \centering
        \includegraphics[width=\textwidth]{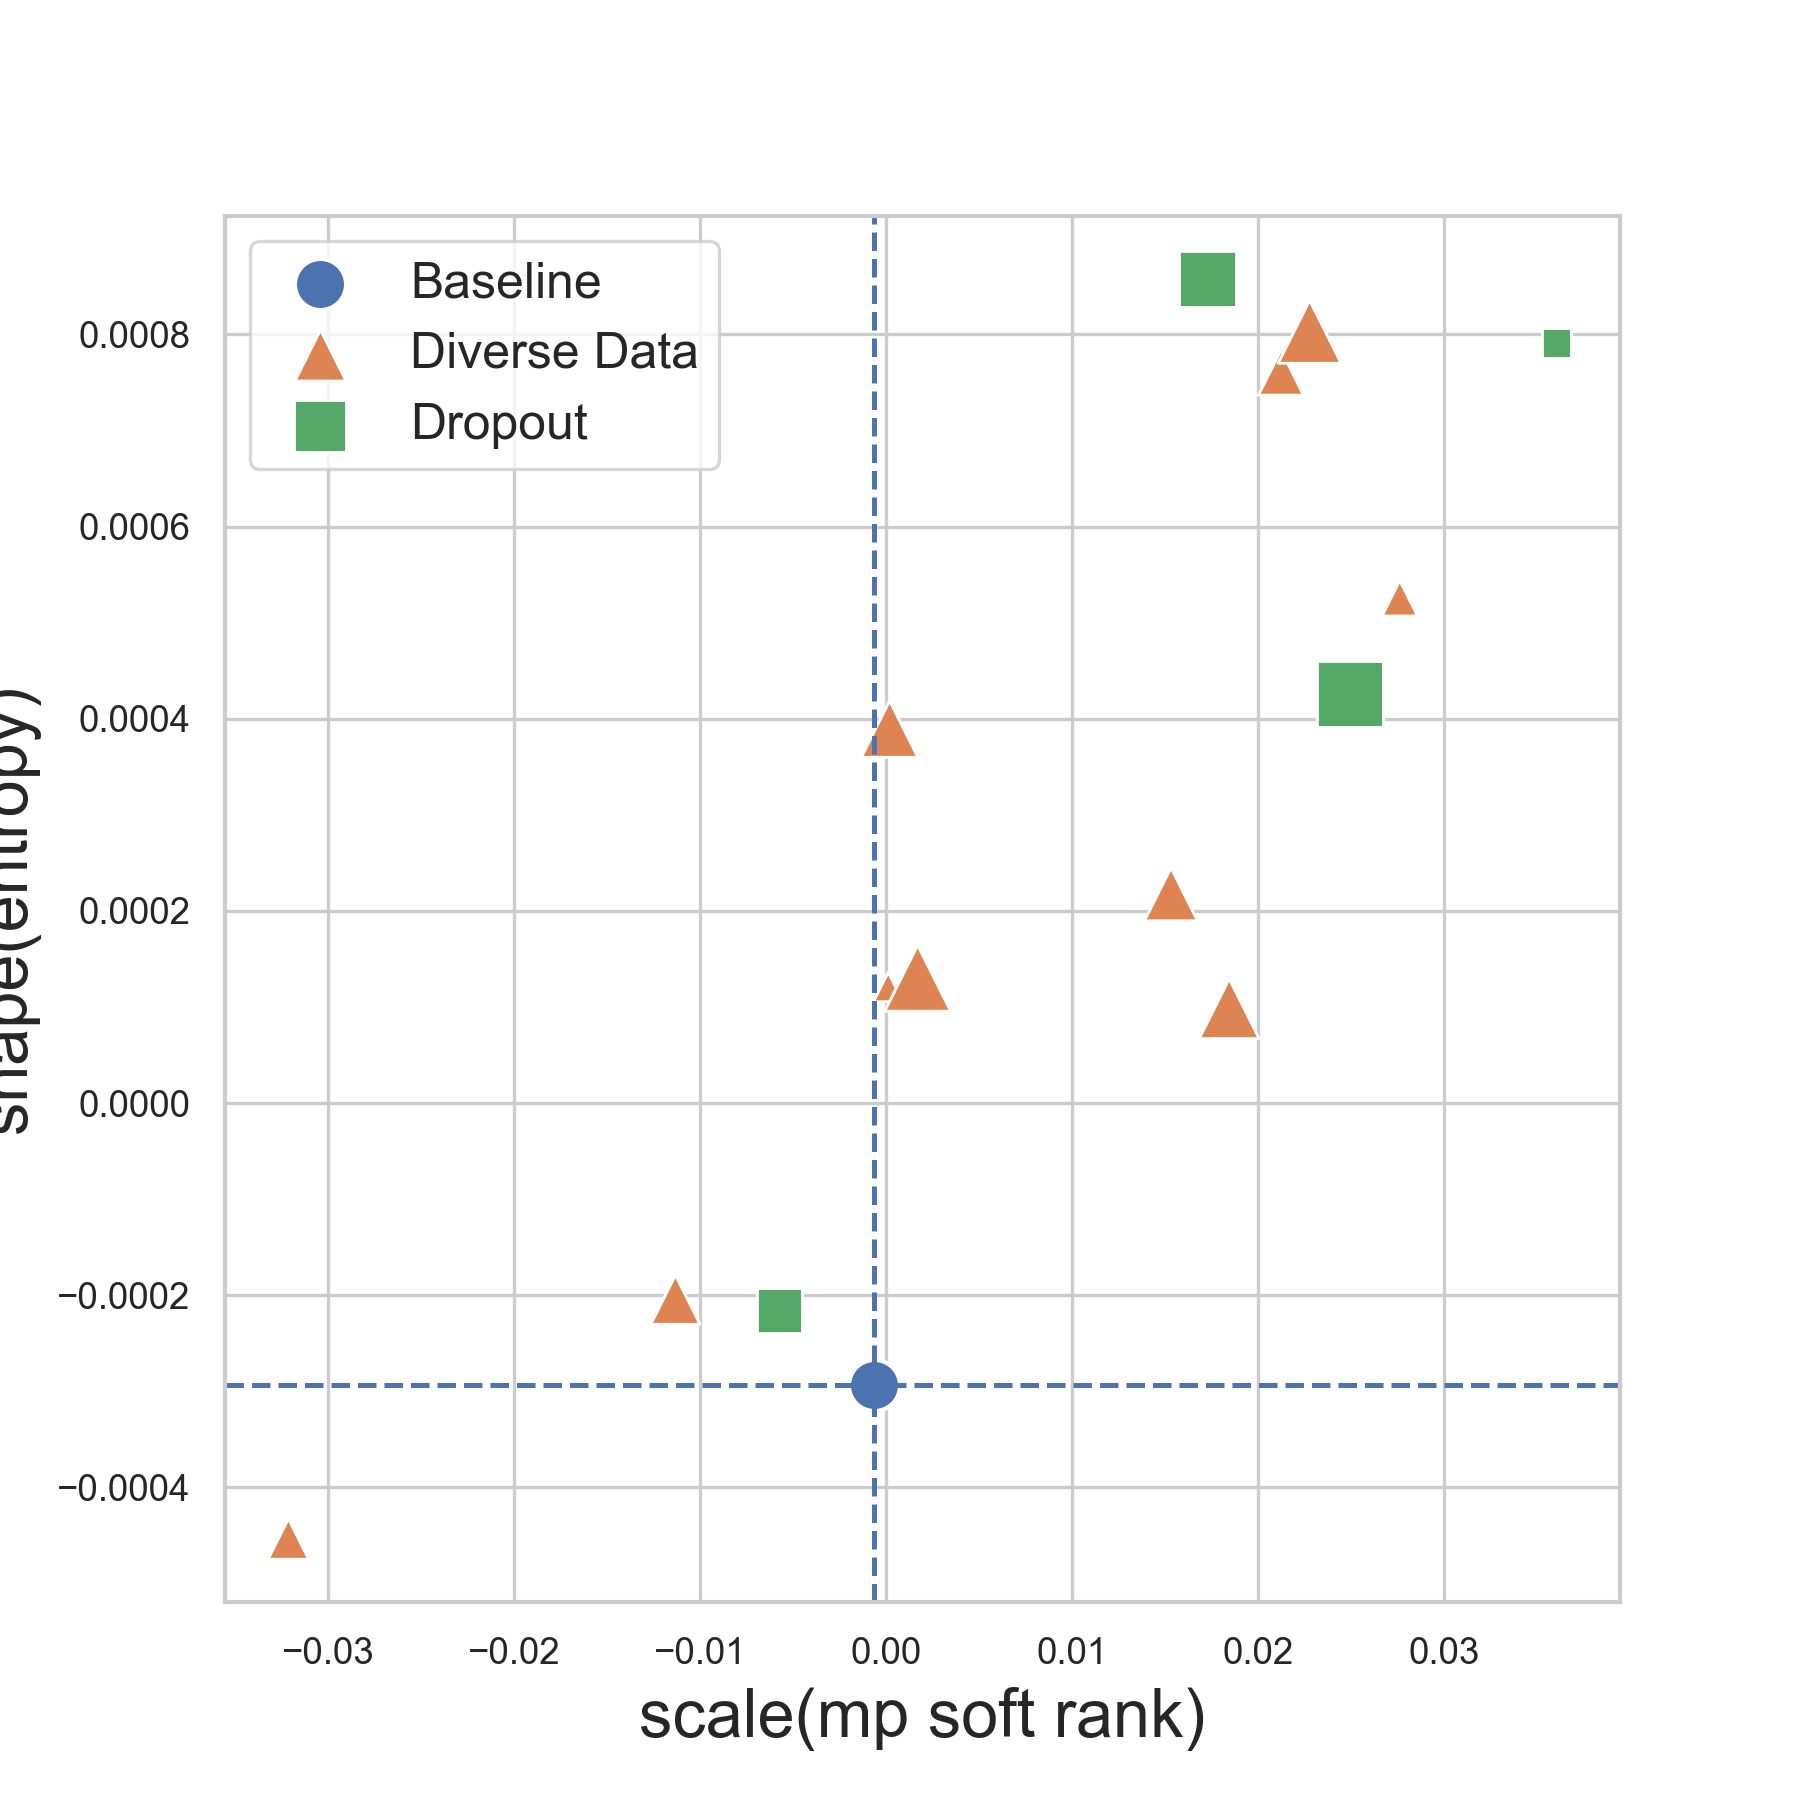}
        \caption{MP soft rank vs. entropy on CIFAR-10}
        % \label{fig:div3}
    \end{subfigure}
    
    \vspace{1em} % Add some vertical space between rows
    
    % Second row
    \begin{subfigure}[b]{0.3\textwidth}
        \centering
        \includegraphics[width=\textwidth]{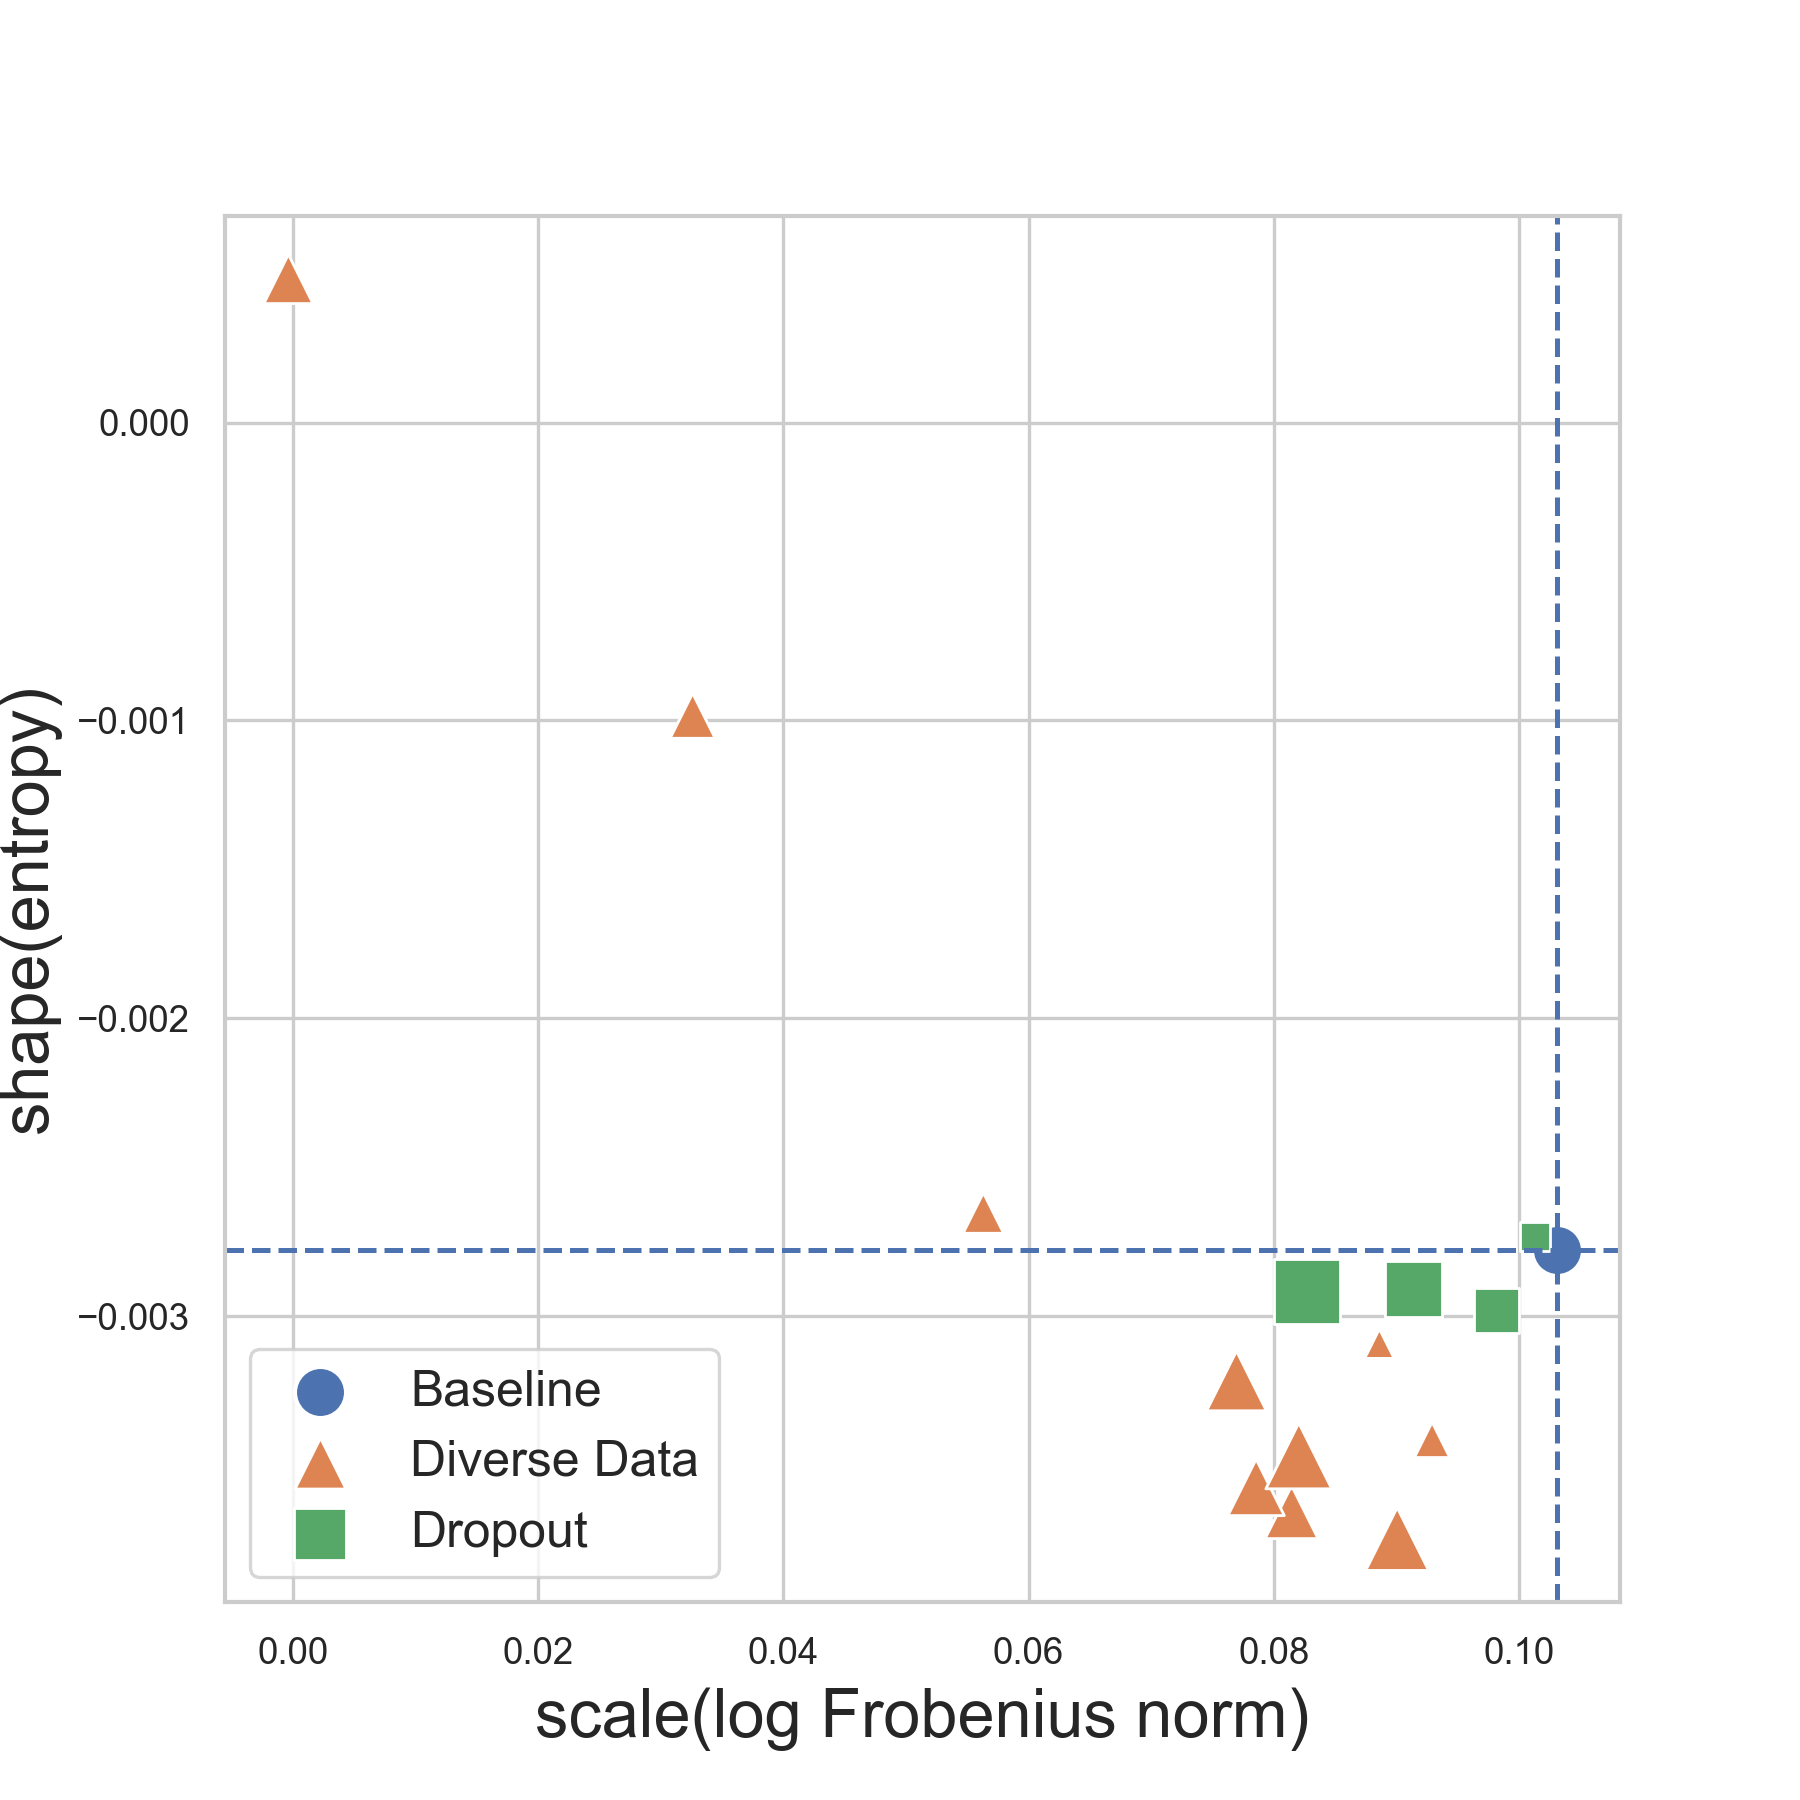}
        \caption{Frobenius norm vs. entropy on CIFAR-100}
        % \label{fig:di-4}
    \end{subfigure}
    \hfill
    \begin{subfigure}[b]{0.3\textwidth}
        \centering
        \includegraphics[width=\textwidth]{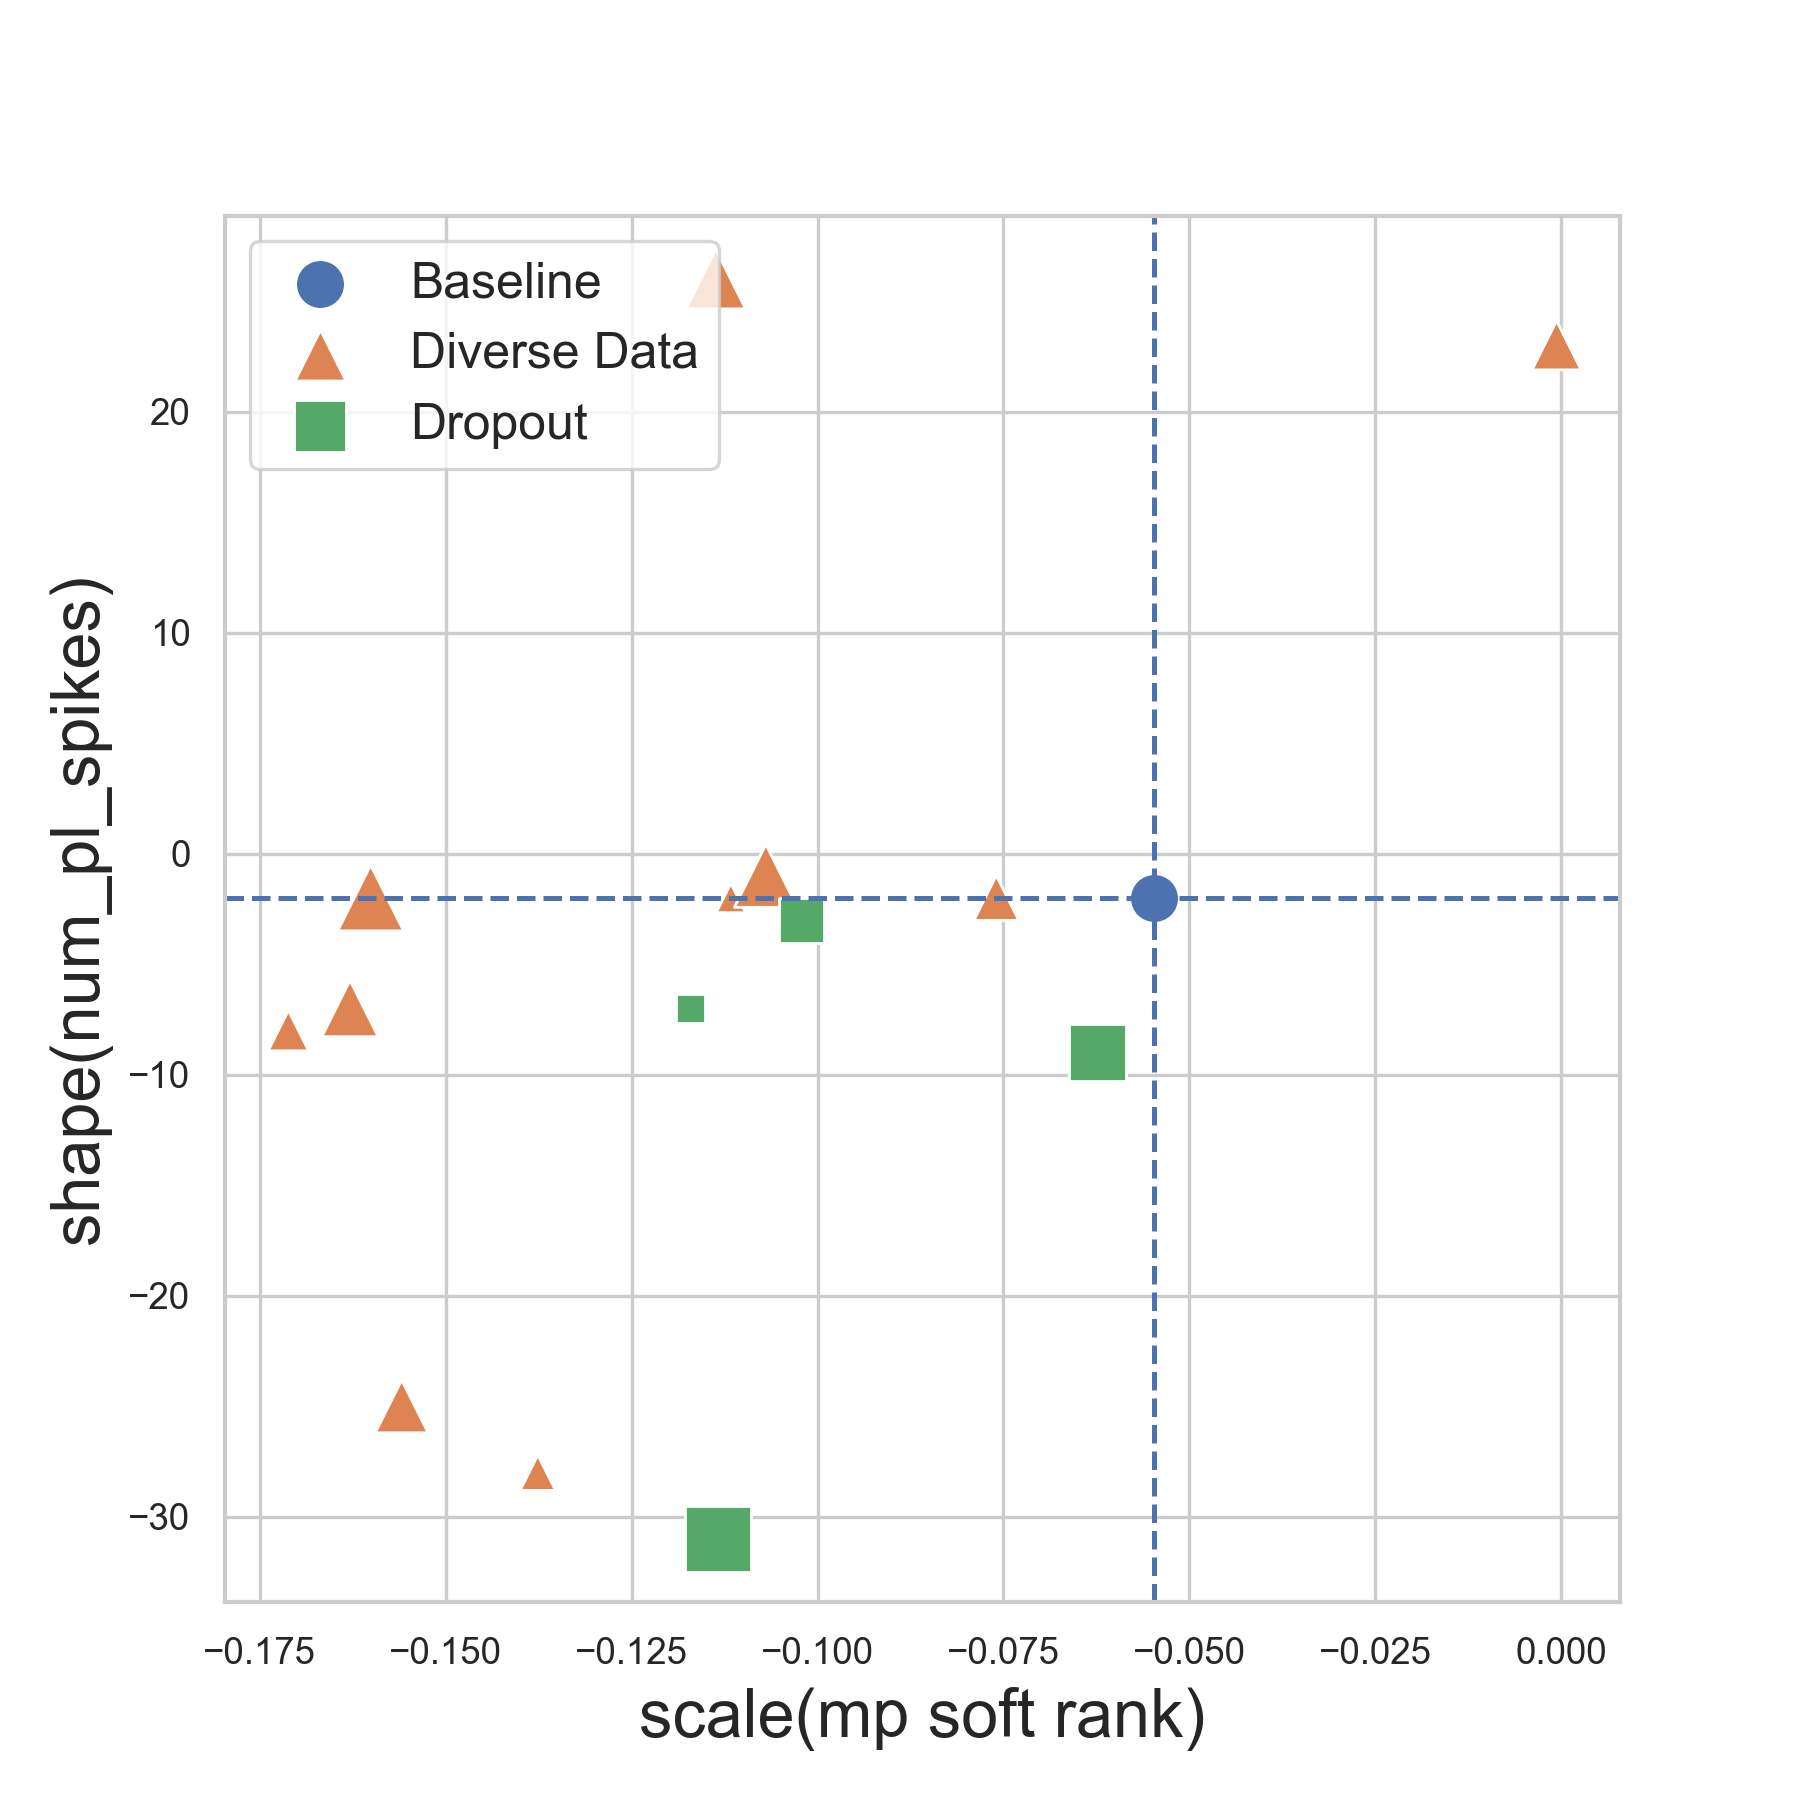}
        \caption{MP soft rank  vs. $\textit{num\_pl\_spikes}$ on CIFAR-100}
        % \label{fig:di-5}
    \end{subfigure}
    \hfill
    \begin{subfigure}[b]{0.3\textwidth}
        \centering
        \includegraphics[width=\textwidth]{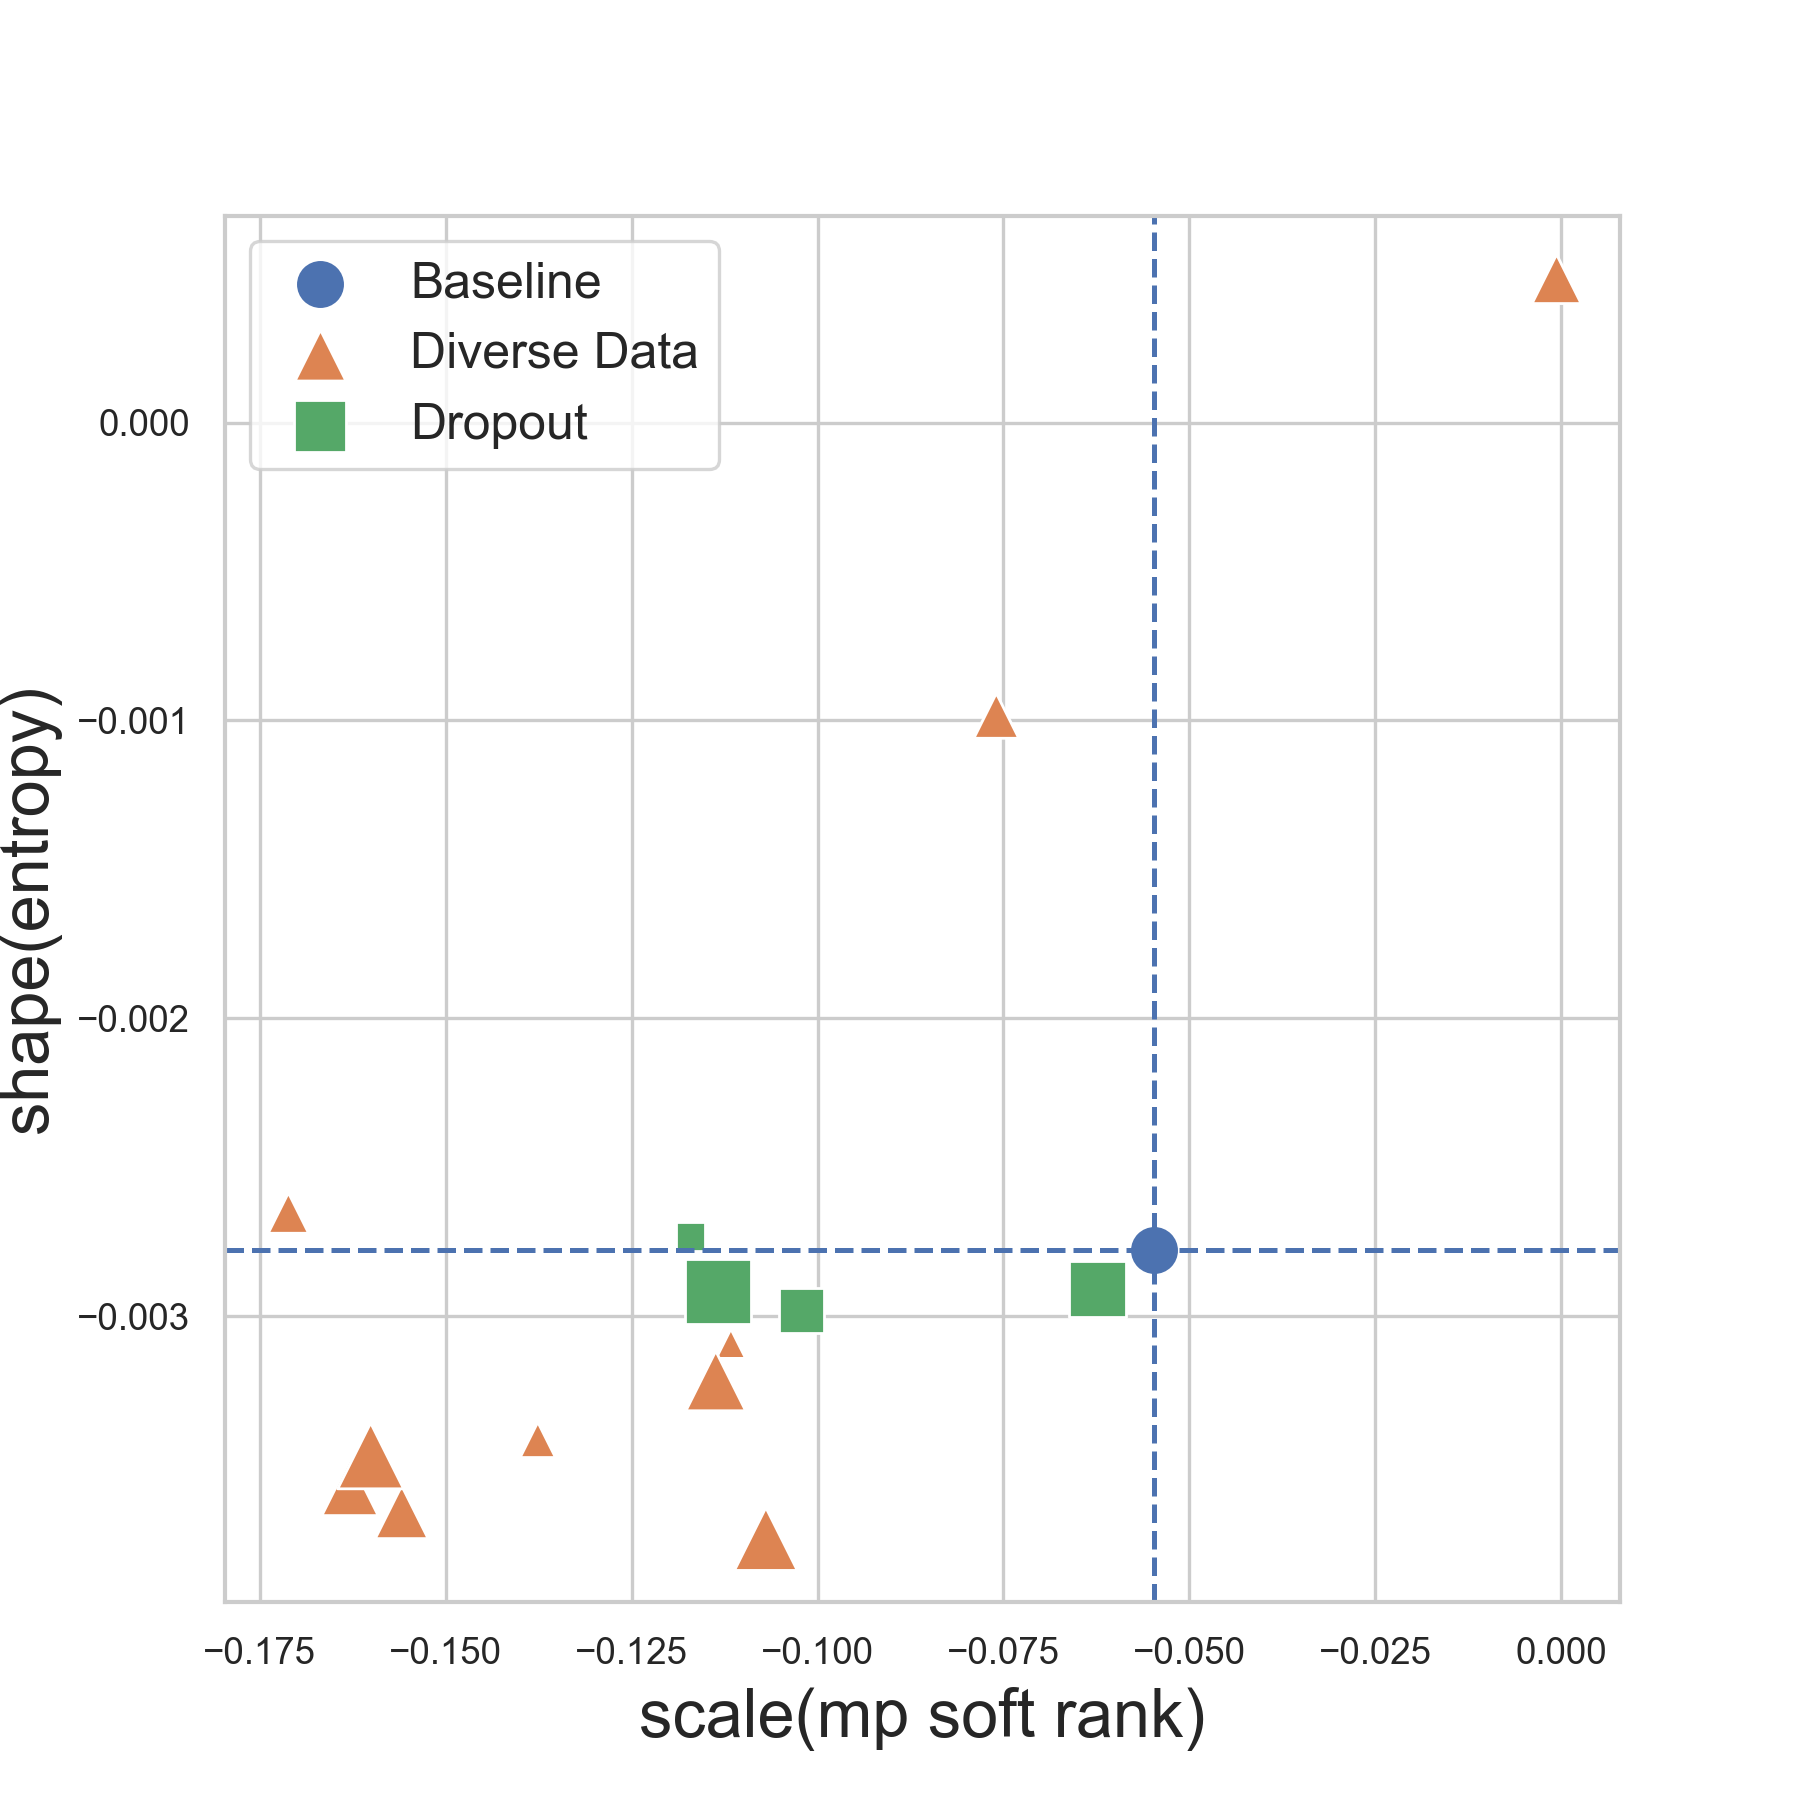}
        \caption{MP soft rank vs. entropy on CIFAR-100}
    \end{subfigure}
    
    \caption{Various scale-shape plots of ESDs of the classification layer on CIFAR-10 and CIFAR-100. The results are marked with triangle and square shapes for data augmentation and dropout, respectively. T\textbf{he size of markers represents the magnitude of the dropout rate and embedding-based Vendi score. More metrics from both scale and shape sides to compare dropout with data augmentations. These plots strengthen our conclusion about the similarity between dropout and diverse data in section 3. }}
    \label{fig:vision}
\end{figure}

\begin{figure}[h]
    \centering
    % First row
    \begin{subfigure}[b]{0.3\textwidth}
        \centering
        \includegraphics[width=\textwidth]{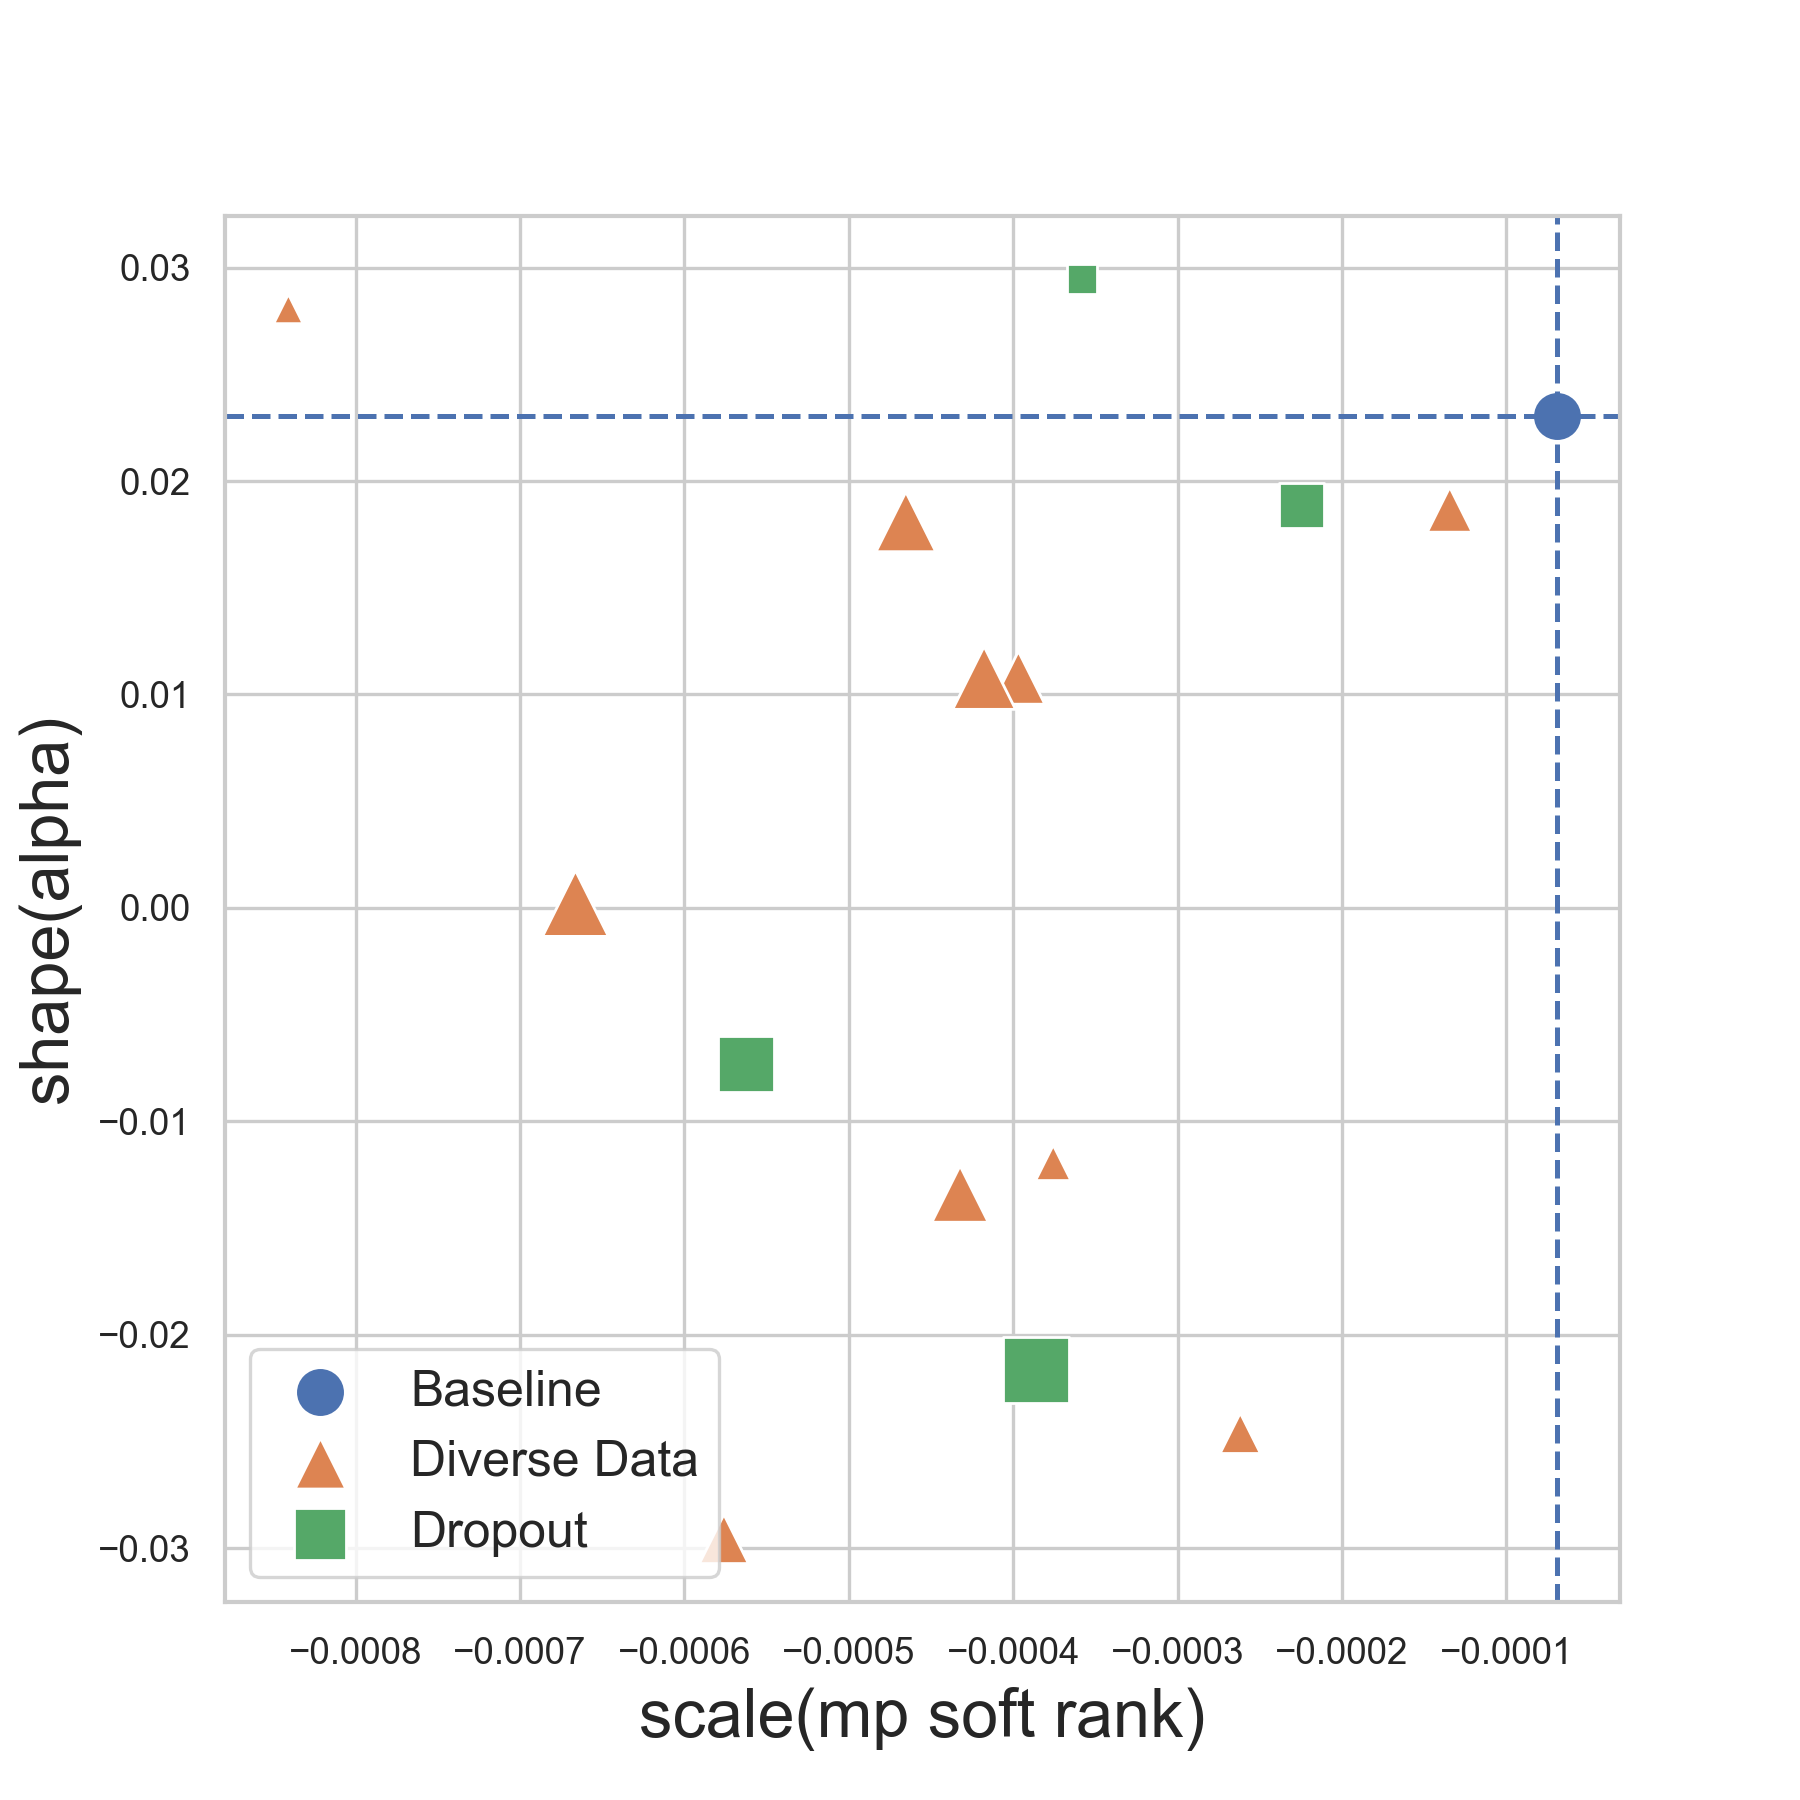}
        \caption{MP soft rank vs. alpha on CIFAR-10}
        % \label{fig:div-1}
    \end{subfigure}
    \hfill
    \begin{subfigure}[b]{0.3\textwidth}
        \centering
        \includegraphics[width=\textwidth]{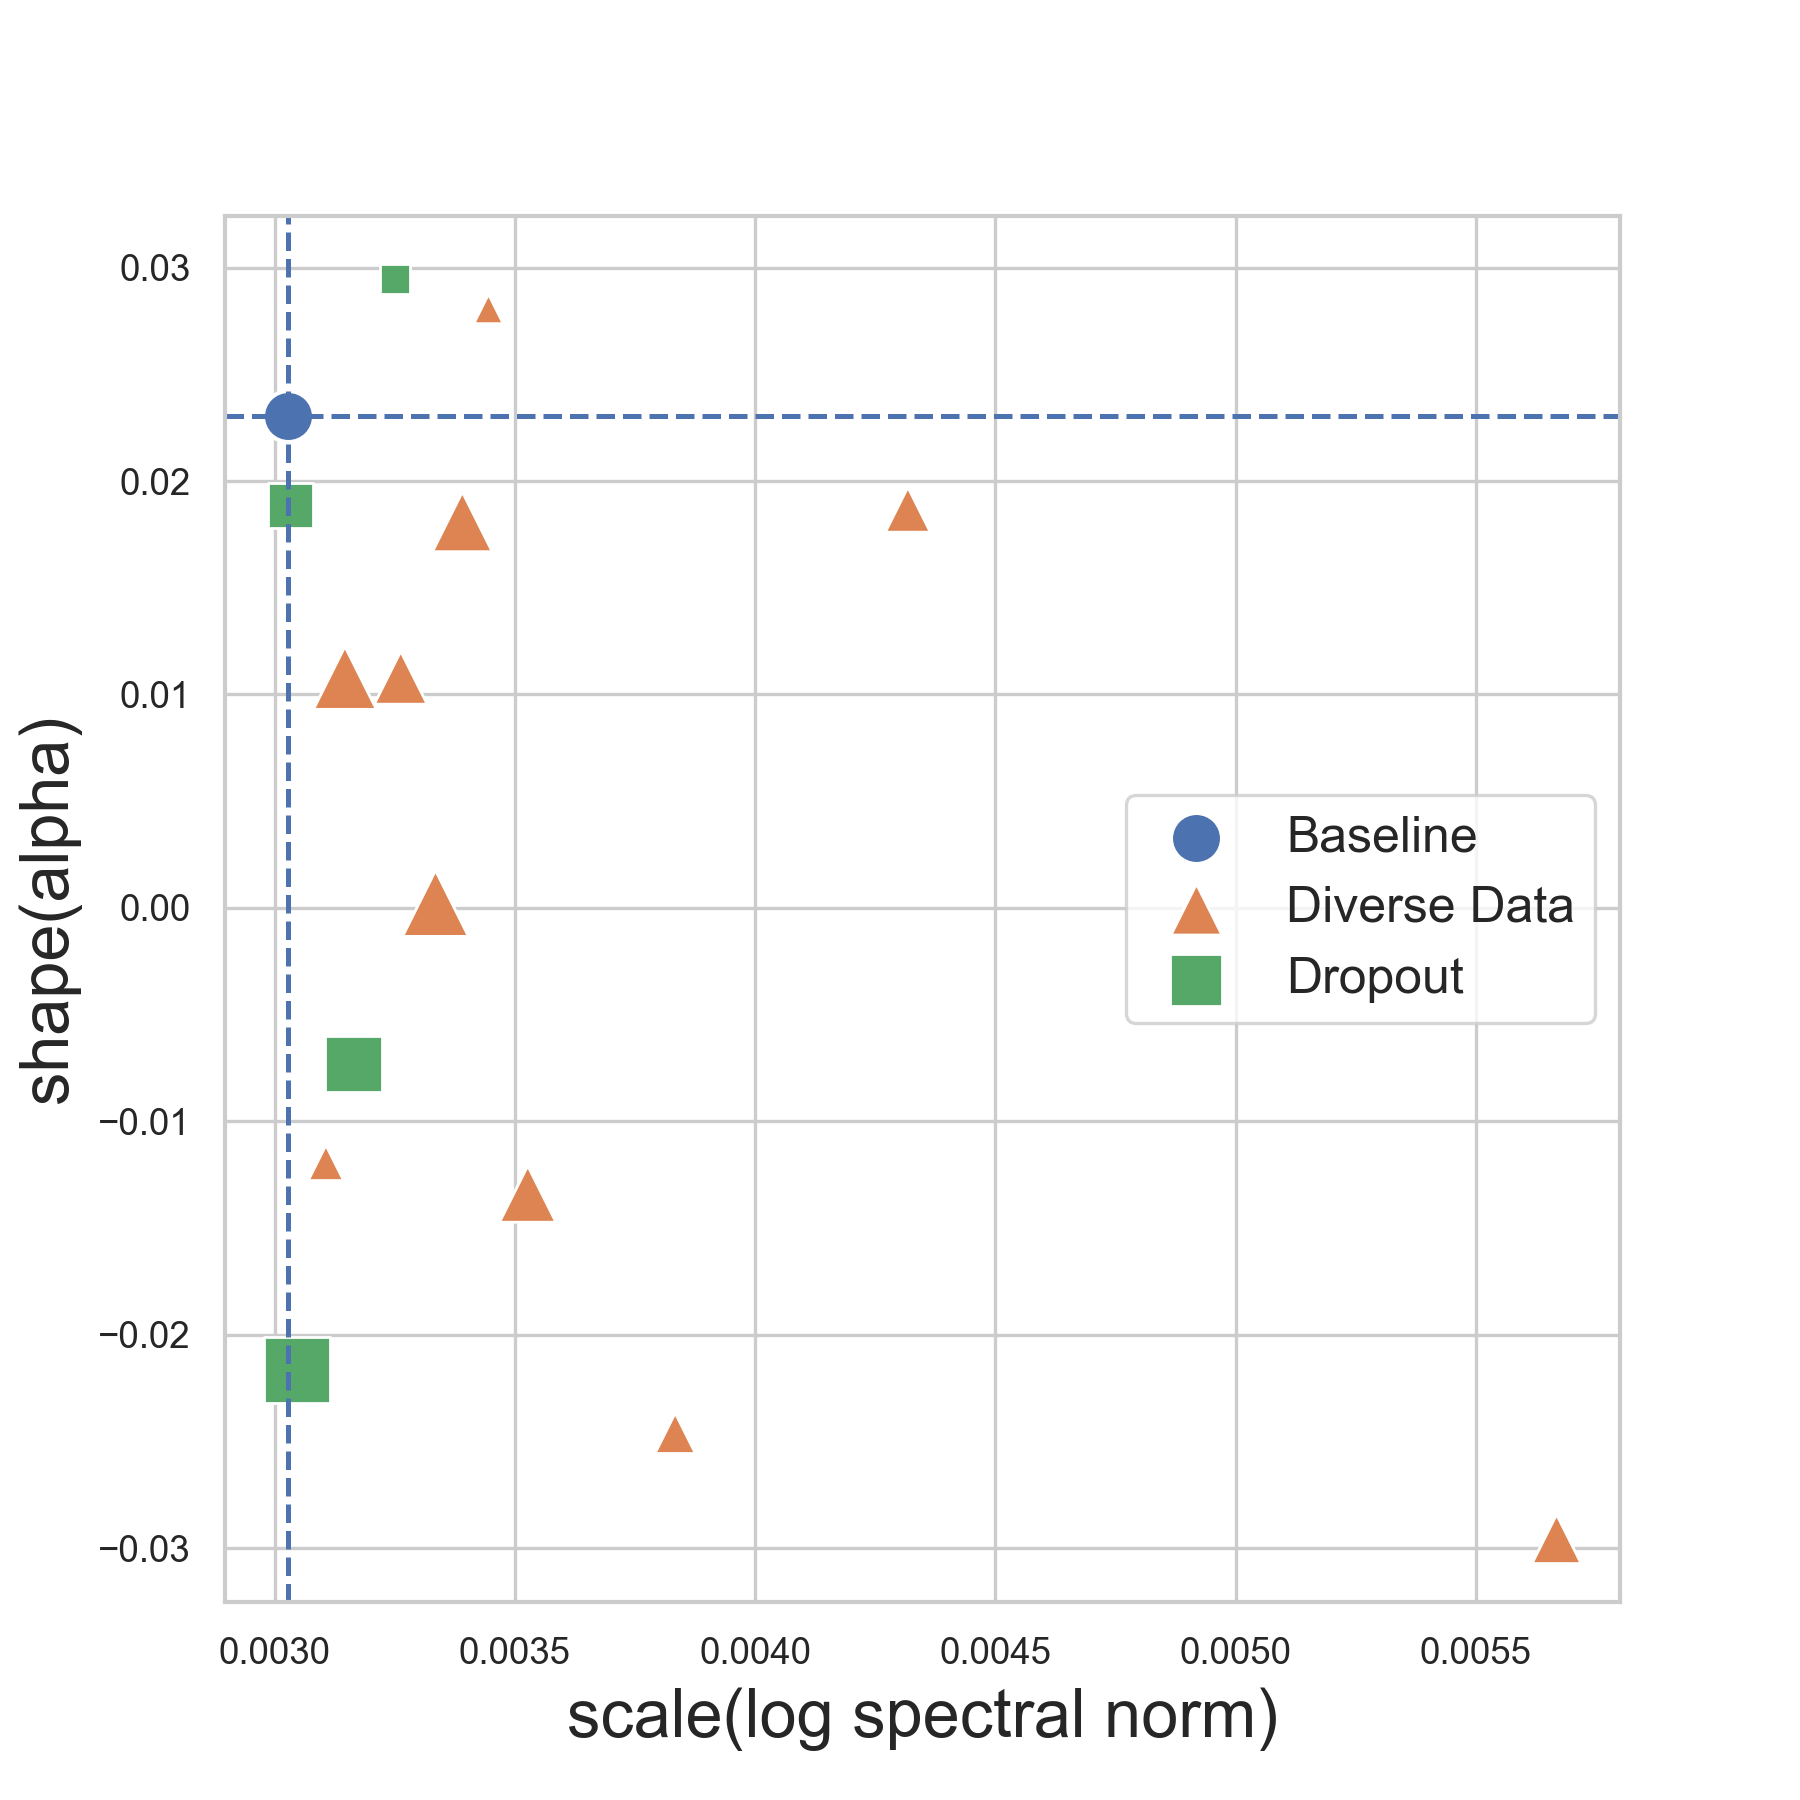}
        \caption{Spectral norm vs. alpha on CIFAR-10}
        % \label{fig:div-2}
    \end{subfigure}
    \hfill
    \begin{subfigure}[b]{0.3\textwidth}
        \centering
        \includegraphics[width=\textwidth]{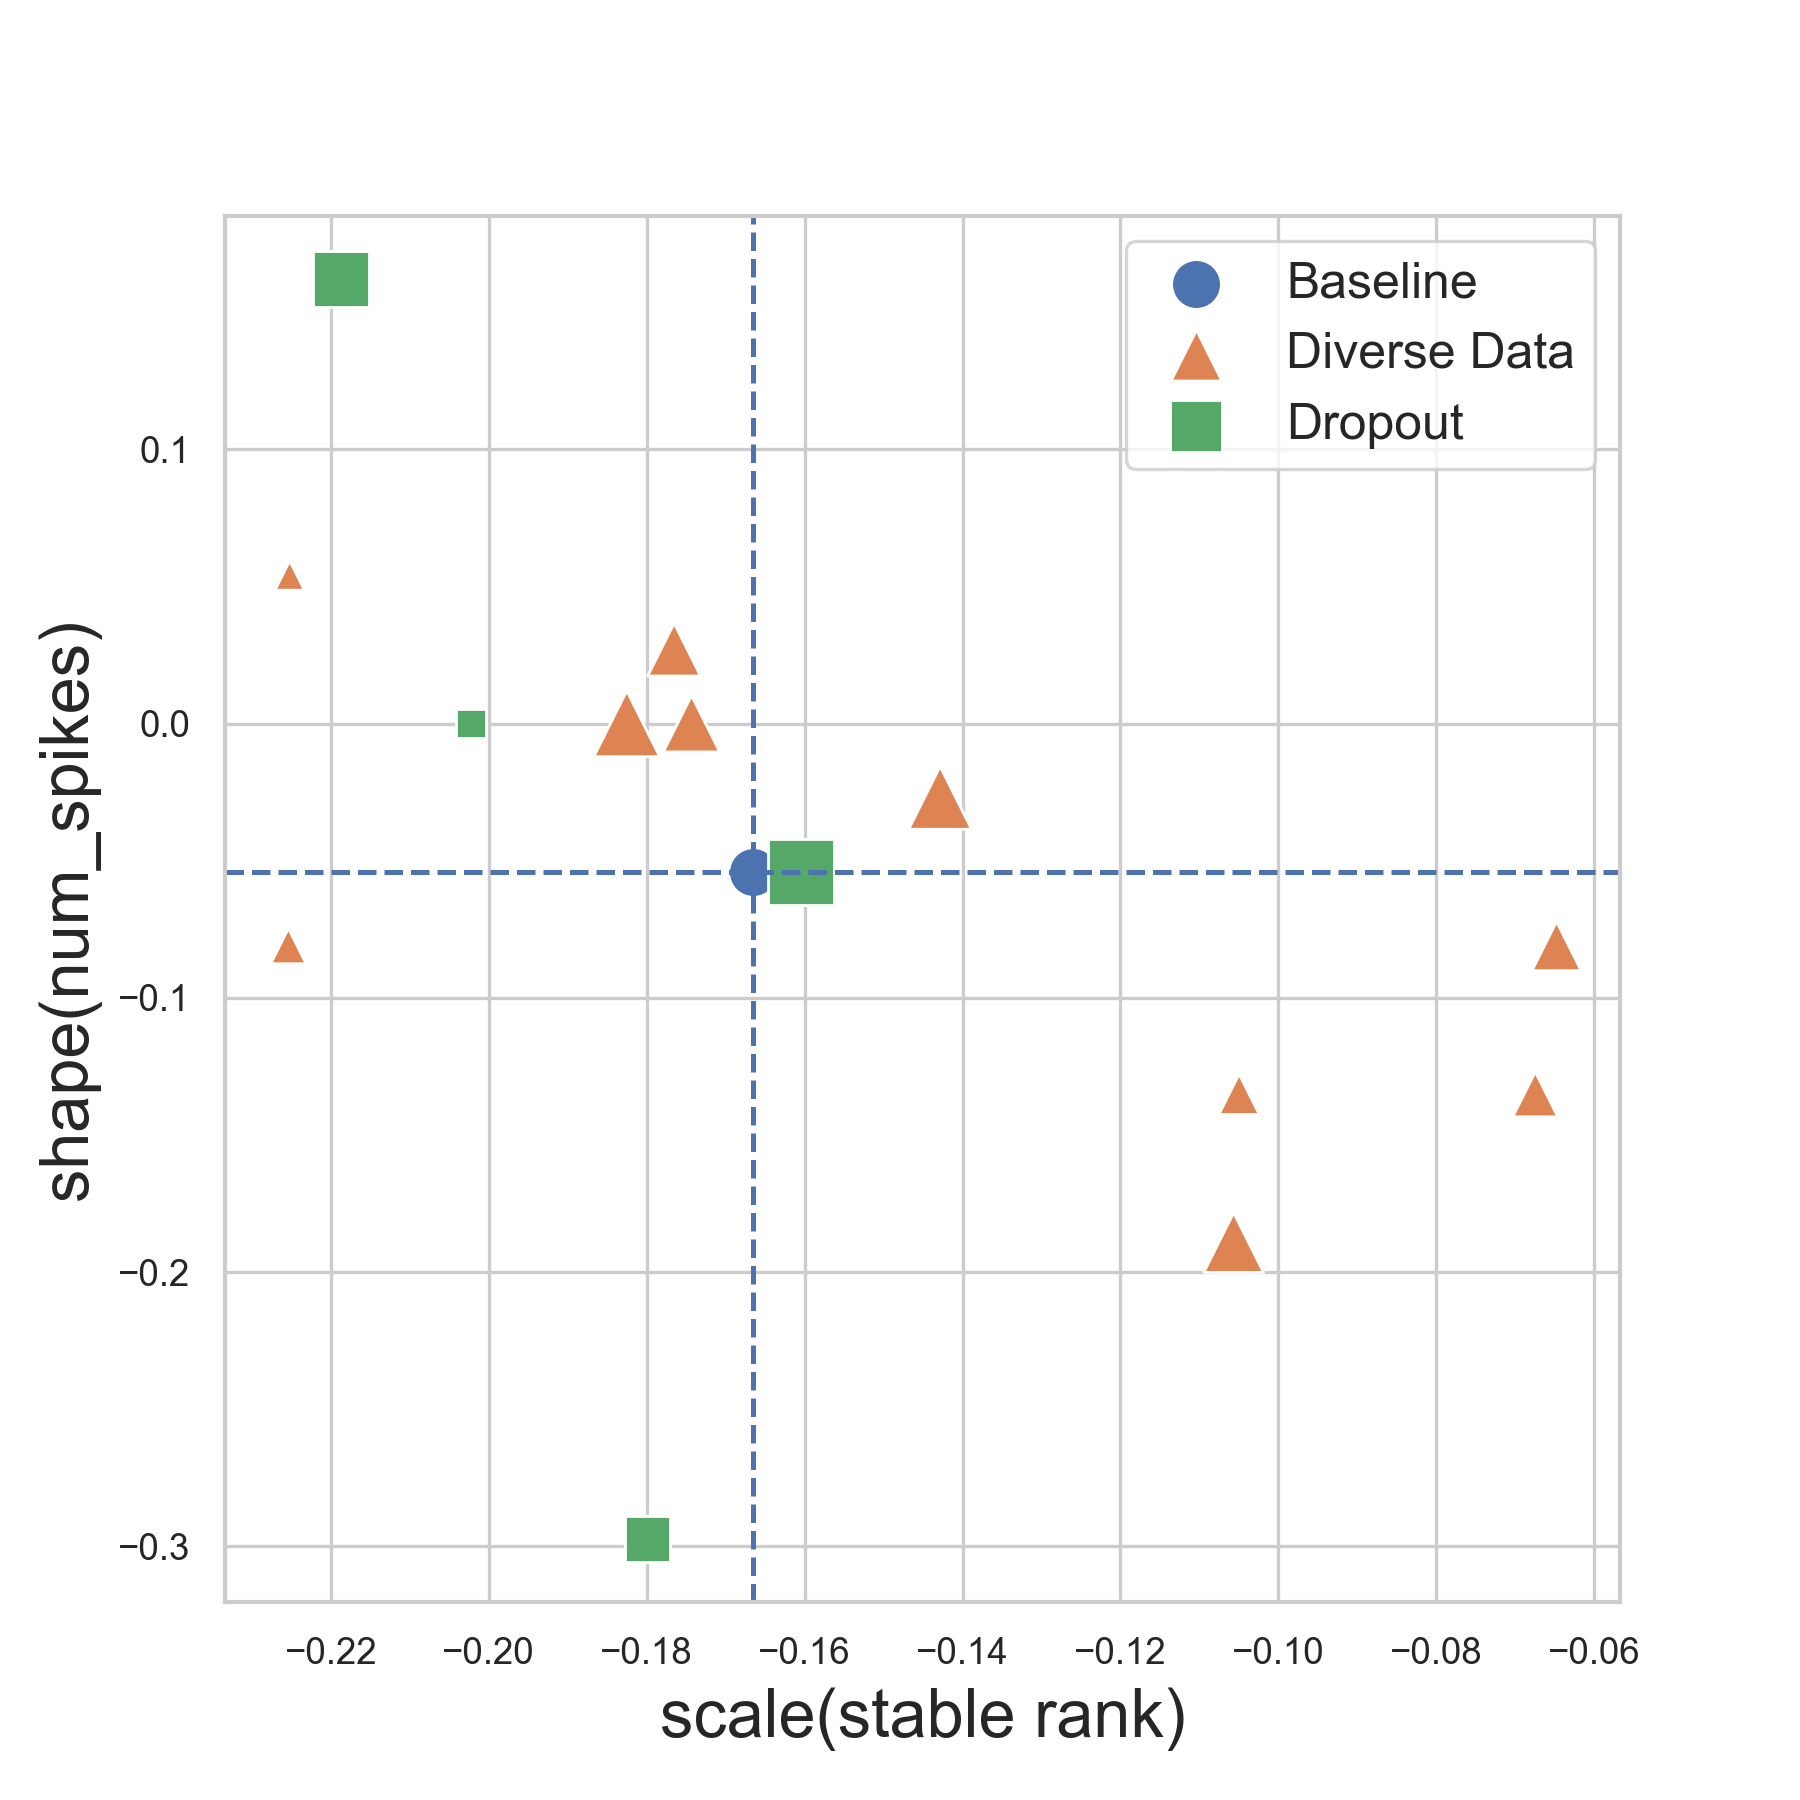}
        \caption{Stable rank vs. $\textit{num\_spikes}$ on CIFAR-10}
        % \label{fig:div-3}
    \end{subfigure}
    
    \vspace{1em} % Add some vertical space between rows
    
    % Second row
    \begin{subfigure}[b]{0.3\textwidth}
        \centering
        \includegraphics[width=\textwidth]{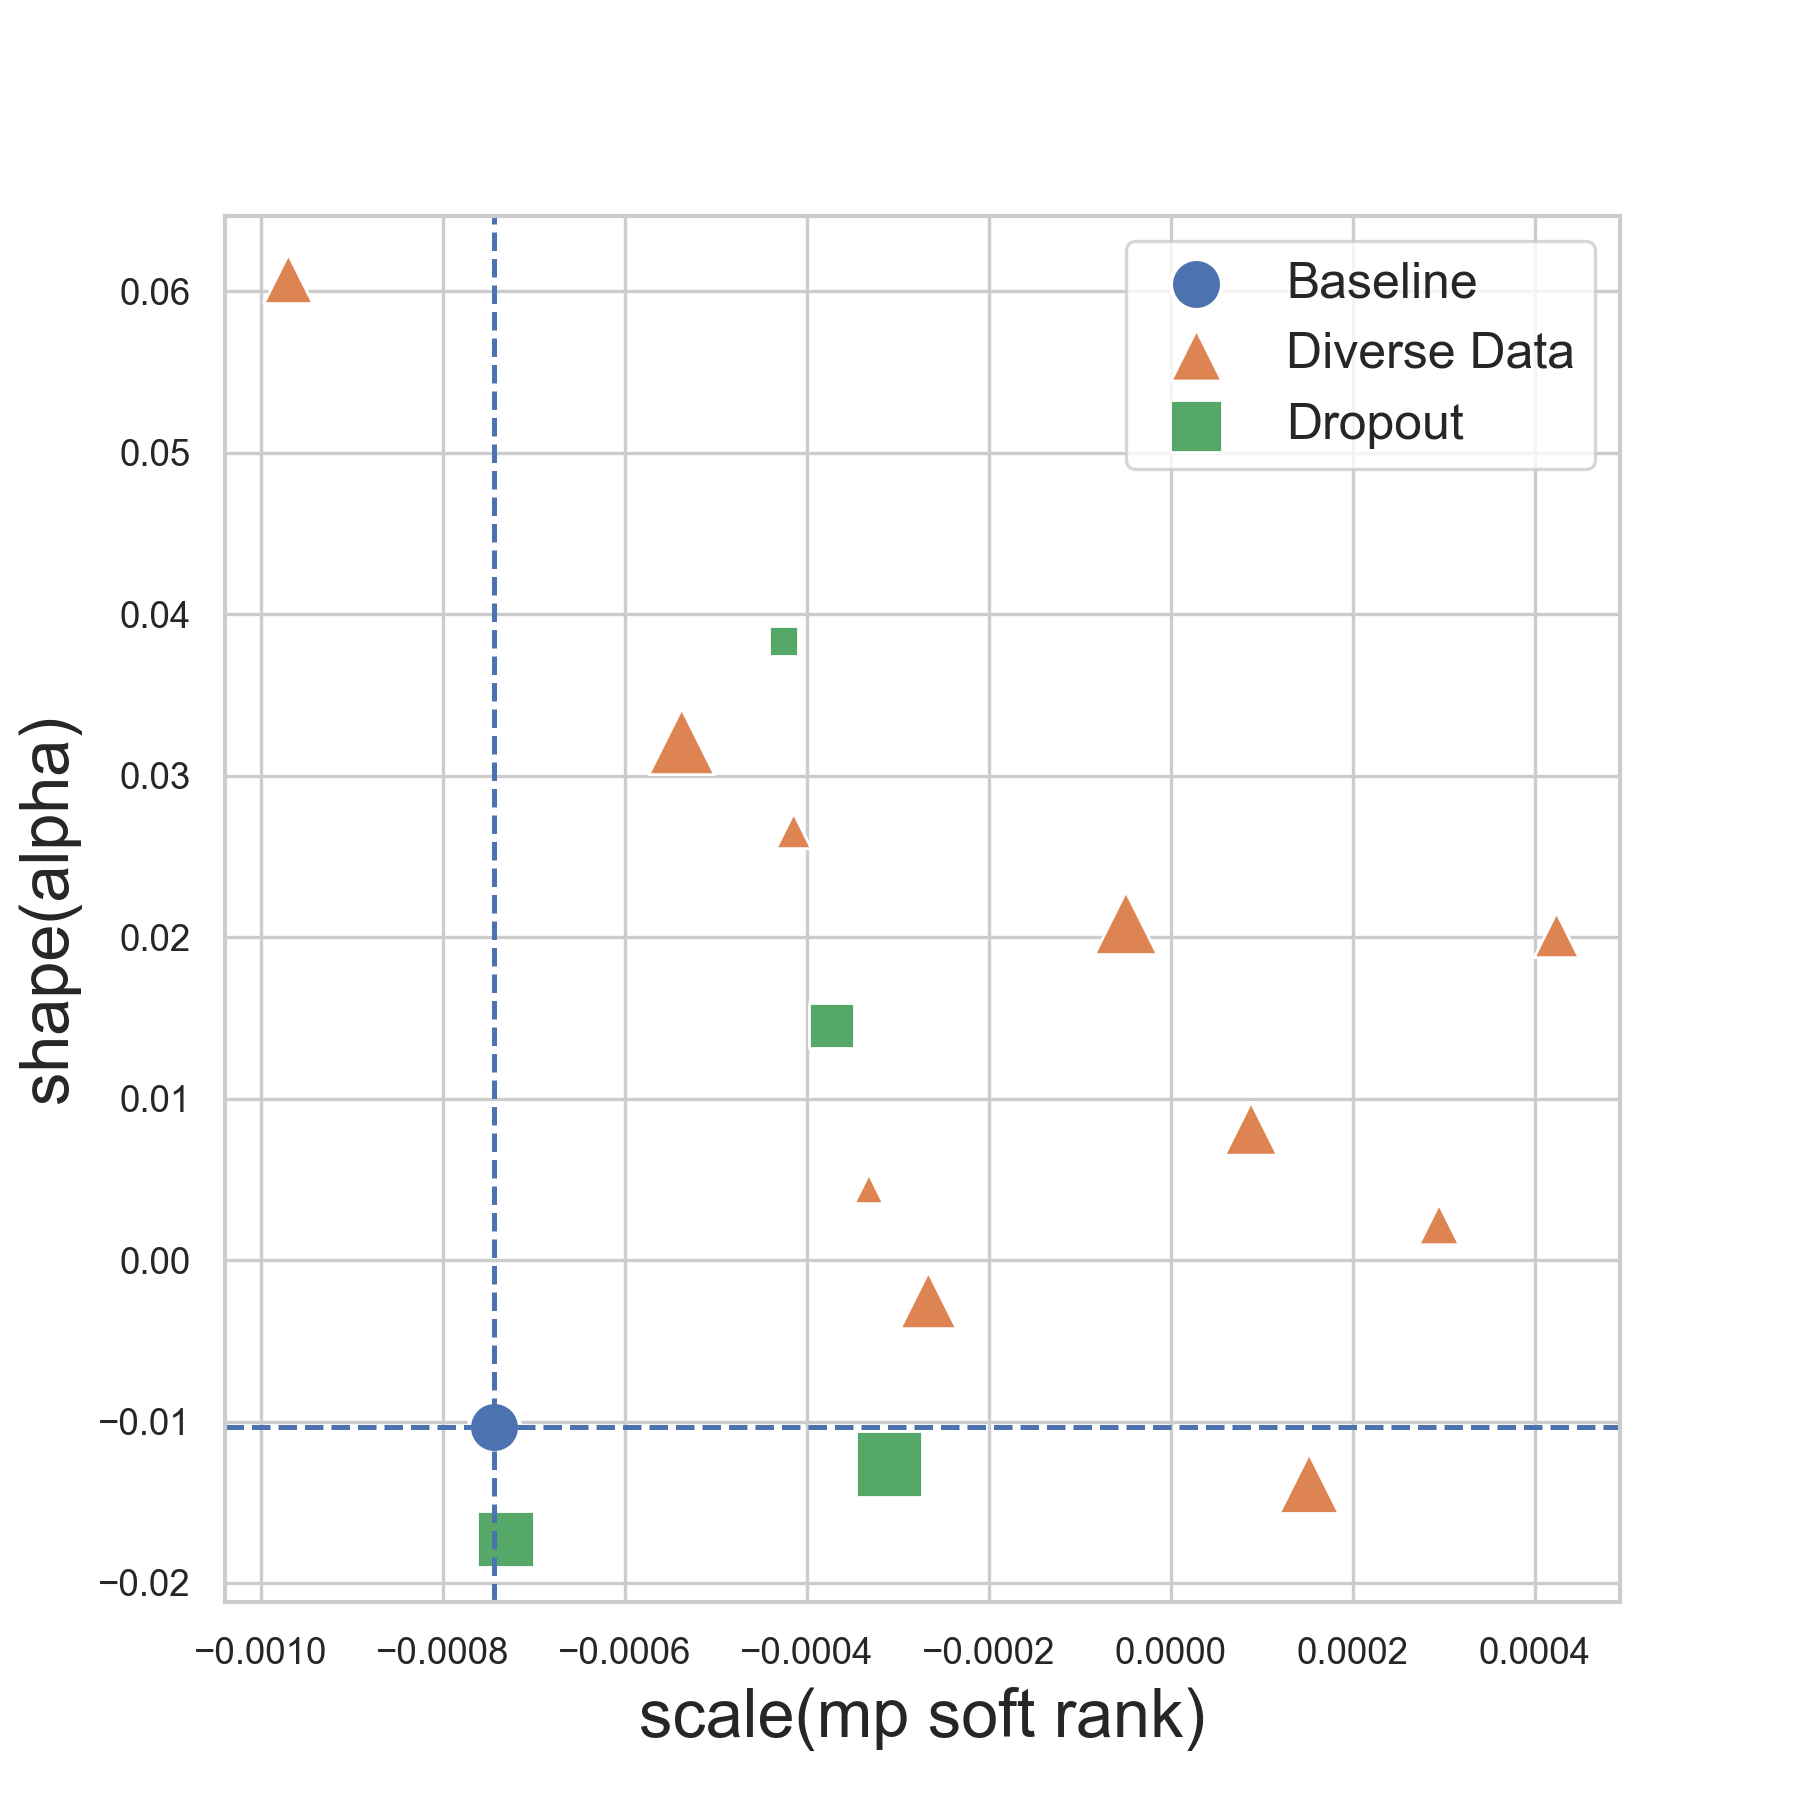}
        \caption{MP soft rank vs. alpha on CIFAR-100}
        % \label{fig:div-4}
    \end{subfigure}
    \hfill
    \begin{subfigure}[b]{0.3\textwidth}
        \centering
        \includegraphics[width=\textwidth]{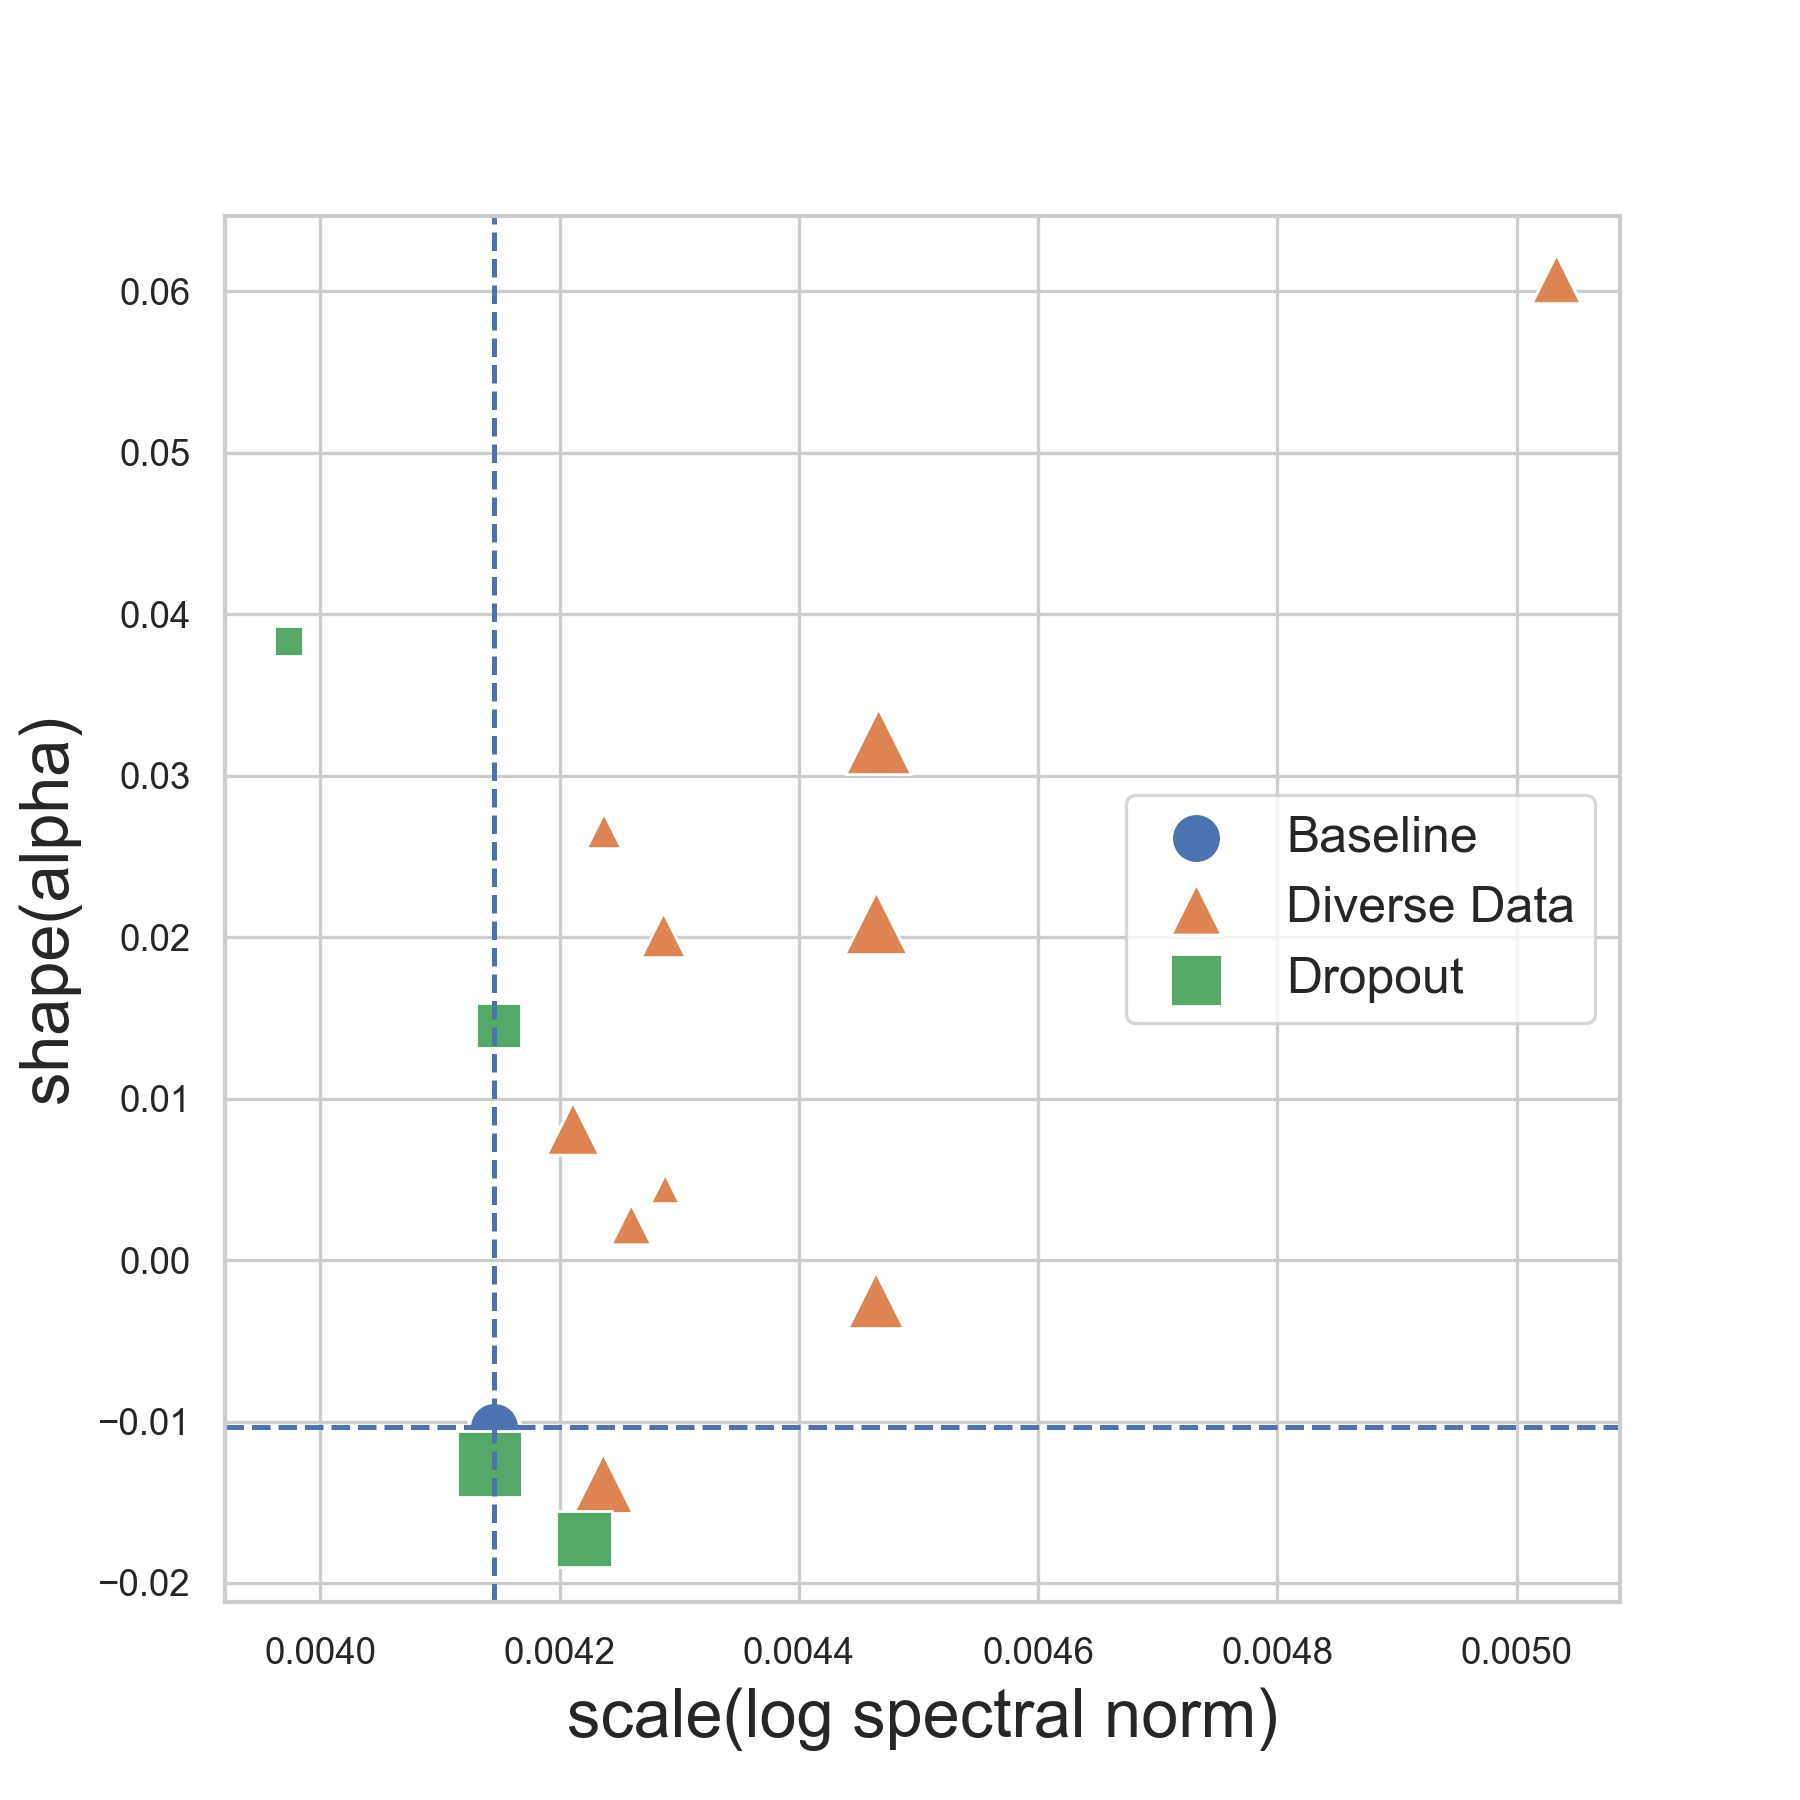}
        \caption{Spectral norm vs. alpha on CIFAR-100}
        % \label{fig:div-5}
    \end{subfigure}
    \hfill
    \begin{subfigure}[b]{0.3\textwidth}
        \centering
        \includegraphics[width=\textwidth]{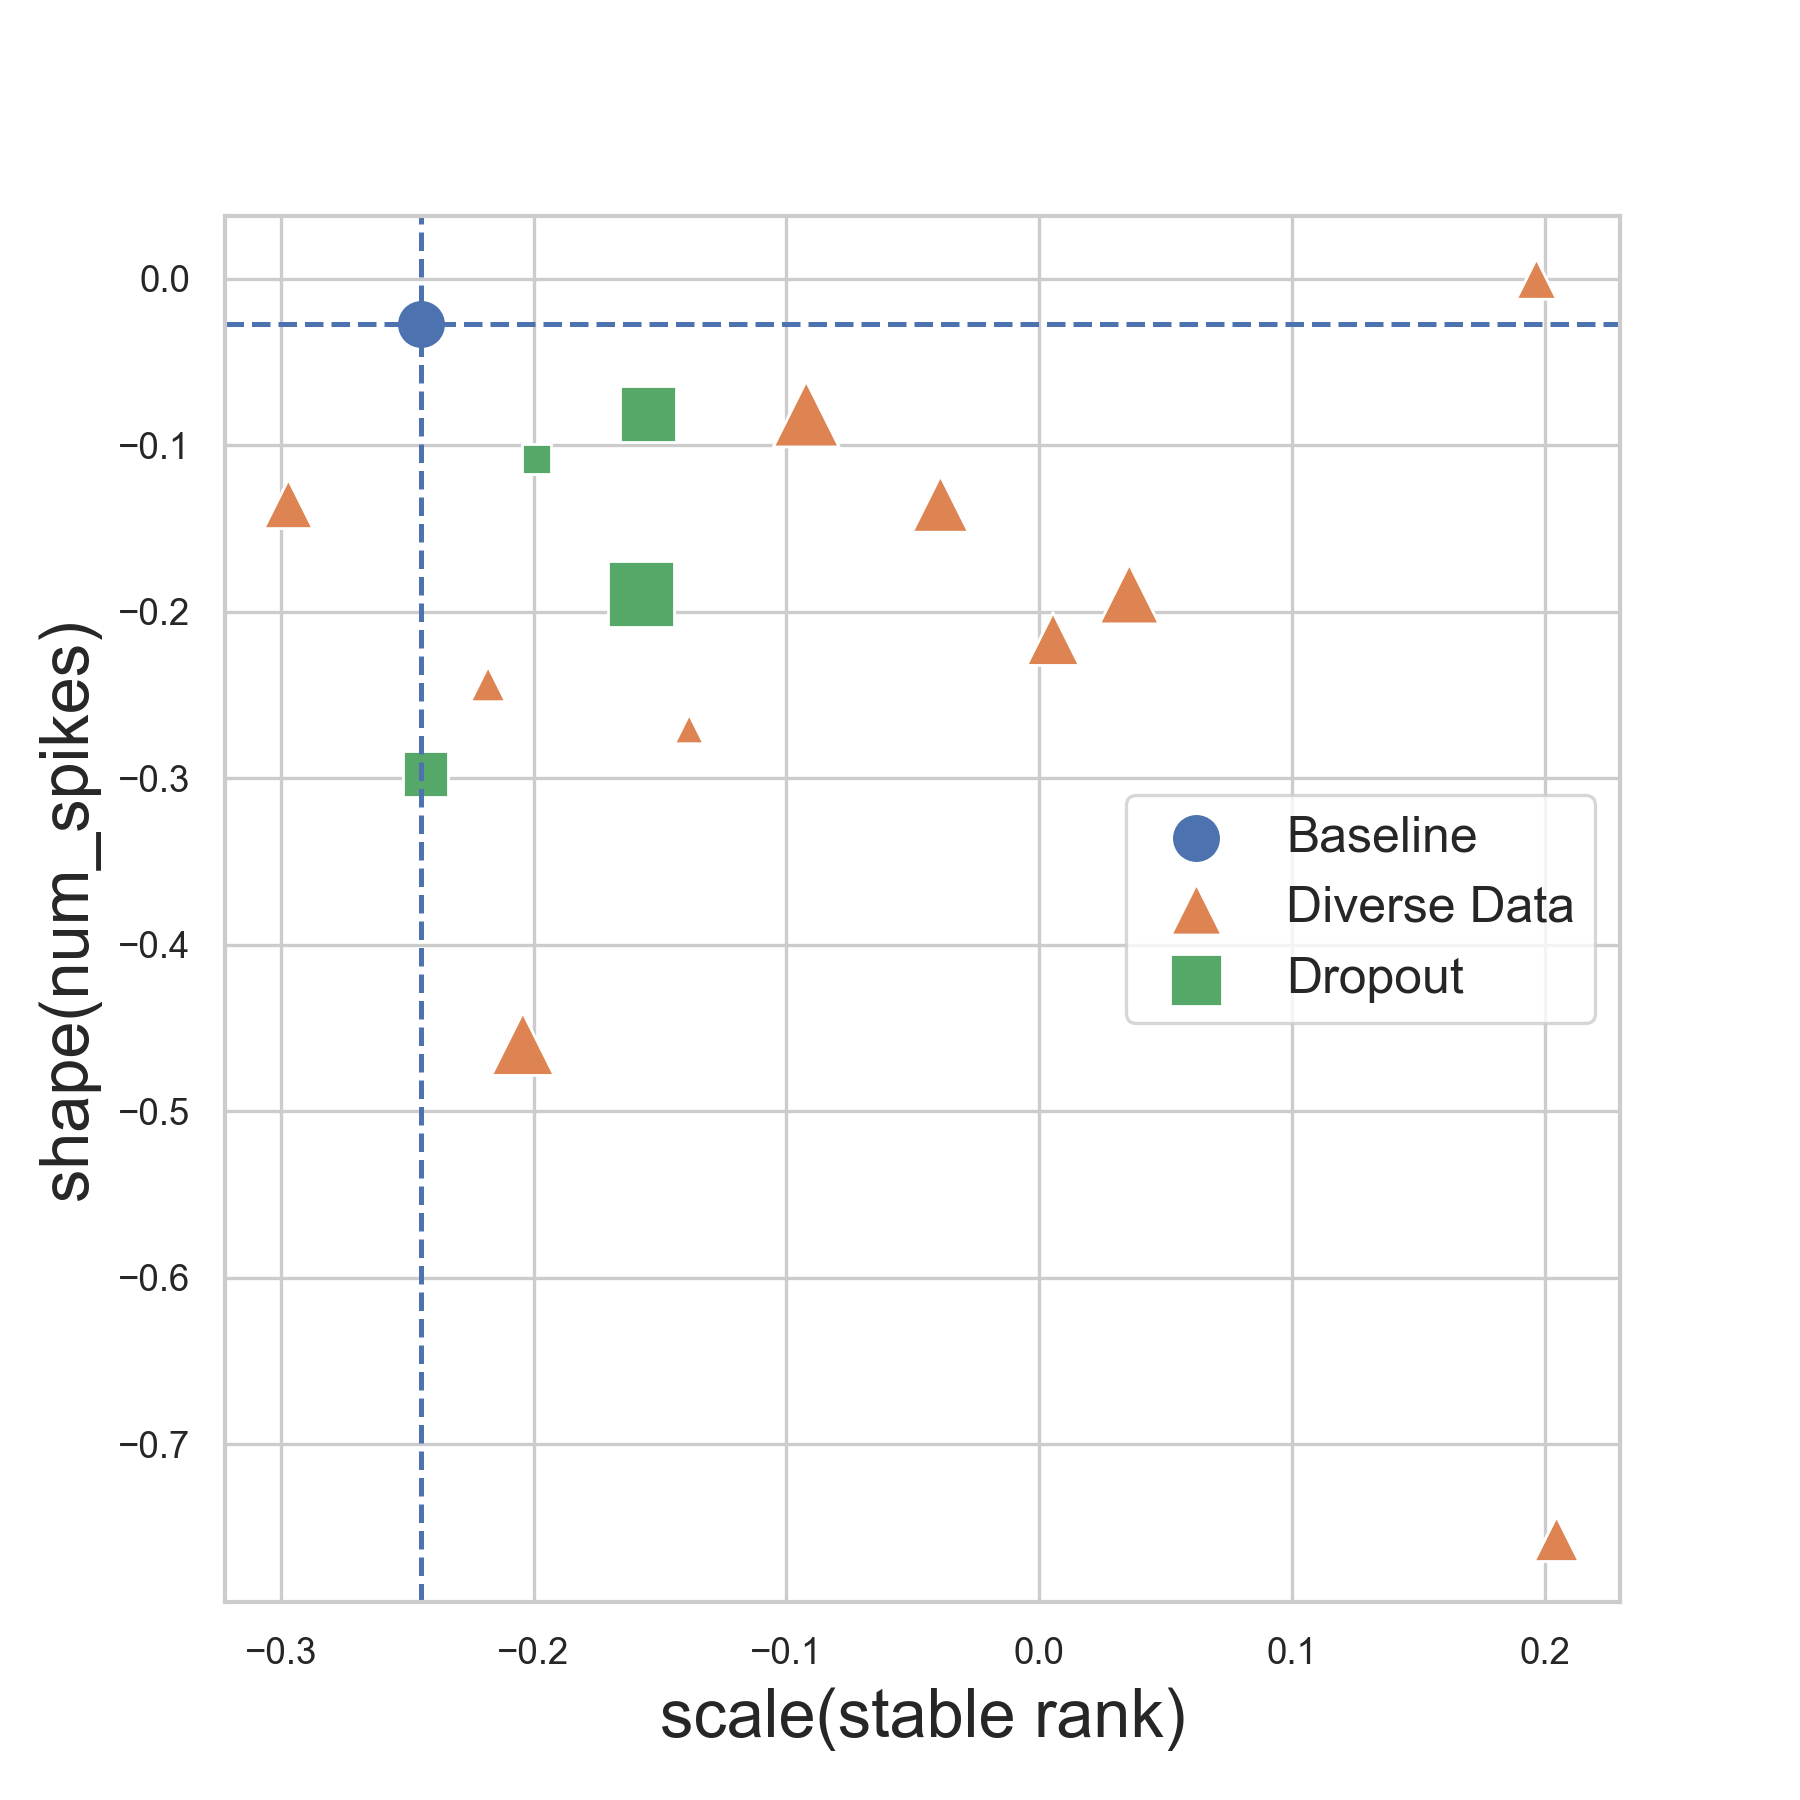}
        \caption{Stable rank vs. $\textit{num\_spikes}$ on CIFAR-100}
        % \label{fig:div-6}
    \end{subfigure}
    
    \caption{Various scale-shape plots of ESDs of all vision layers on CIFAR-10 and CIFAR-100. \textbf{We calculated the average changes through all layers in the vision encoder.The results are marked with triangle and square shapes for data augmentation and dropout, respectively. The size of markers represents the magnitude of the dropout rate and embedding-based Vendi score. In addition to the classification layer, the average changes of all vision encoder layers in CLIP exhibit similarities between dropout and data augmentation in both shape and scale. Even though the way they shape the distribution of eigenvalues is similar,  diverse data changes of scale side to a larger value than dropout. Also, their changes compared with the baseline have a similar trend.}}
    \label{fig:vision}
\end{figure}

\begin{figure}[h]
    \centering
    % First row
    \begin{subfigure}[b]{0.3\textwidth}
        \centering
        \includegraphics[width=\textwidth]{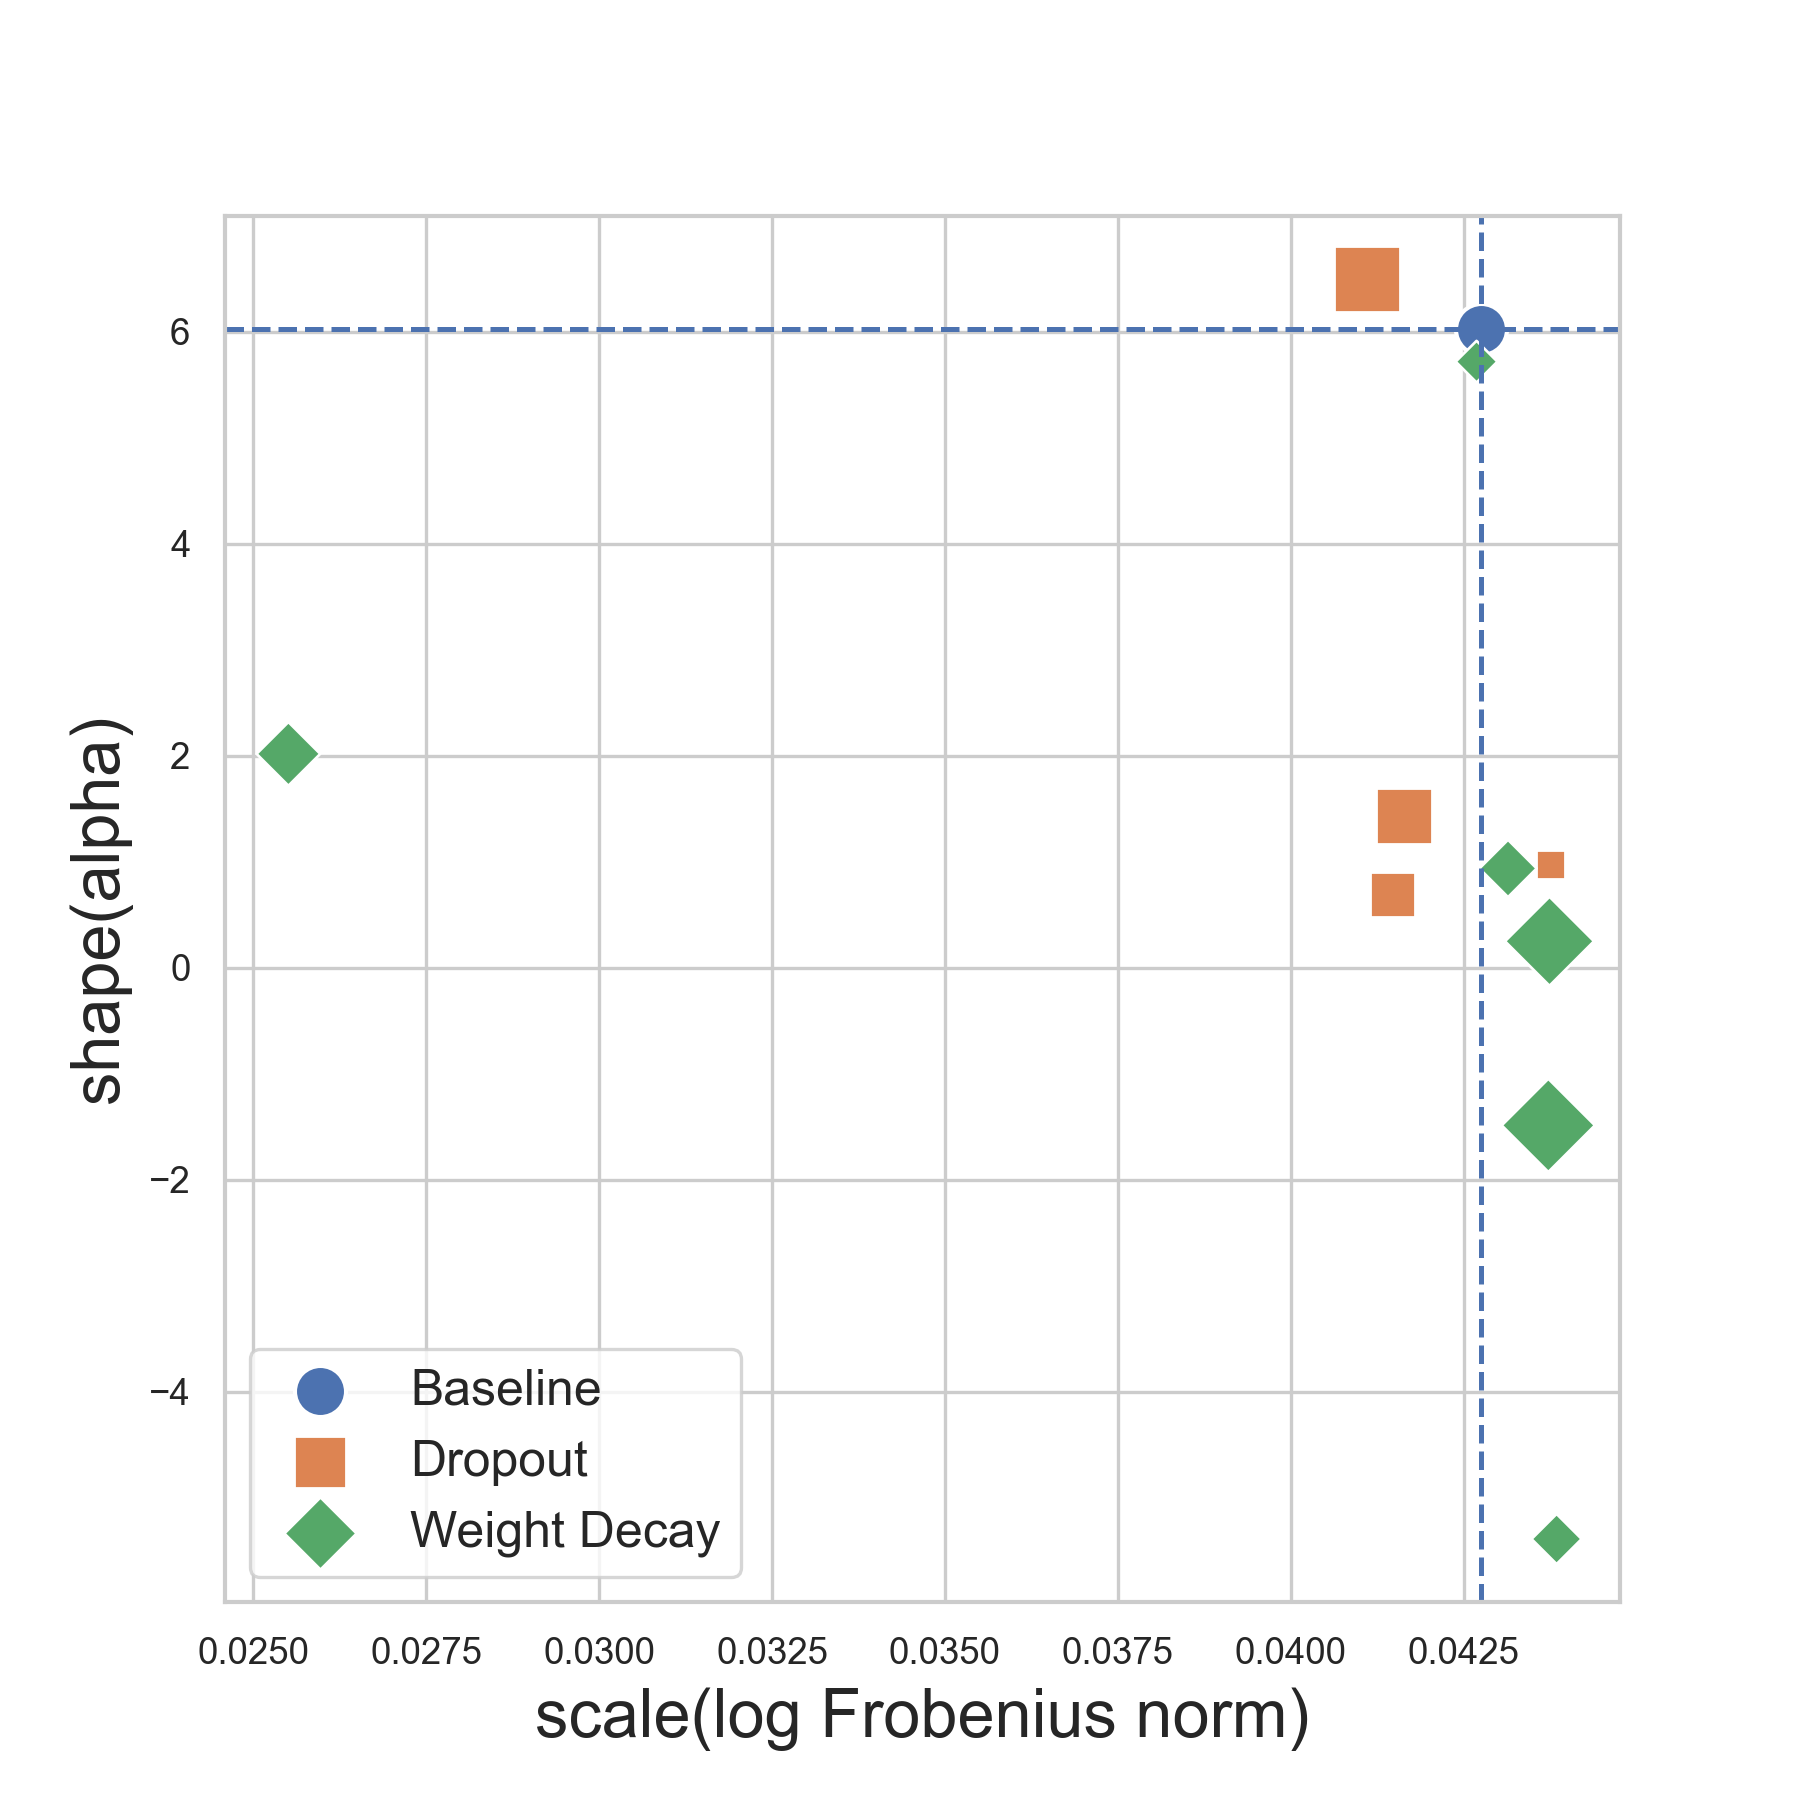}
        \caption{Frobenius norm vs. alpha on CIFAR-10}
        \label{fig:reg-1}
    \end{subfigure}
    \hfill
    \begin{subfigure}[b]{0.3\textwidth}
        \centering
        \includegraphics[width=\textwidth]{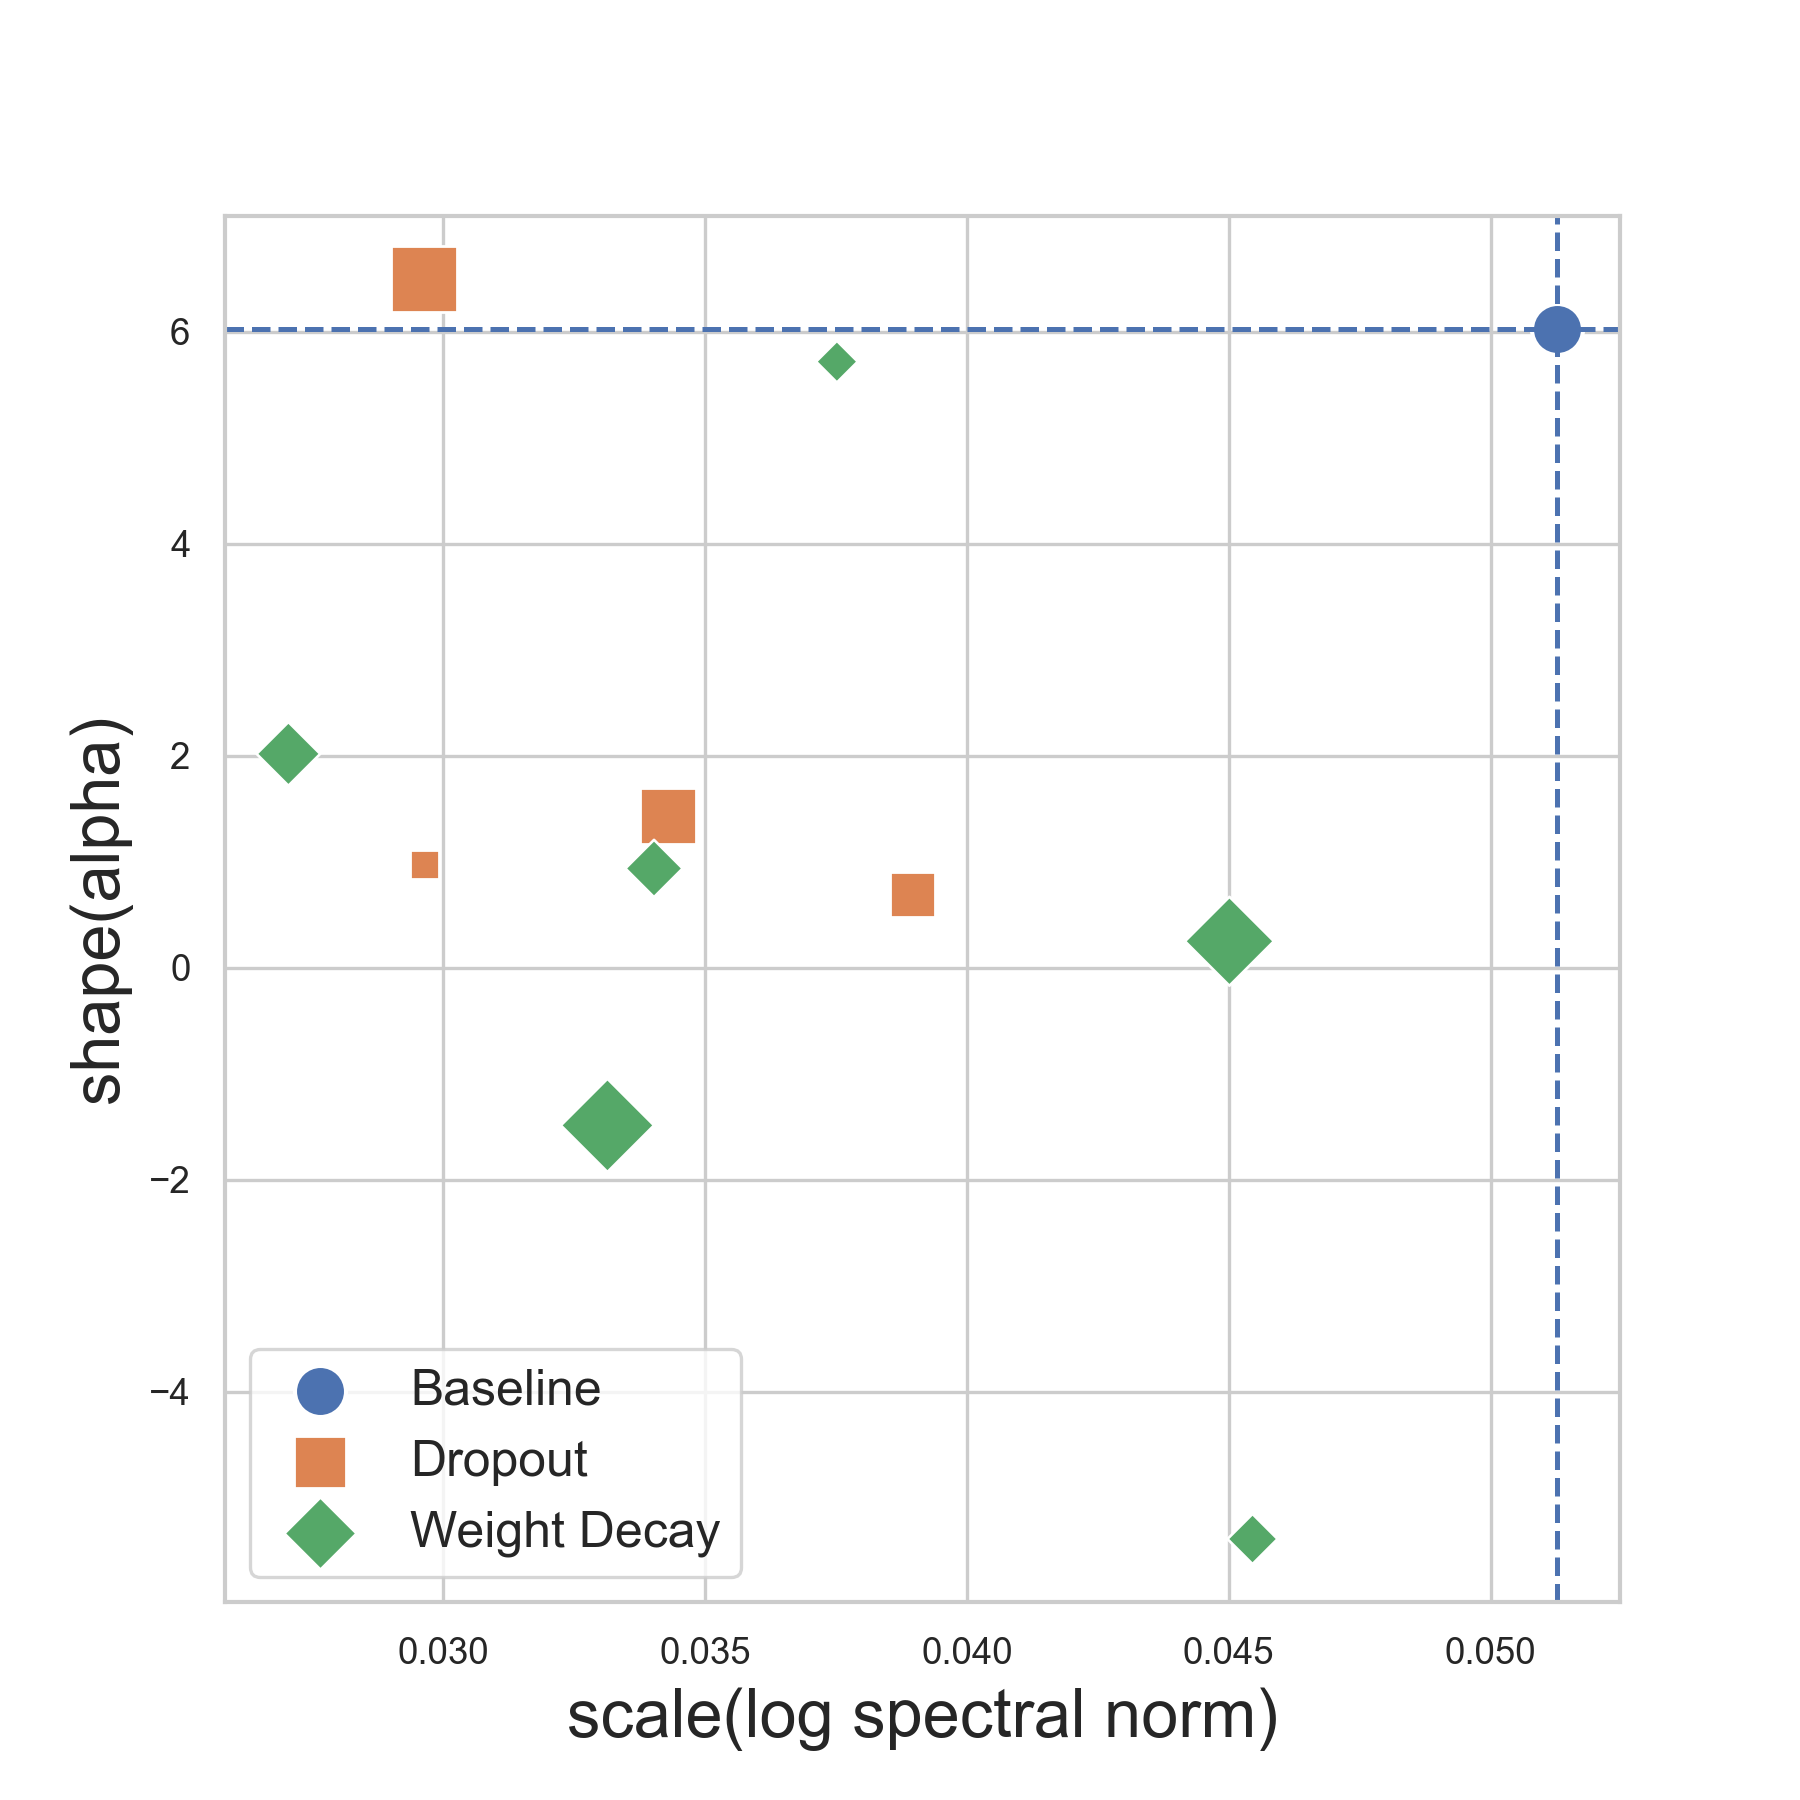}
        \caption{Spectral norm vs. alpha on CIFAR-10}
        \label{fig:reg-2}
    \end{subfigure}
    \hfill
    \begin{subfigure}[b]{0.3\textwidth}
        \centering
        \includegraphics[width=\textwidth]{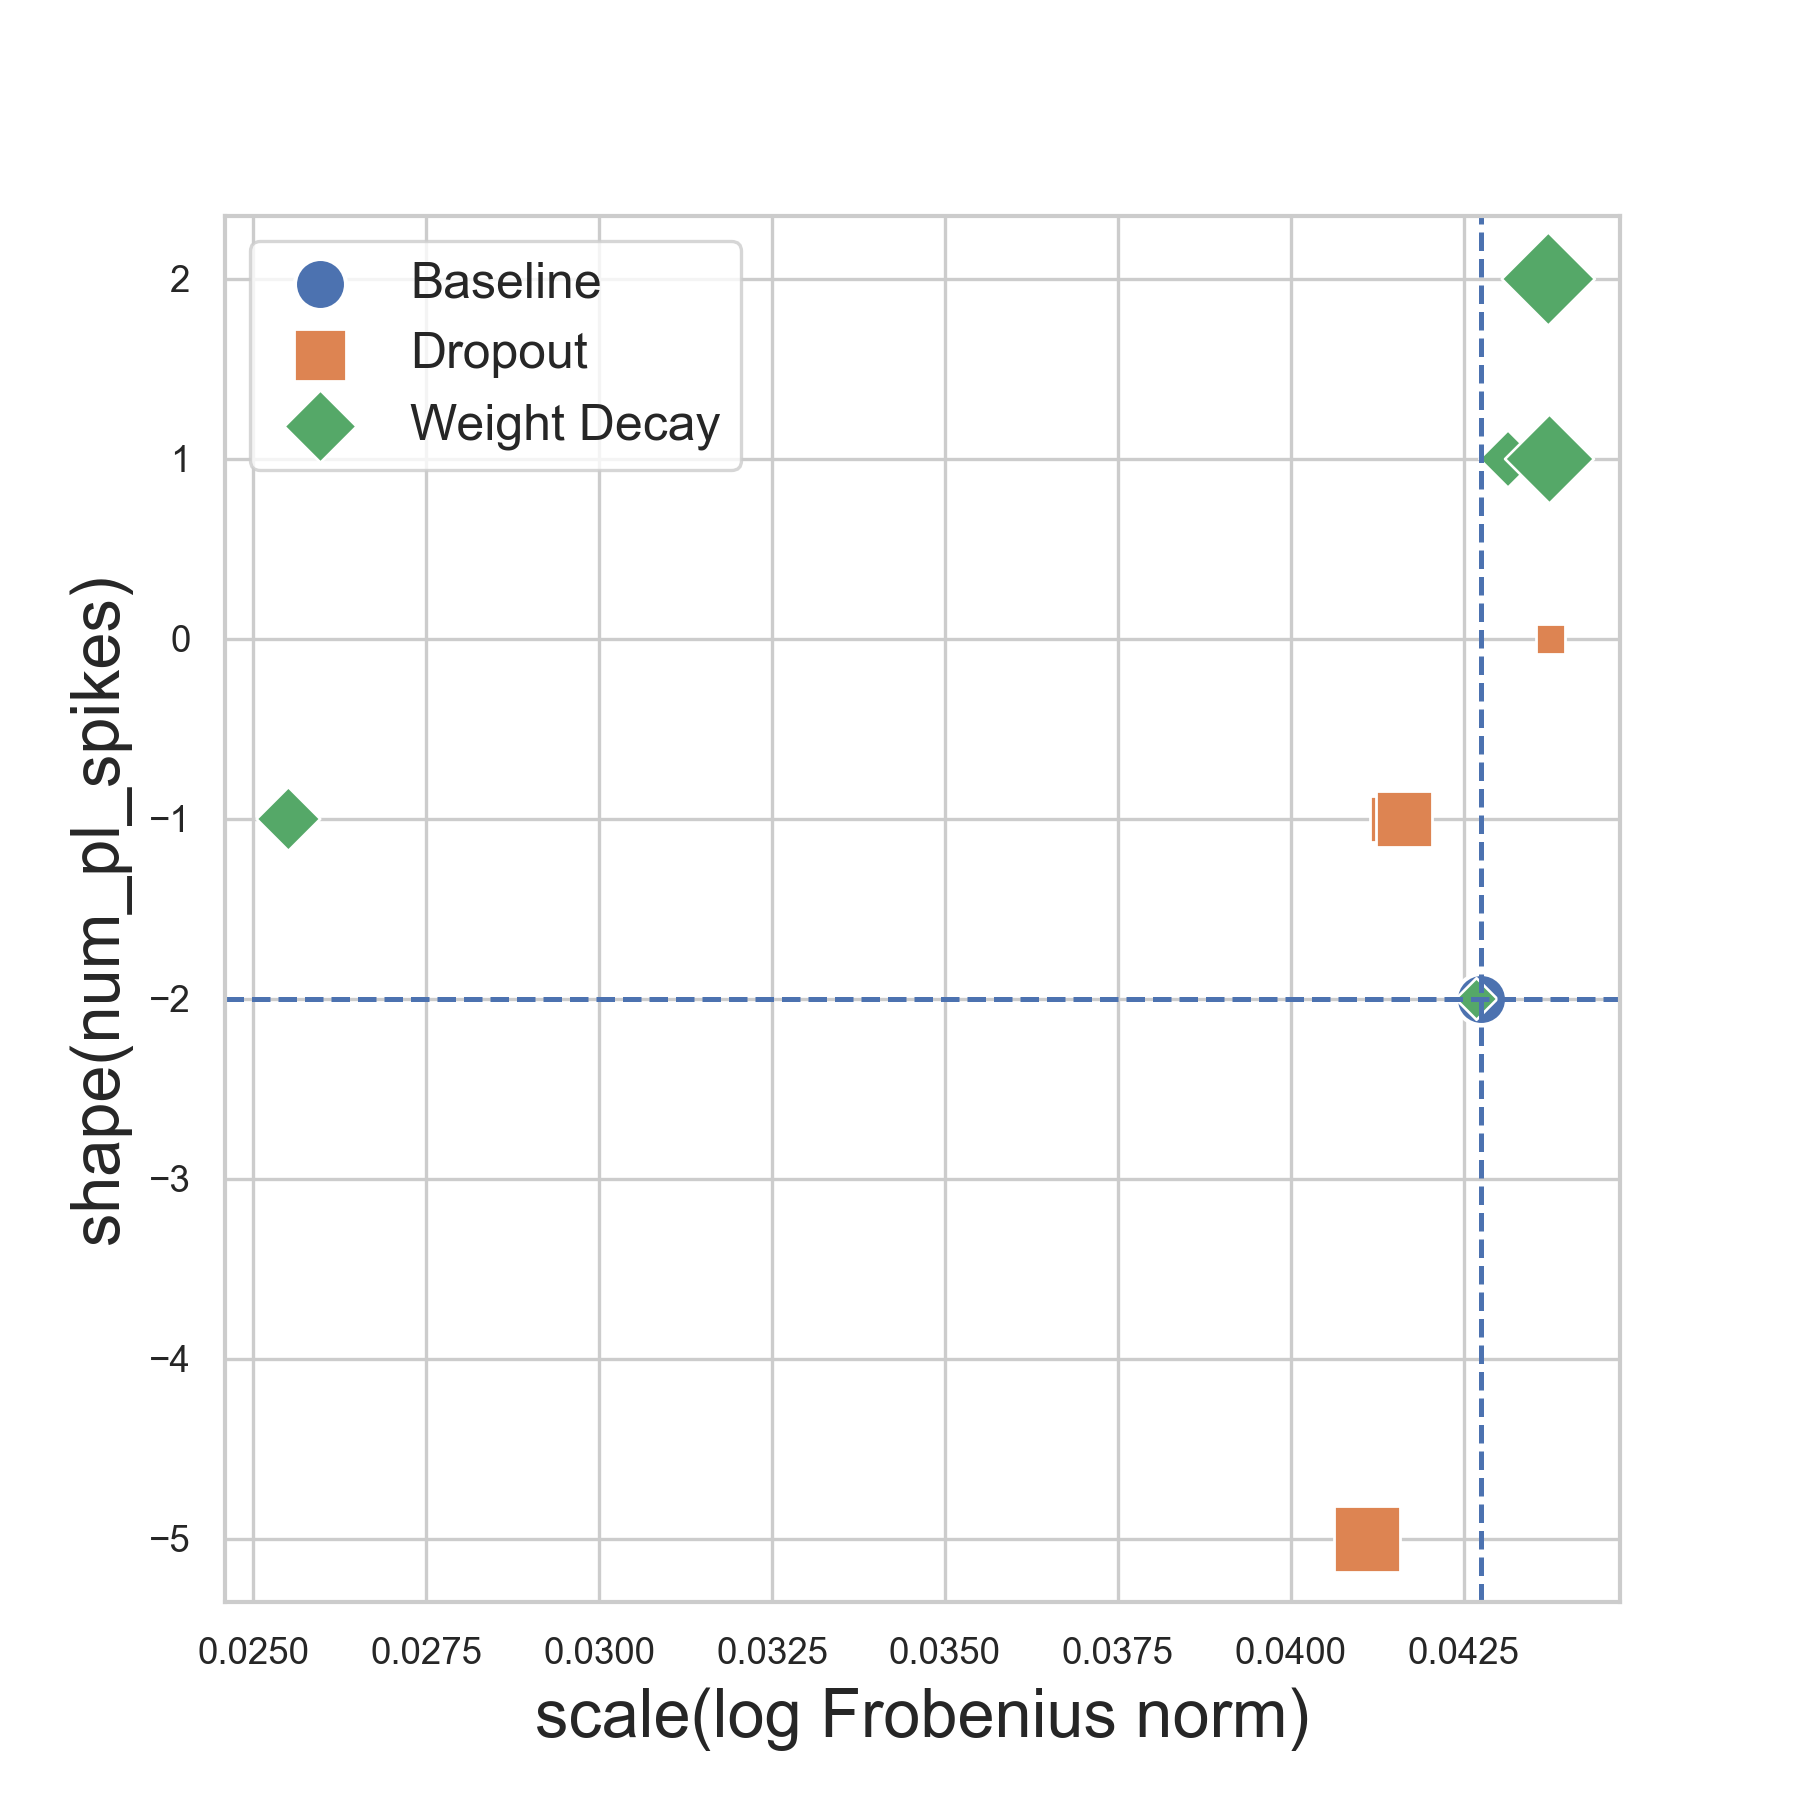}
        \caption{Frobenius vs. $\textit{num\_pl\_spikes}$ on CIFAR-10}
        \label{fig:ref-3}
    \end{subfigure}
    
    \vspace{1em} % Add some vertical space between rows
    
    % Second row
    \begin{subfigure}[b]{0.3\textwidth}
        \centering
        \includegraphics[width=\textwidth]{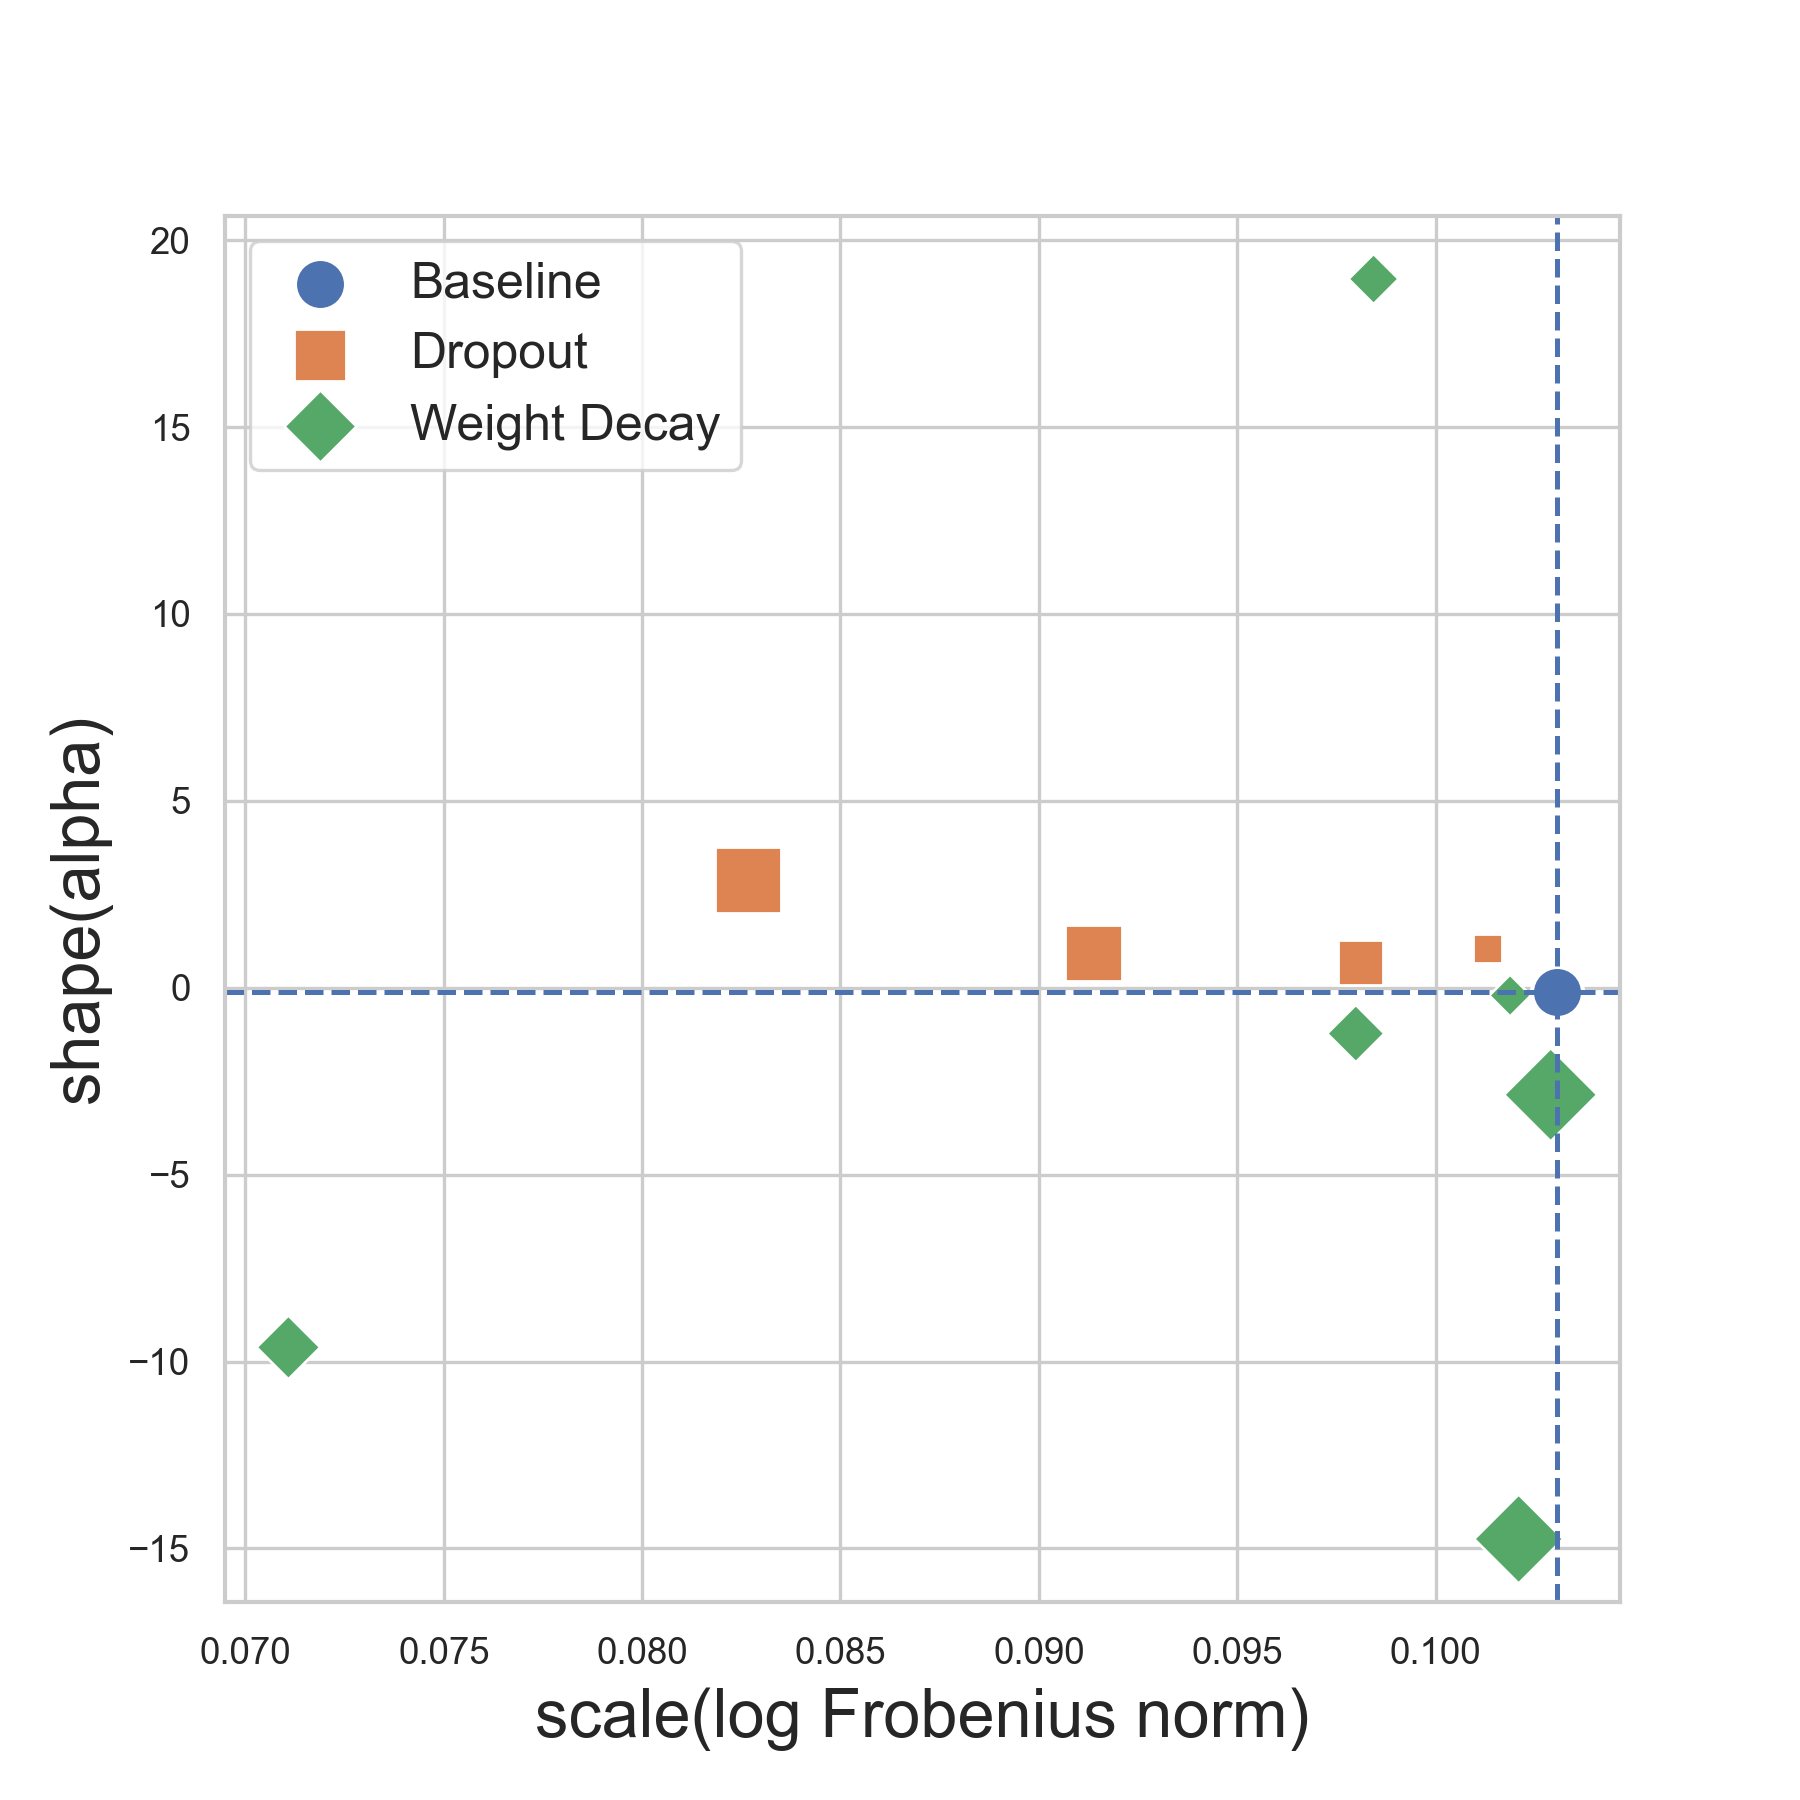}
        \caption{Frobenius norm vs. alpha on CIFAR-100}
        \label{fig:reg-4}
    \end{subfigure}
    \hfill
    \begin{subfigure}[b]{0.3\textwidth}
        \centering
        \includegraphics[width=\textwidth]{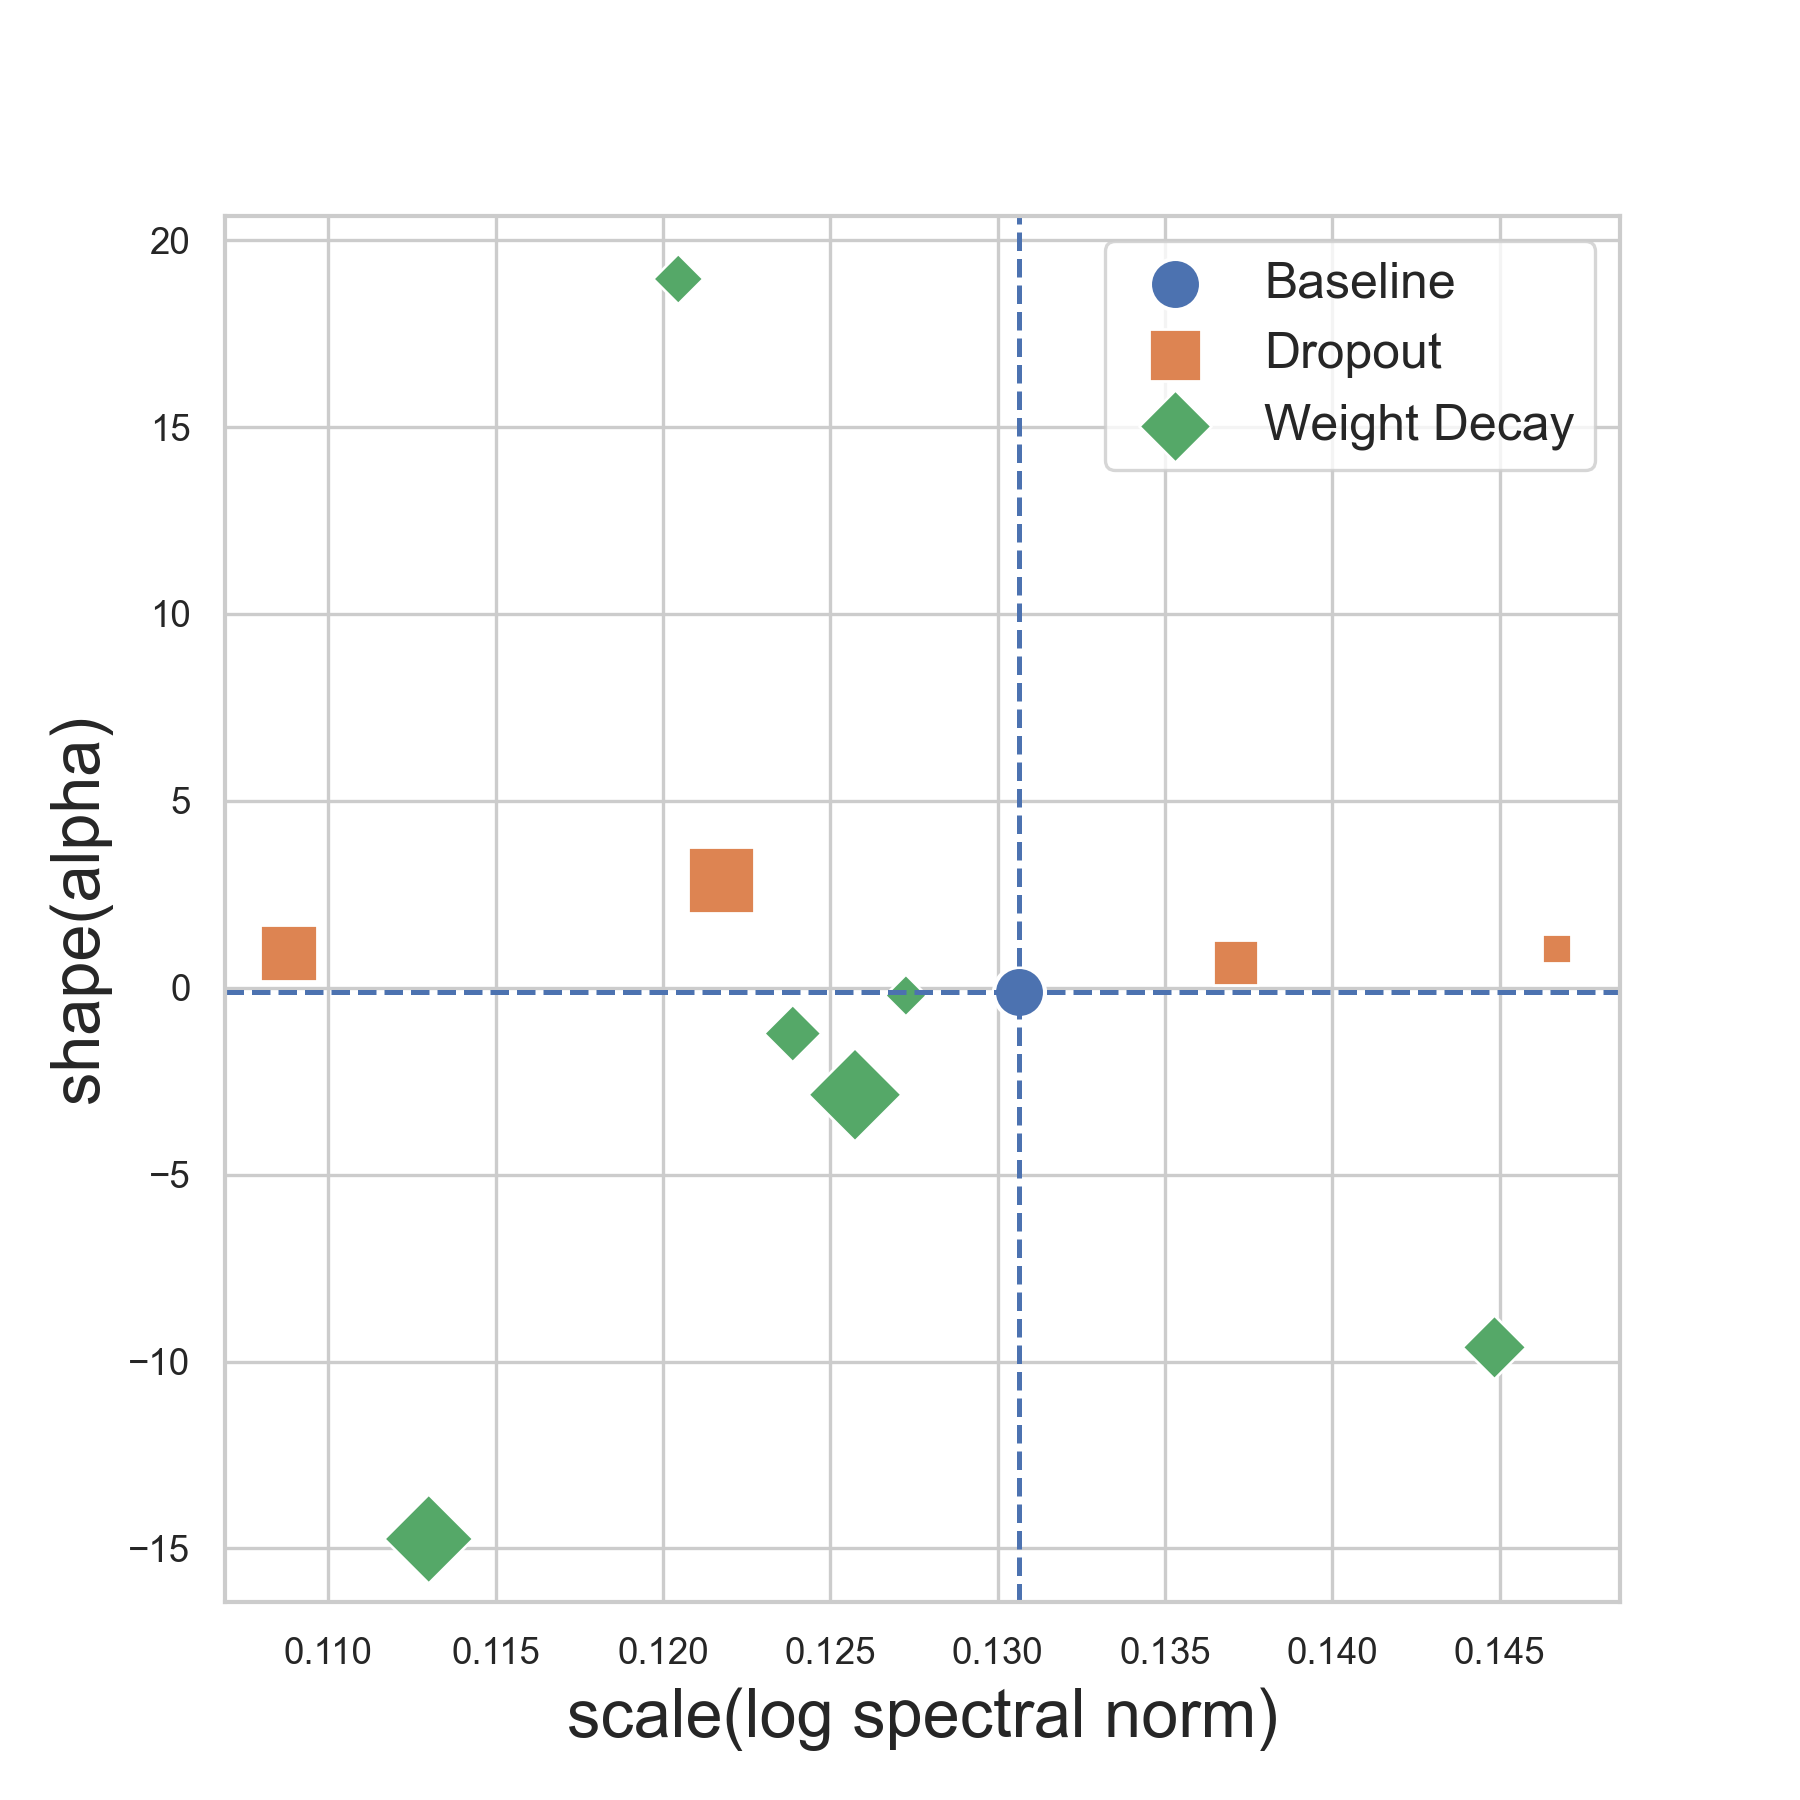}
        \caption{Spectral norm vs. alpha on CIFAR-100}
        \label{fig:reg-5}
    \end{subfigure}
    \hfill
    \begin{subfigure}[b]{0.3\textwidth}
        \centering
        \includegraphics[width=\textwidth]{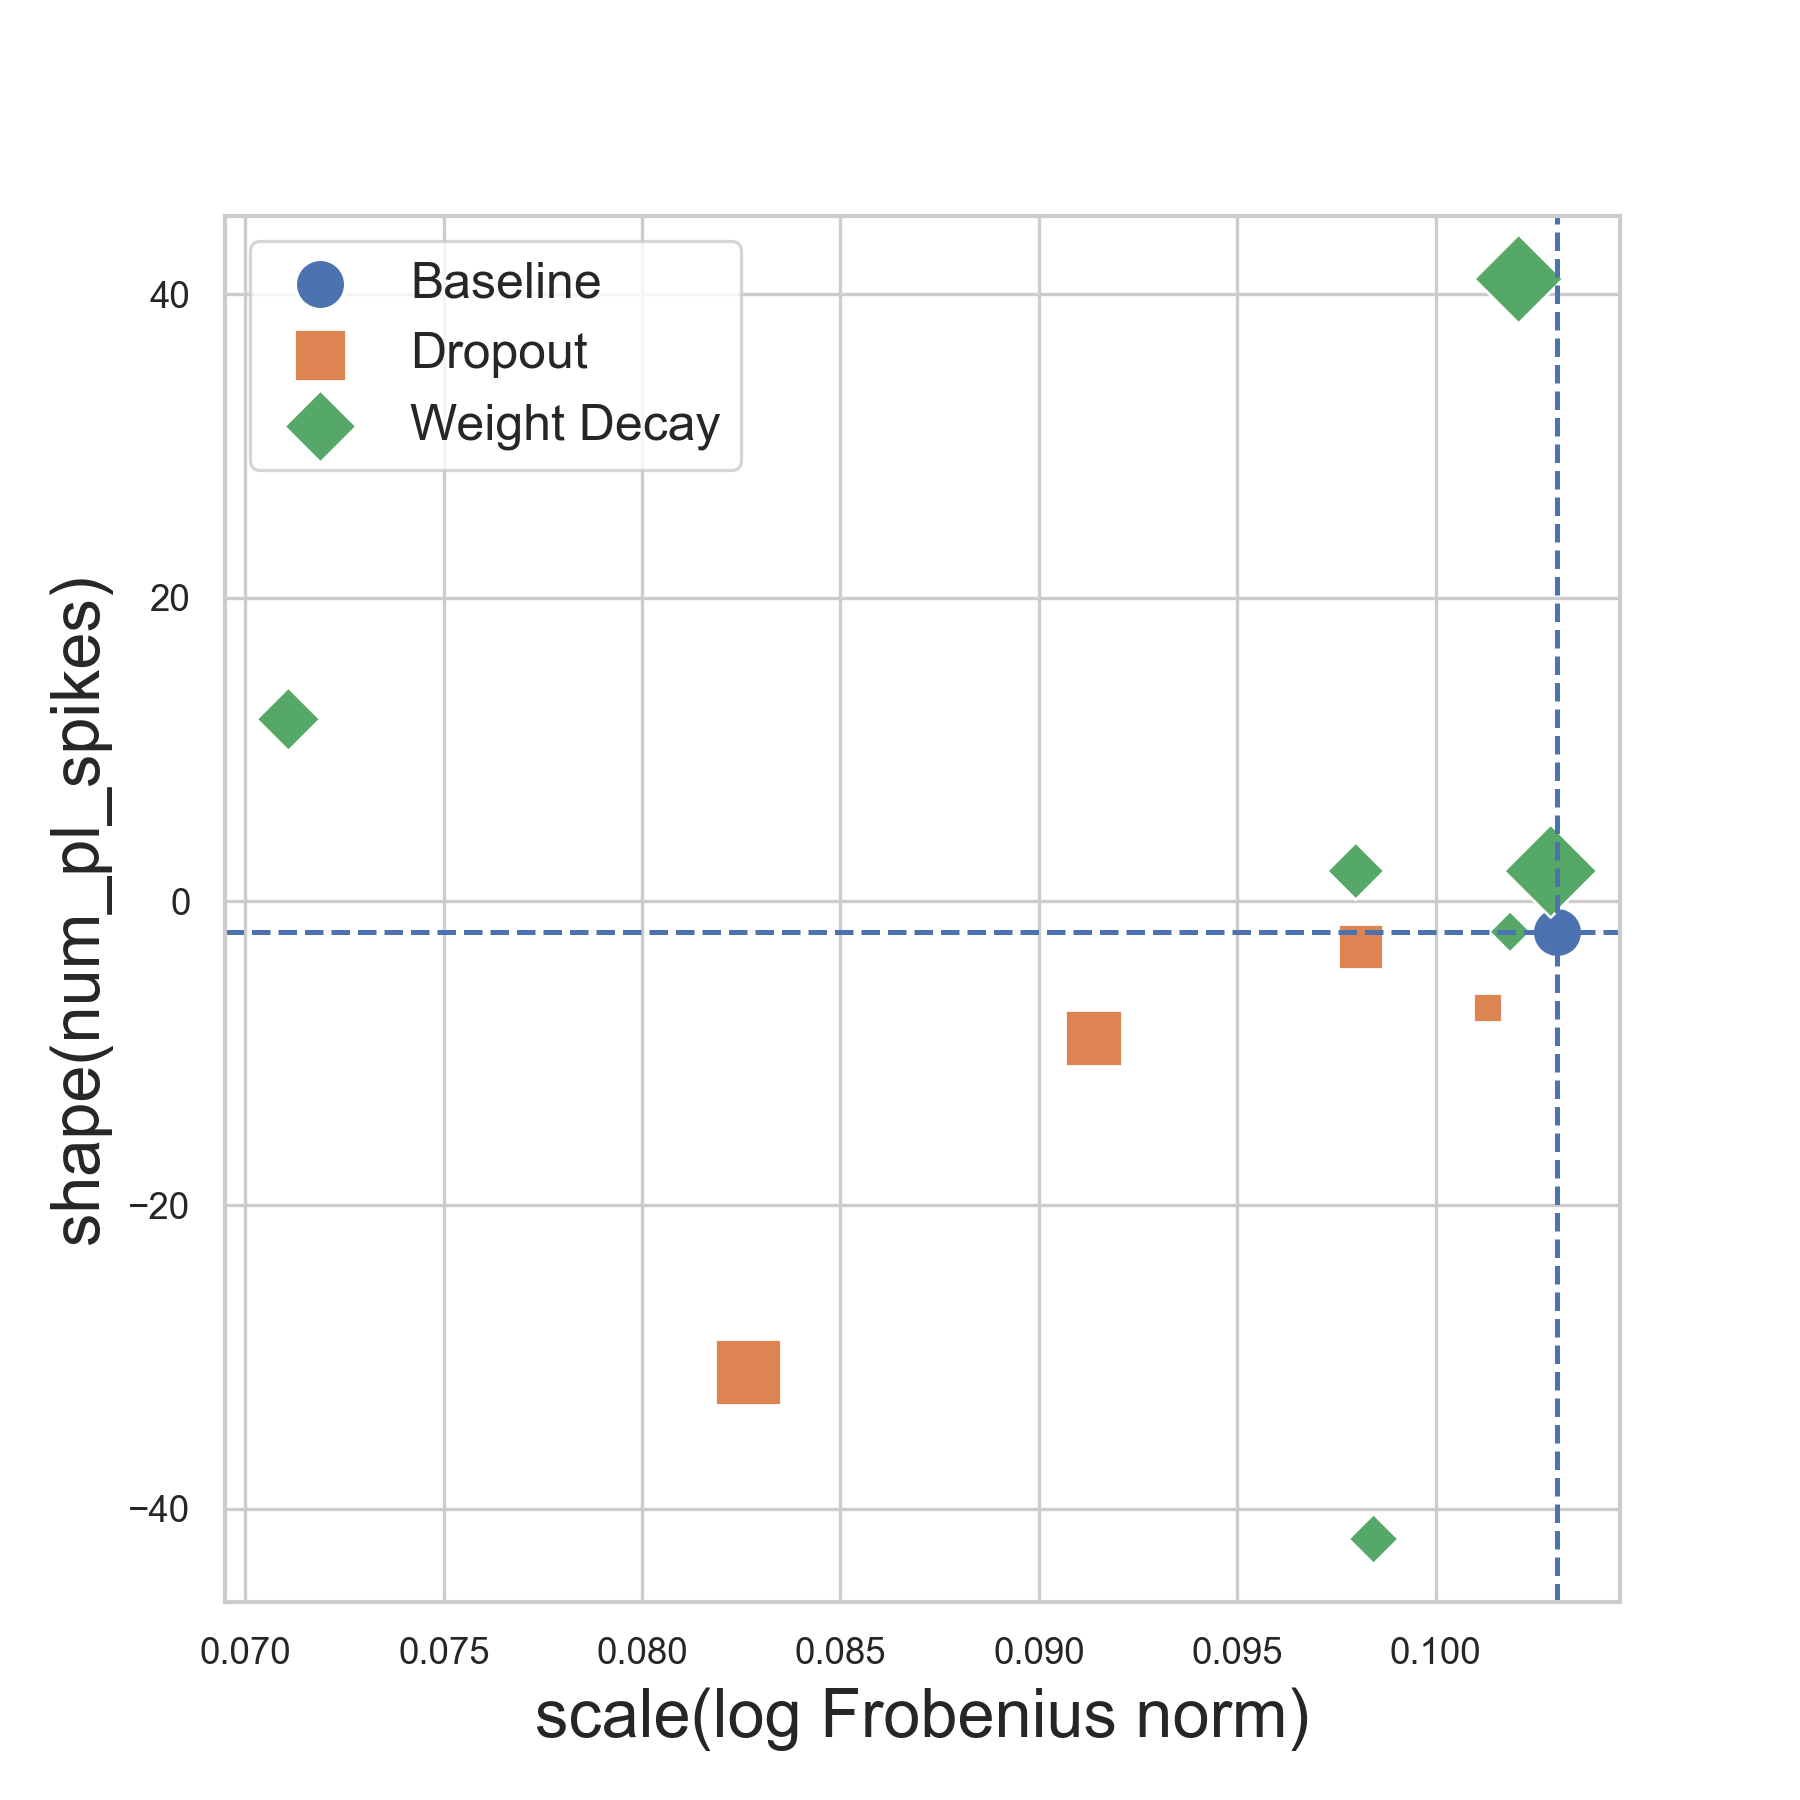}
        \caption{Frobenius vs. $\textit{num\_pl\_spikes}$ on CIFAR-100}
        \label{fig:reg-6}
    \end{subfigure}
    
    \caption{Various scale-shape plots of ESDs of the classifier layers on CIFAR-10 and CIFAR-100. The results are marked with square and diamond shapes for dropout and weight decay regularization techniques, respectively. The size of markers represents the magnitude of the dropout rate and weight decay values.}
    \label{fig:regularization-cl}
\end{figure}

\begin{figure}[h]
    \centering
    % First row
    \begin{subfigure}[b]{0.3\textwidth}
        \centering
        \includegraphics[width=\textwidth]{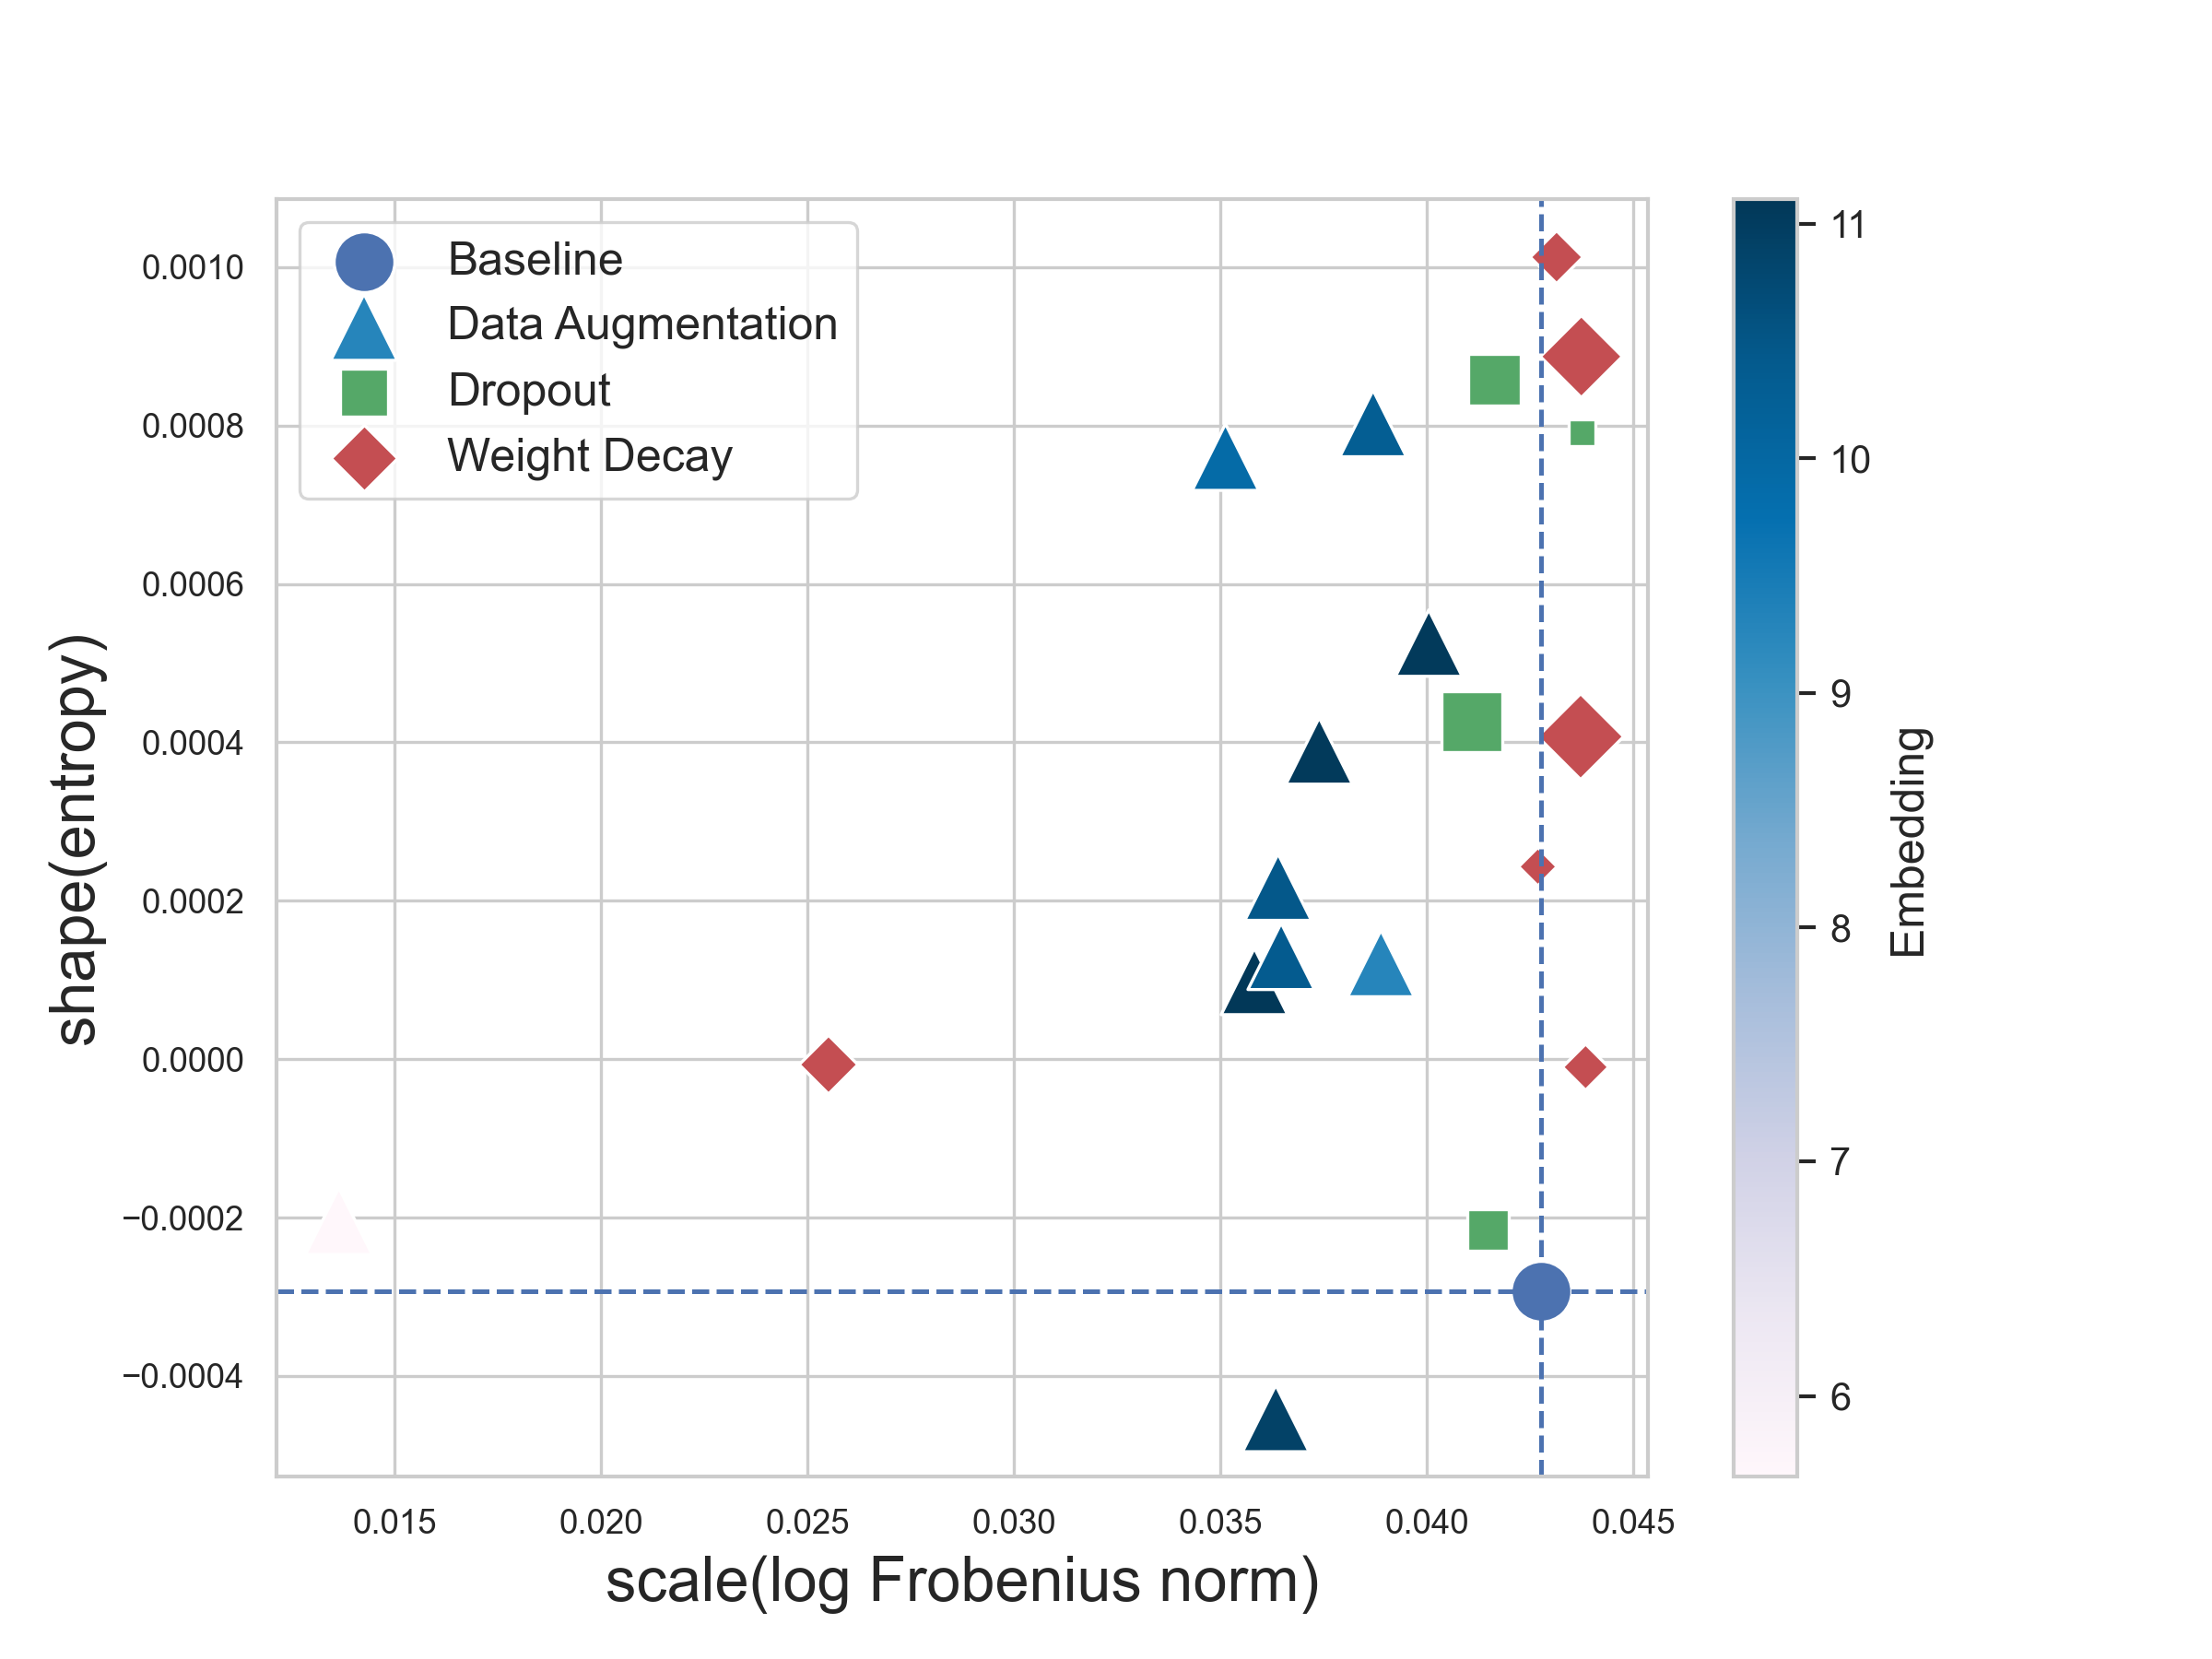}
        \caption{Frobenius norm vs. entropy on CIFAR-10}
        \label{fig:di1}
    \end{subfigure}
    \hfill
    \begin{subfigure}[b]{0.3\textwidth}
        \centering
        \includegraphics[width=\textwidth]{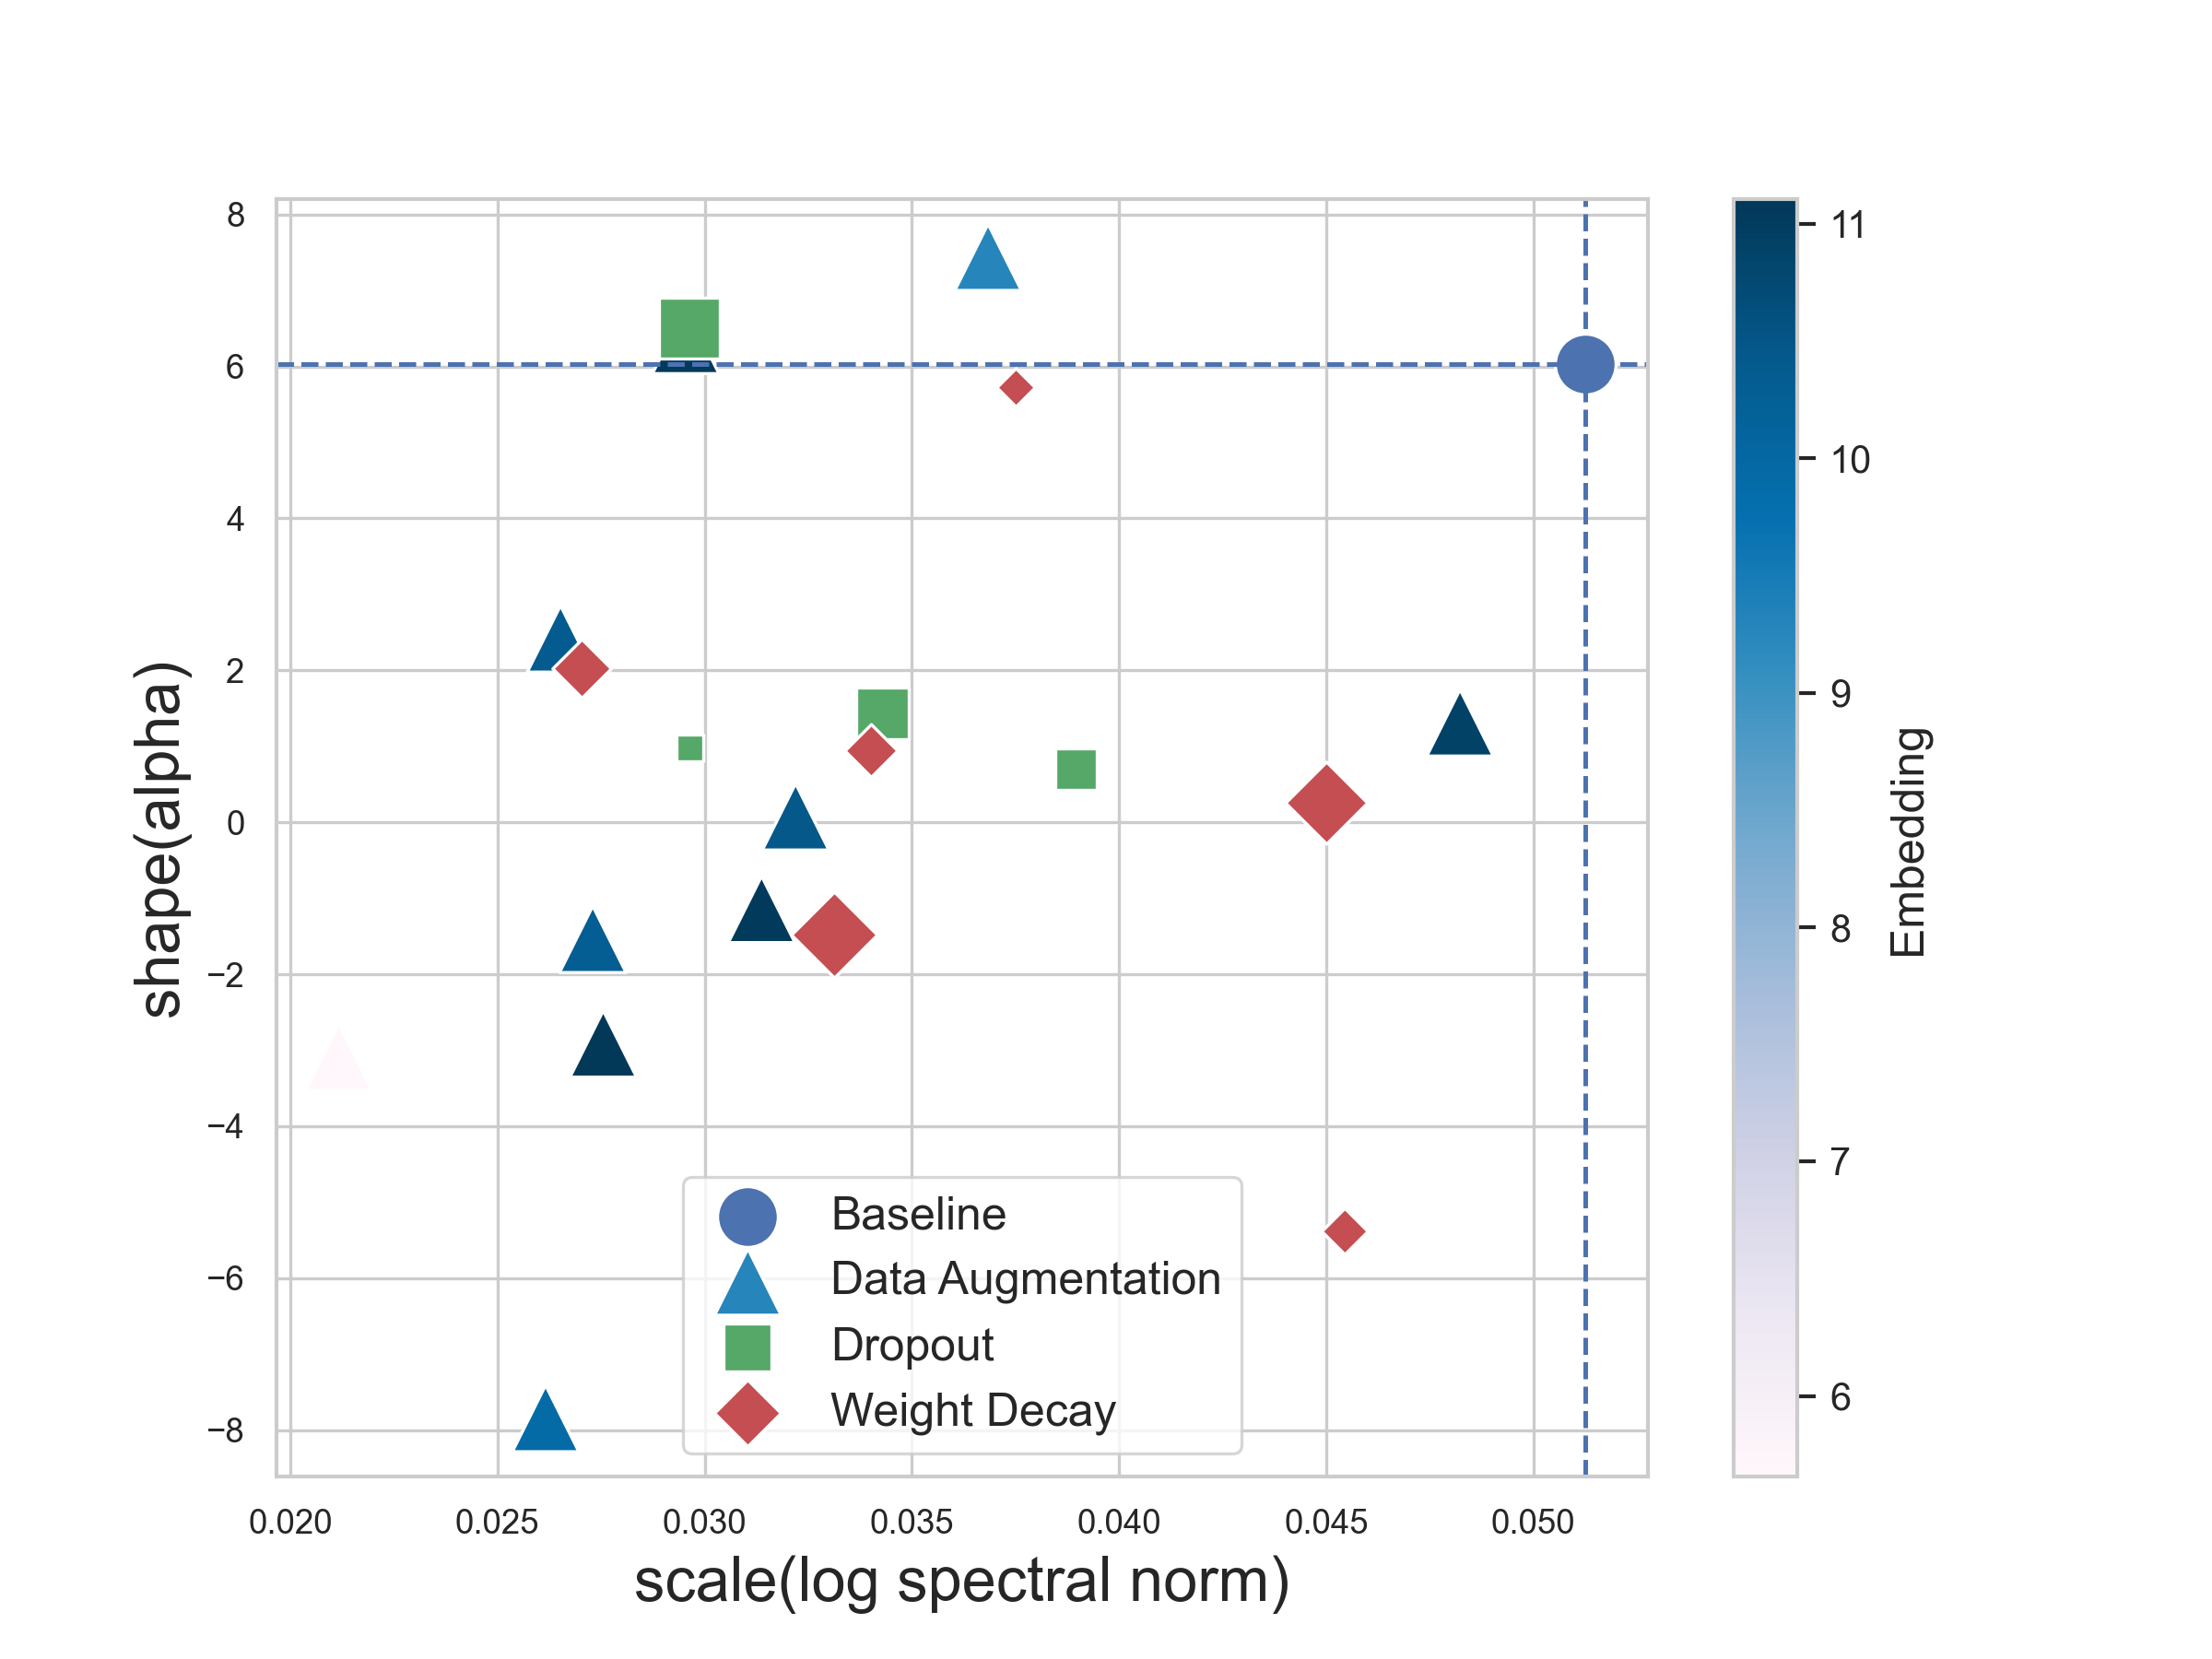}
        \caption{Spectral norm vs. alpha on CIFAR-10}
        \label{fig:di2}
    \end{subfigure}
    \hfill
    \begin{subfigure}[b]{0.3\textwidth}
        \centering
        \includegraphics[width=\textwidth]{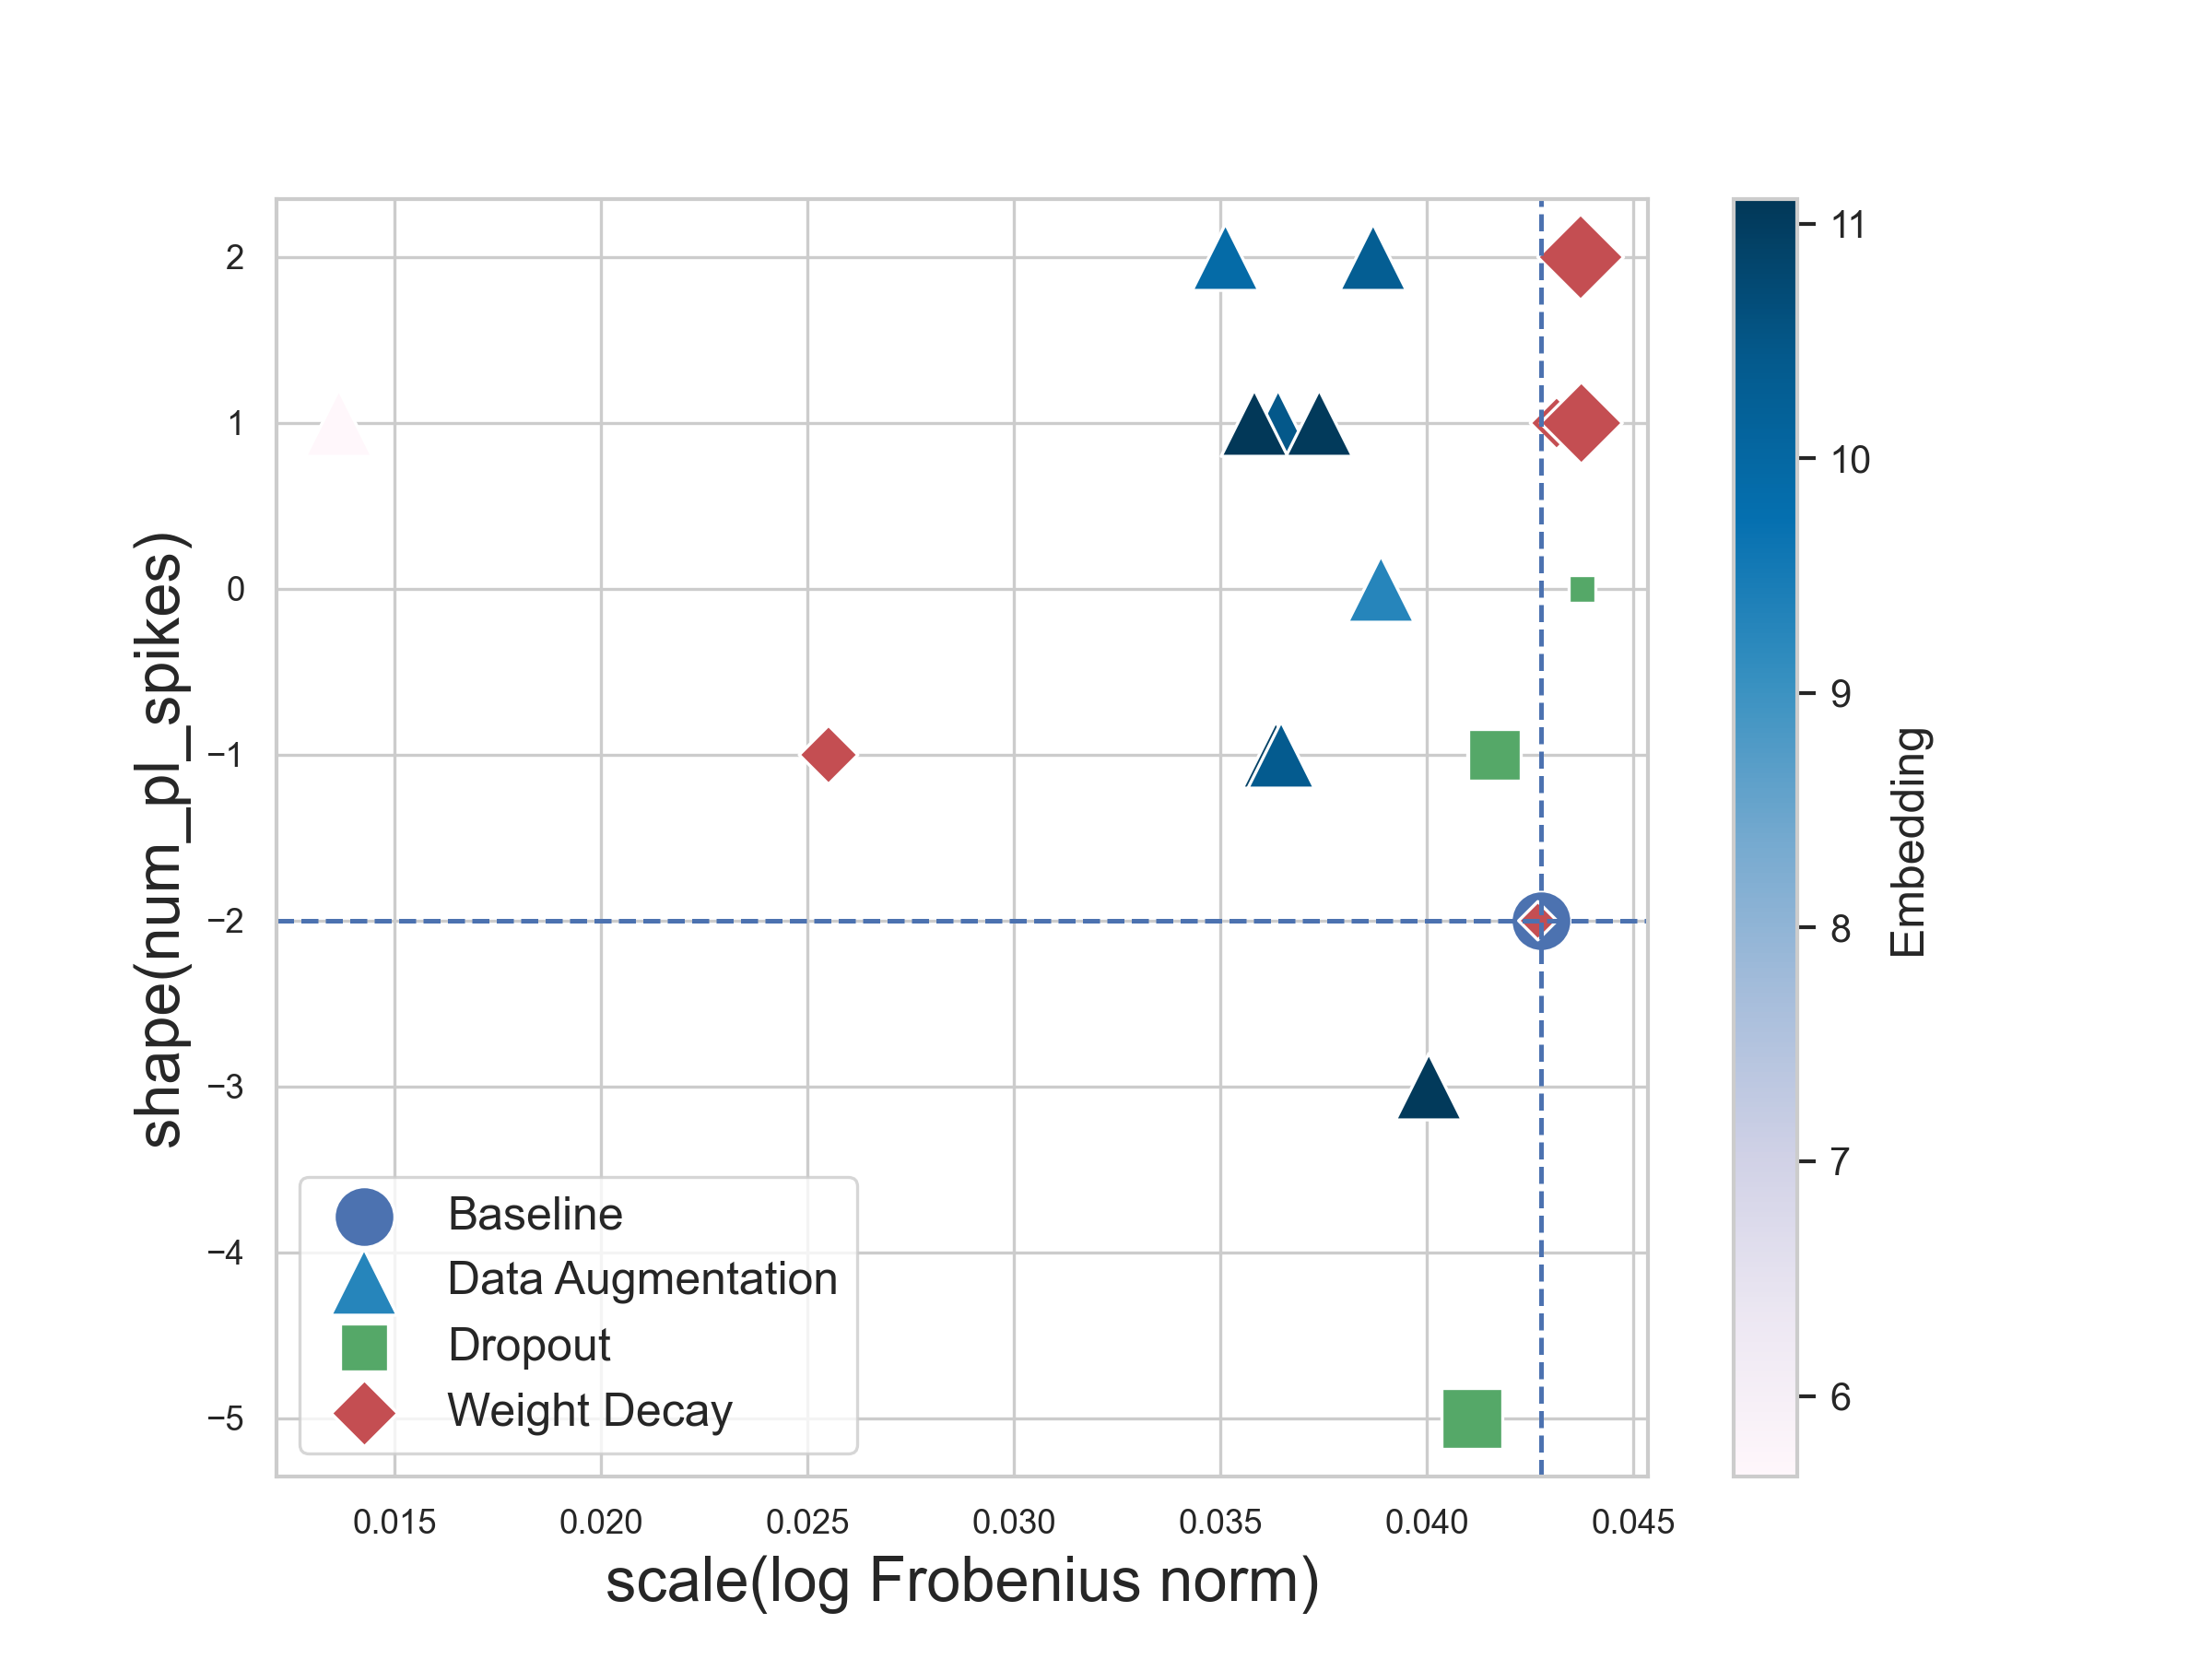}
        \caption{Frobenius vs. $\textit{num\_pl\_spikes}$ on CIFAR-10}
        \label{fig:di3}
    \end{subfigure}
    
    \vspace{1em} % Add some vertical space between rows
    
    % Second row
    \begin{subfigure}[b]{0.3\textwidth}
        \centering
        \includegraphics[width=\textwidth]{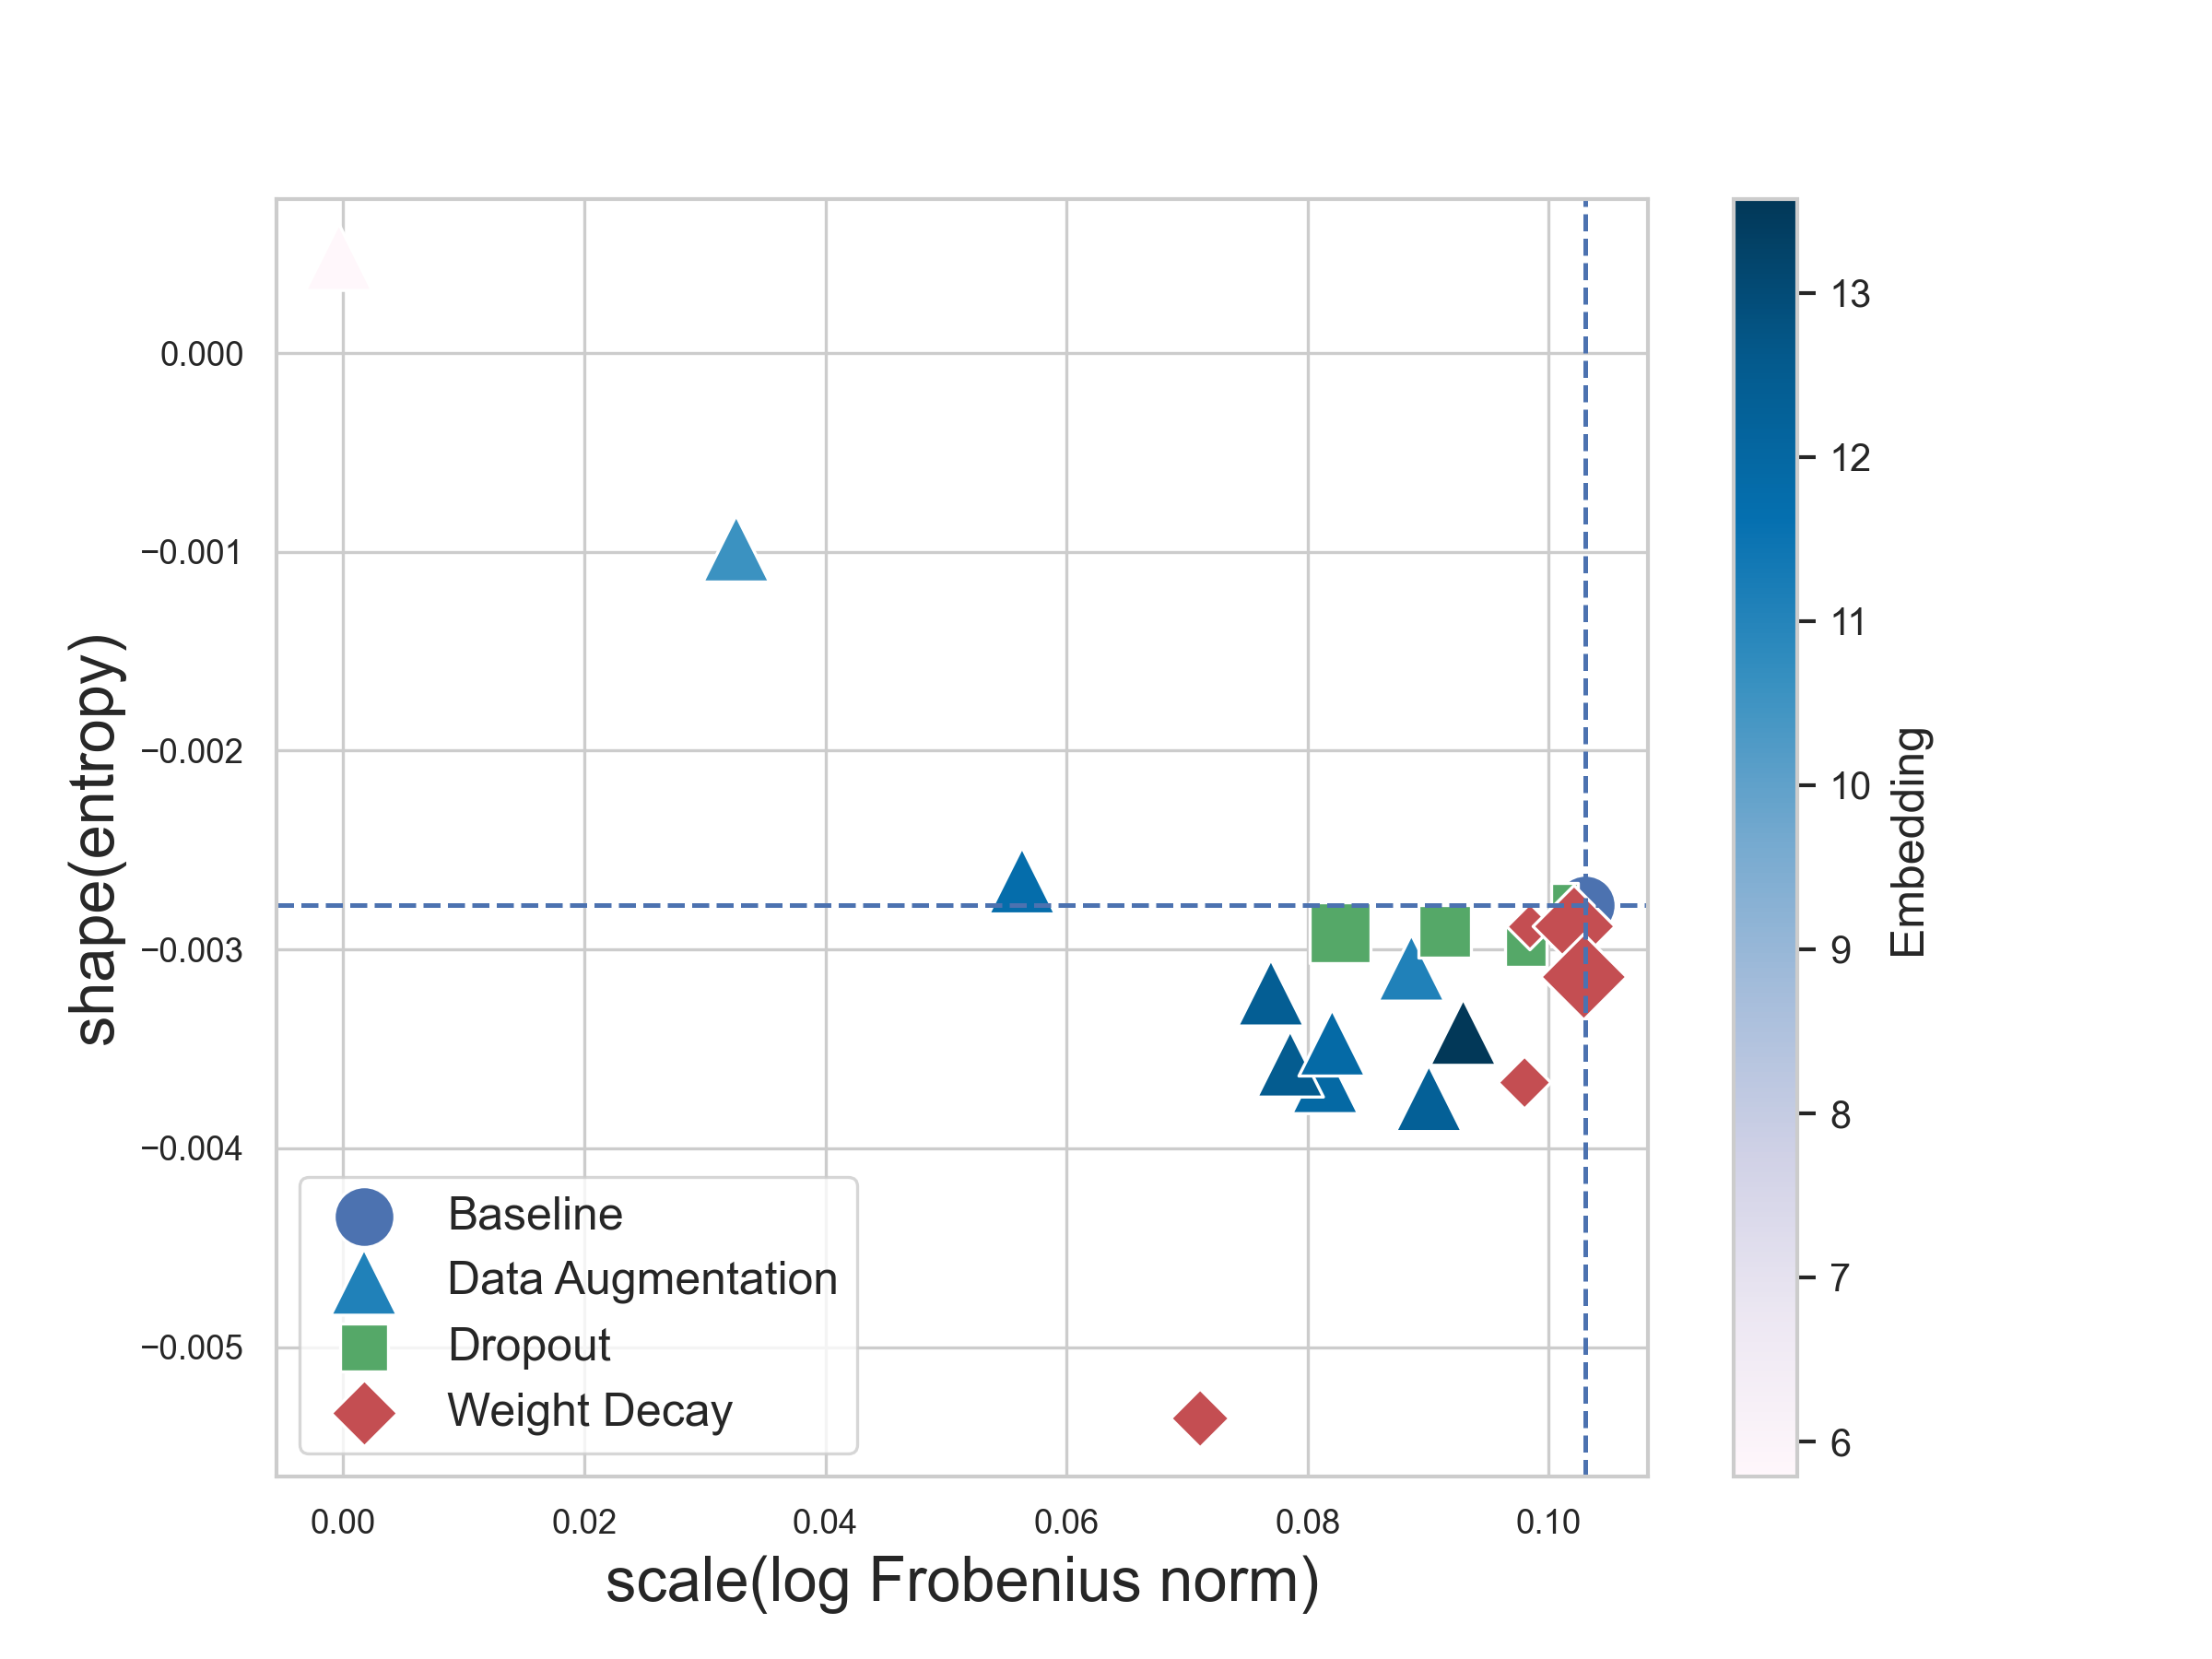}
        \caption{Frobenius norm vs. entropy on CIFAR-100}
        \label{fig:di4}
    \end{subfigure}
    \hfill
    \begin{subfigure}[b]{0.3\textwidth}
        \centering
        \includegraphics[width=\textwidth]{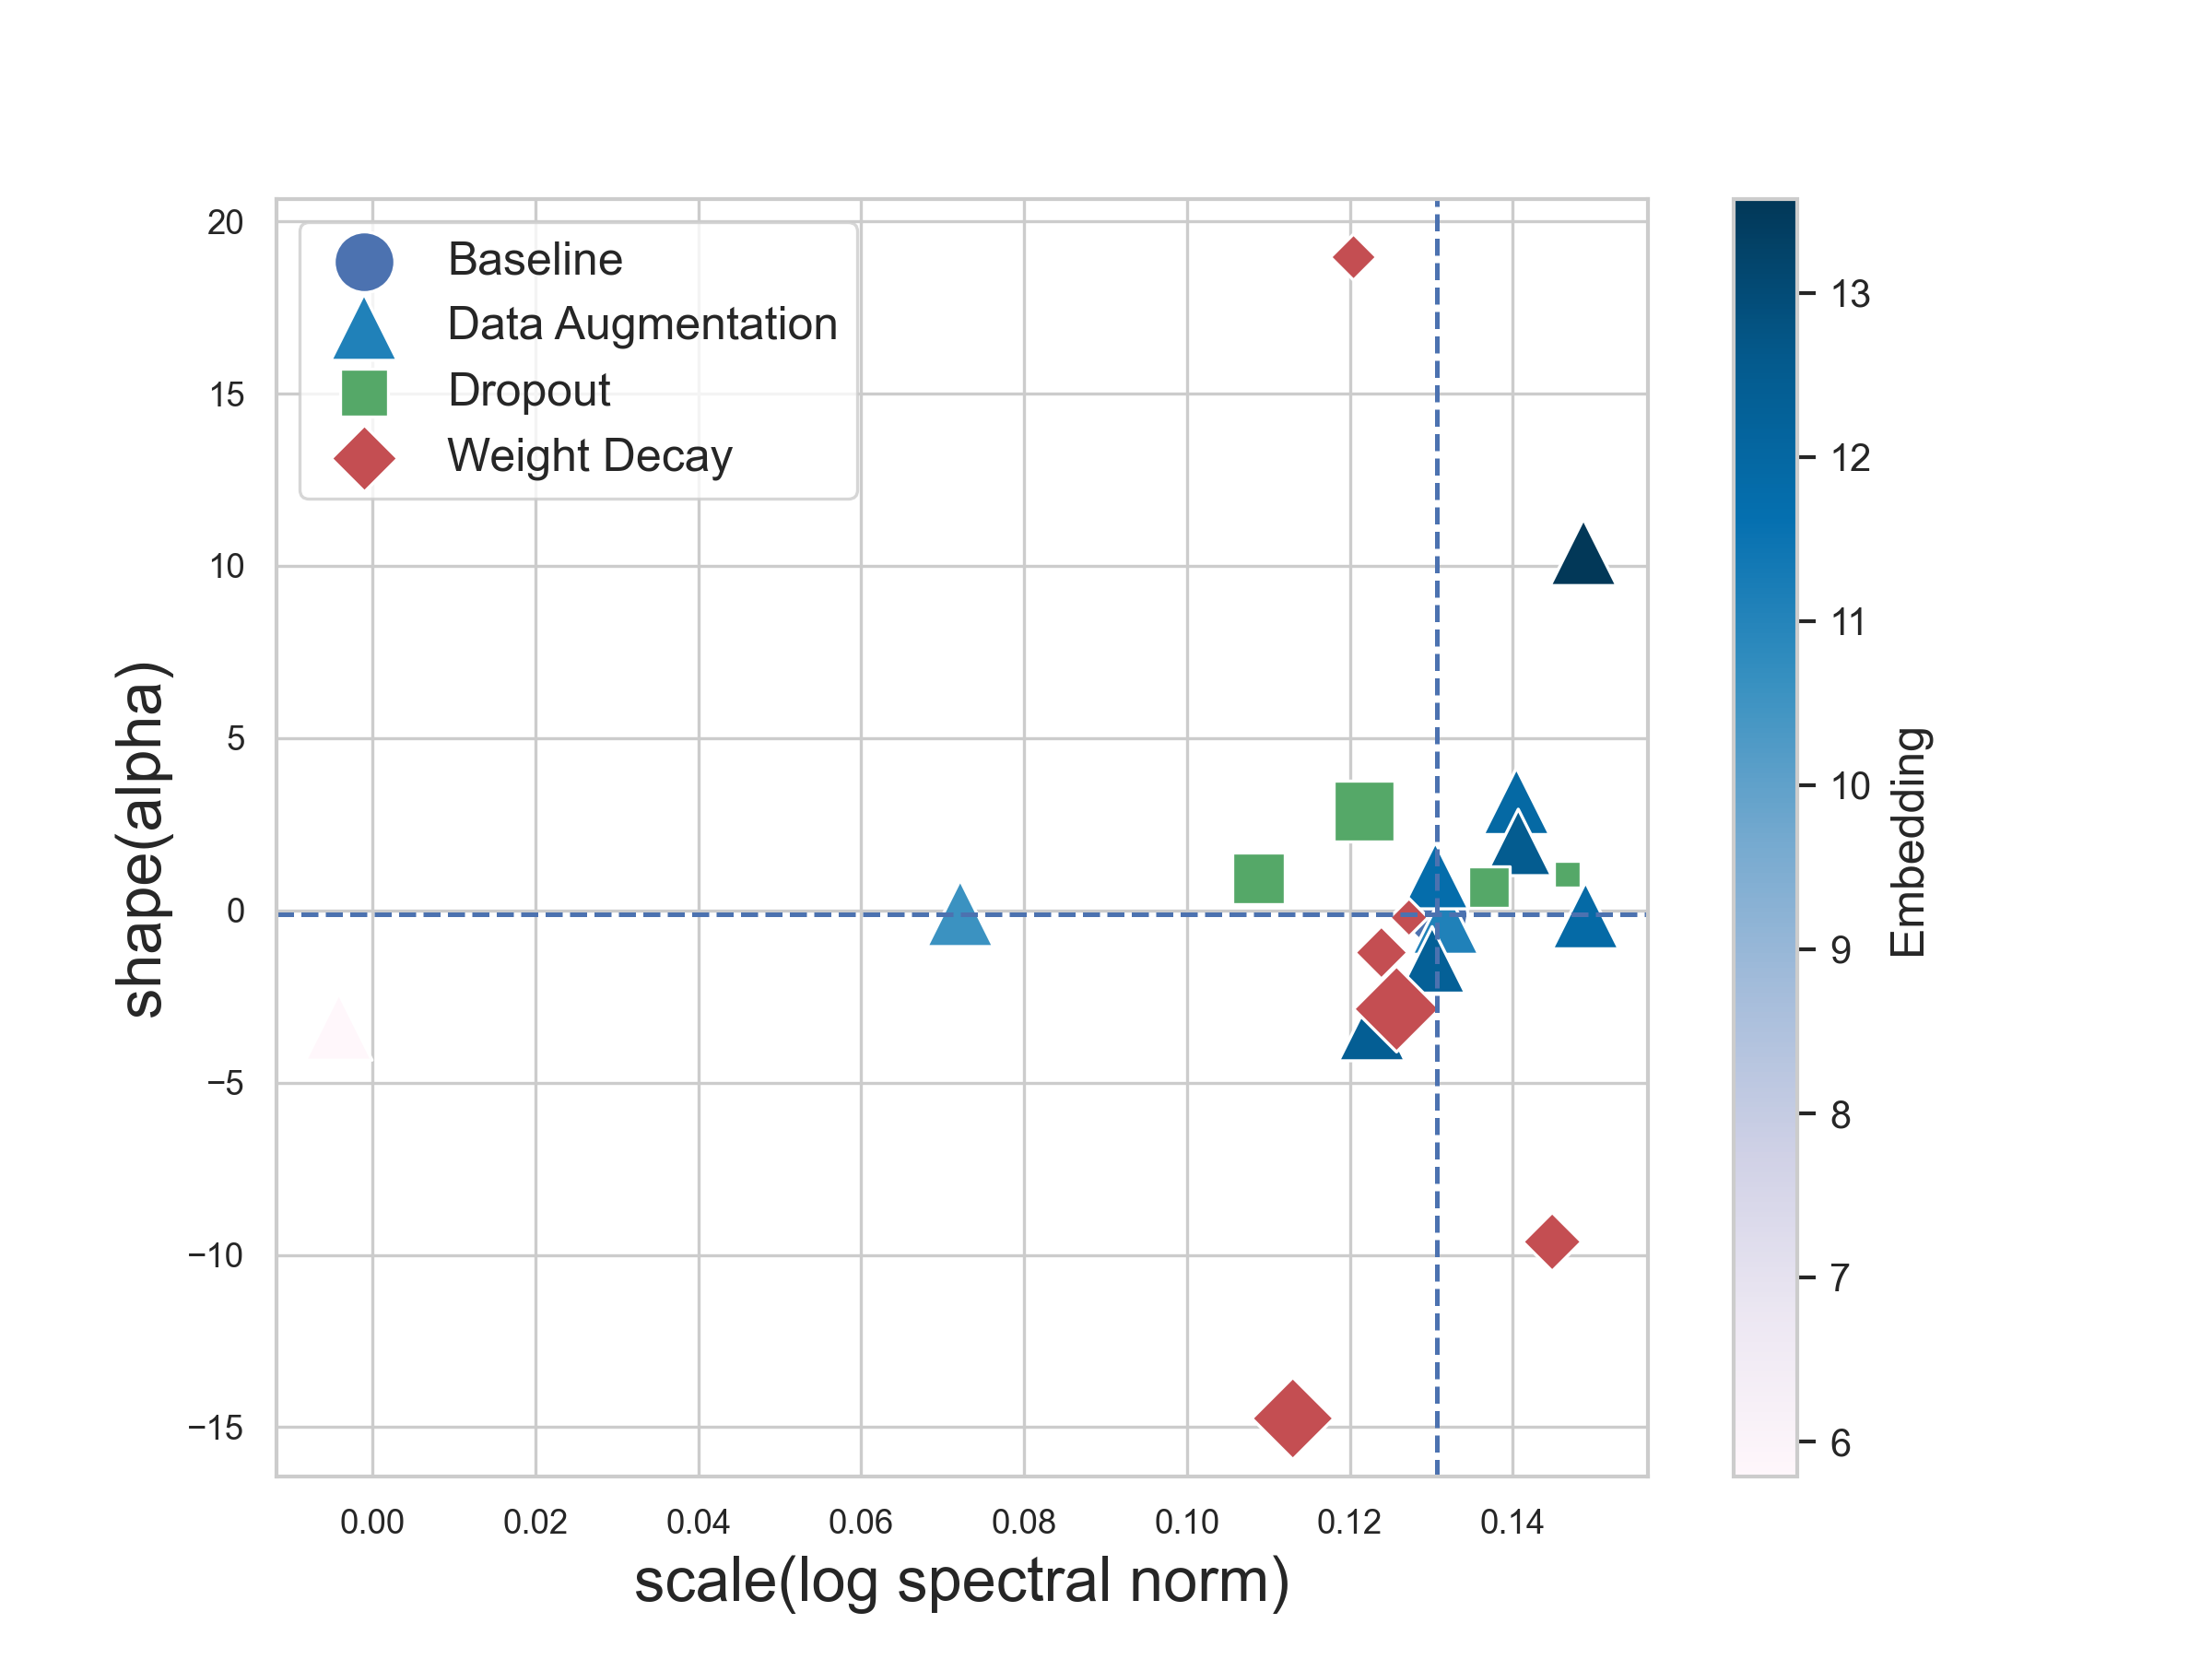}
        \caption{Spectral norm vs. alpha on CIFAR-100}
        \label{fig:di5}
    \end{subfigure}
    \hfill
    \begin{subfigure}[b]{0.3\textwidth}
        \centering
        \includegraphics[width=\textwidth]{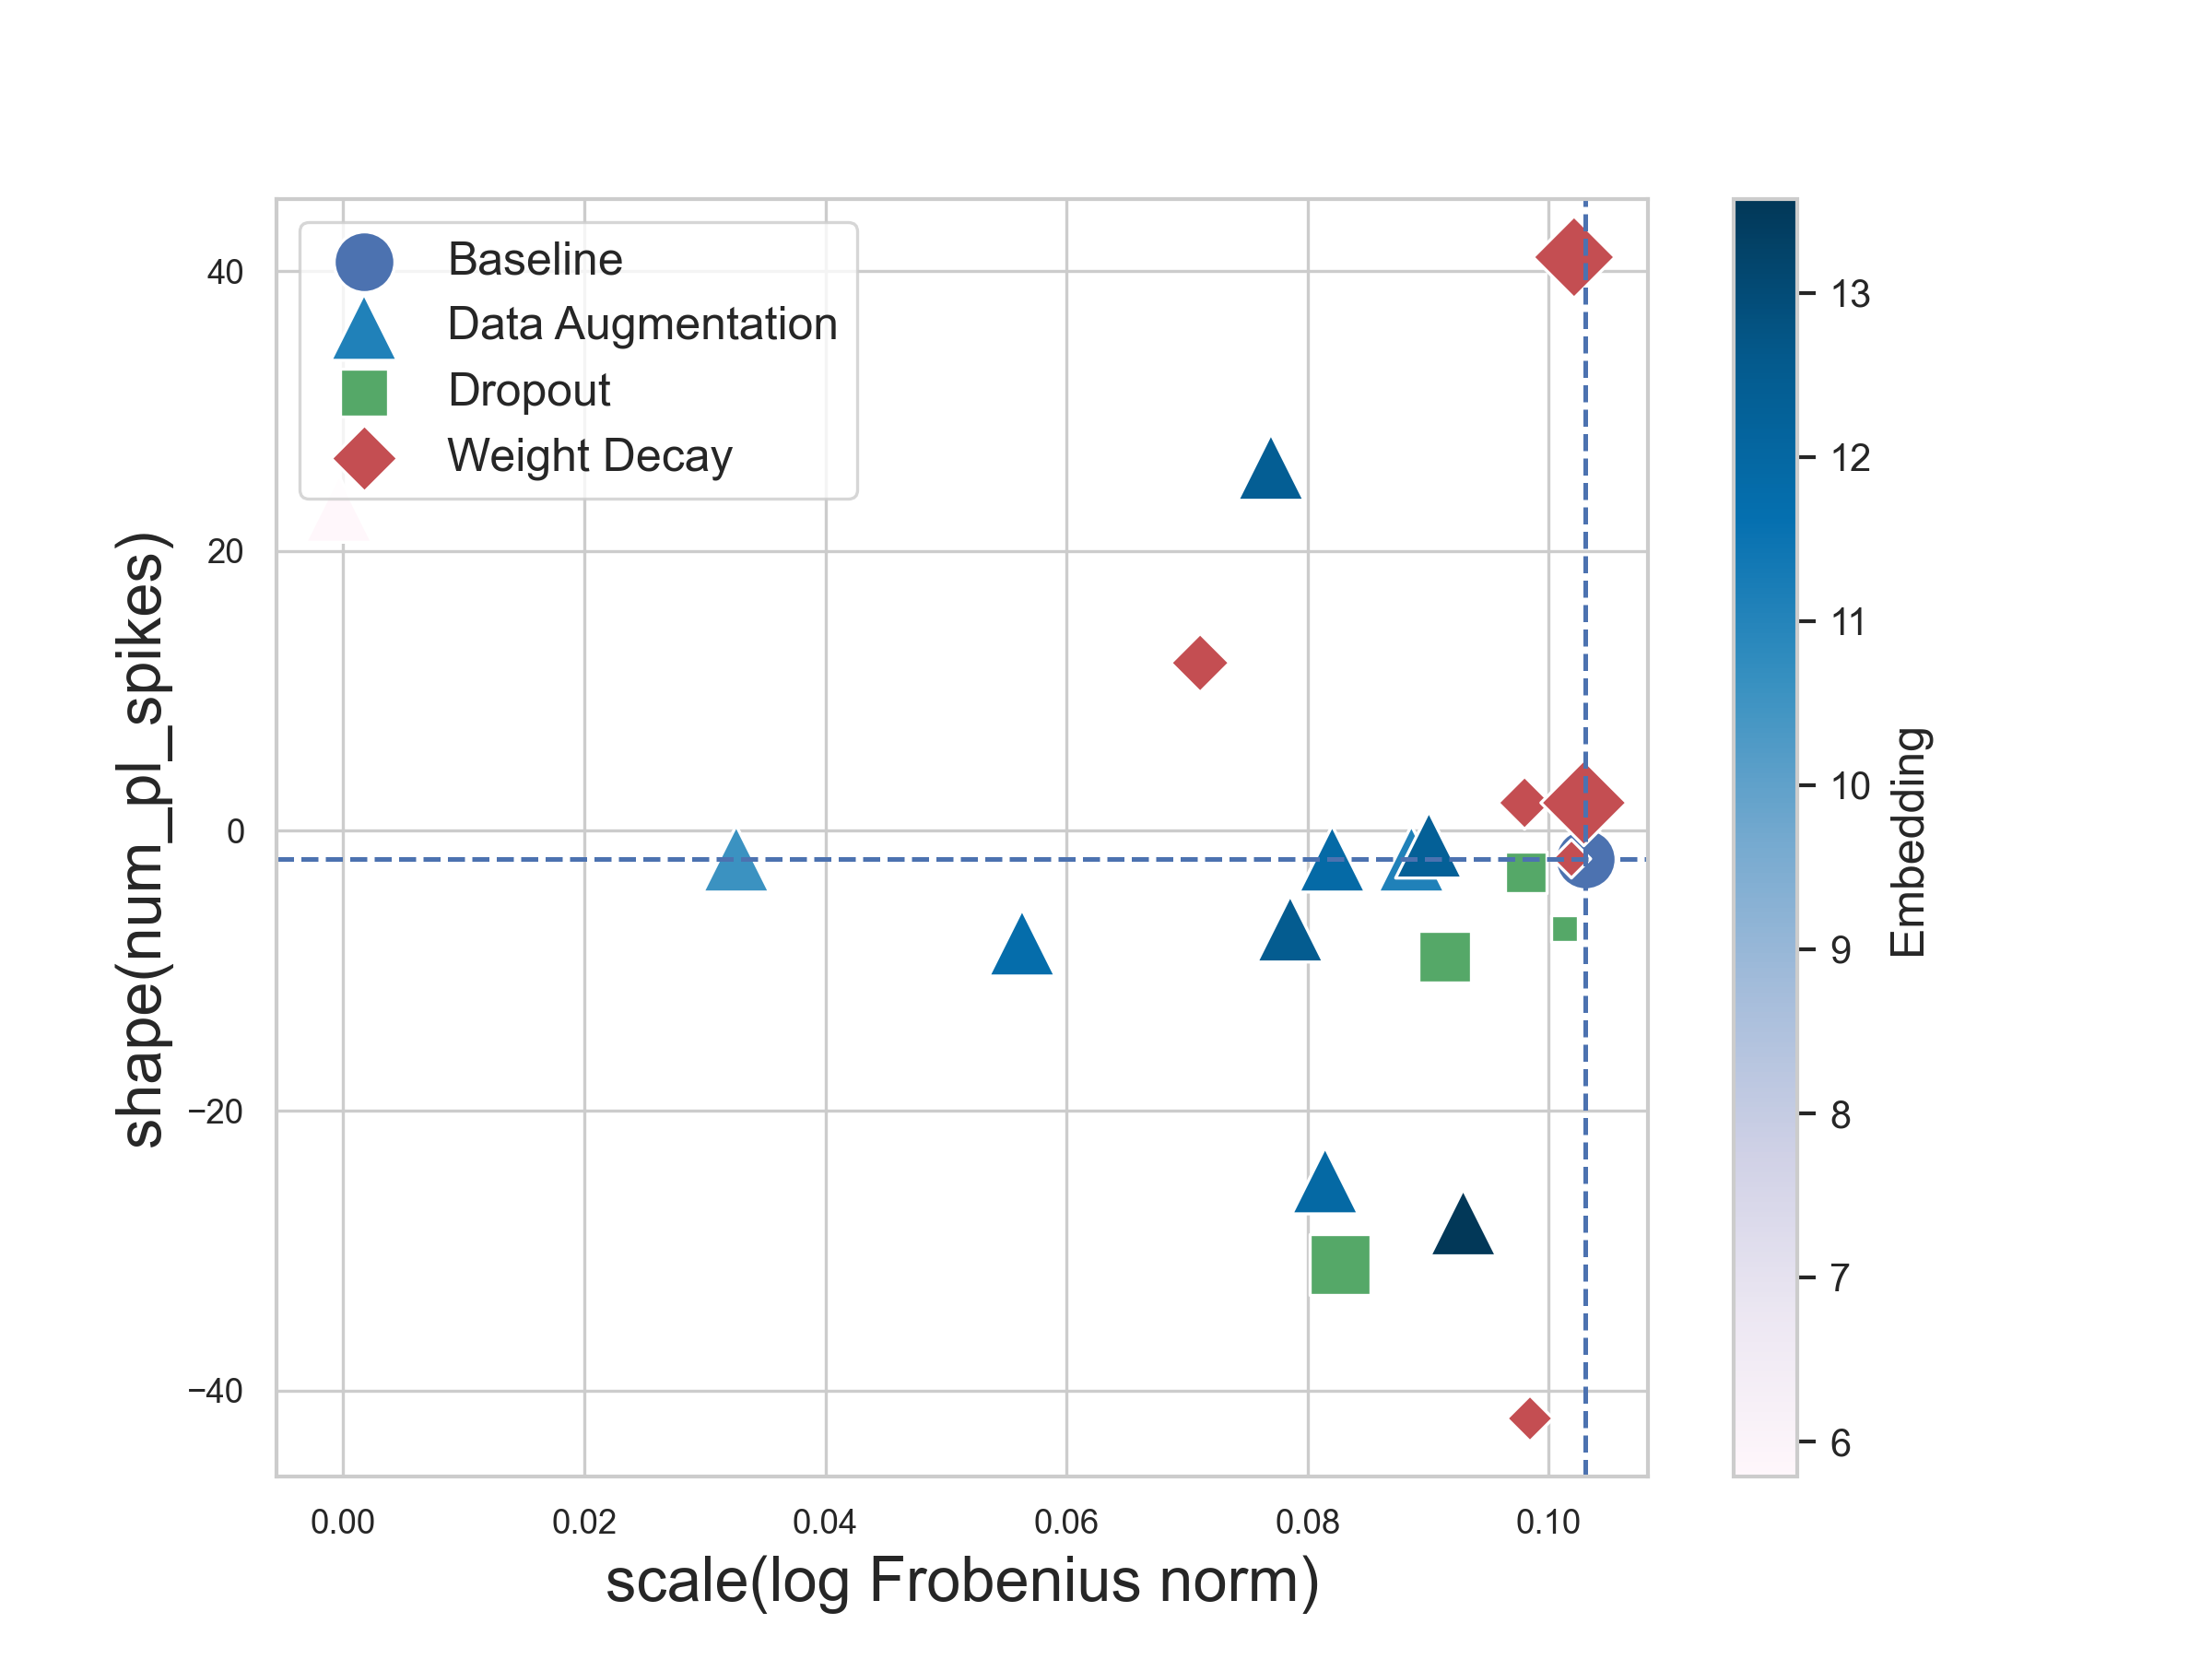}
        \caption{Frobenius vs. $\textit{num\_pl\_spikes}$ on CIFAR-100}
        \label{fig:di6}
    \end{subfigure}
    
    \caption{Various scale-shape plots of ESDs of the classifier layers on CIFAR-10 and CIFAR-100. The results are marked with triangle, square, and diamond shapes for data augmentation, dropout, and weight decay, respectively. The color intensity of triangles represents the magnitude of embedding-based diversity scores.}
    \label{fig:div-cl}
\end{figure}
