# Supplementary material for: Data Diversity as Implicit Regularization: How Does Diversity Shape the Weight Space of Deep Neural Networks?
Source: arXiv:2410.14602 source file (2025-08-15)
Supplement: Supplementary file 5 [file appendix6.tex]

\label{appendix:visual}

% \begin{figure*}[ht]
%     % \centering
%     % First subfigure (left column)
%     \begin{subfigure}
%         \centering
%         \includegraphics[width=0.24\textwidth]{fig/bert/bert_alpha_diff_bert_div_line.png}
%         % \caption{Logarithmic scale}\input{sections/4.related_work}
%         \label{fig:a1}
%     \end{subfigure}
%     % \vfill
%     % Second subfigure (right column)
%     \begin{subfigure}
%         \centering
%         \includegraphics[width=0.24\textwidth]{fig/bert/bert_entropy_diff_bert_div_line.png}
%         % \caption{Linear scale}
%         \label{fig:a2}
%     \end{subfigure}
%     % \vfill
%     \begin{subfigure}
%         \centering
%         \includegraphics[width=0.24\textwidth]{fig/bert/bert_log_norm_diff_bert_div_line.png}
%         % \caption{Linear scale}
%         \label{fig:a3}
%     \end{subfigure}
%     \begin{subfigure}
%         \centering
%         \includegraphics[width=0.24\textwidth]{fig/bert/bert_log_spectral_norm_diff_bert_div_line.png}
%         % \caption{Linear scale}
%         \label{fig:a4}
%     \end{subfigure}
    
%     \caption{Spectral Metrics Changes through layers}

% \end{figure*}
