# Supplementary material for: Data Diversity as Implicit Regularization: How Does Diversity Shape the Weight Space of Deep Neural Networks?
Source: arXiv:2410.14602 source file (2025-08-15)
Supplement: Supplementary file 6 [file appendix7.tex]

\label{appendix:id-ood_ece}

\begin{table*}[h]
\resizebox{\textwidth}{!}{
\begin{tabular}{l c *{4}{c} c | c *{3}{c} c}
\hline
\multicolumn{7}{c|}{\textbf{DomainNet}} & \multicolumn{5}{c}{\textbf{Office-Home}} \\
\hline
& \textbf{ID} & \multicolumn{4}{c}{\textbf{OOD}} & \textbf{AVG} & \textbf{ID} & \multicolumn{3}{c}{\textbf{OOD}} & \textbf{AVG} \\
\cline{2-12}
\multirow{2}{*}[0.5em]{} & \multirow{2}{*}{ECE} & \multicolumn{1}{c}{Clipart} & \multicolumn{1}{c}{Infograph} & \multicolumn{1}{c}{Painting} & \multicolumn{1}{c}{Sketch} & \multirow{2}{*}{ECE} & \multirow{2}{*}{ECE} & \multicolumn{1}{c}{Clipart} & \multicolumn{1}{c}{Product} & \multicolumn{1}{c}{Art} & \multirow{2}{*}{ECE} \\
\cline{3-6} \cline{9-11}
& & ECE & ECE & ECE & ECE & & & ECE & ECE & ECE & \\
\hline
Baseline &  0.016 & 0.179 & 0.320 & 0.136 & 0.168 & 0.201 &  \textbf{0.030} & 0.162 &  0.028 & 0.068 &0.086 \\
DP01 & 0.018 & 0.194 &  0.334&  0.148 & 0.184 & 0.215&  0.043 &  0.181&  0.029&   0.050&  0.087\\
DP03 & 0.019 &  0.197 &  0.318 & 0.155 & 0.187& 0.214 & 0.054 &0.150 & 0.030 & 0.035 & 0.072 \\
DP05 & 0.020 & 0.183 & 0.332 &  0.167 & 0.184 & 0.217 &  0.068& 0.091 & 0.037 & \textbf{0.028}  & \textbf{0.052} \\
DP07 & 0.019 & 0.207& 0.310 & 0.156 &  0.191&  0.216 &  0.082&  \textbf{0.066}&  0.055 &  0.060& 0.060 \\
WD1e-05 &  0.021 & 0.205 & 0.376 & 0.154 & 0.198 & 0.233 &  0.034 &0.121 & \textbf{0.021} & 0.058 & 0.067\\
WD5e-05 &  0.018 &  0.168 & 0.329 & 0.132 & 0.137 &  0.192& 0.037 & 0.136 &  0.032&  0.059& 0.076 \\
WD1e-4 & 0.026 & 0.151 &  0.354 &  0.154 & 0.128  & 0.197 &  0.050& 0.166 & 0.026 & 0.061 & 0.084\\
WD5e-4 &0.024 &  0.193&  0.340&   0.141 &  0.154  & 0.207 &  0.043& 0.171 & 0.029 & 0.046 &0.082 \\
WD1e-3 &  0.023& 0.143 &  0.303 &  0.141 & 0.142 &  0.182&  0.038&  0.158 &  \textbf{0.021} &  0.051 &0.077 \\
WD5e-3 & \textbf{0.015} &   0.196 &  0.400 &   0.165& 0.153 & 0.229 &  0.041&  0.177 & 0.036 & 0.058 &  0.09\\
Auto & 0.025&  0.197& 0.416 &  0.164 & 0.194 & 0.243 & 0.040 &  0.192 & 0.035 & 0.066 & 0.098\\
Rand &  0.022& 0.195 &  0.322 &  0.125 & 0.127 & 0.192 &  0.056 & 0.205 &  0.026&0.069  & 0.100 \\
AugM &  0.021 & 0.198 & 0.373 &  0.157 & 0.187 & 0.229 & 0.044 &  0.148&  0.029 & 0.050 &  0.076\\
TrAu &  0.023 &\textbf{0.135} &   0.323 & \textbf{0.116}  &  \textbf{0.119} & \textbf{0.173} & 0.034 & 0.147 & 0.041 &  0.064& 0.084 \\
Noise10 &  0.021 & 0.169 & 0.354 & 0.130 & 0.158 & 0.203& 0.046 & 0.141 & \textbf{0.025} & 0.062 & \textbf{0.076} \\
Noise30 &  0.024 & 0.207 & 0.309 & 0.141 & 0.156 & 0.203& 0.041 &0.156 & 0.036& 0.057 & 0.081 \\
Noise50 & \textbf{0.016} &   0.142&   \textbf{0.267} &0.149 &  0.145& 0.176 & 0.049 &  0.139 & 0.027 & 0.068 & 0.078 \\
Auto-v1 & 0.020 & 0.178 &  0.338 & 0.173 & 0.188 & 0.219 &  0.056& 0.168&  0.026 &  0.079 &  0.091\\
Auto-v2 & 0.022& 0.136 & 0.361 &  0.122& 0.128 & 0.187 & 0.046 &  0.168 & 0.033& 0.070 &  0.09\\
Auto-v3 &  0.021& 0.169 & 0.362 &0.140  & 0.153 & 0.206 &  \textbf{0.034} &  0.137 & 0.035 & 0.065 & 0.077 \\
\hline
\end{tabular}
\label{tab-id-ood-ECE}
}
\caption{Expected Calibration Error (ECE) quantifies how well a model's predicted probabilities (confidence) align with its actual outcomes (accuracy) \citep{guo2017calibration}. \textbf{The smaller the ECE is, the better the model is calibrated.} This table shows ECE valuations for both in-distribution (ID) and out-of-distribution (OOD) tasks. Both tables present the results from fine-tuning CLIP with a ResNet-50 backbone. The left table shows the results for training and
testing on the DomainNet dataset, while the right table displays the results for the Office-Home dataset. \textbf{Data augmentation demonstrates superior performance in model calibration on DomainNet for both ID and OOD scenarios. However, on the Office-Home dataset, dropout achieves the best performance, despite data augmentation outperforming the baseline.}}
\label{tab-id-ood-more}
\end{table*}
